# Supplementary material for: FlashP: An Analytical Pipeline for Real-time Forecasting of Time-Series Relational Data
Source: arXiv:2101.03298 source file (2021-01-16)
Supplement: Supplementary file 1 [file paper-appendix.tex]

%!TEX root = paper.tex

All the figures are here:

%%=================performance expr=================
%%total 150 days including 2067386455 rows and 305081814 users, time unit is millseconds
%%=============================================
%-----ARIMA+AQP time----------
\begin{figure*}[ht]
\begin{minipage}[t]{0.33\linewidth}
\subfigure[Selectivity 0.5\%]{
\centering
\includegraphics[width=2.2in, height=2.0in]{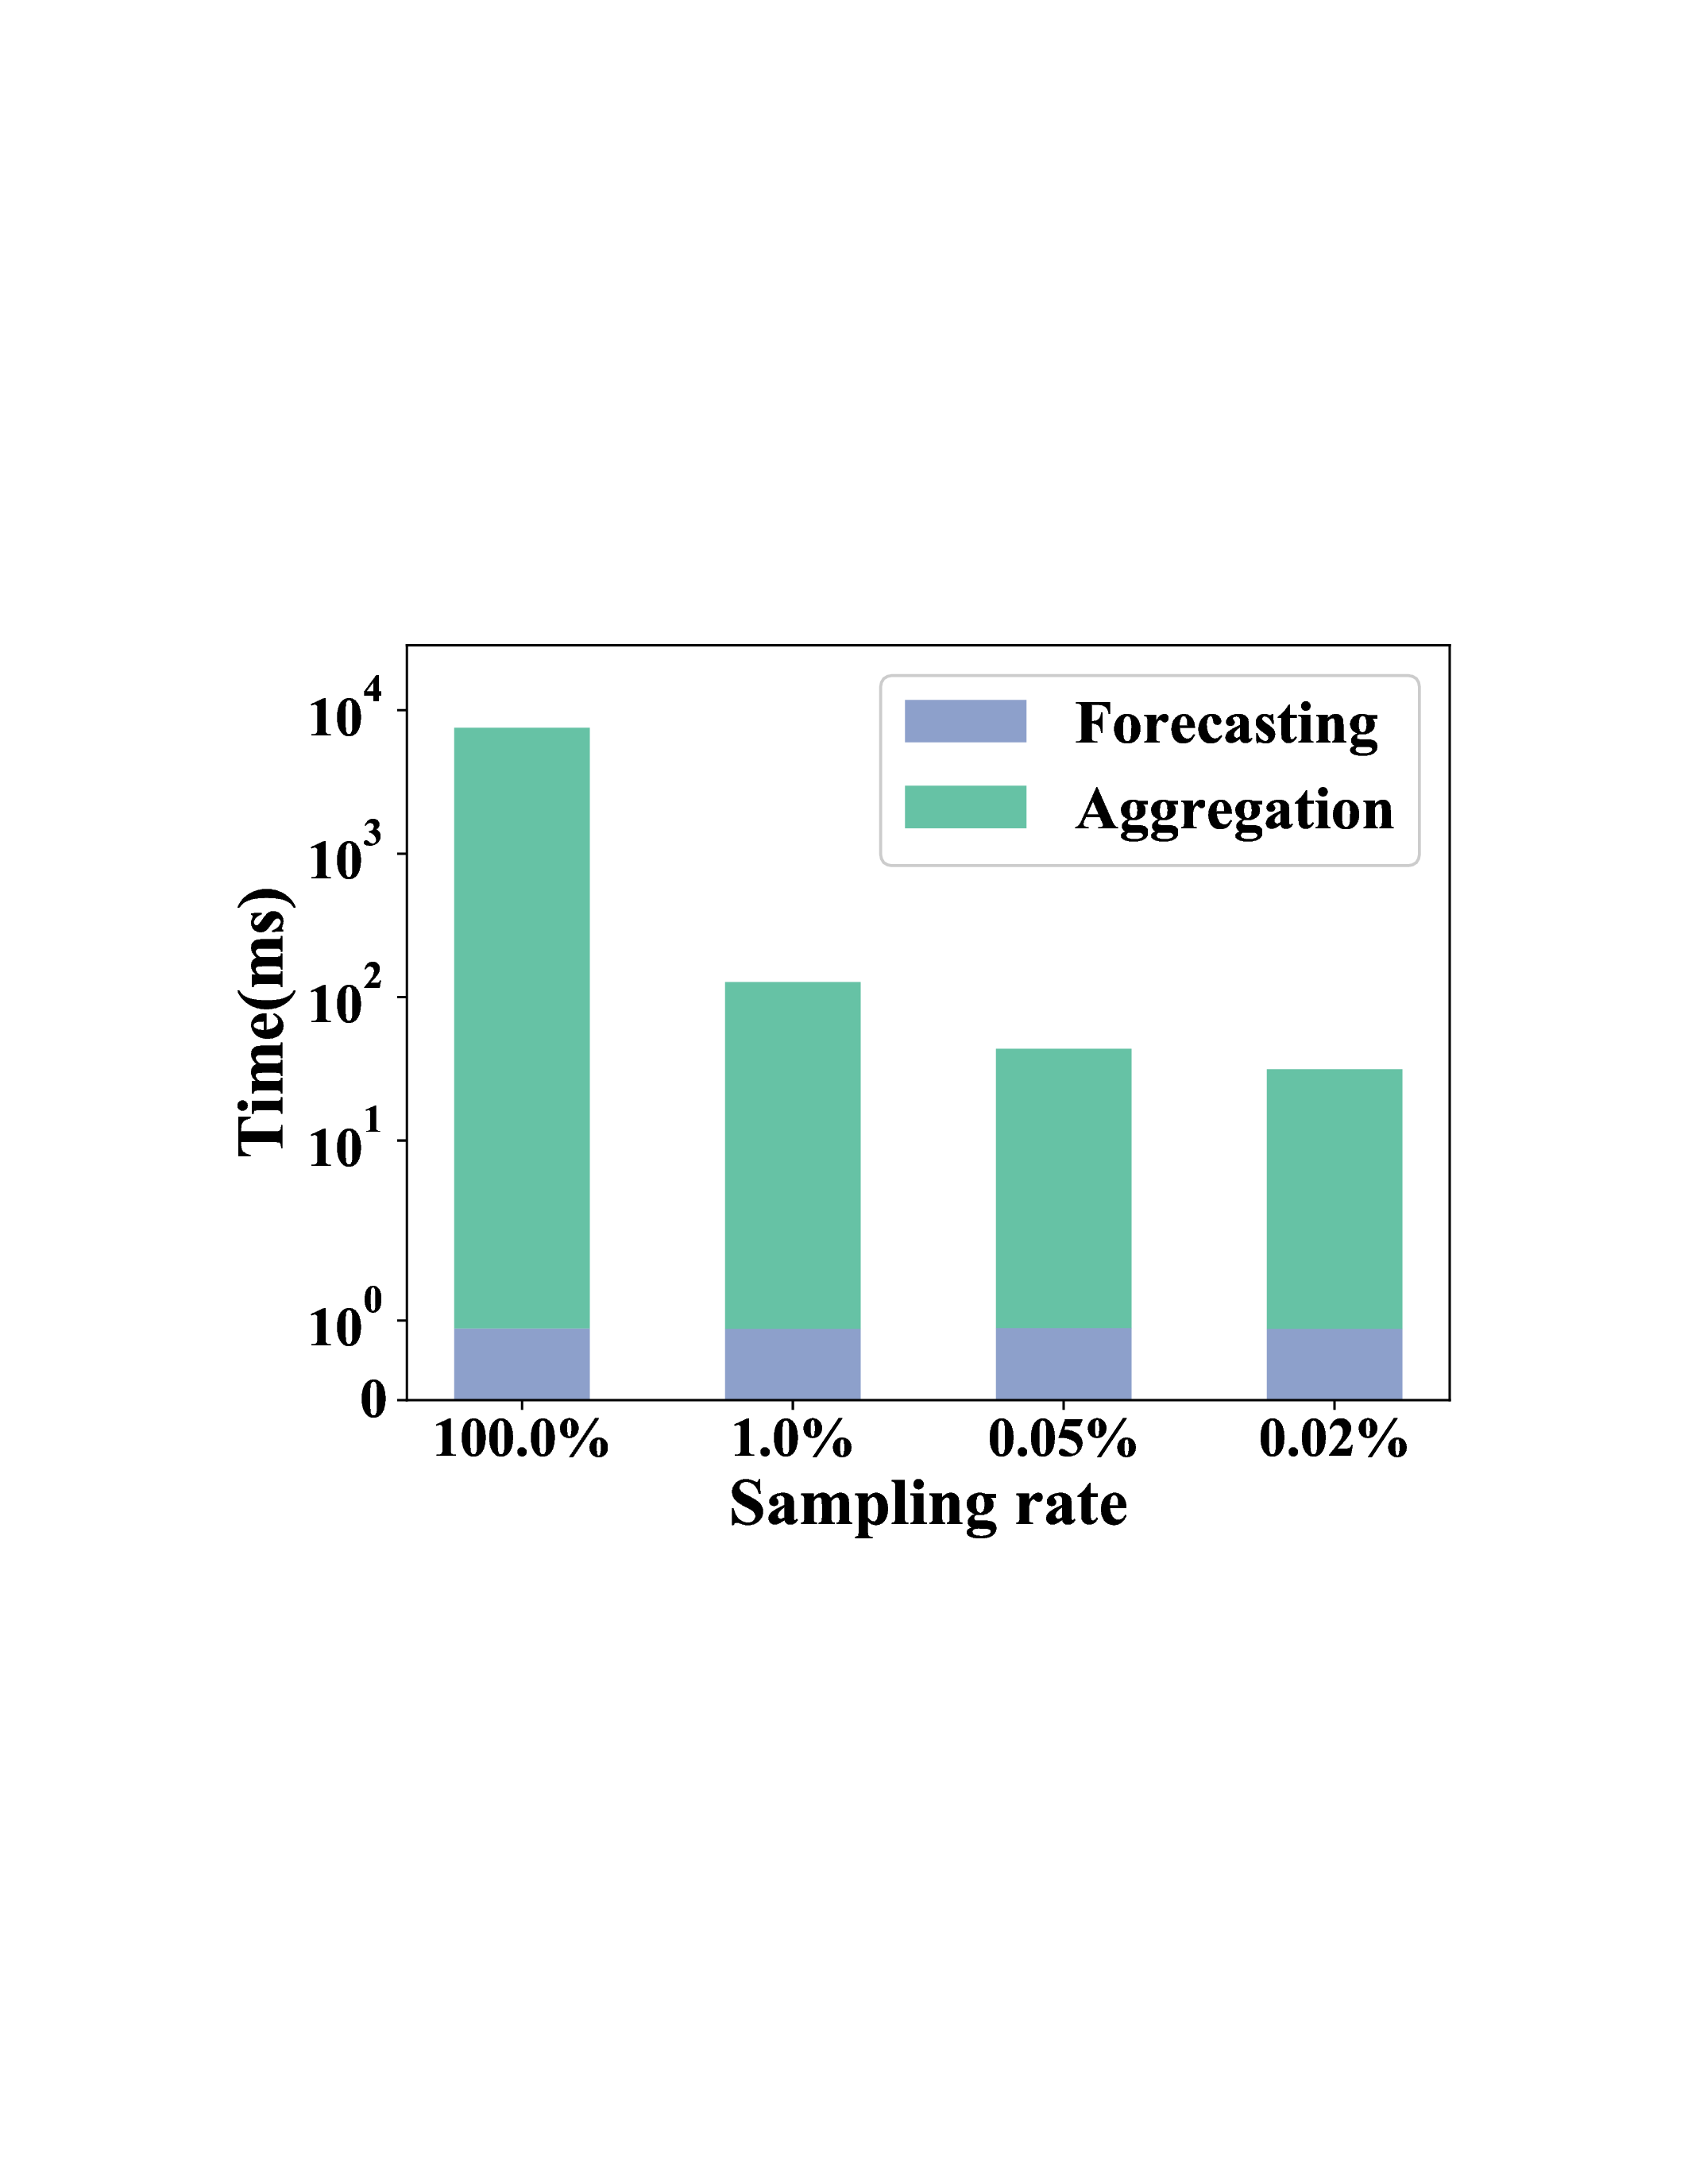}
}
\end{minipage}
\begin{minipage}[t]{0.33\linewidth}
\subfigure[Selectivity 1\%]{
\centering
\includegraphics[width=2.2in, height=2.0in]{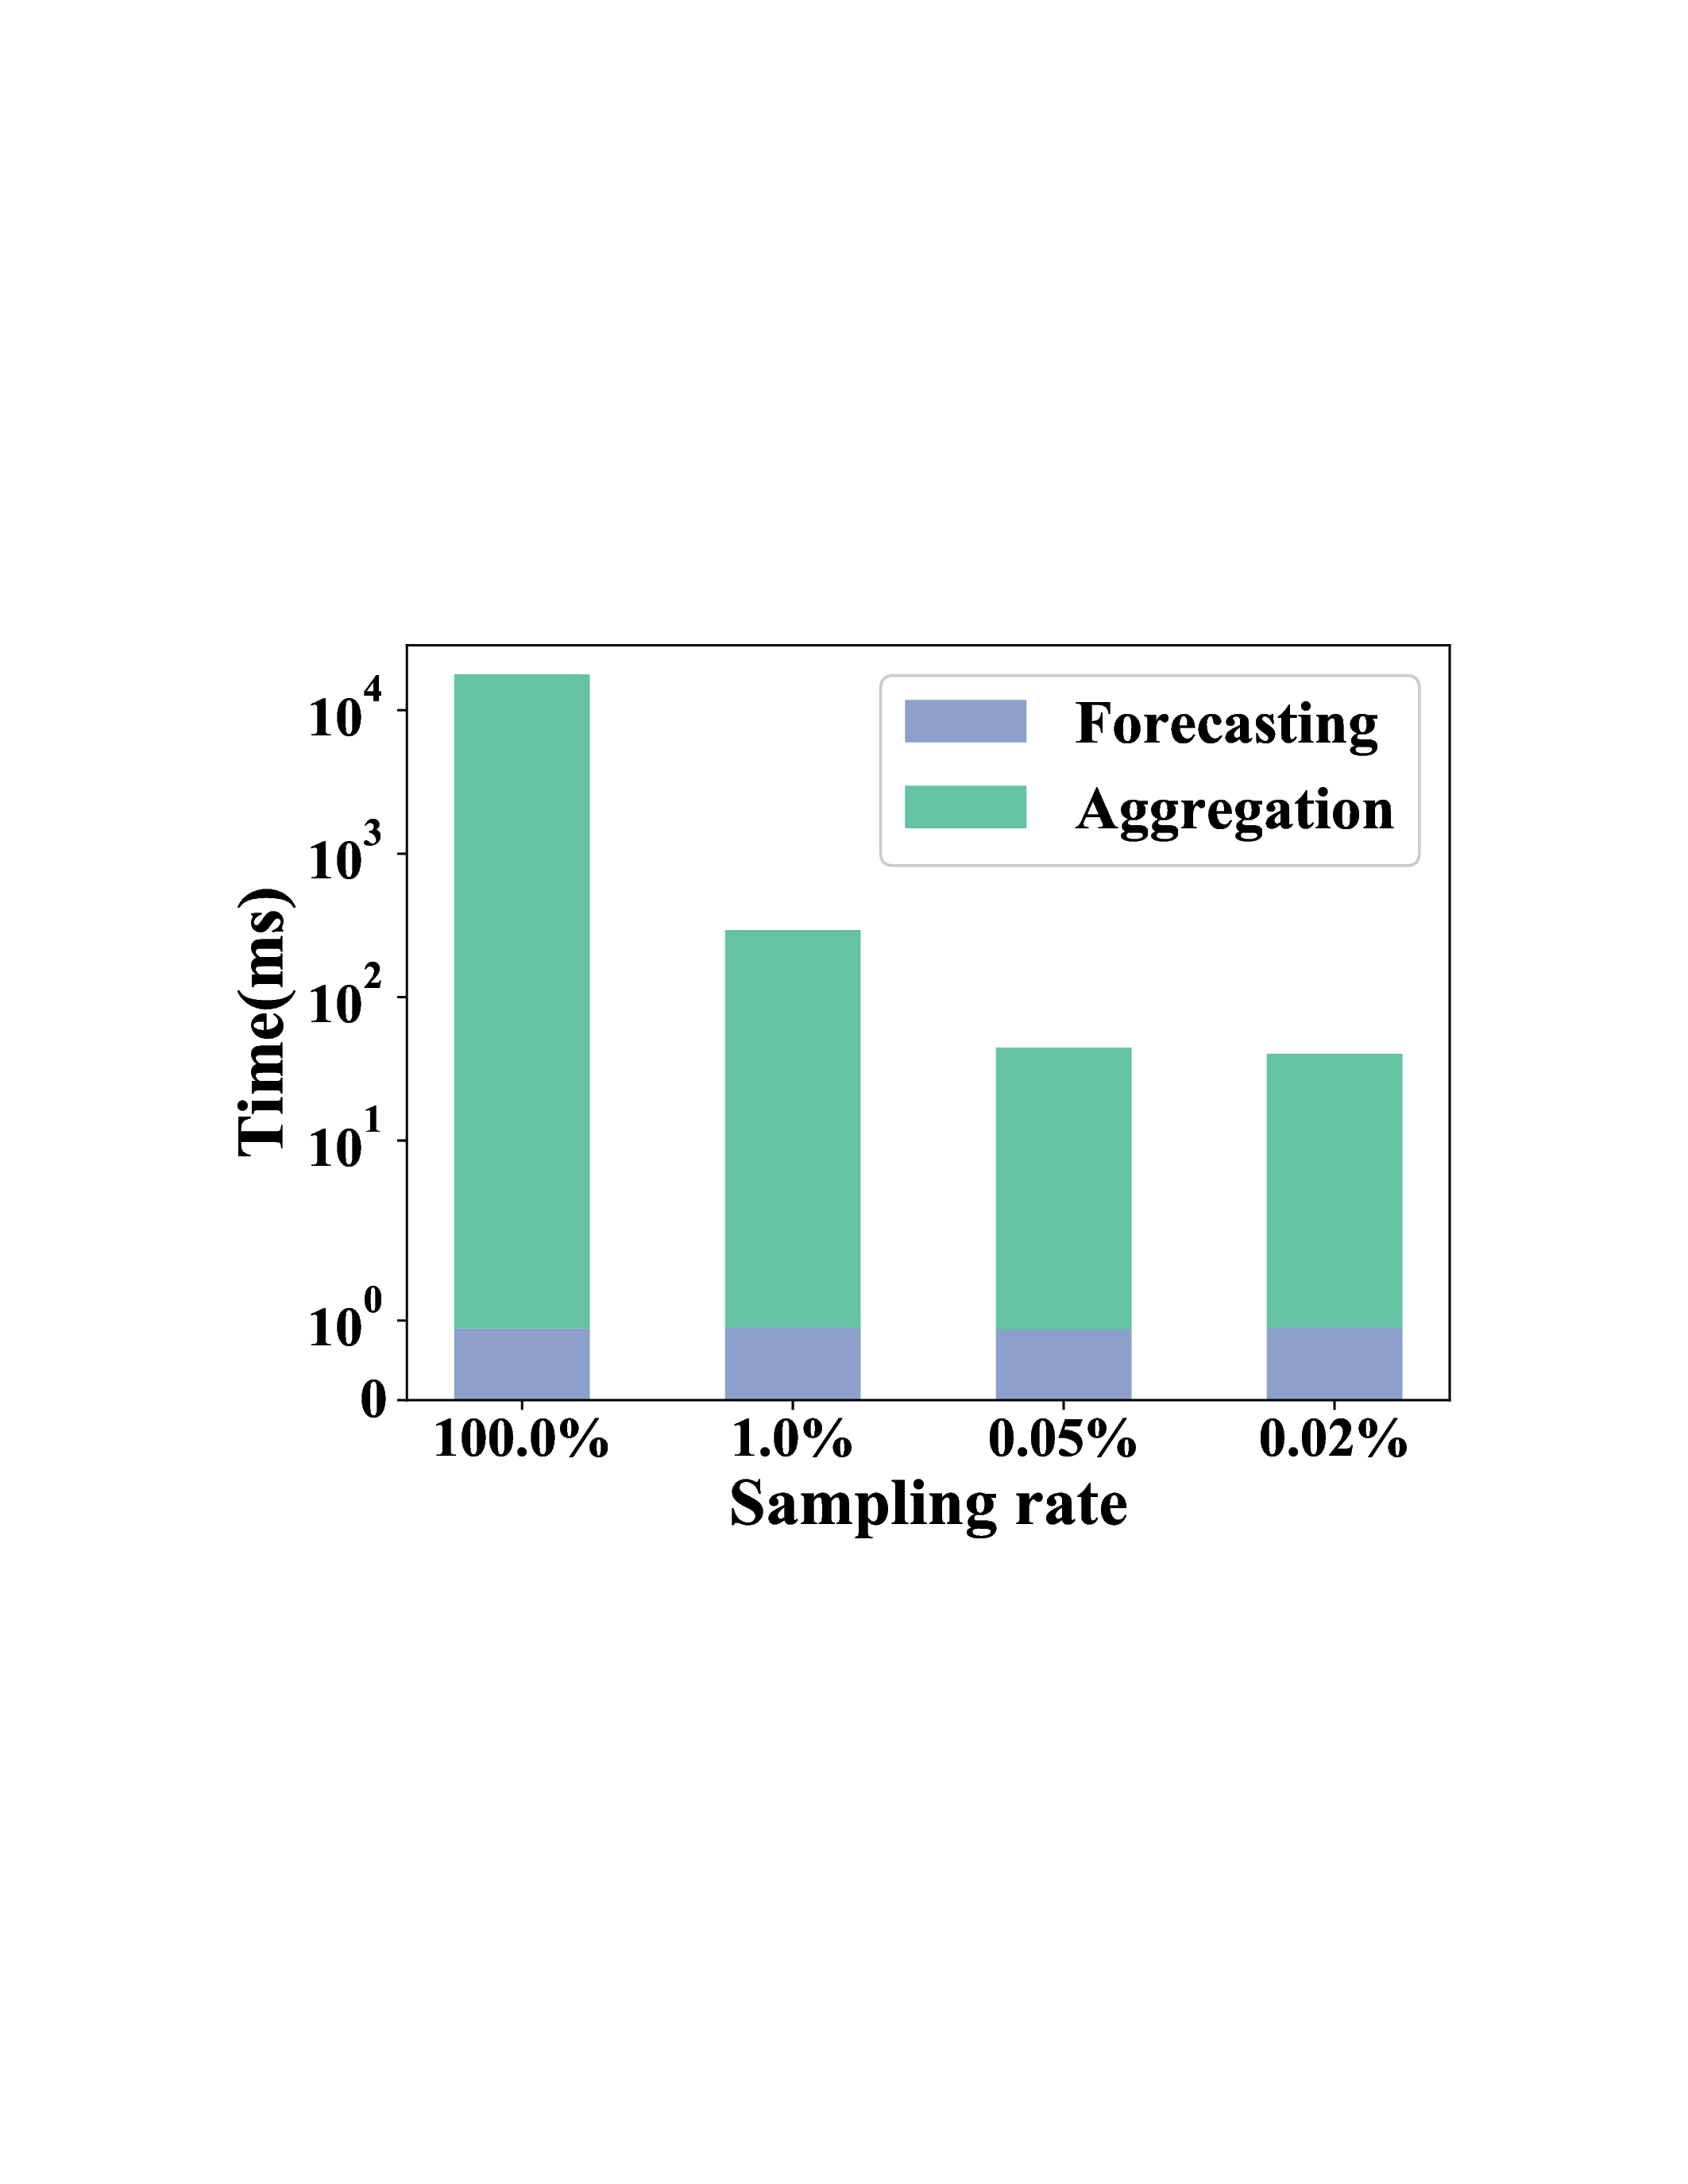}
}
\end{minipage}
\begin{minipage}[t]{0.33\linewidth}
\subfigure[Selectivity 5\%]{
\centering
\includegraphics[width=2.2in, height=2.0in]{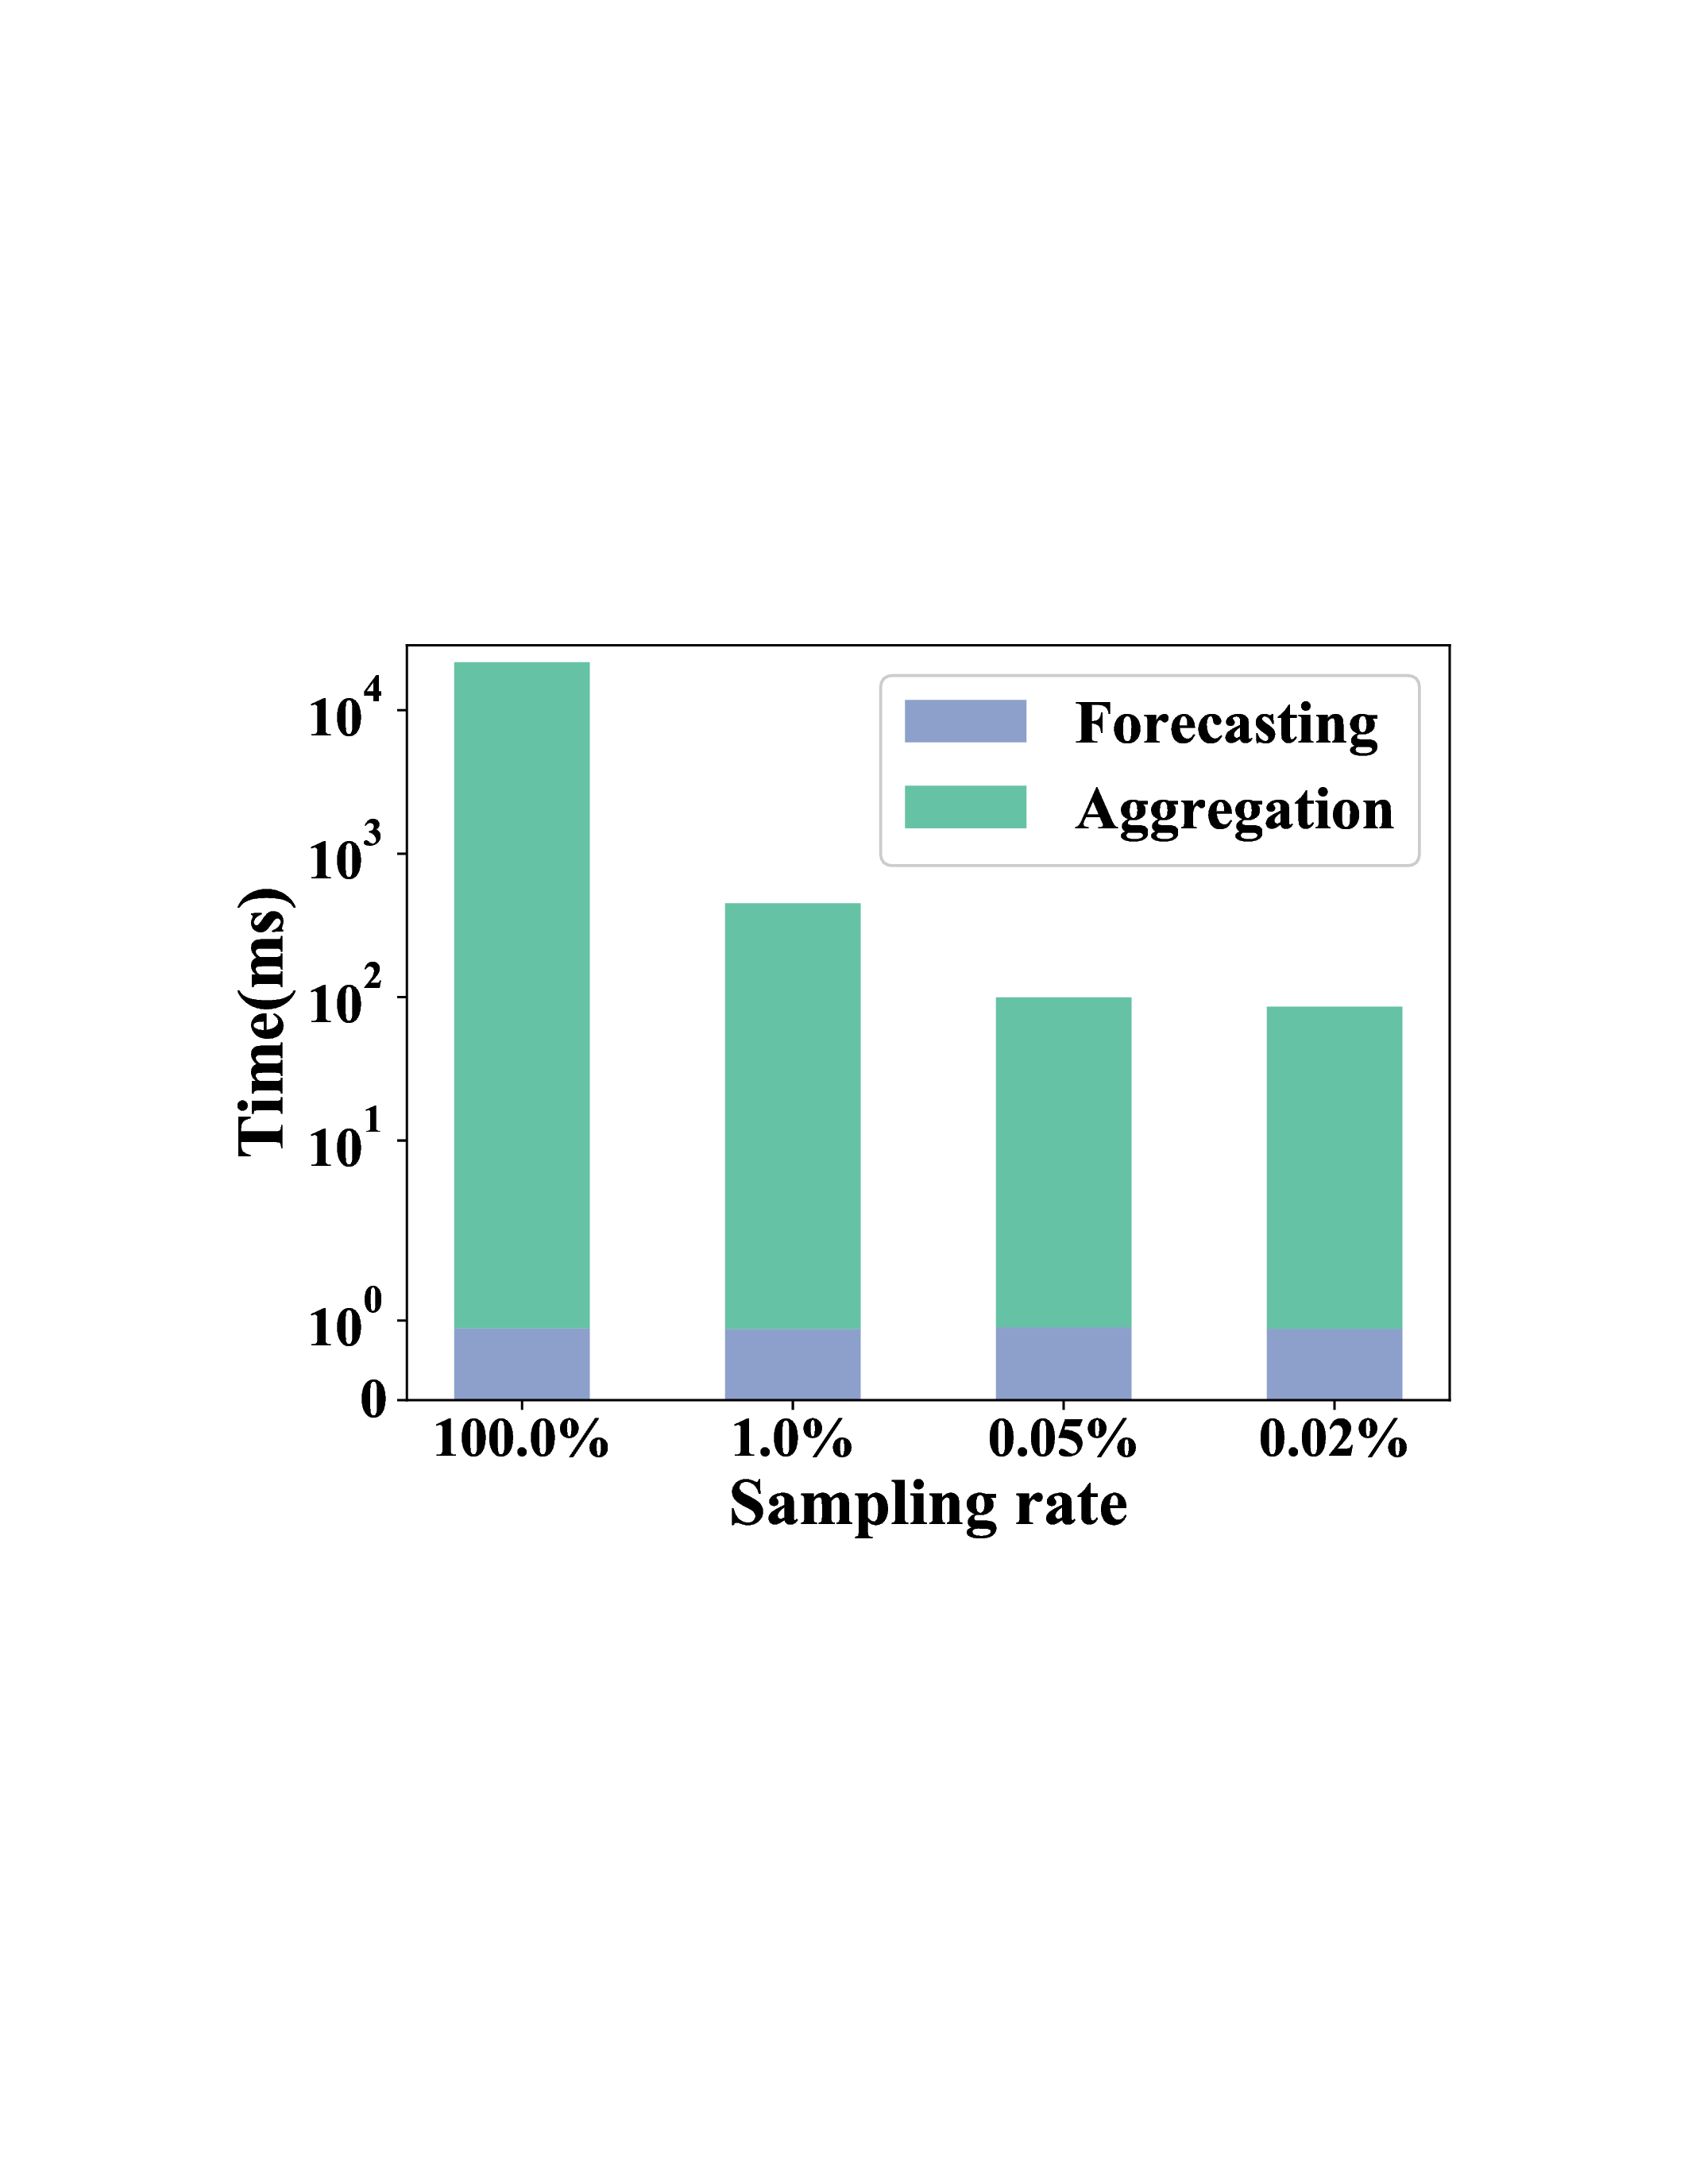}
}
\end{minipage}
\caption{AQP and ARIMA Performance with different sampling rate at fixed selectivity (how many rows and days in total? ms?)}
\end{figure*}
%---------end-------------

%%=================accuracy expr=================
%%total 150 days including 1326760215 rows and 61379988 users
%%=============================================
%========================PERIOD===================================
%-----训练周期对arima模型的影响----------
\begin{figure*}[ht]
\subfigure[Selectivity 0.5\%]{
\begin{minipage}[t]{0.33\linewidth}
\centering
\includegraphics[width=2.2in, height=2.0in]{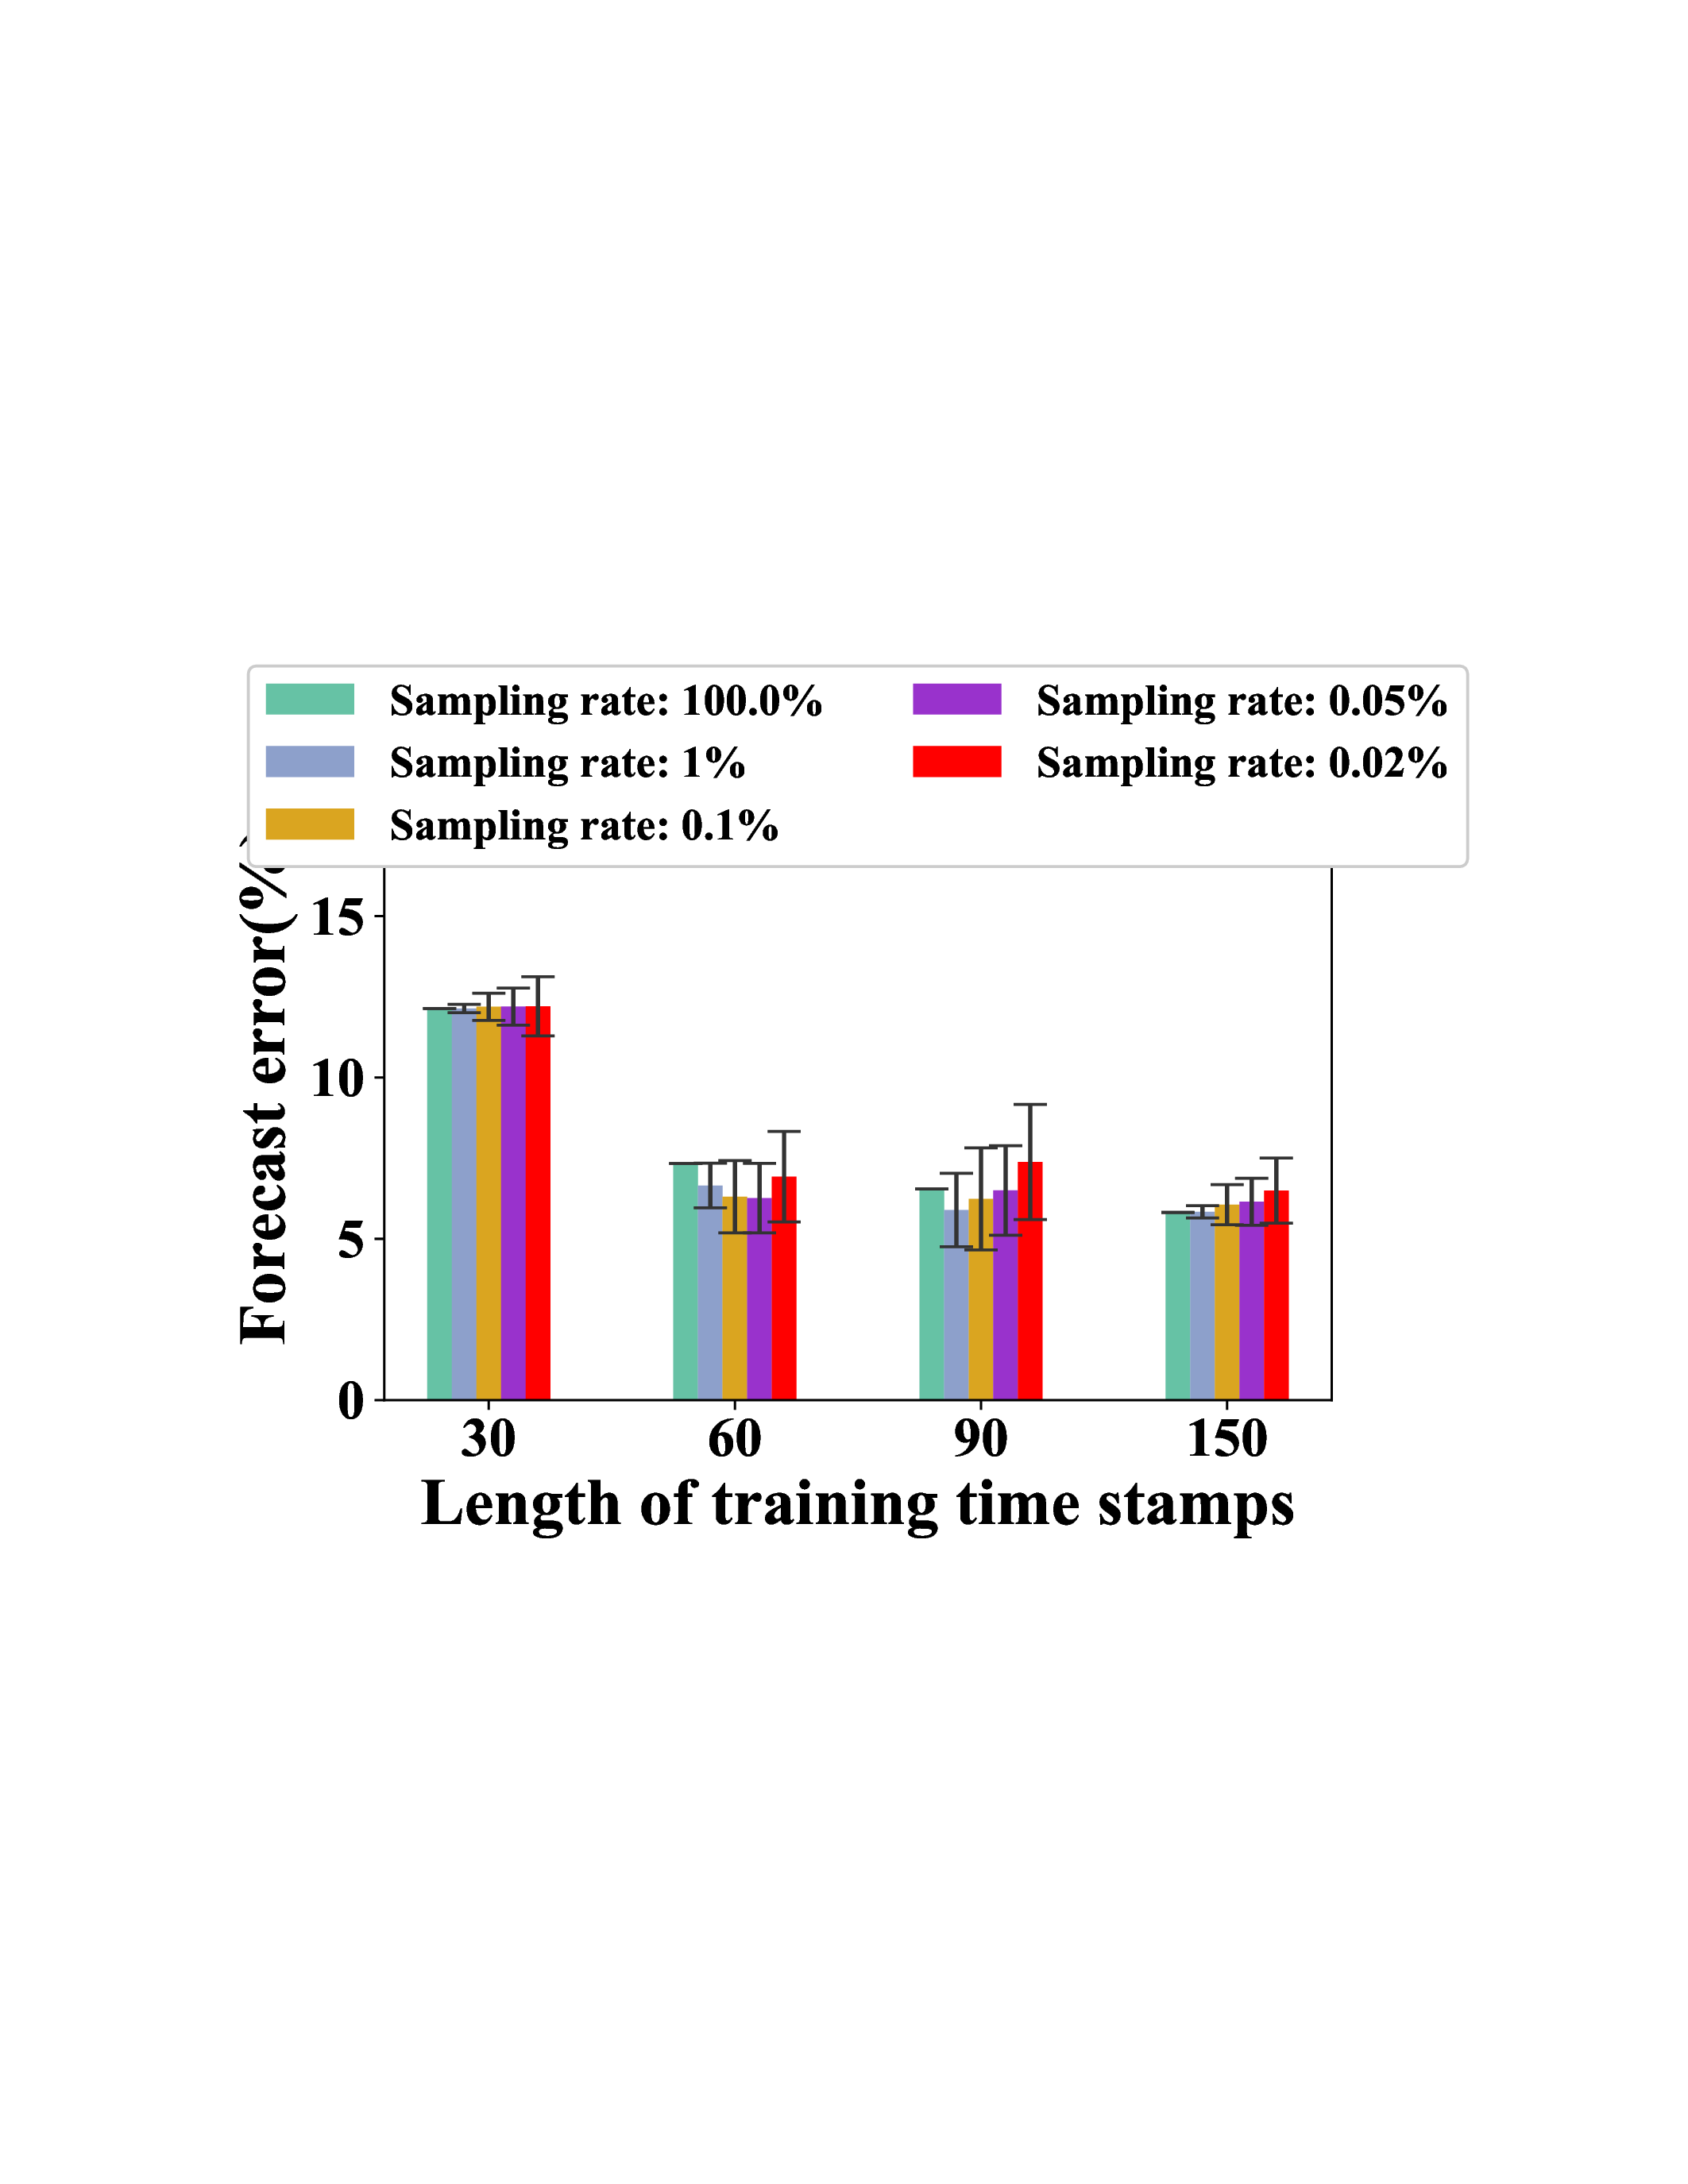}
% \label{fig:side:a}
\end{minipage}
}
\subfigure[Selectivity 1\%]{
\begin{minipage}[t]{0.33\linewidth}
\centering
\includegraphics[width=2.2in, height=2.0in]{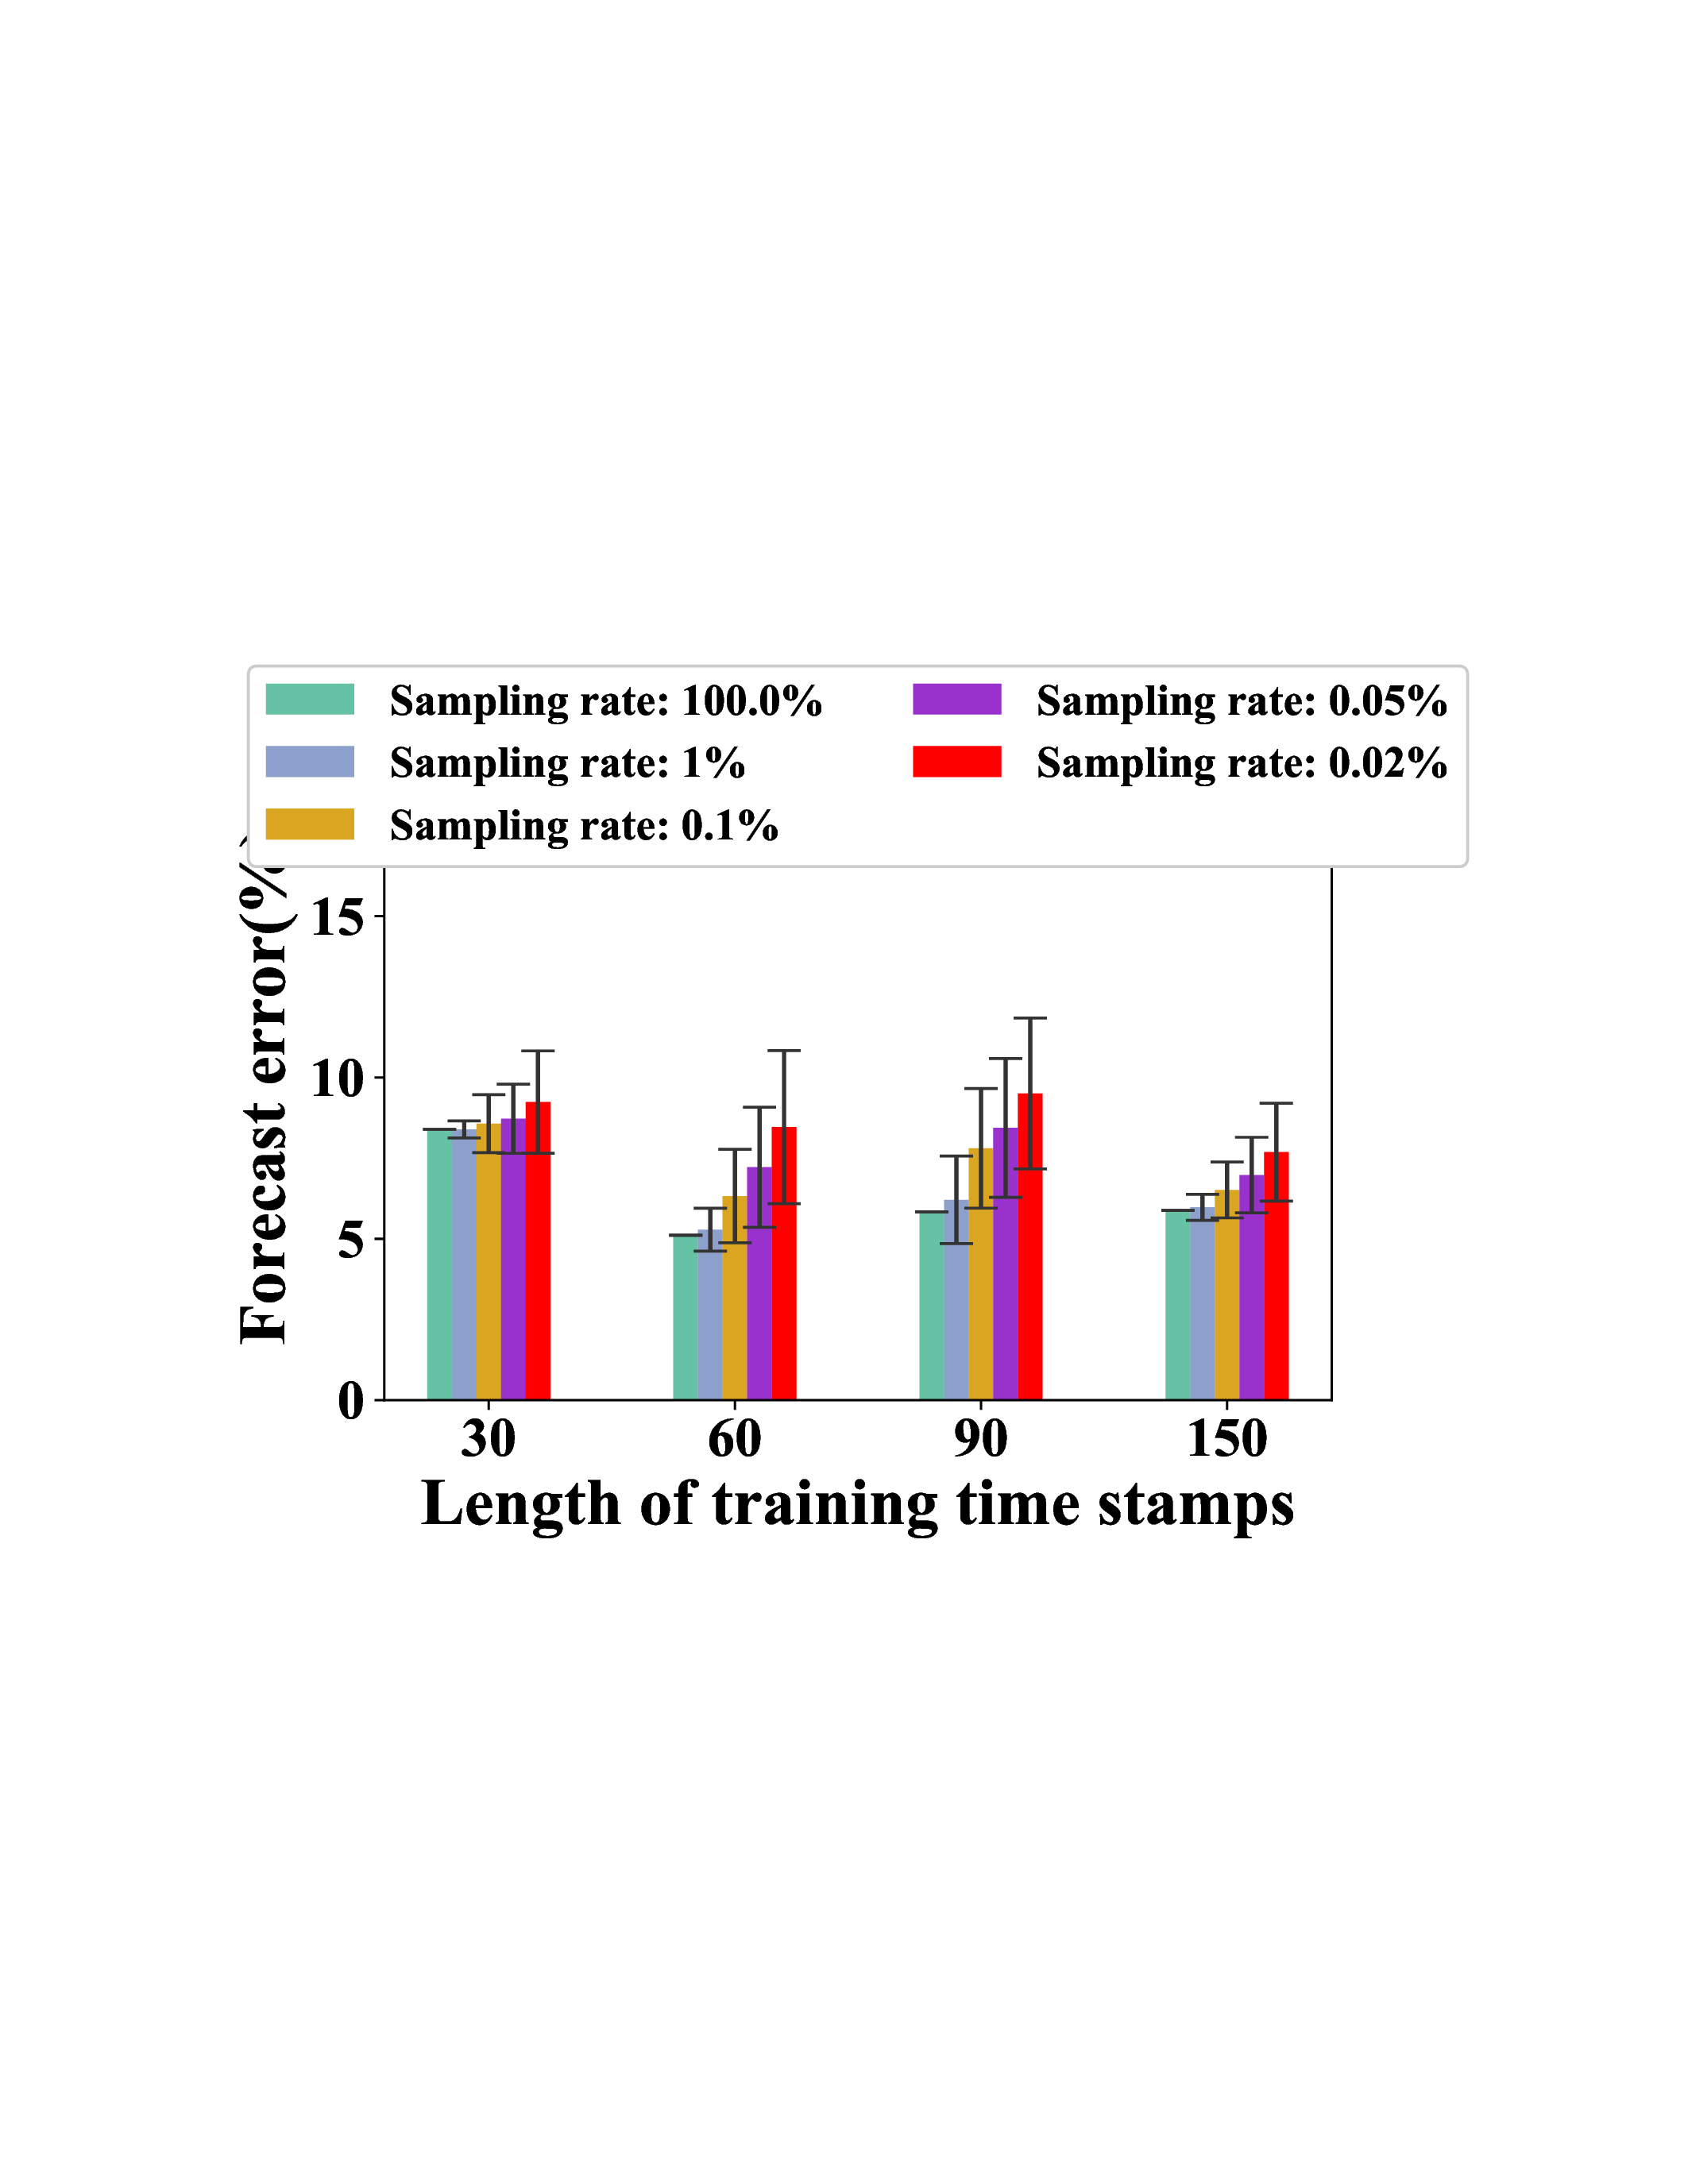}
\end{minipage}
}
\subfigure[Selectivity 5\%]{
\begin{minipage}[t]{0.33\linewidth}
\centering
\includegraphics[width=2.2in, height=2.0in]{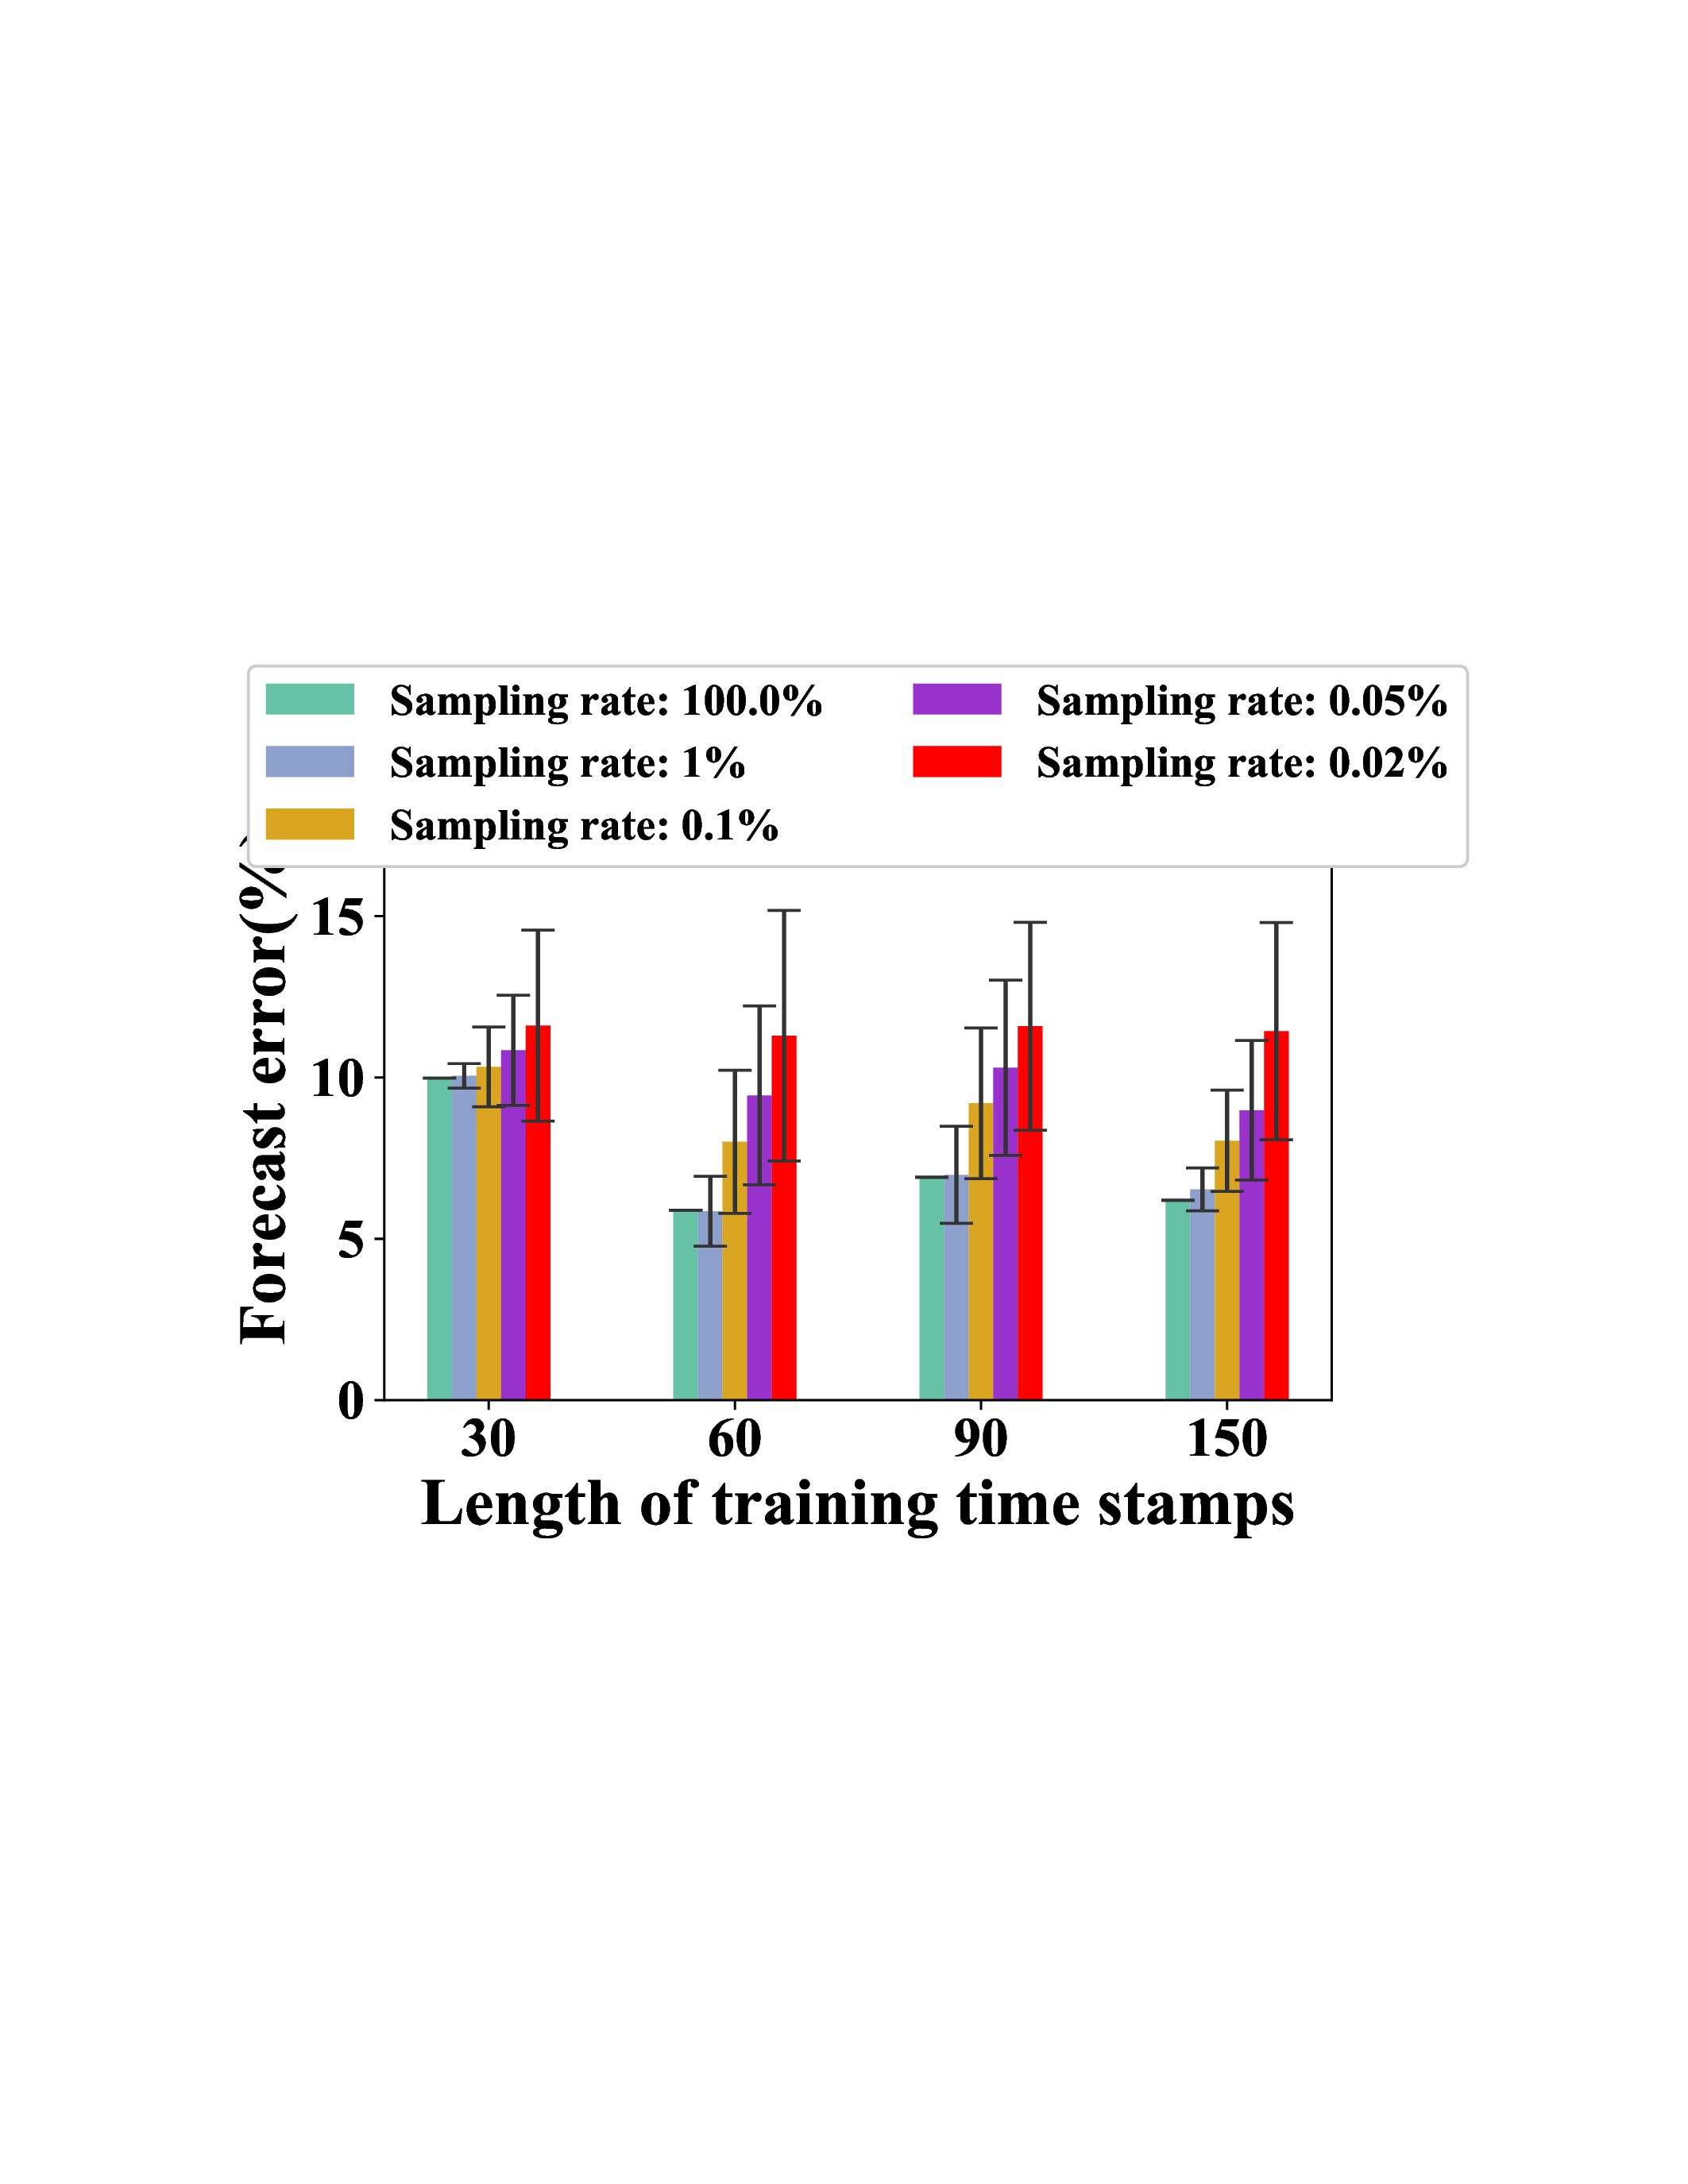}
\end{minipage}
}
\caption{ARIMA predict error on impression at different training time stamps with different sampling rate  (add sampling rate 0.1\%)}
% \label{AQP and ARIMA Performance}
\end{figure*}

%========================AQP+ARIMA+INTERVAL===================================
%-----Impression不同抽样方法对AQP误差的影响----------
\begin{figure*}[ht]
\subfigure[Selectivity 0.5\%]{
\begin{minipage}[t]{0.33\linewidth}
\centering
\includegraphics[width=2.2in, height=2.0in]{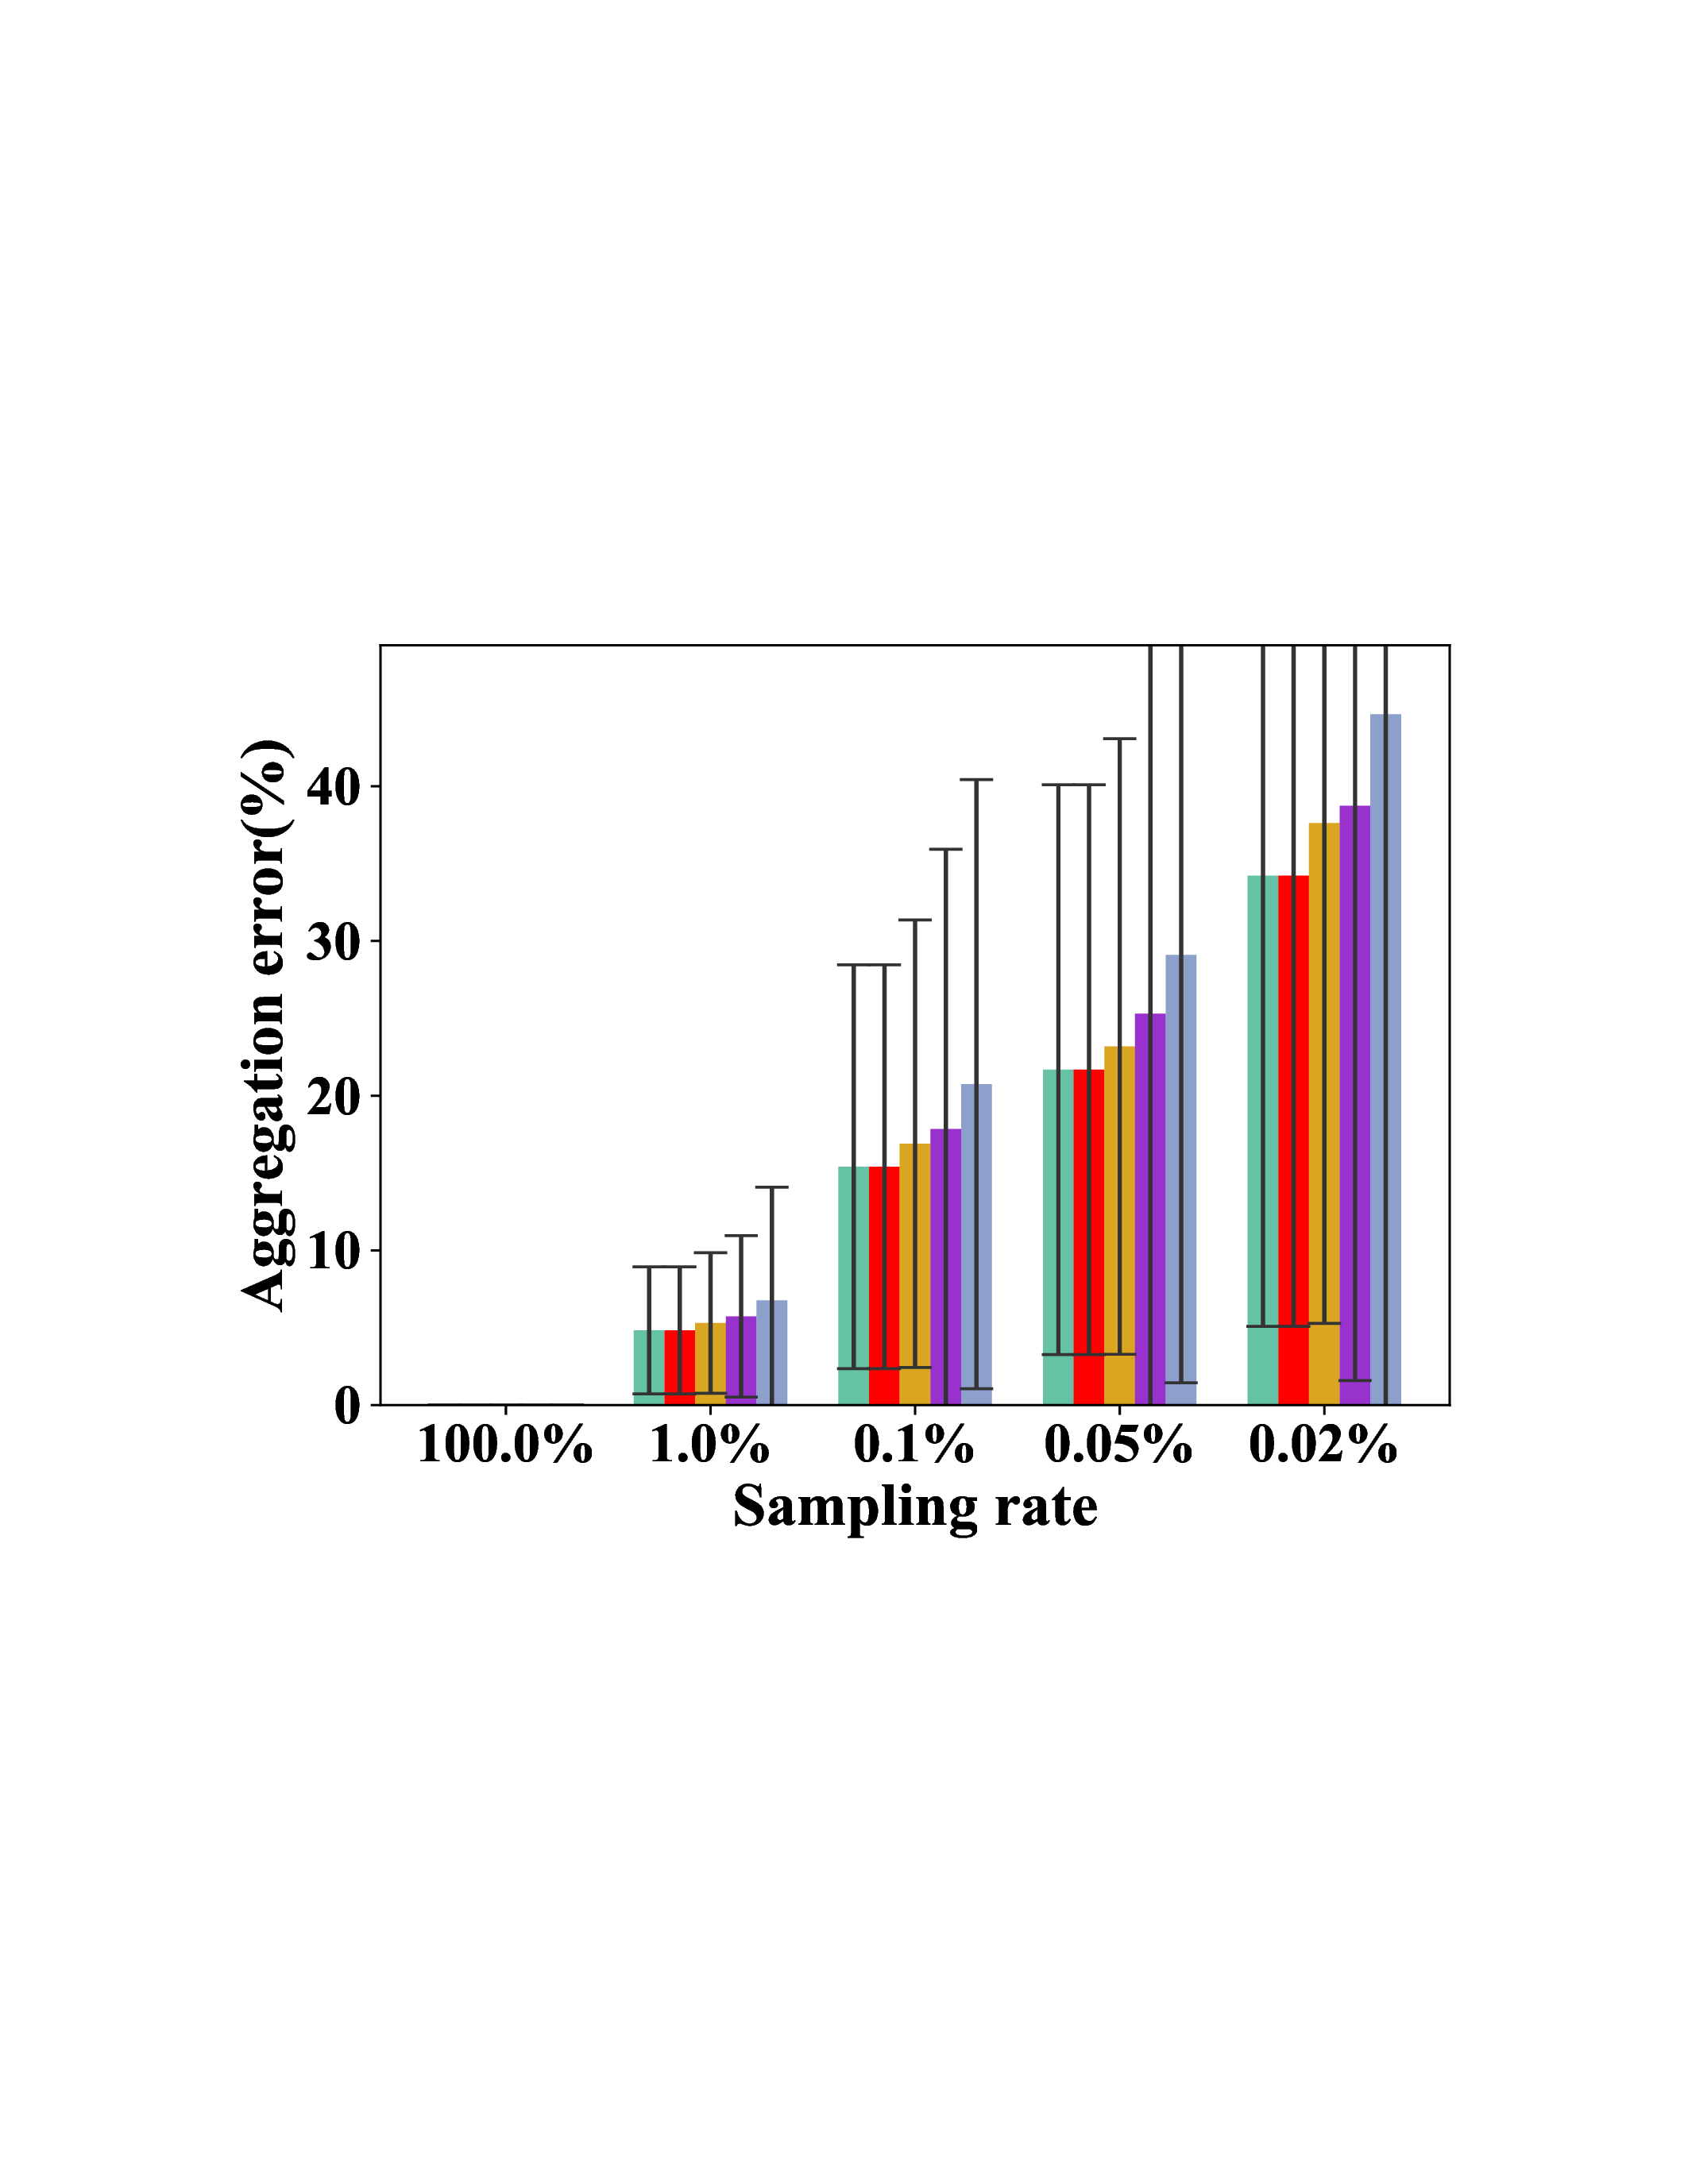}
% \label{fig:side:a}
\end{minipage}
}
\subfigure[Selectivity 1\%]{
\begin{minipage}[t]{0.33\linewidth}
\centering
\includegraphics[width=2.2in, height=2.0in]{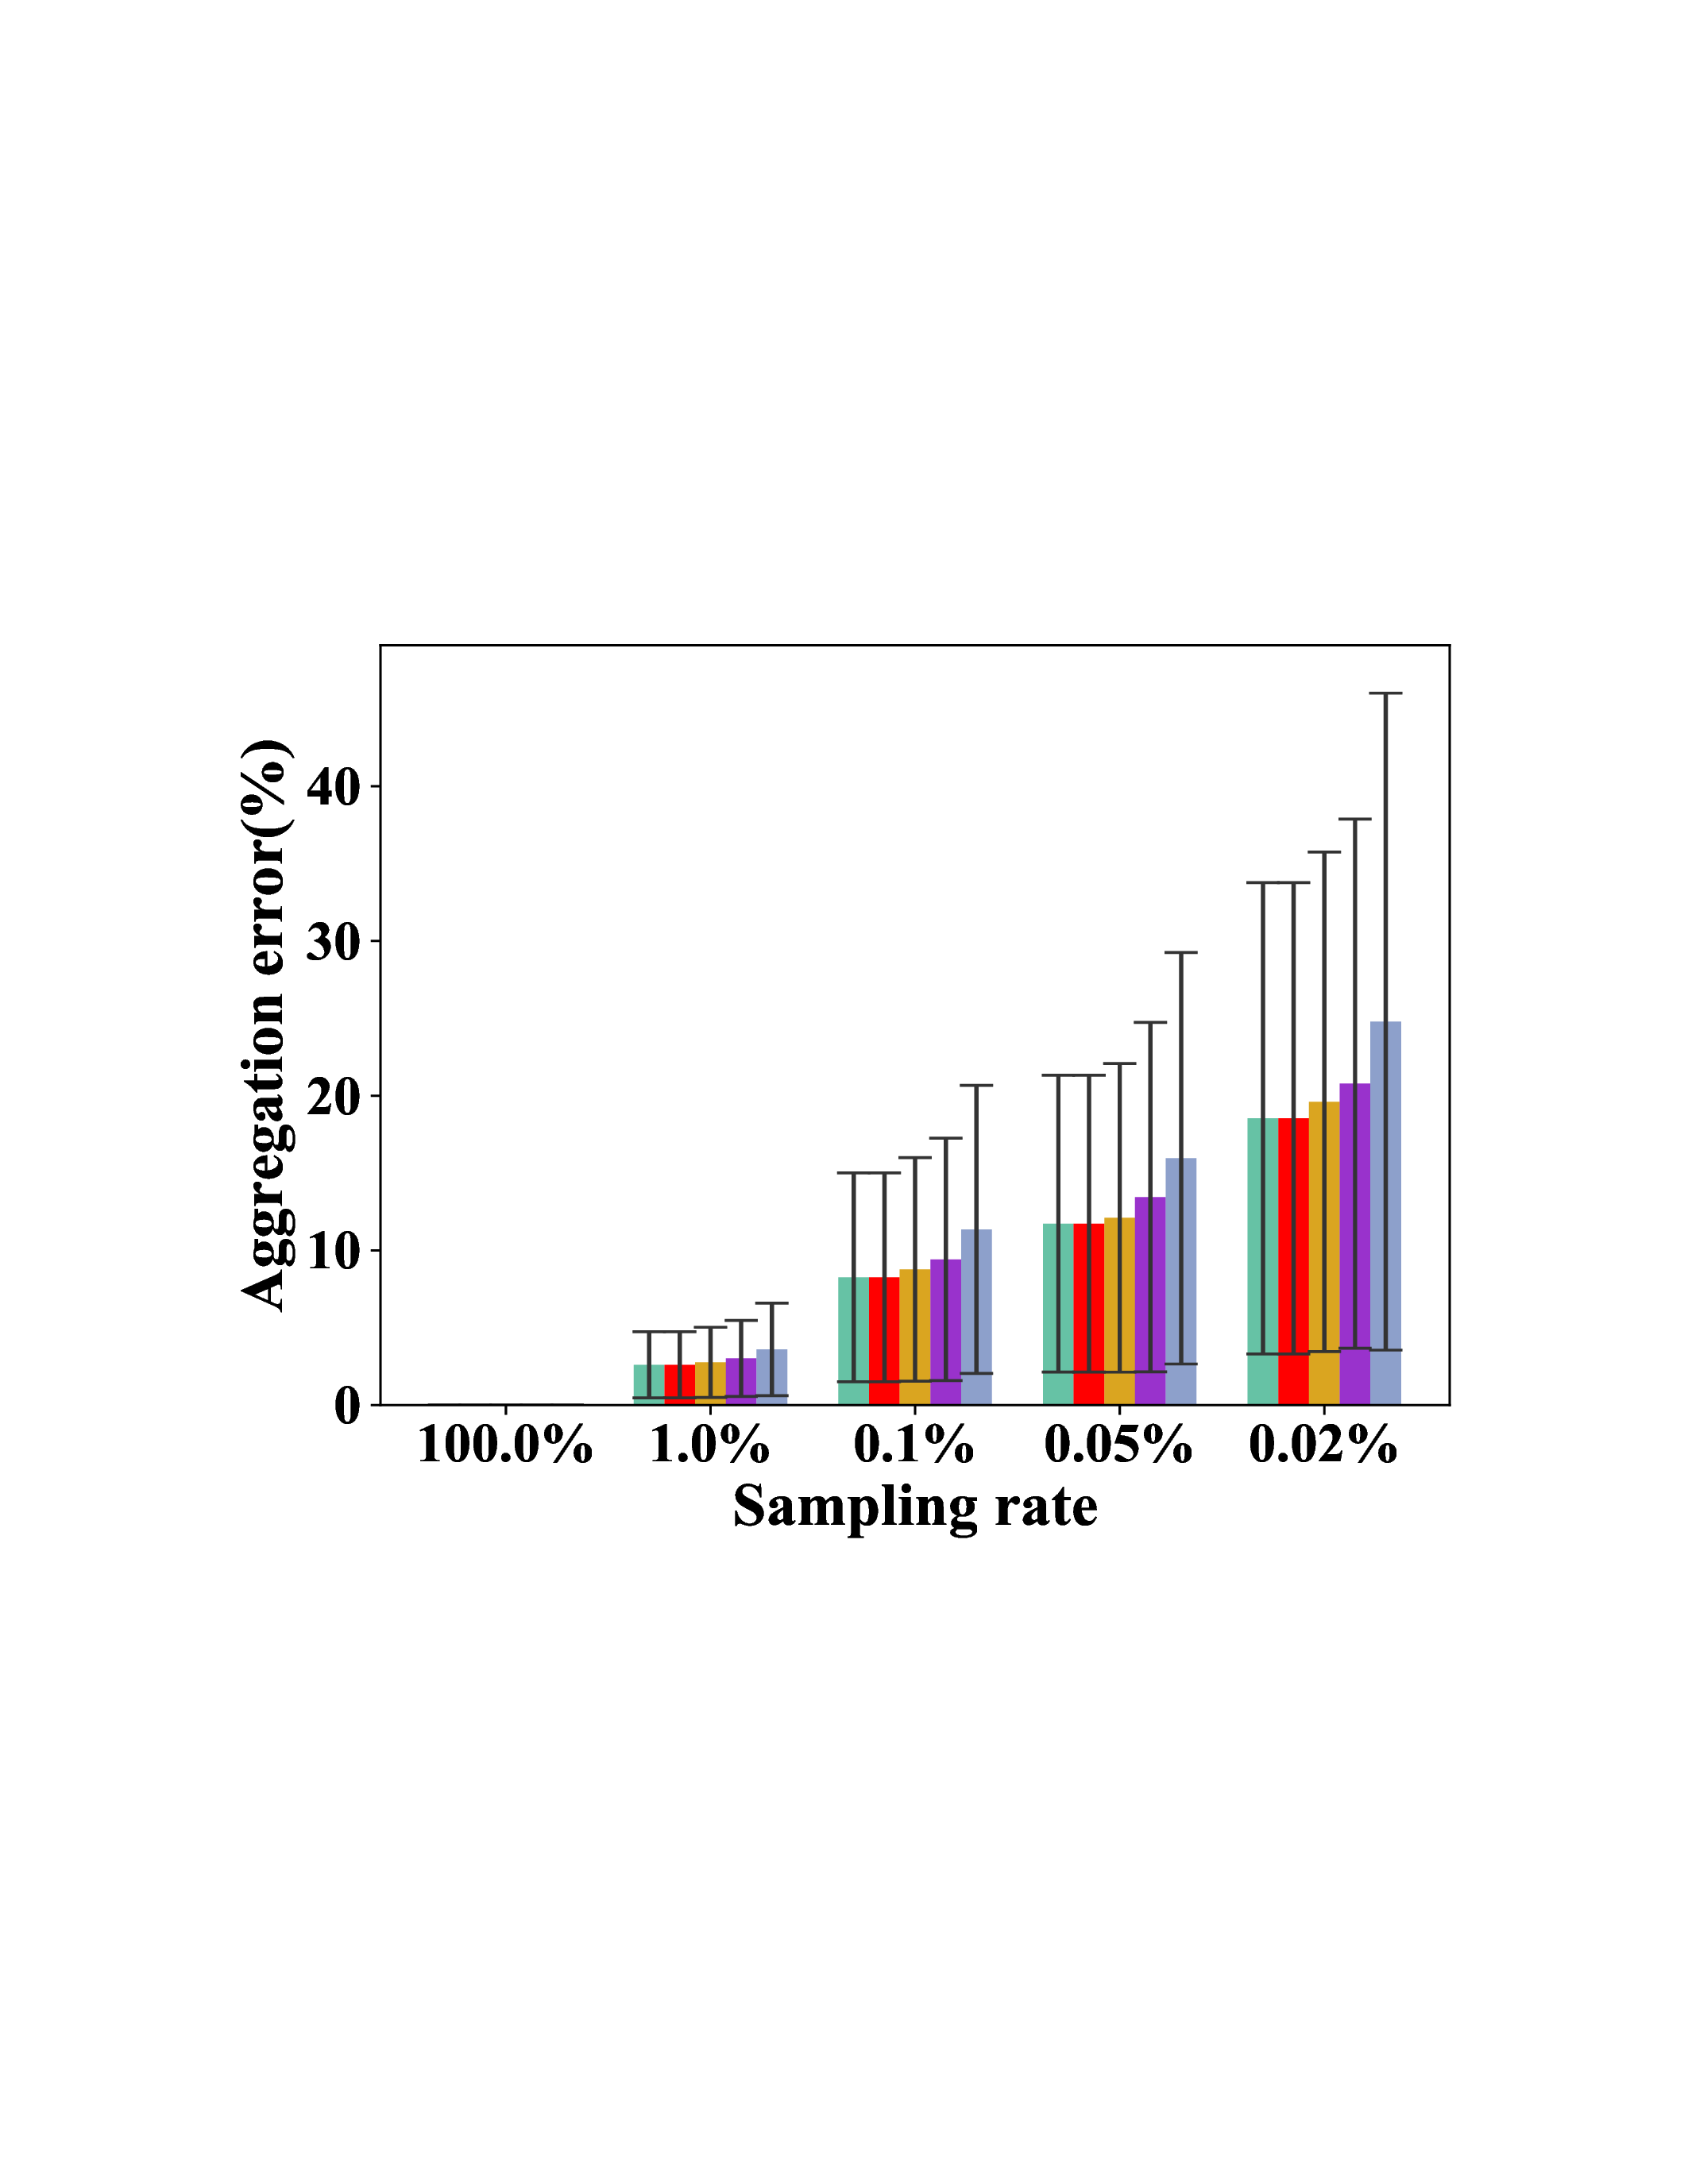}
\end{minipage}
}
\subfigure[Selectivity 5\%]{
\begin{minipage}[t]{0.33\linewidth}
\centering
\includegraphics[width=2.2in, height=2.0in]{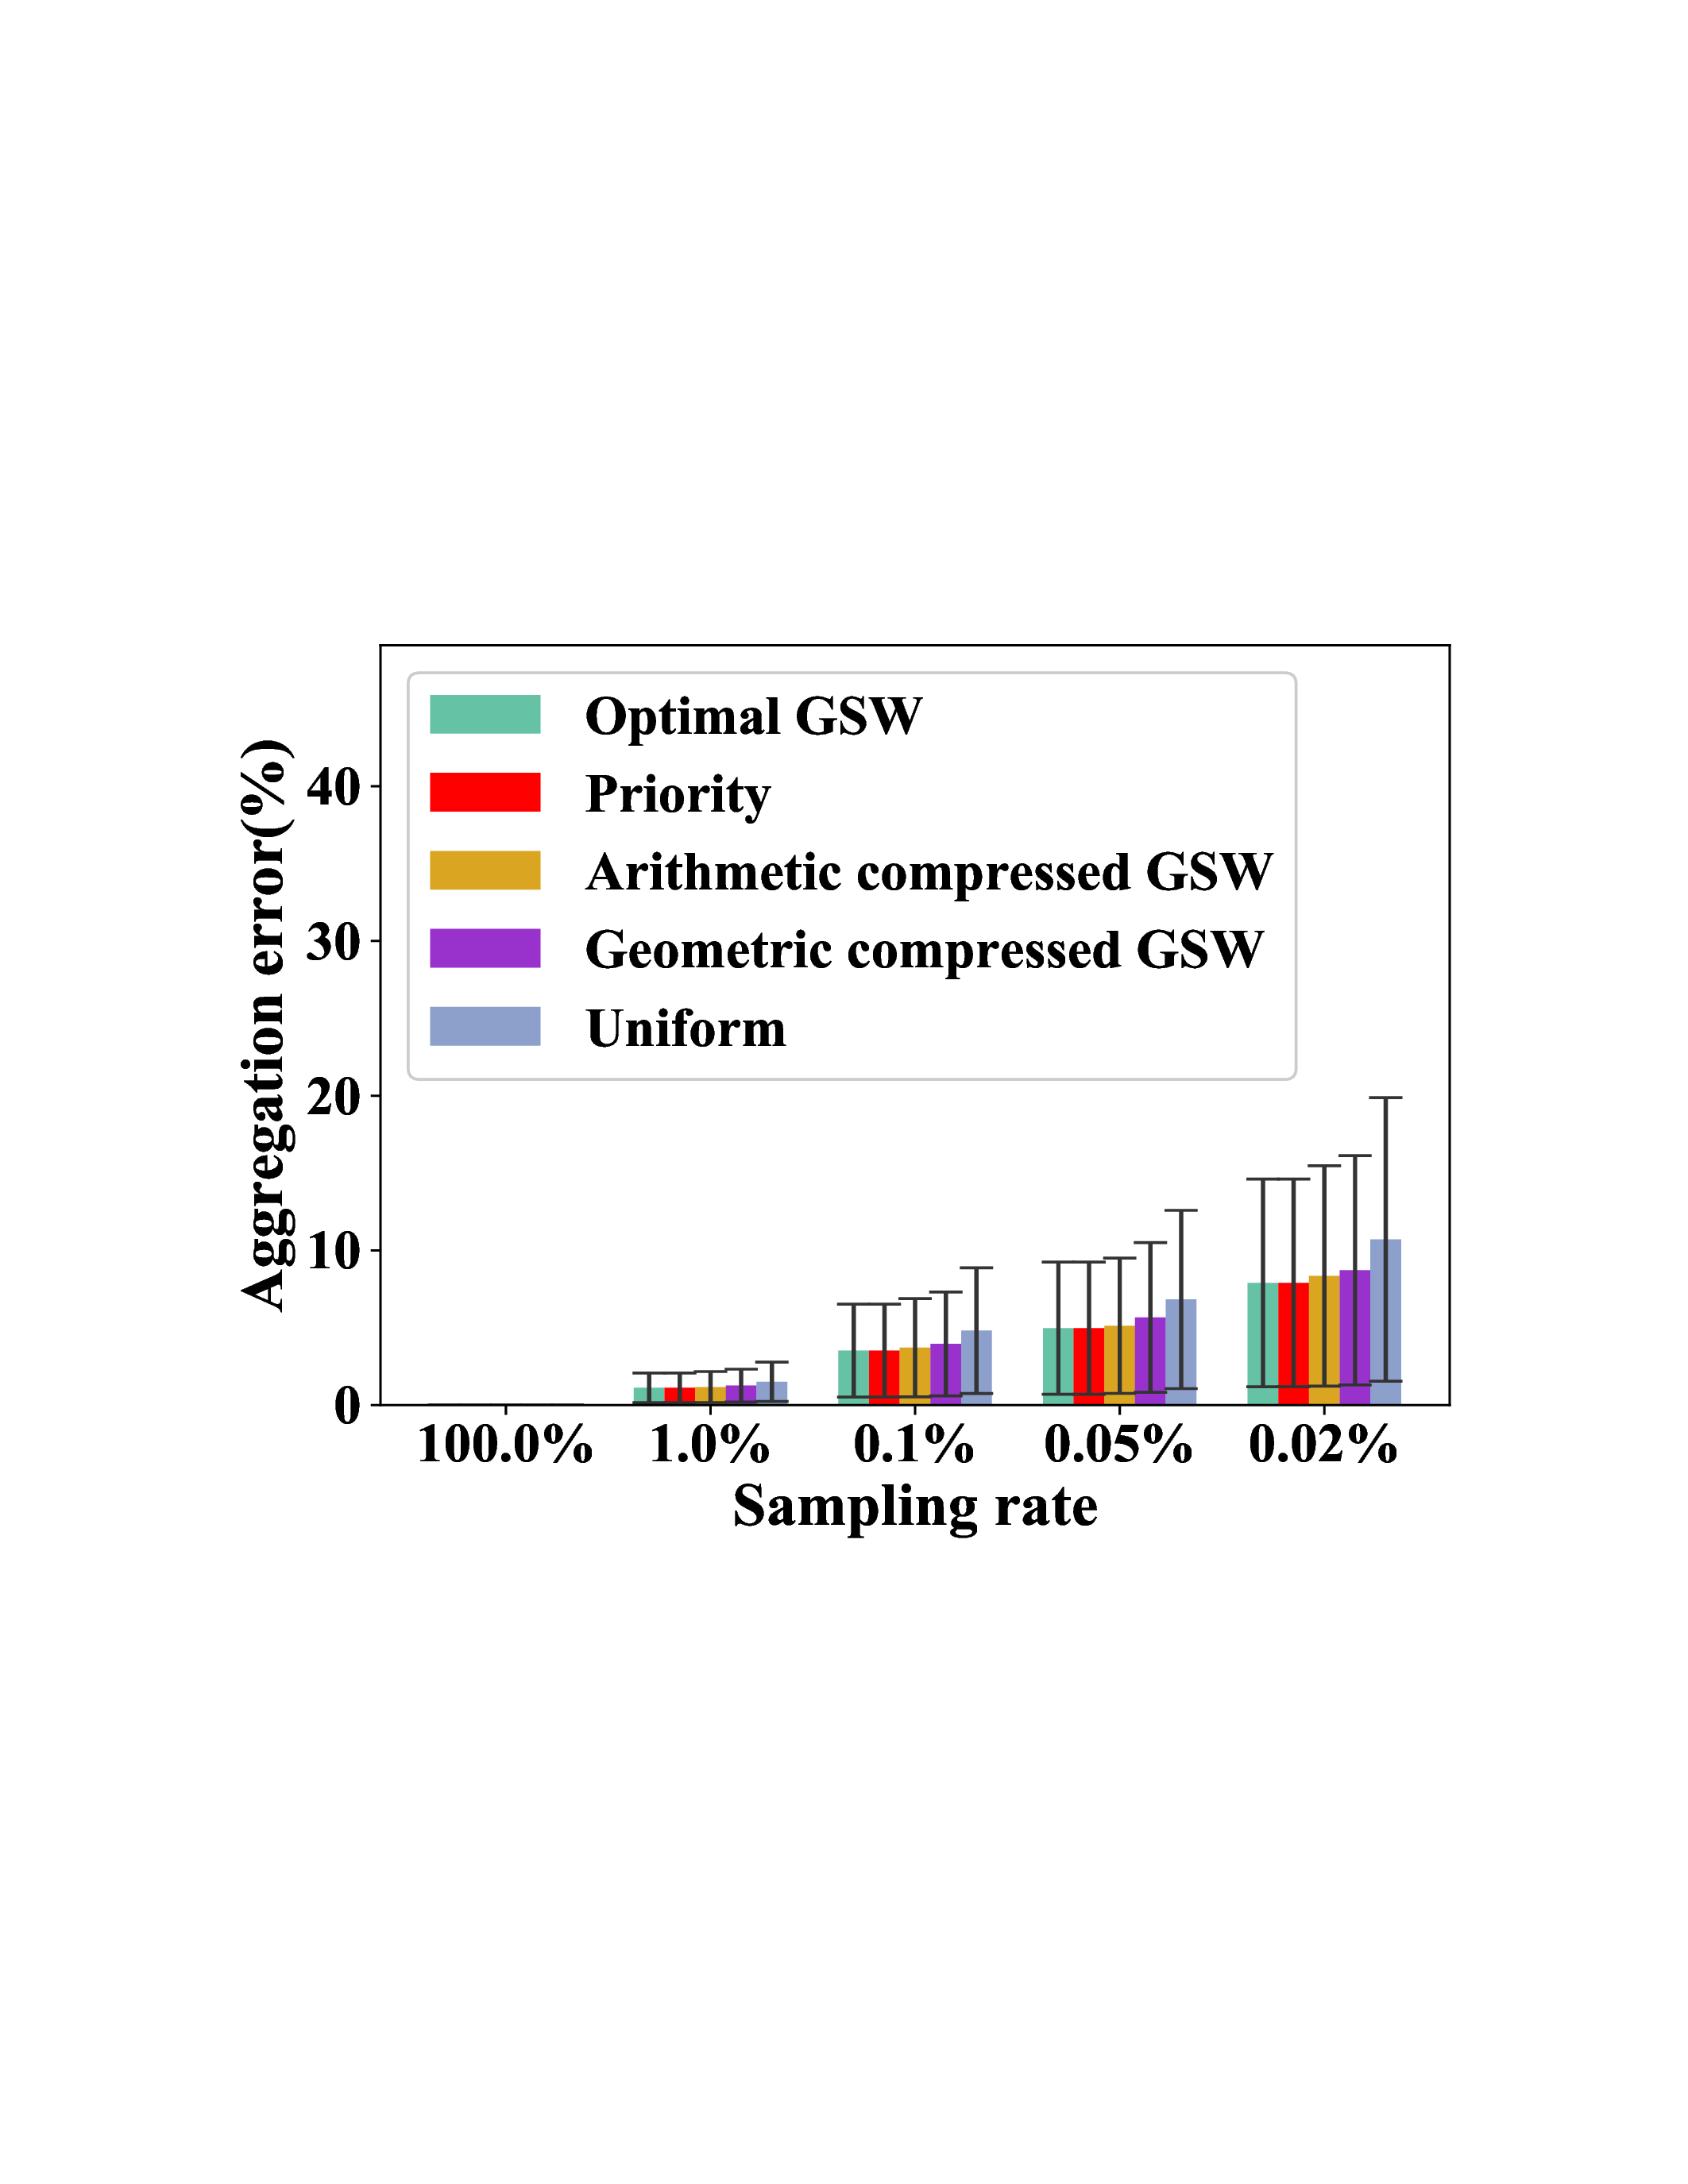}
\end{minipage}
}
\caption{AQP error at different selectivity on impression via different sampling methods}
% \label{AQP and ARIMA Performance}
\end{figure*}

%-----Impression不同抽样方法对ARIMA误差的影响----------
\begin{figure*}[hb]
\subfigure[Selectivity 0.5\%]{
\begin{minipage}[t]{0.33\linewidth}
\centering
\includegraphics[width=2.2in, height=2.0in]{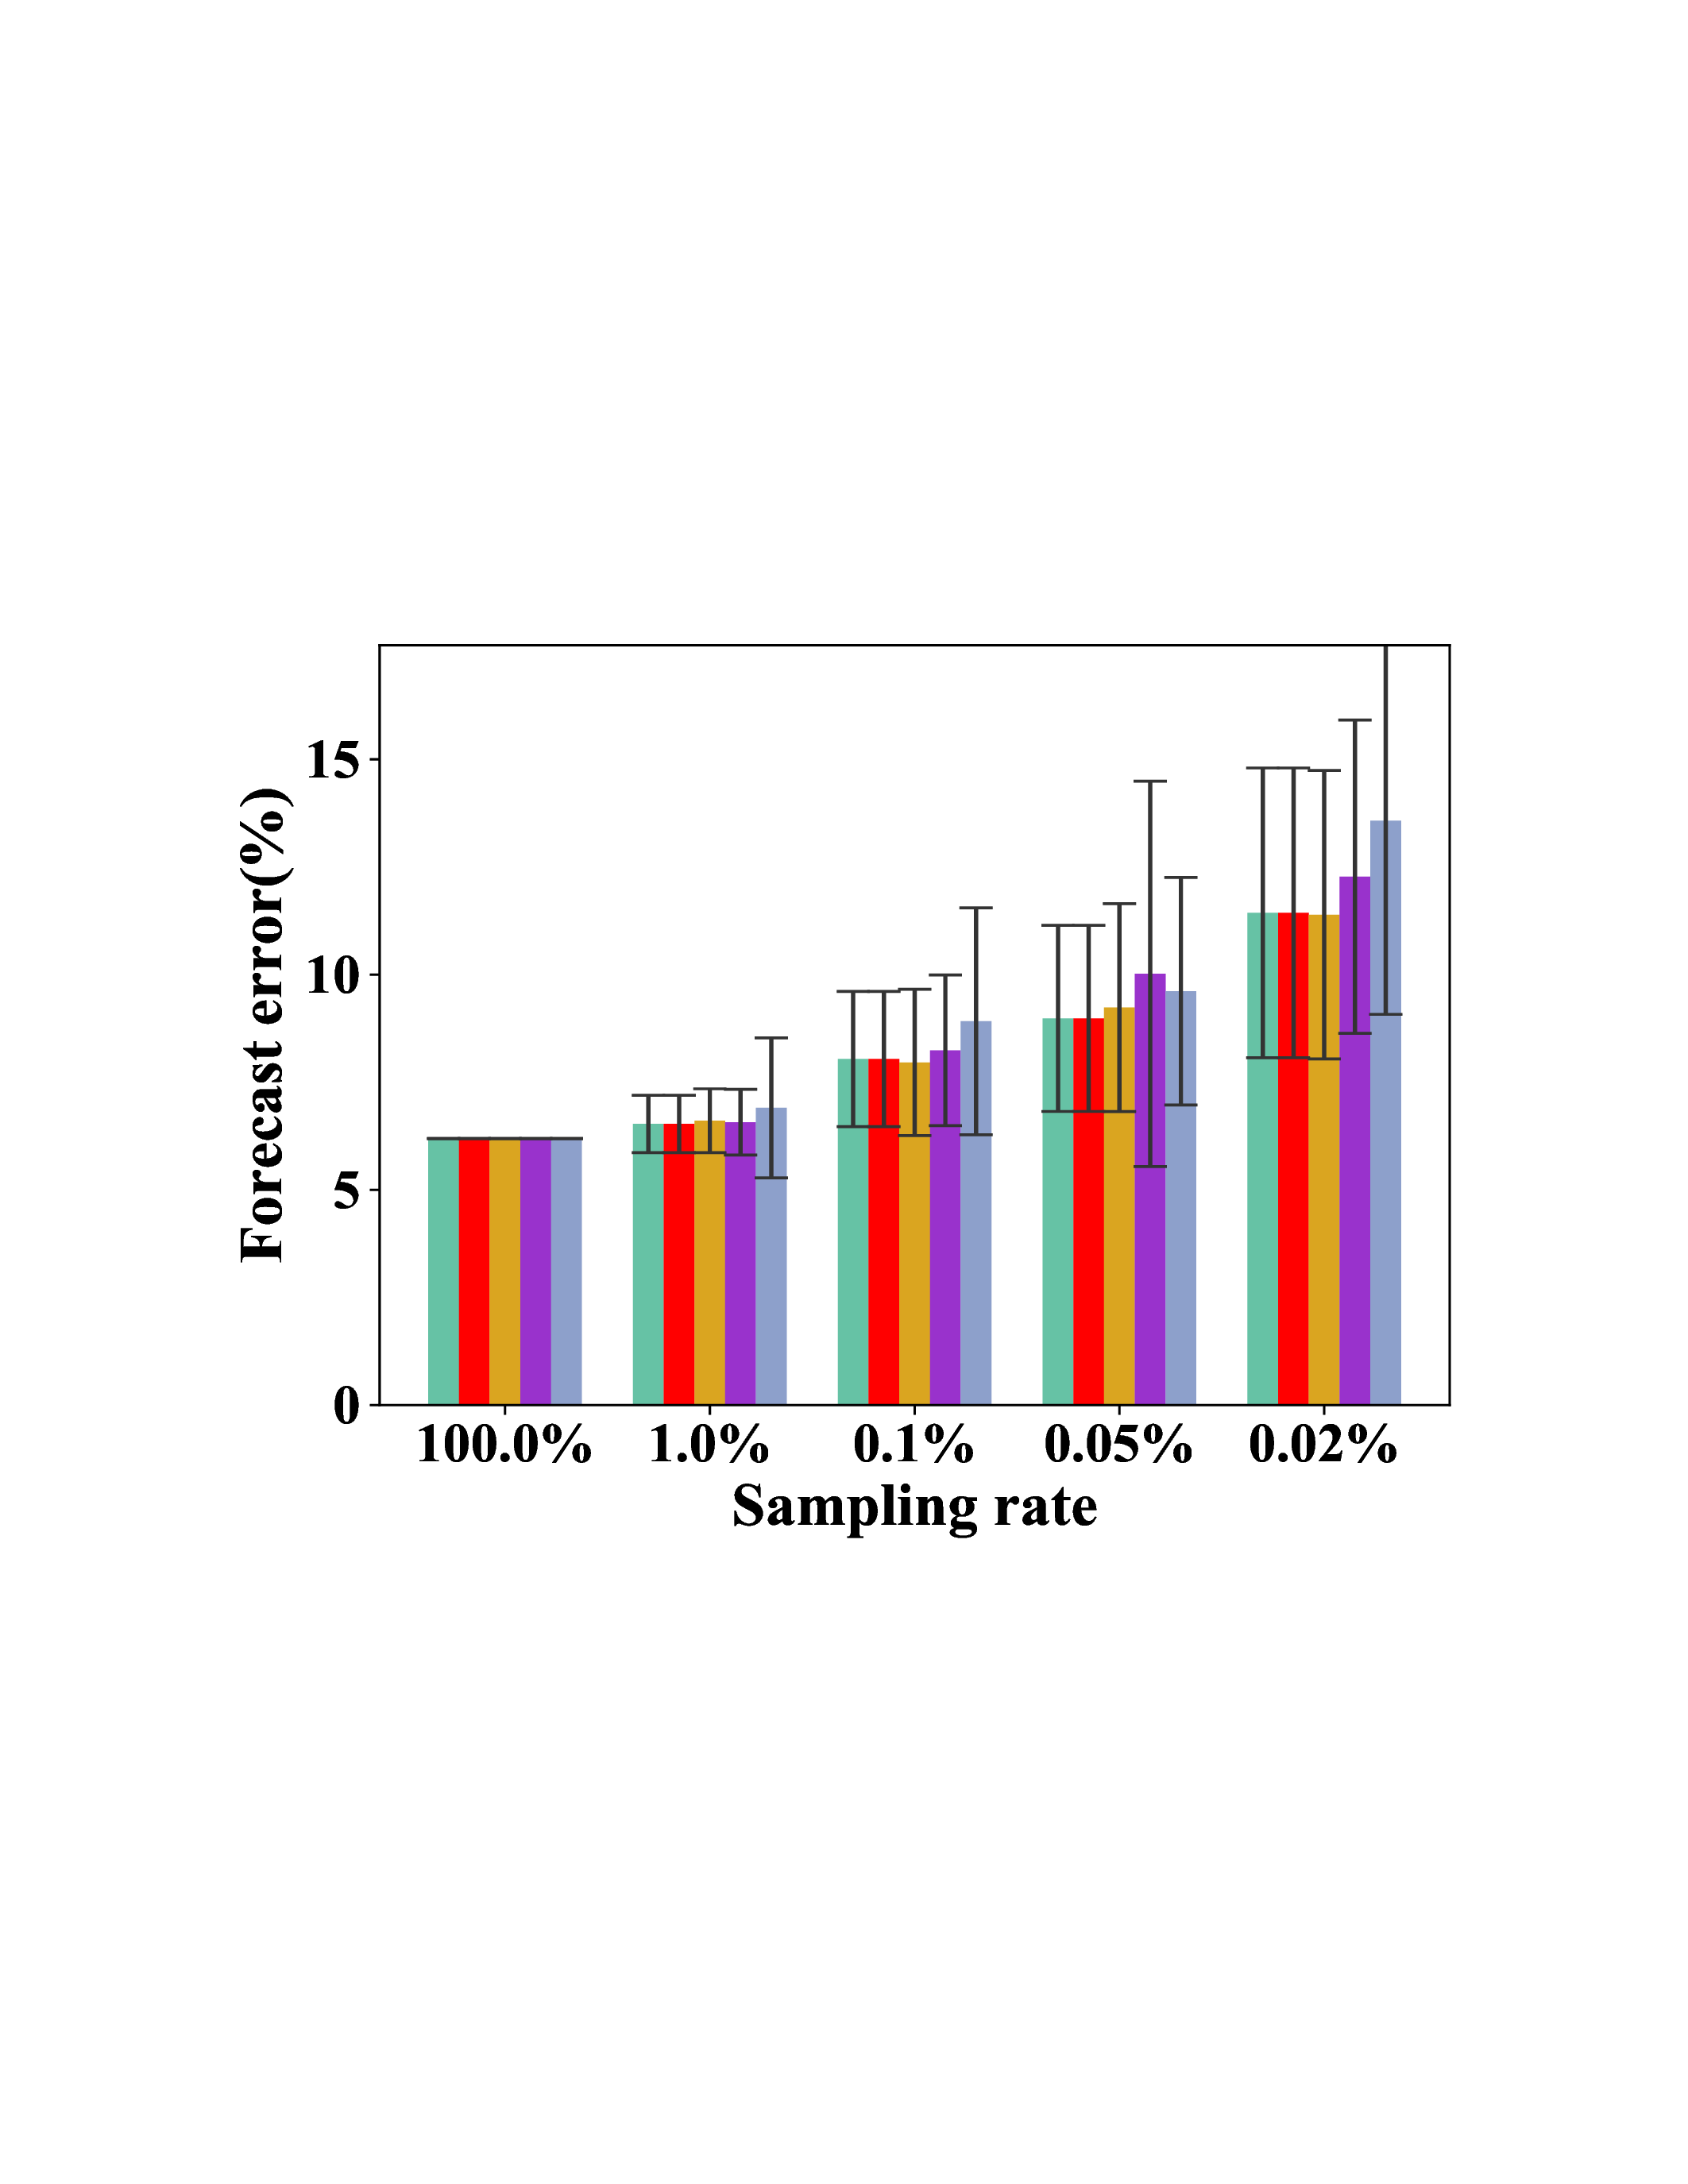}
% \label{fig:side:a}
\end{minipage}
}
\subfigure[Selectivity 1\%]{
\begin{minipage}[t]{0.33\linewidth}
\centering
\includegraphics[width=2.2in, height=2.0in]{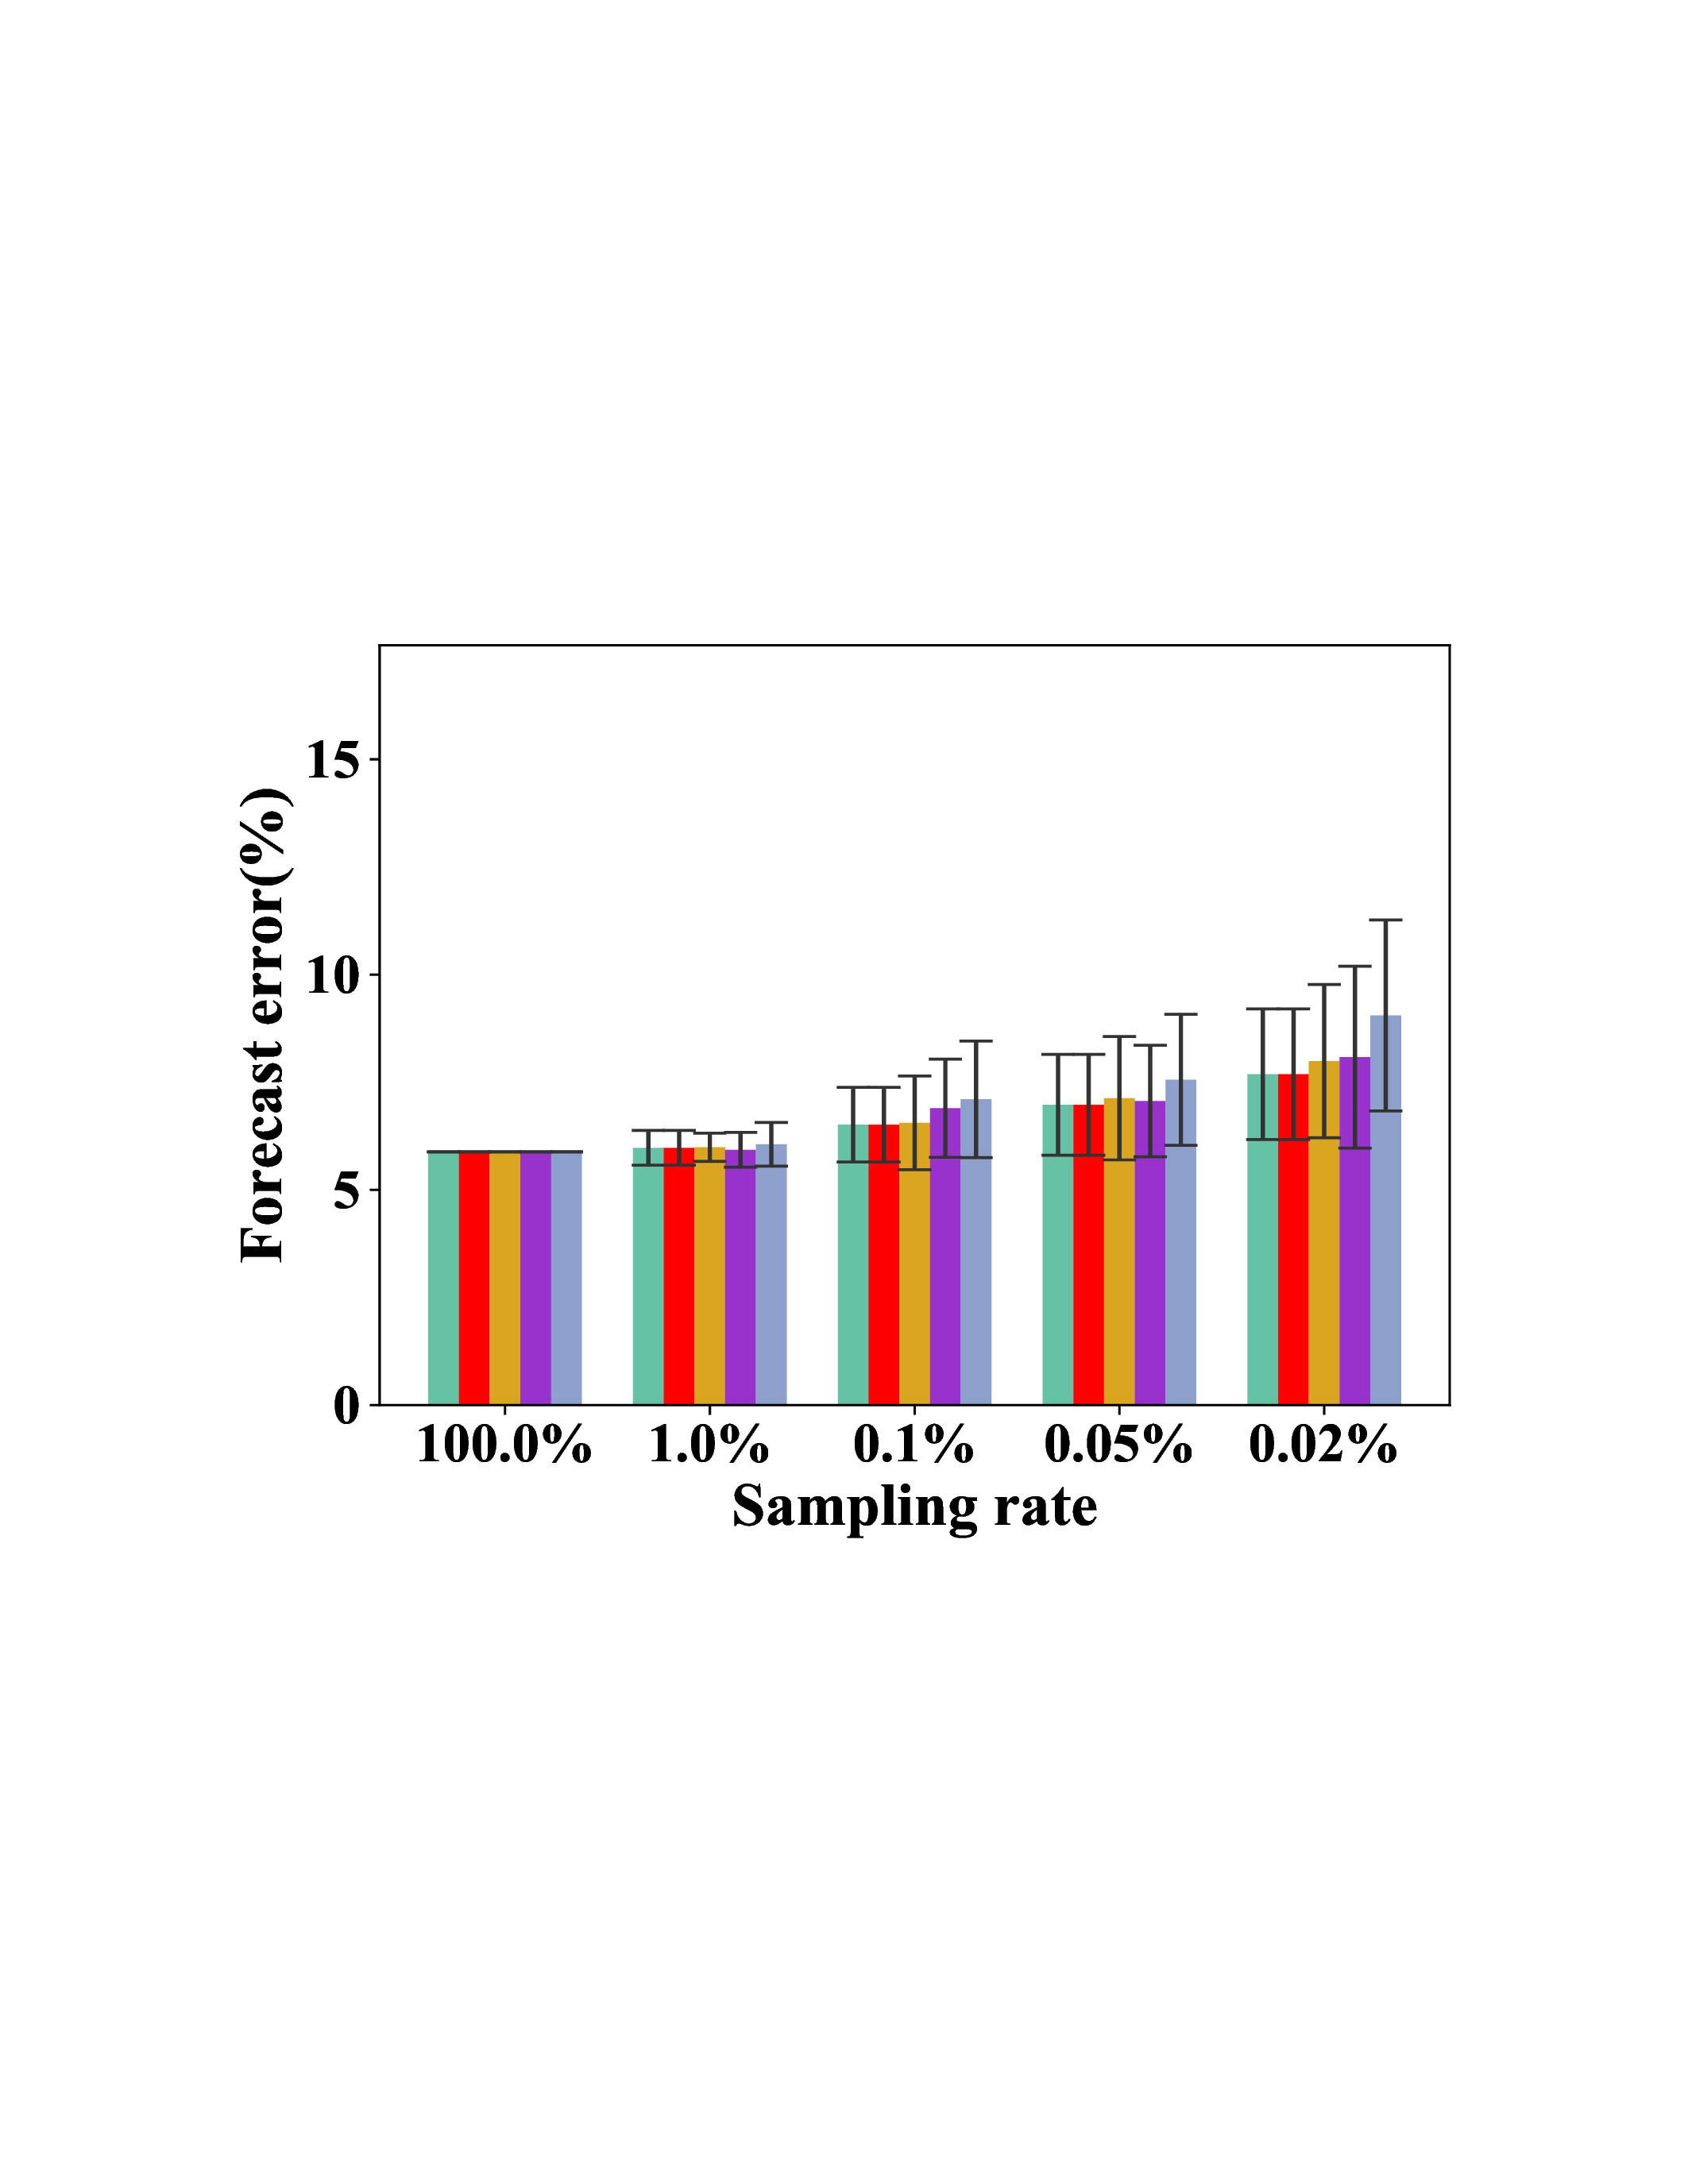}
\end{minipage}
}
\subfigure[Selectivity 5\%]{
\begin{minipage}[t]{0.33\linewidth}
\centering
\includegraphics[width=2.2in, height=2.0in]{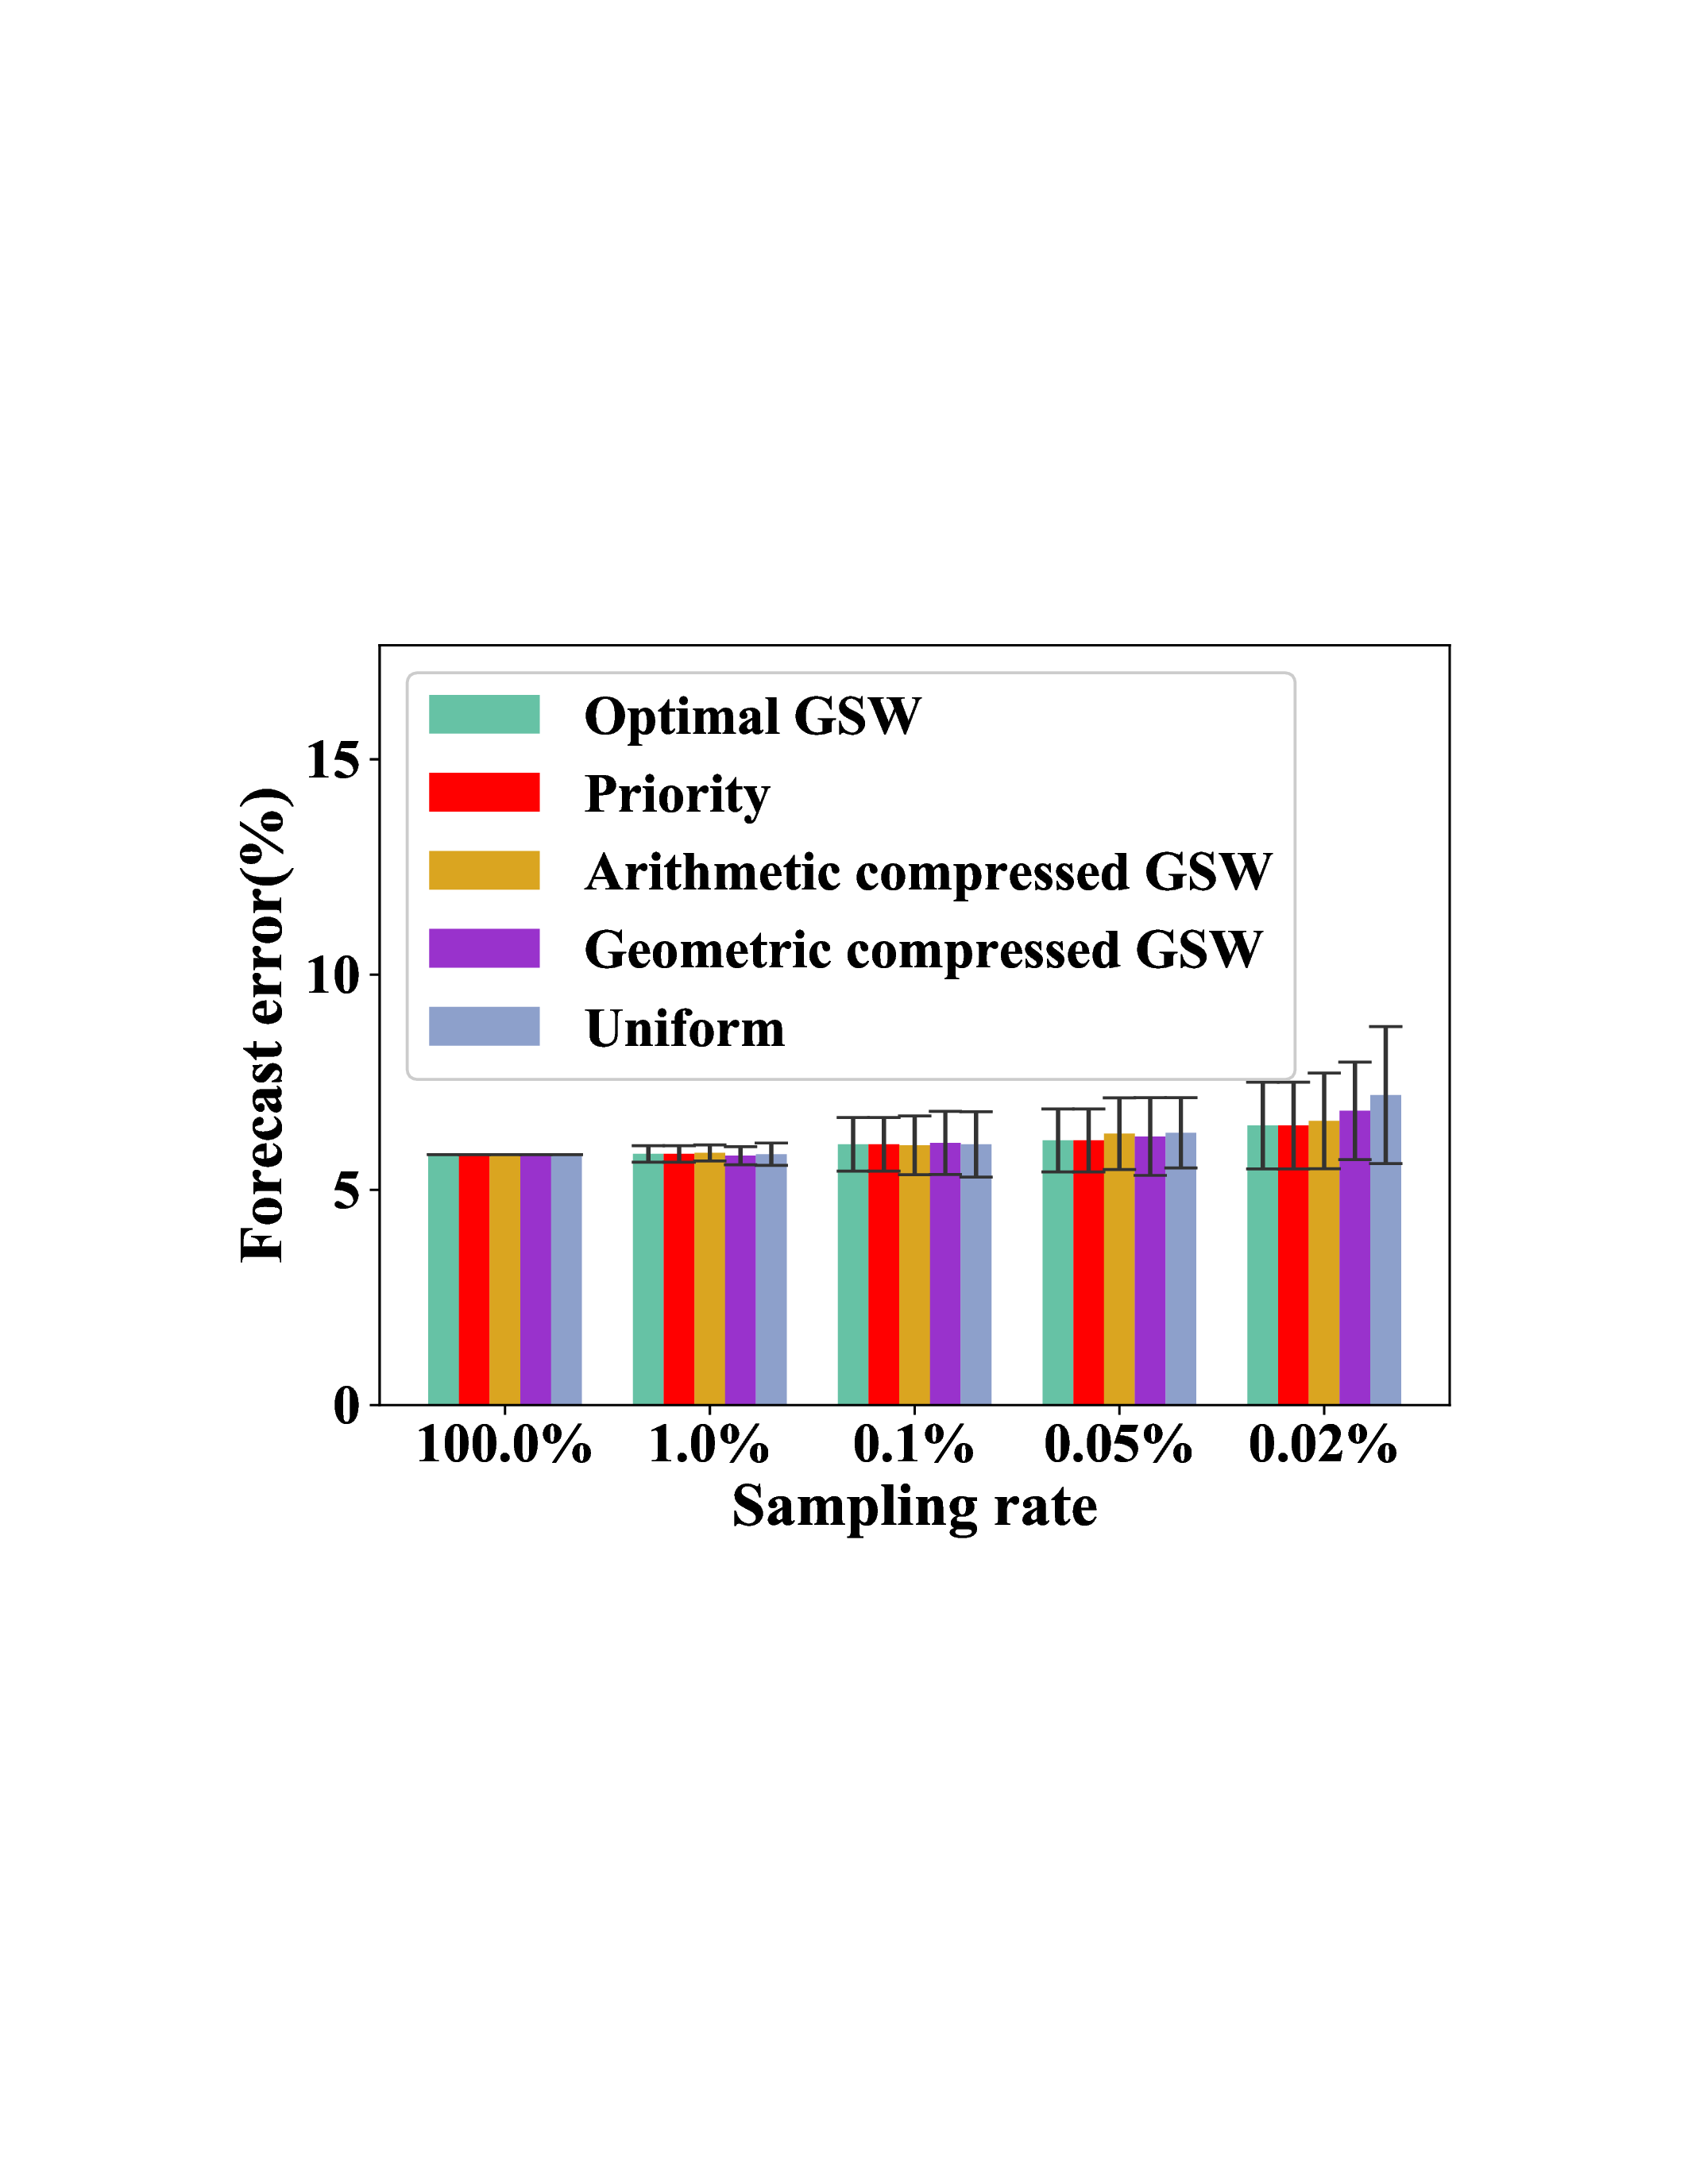}
\end{minipage}
}
\caption{ARIMA prediction error at different selectivity on impression via different sampling methods}
% \label{AQP and ARIMA Performance}
\end{figure*}

%-----Impression不同抽样方法对ARIMA Interval误差的影响----------
\begin{figure*}[hb]
\subfigure[Selectivity 0.5\%]{
\begin{minipage}[t]{0.33\linewidth}
\centering
\includegraphics[width=2.2in, height=2.0in]{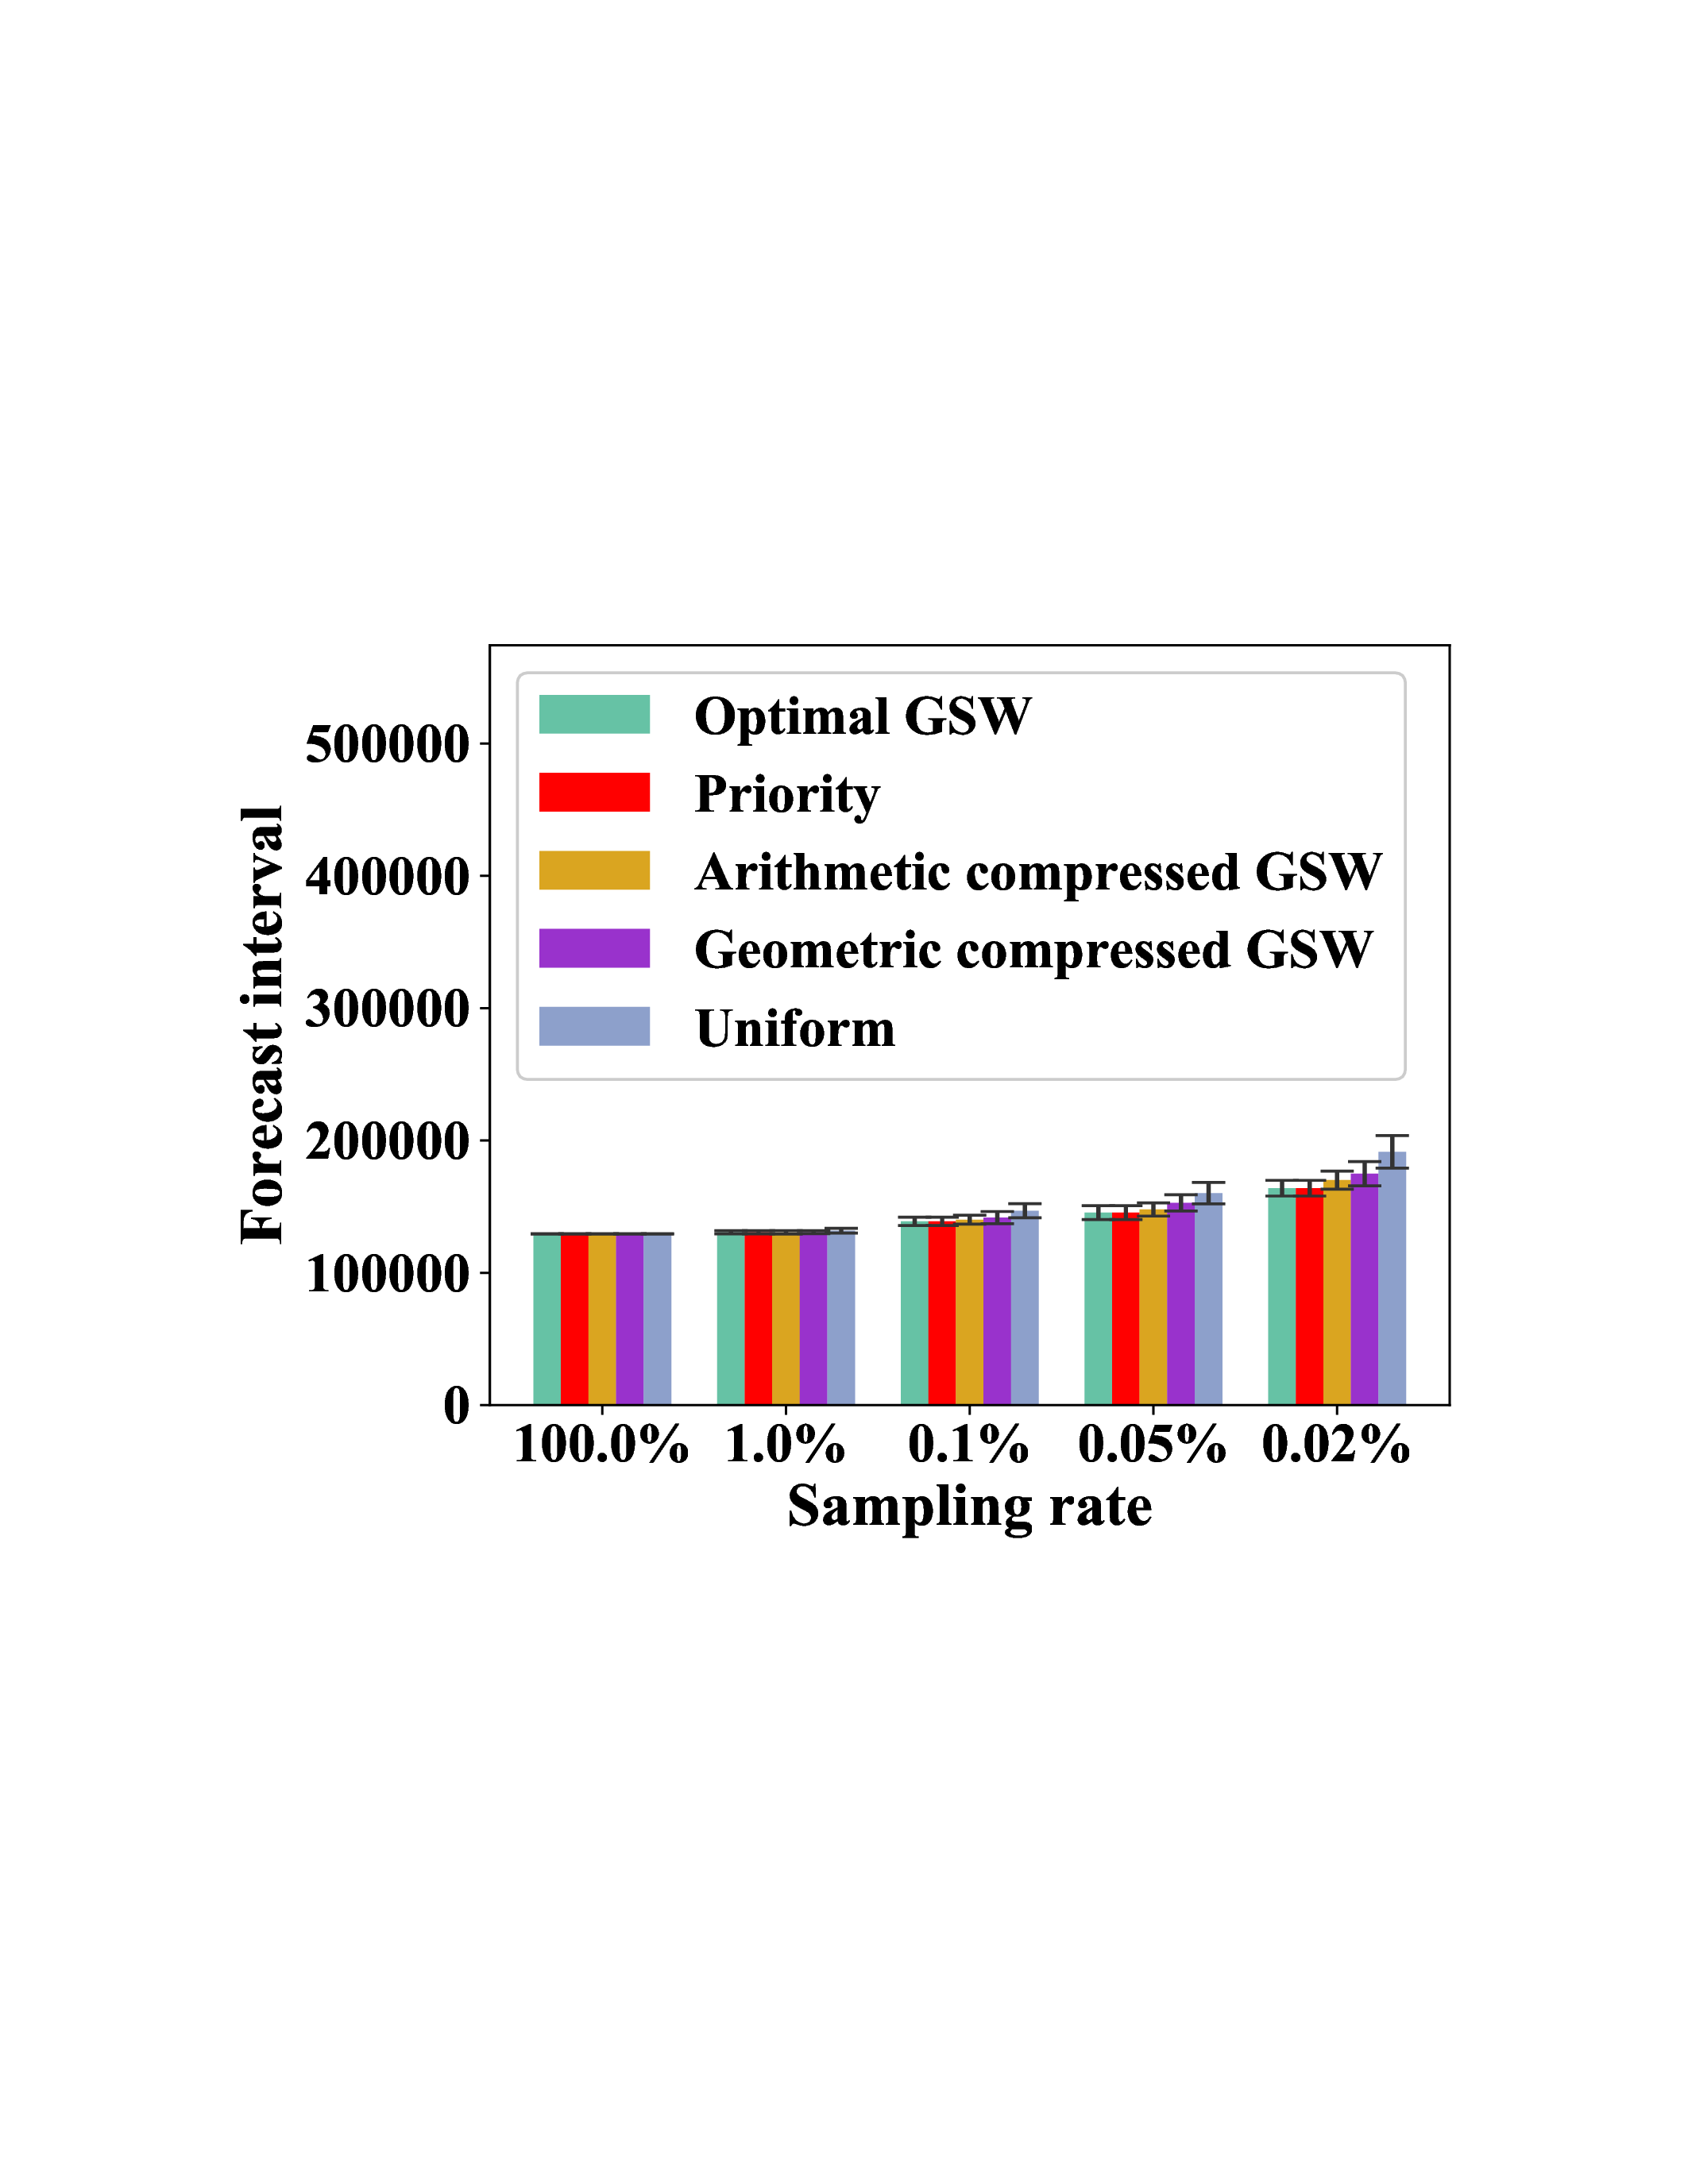}
% \label{fig:side:a}
\end{minipage}
}
\subfigure[Selectivity 1\%]{
\begin{minipage}[t]{0.33\linewidth}
\centering
\includegraphics[width=2.2in, height=2.0in]{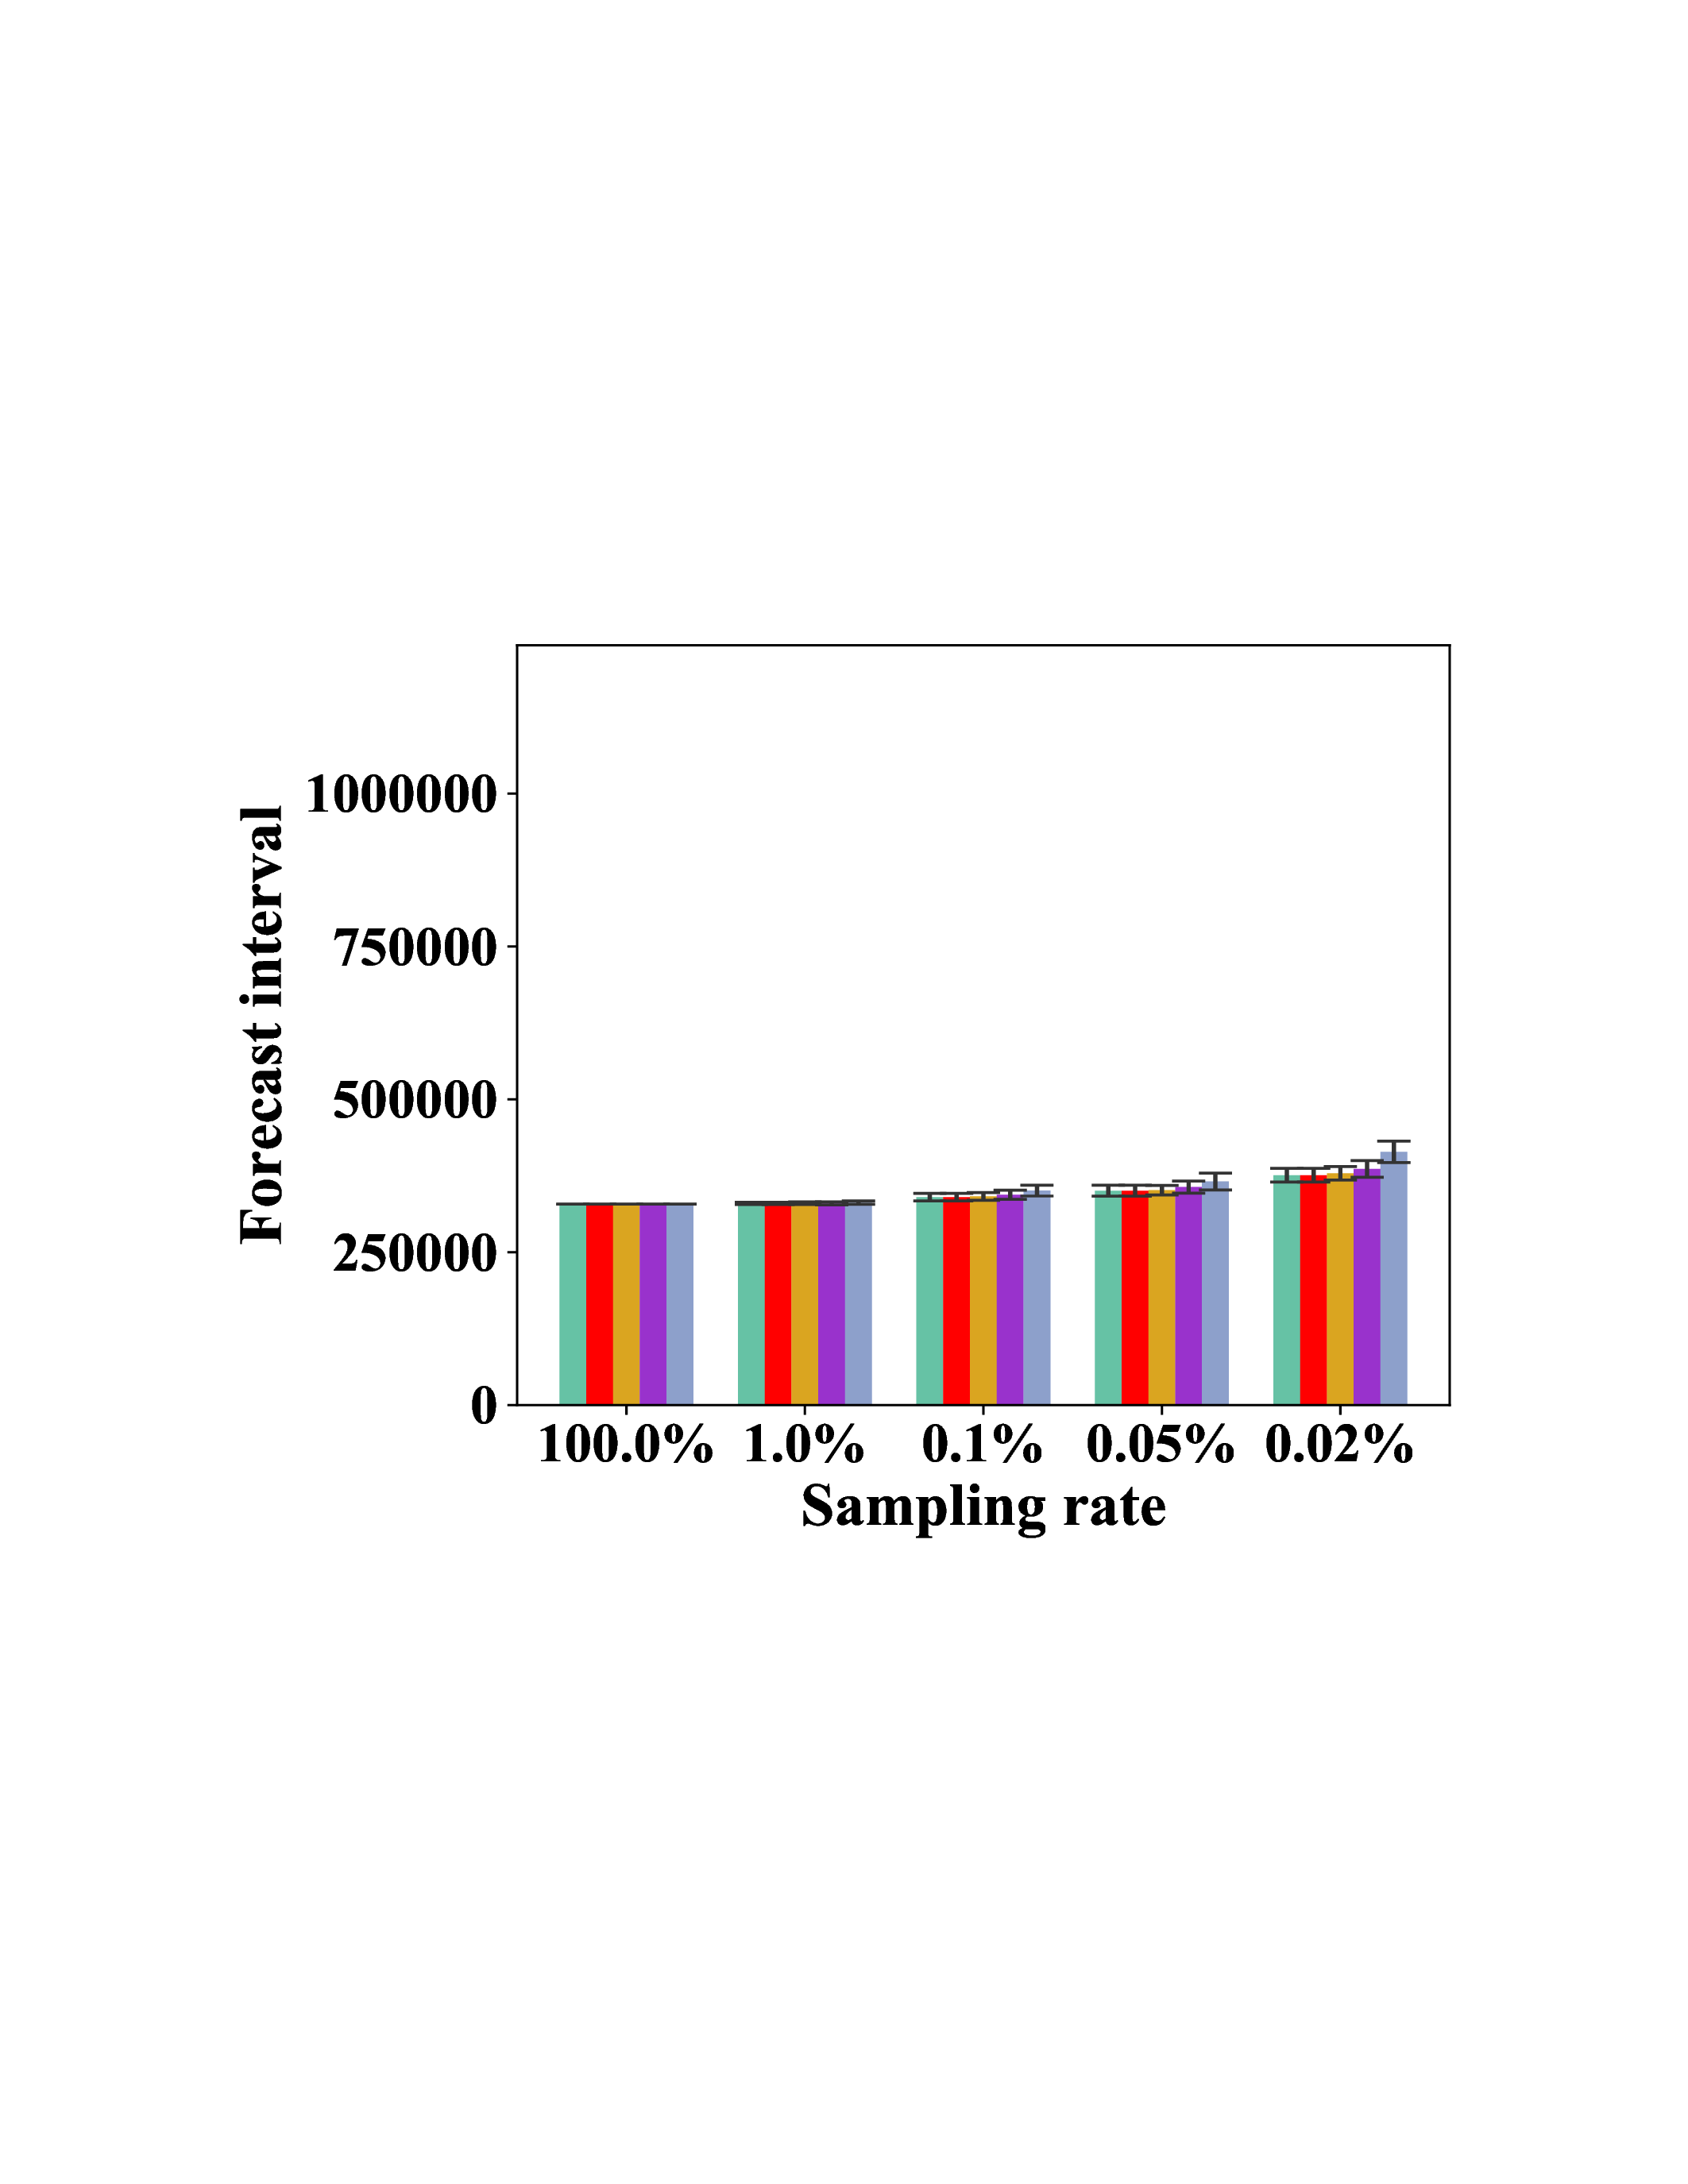}
\end{minipage}
}
\subfigure[Selectivity 5\%]{
\begin{minipage}[t]{0.33\linewidth}
\centering
\includegraphics[width=2.2in, height=2.0in]{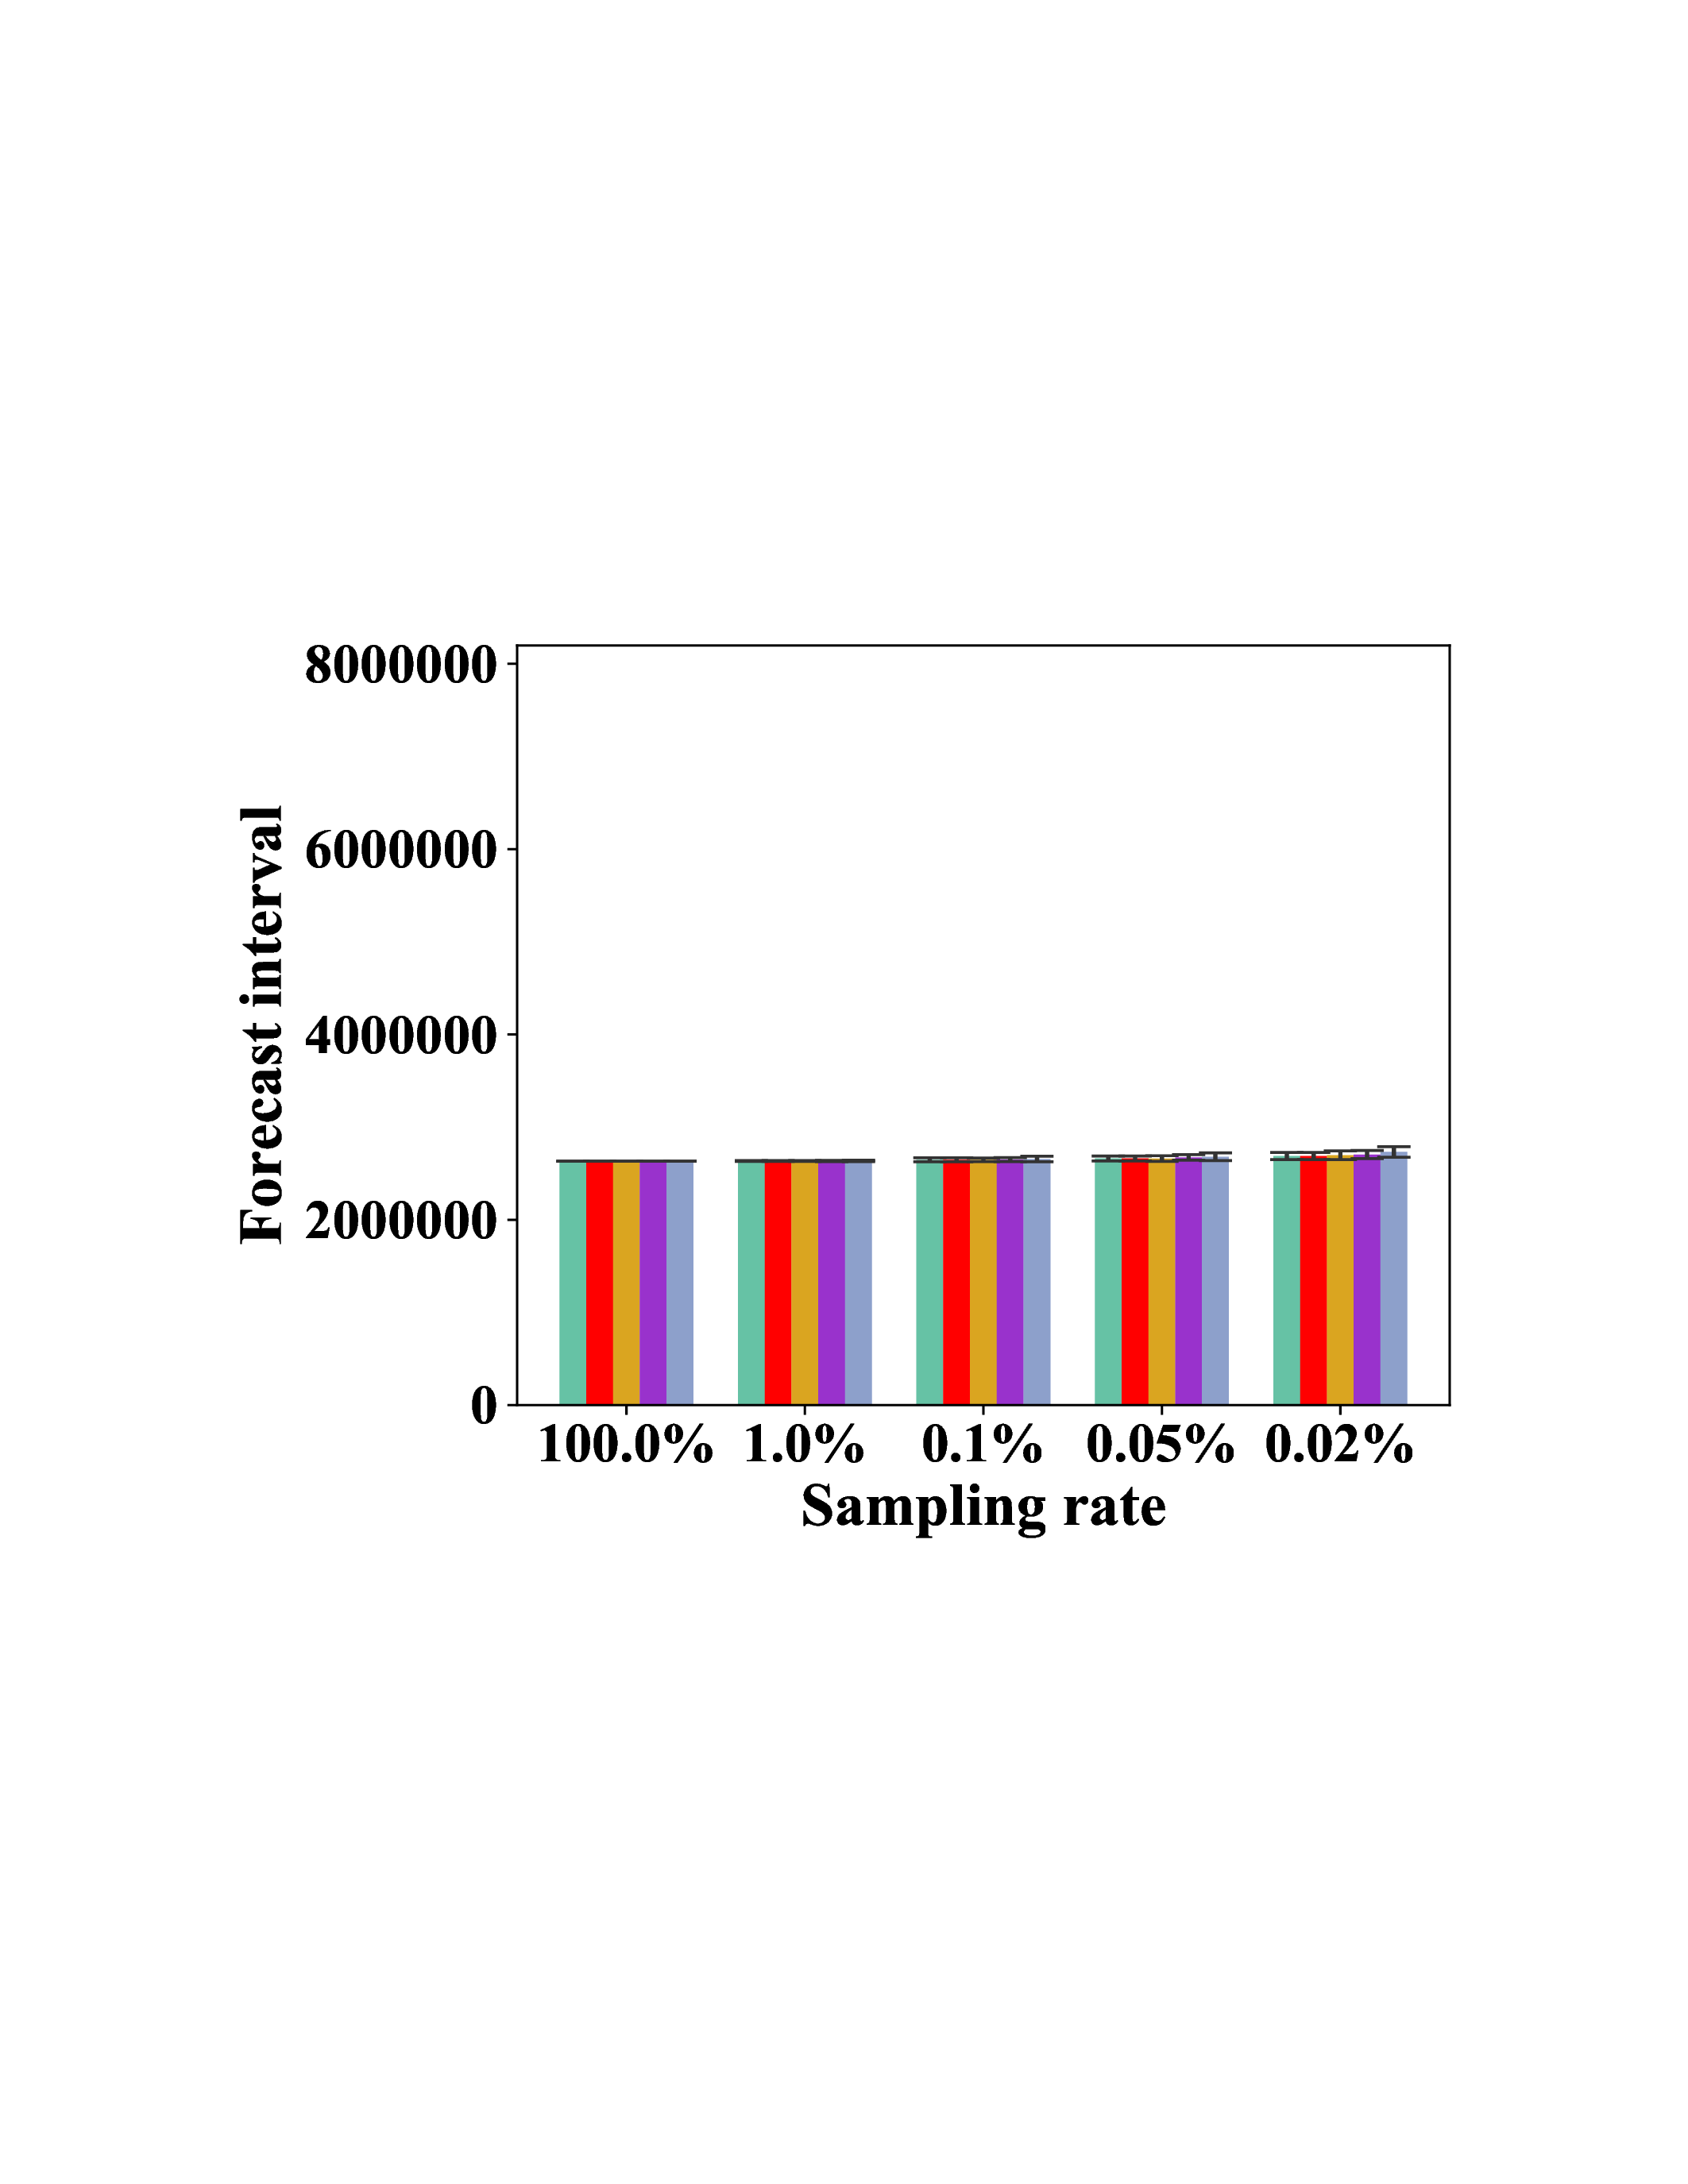}
\end{minipage}
}
\caption{ARIMA prediction interval at different selectivity on impression via different sampling methods}
% \label{AQP and ARIMA Performance}
\end{figure*}

%============================

%-----Click不同抽样方法对AQP误差的影响----------
\begin{figure*}[hb]
\subfigure[Selectivity 0.5\%]{
\begin{minipage}[t]{0.33\linewidth}
\centering
\includegraphics[width=2.2in, height=2.0in]{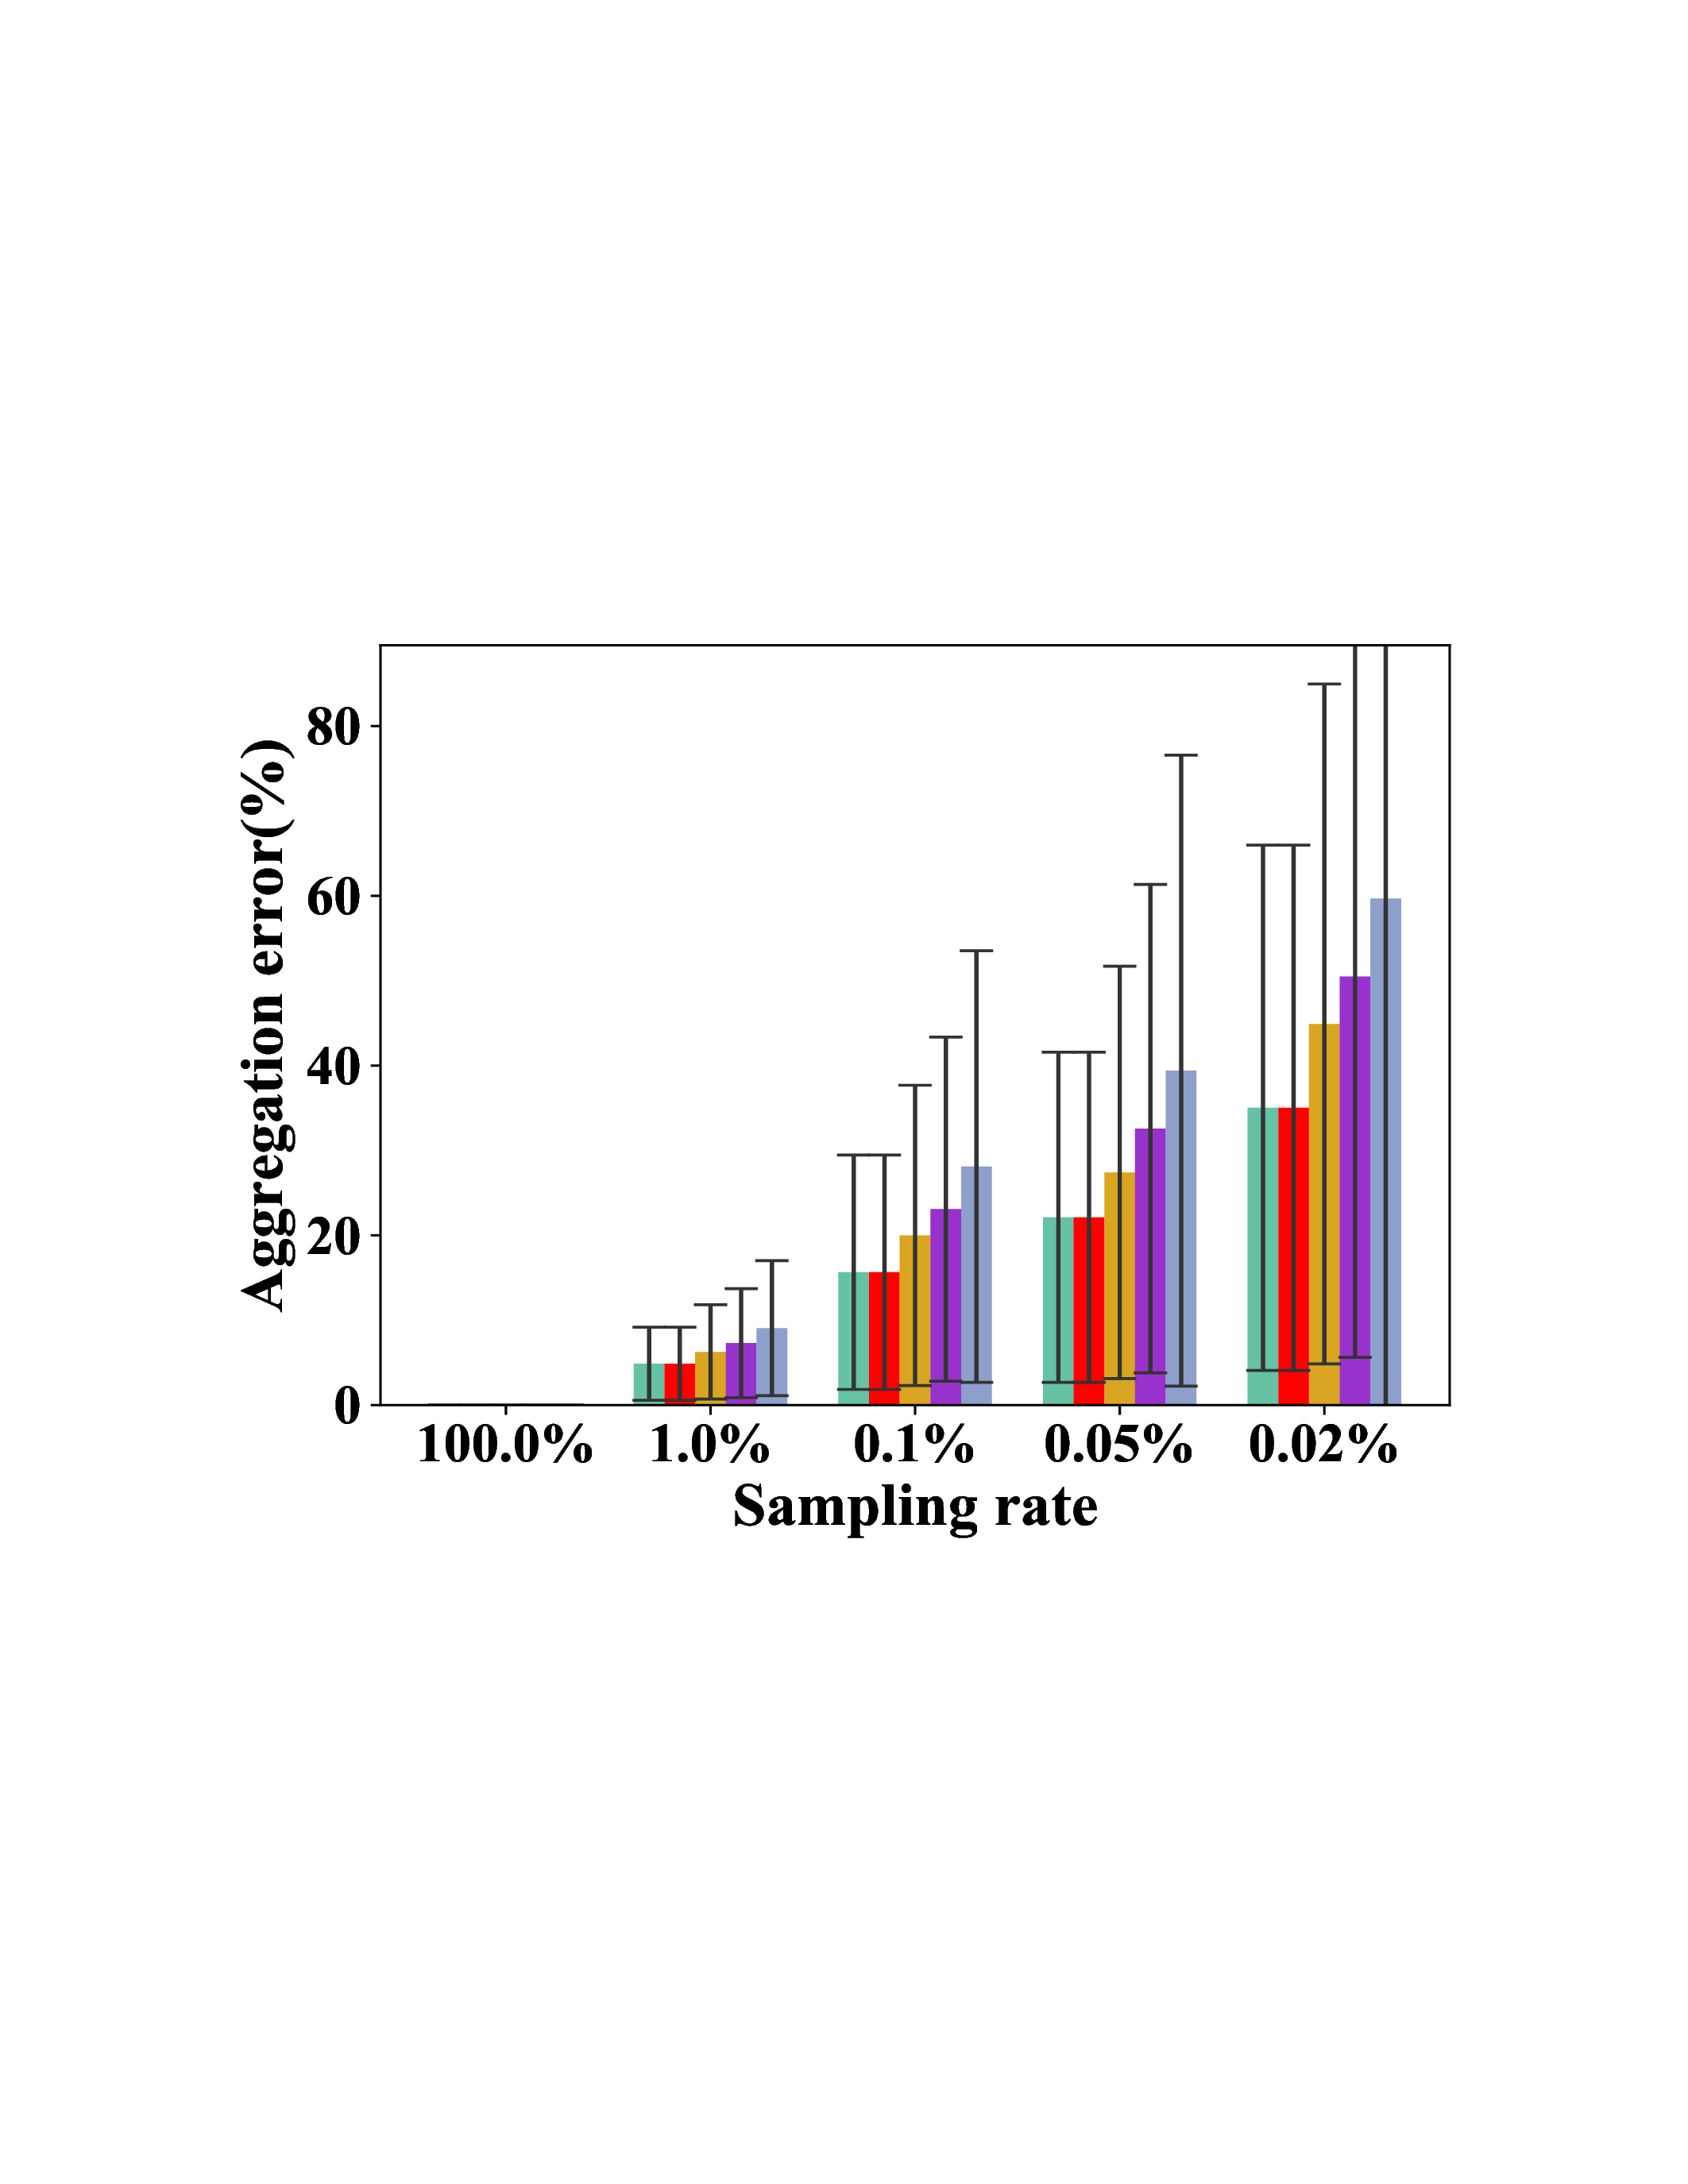}
% \label{fig:side:a}
\end{minipage}
}
\subfigure[Selectivity 1\%]{
\begin{minipage}[t]{0.33\linewidth}
\centering
\includegraphics[width=2.2in, height=2.0in]{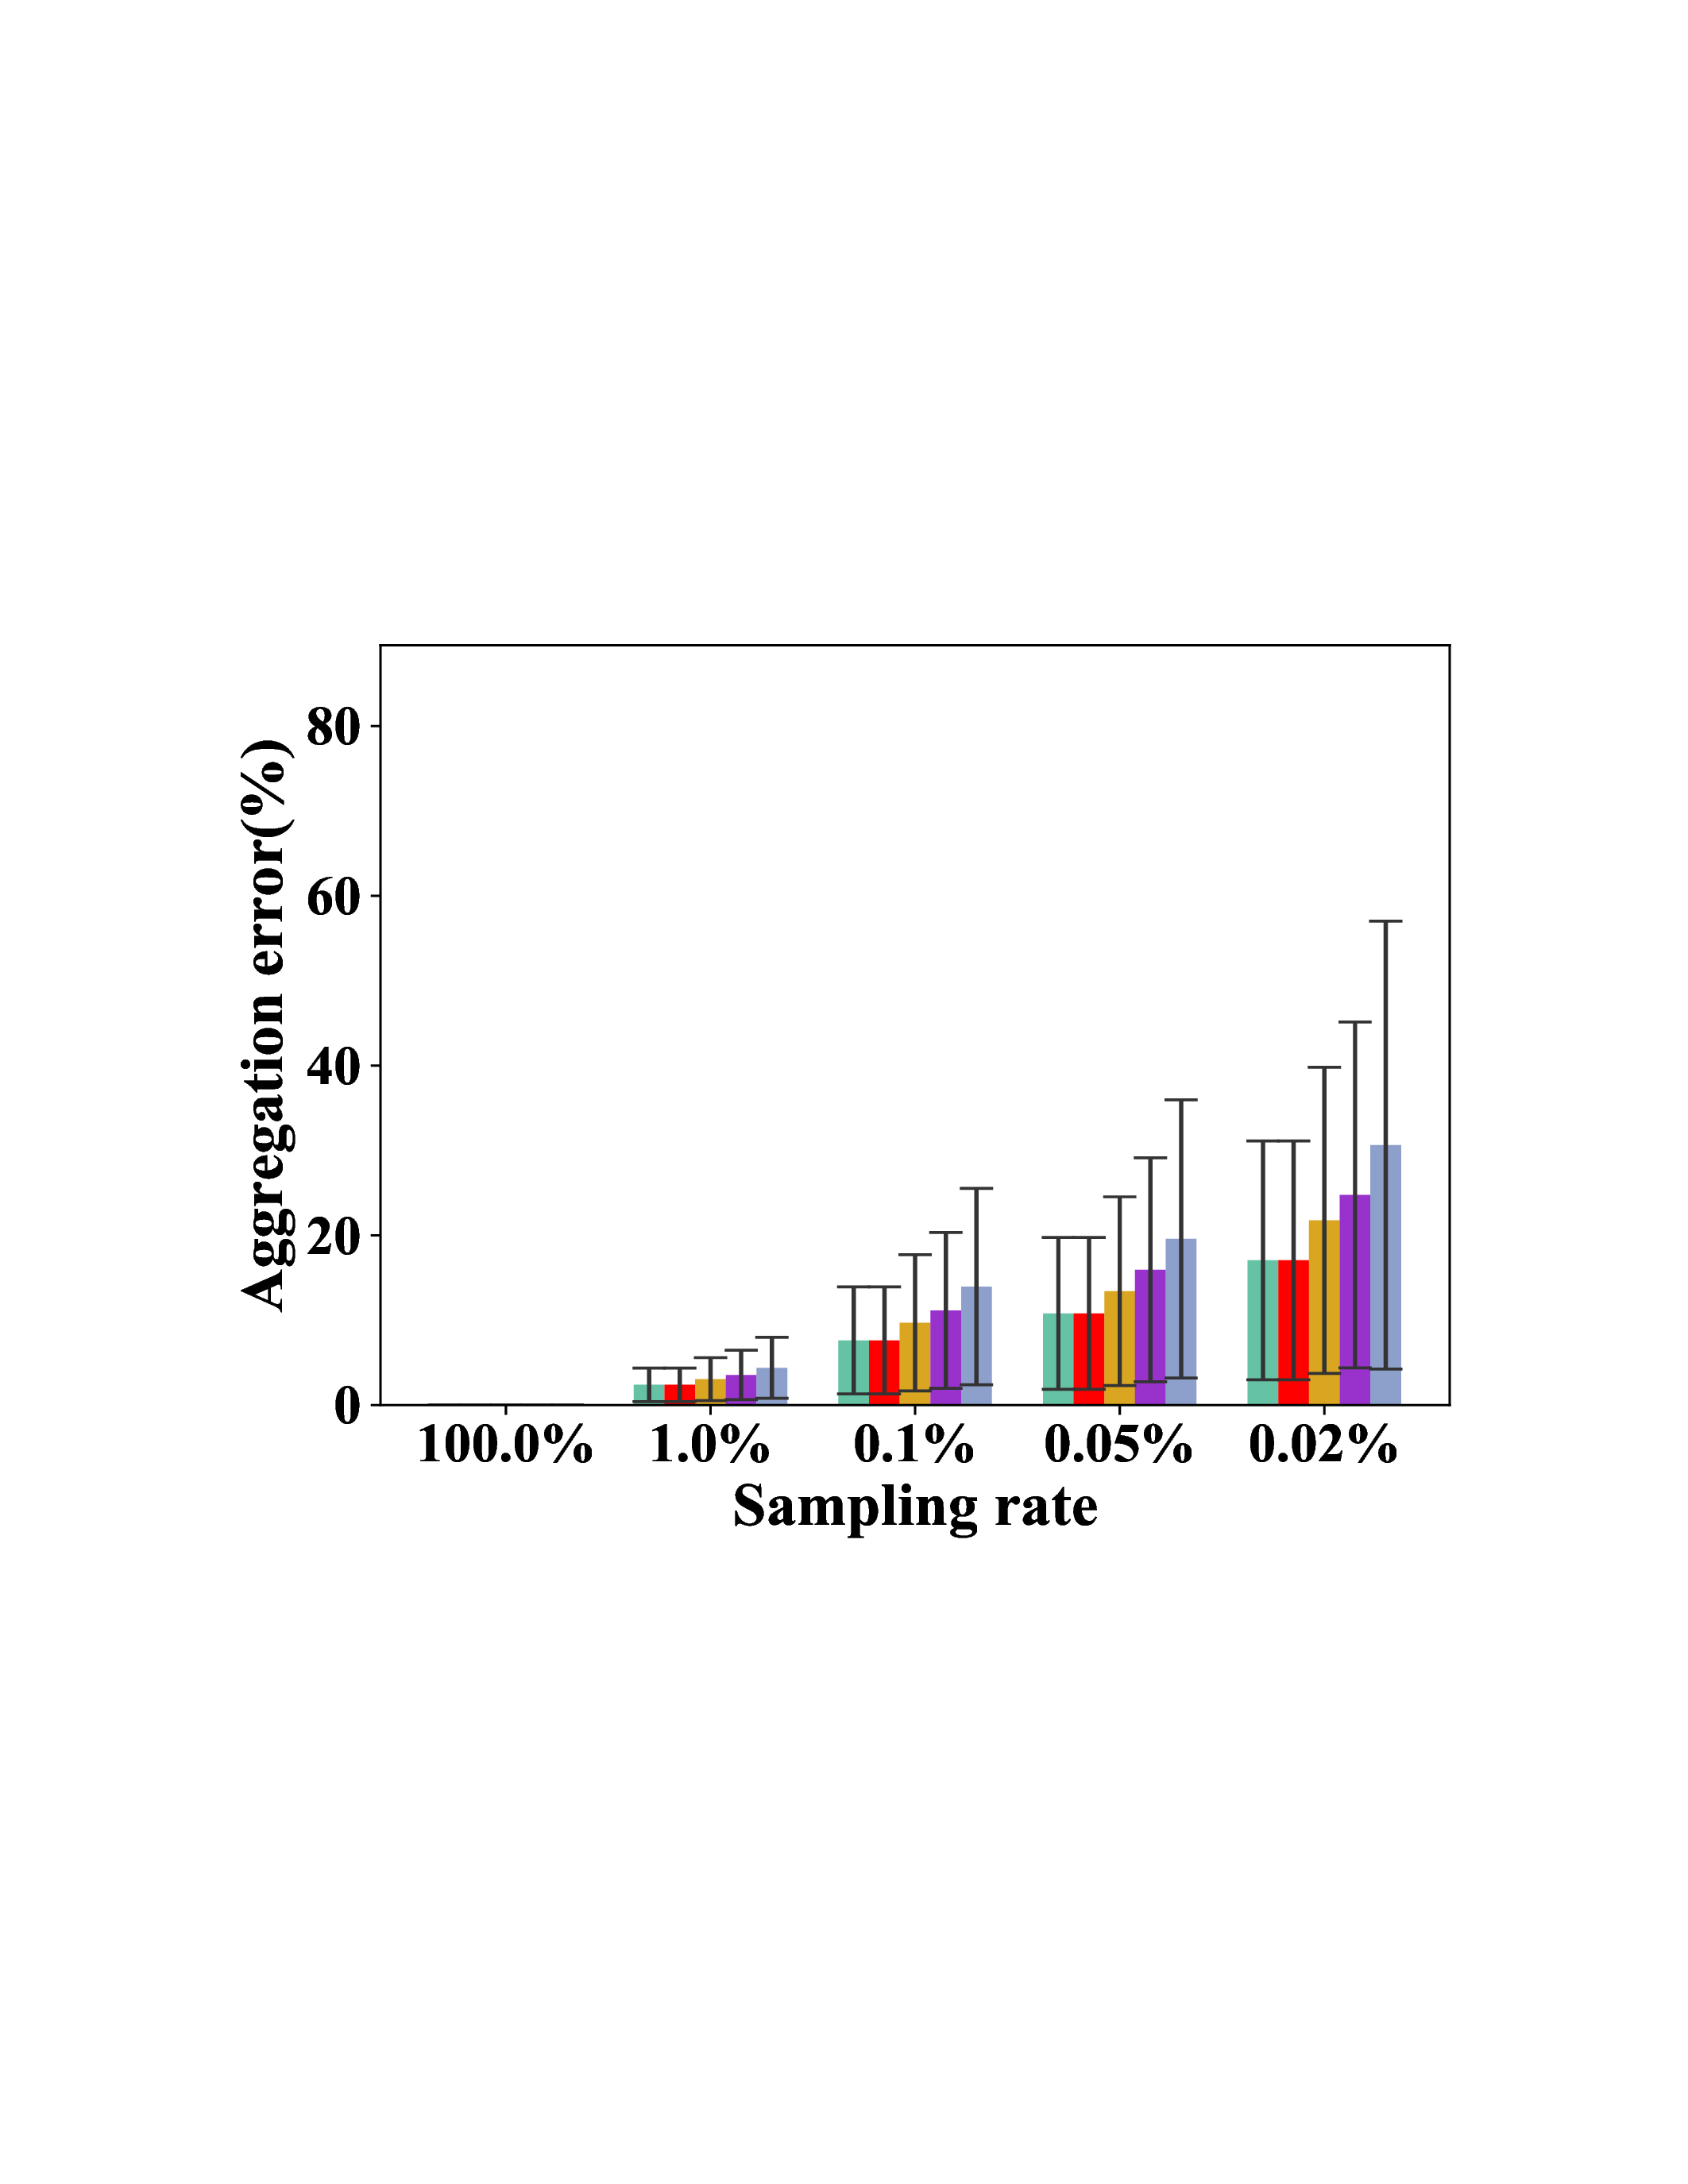}
\end{minipage}
}
\subfigure[Selectivity 5\%]{
\begin{minipage}[t]{0.33\linewidth}
\centering
\includegraphics[width=2.2in, height=2.0in]{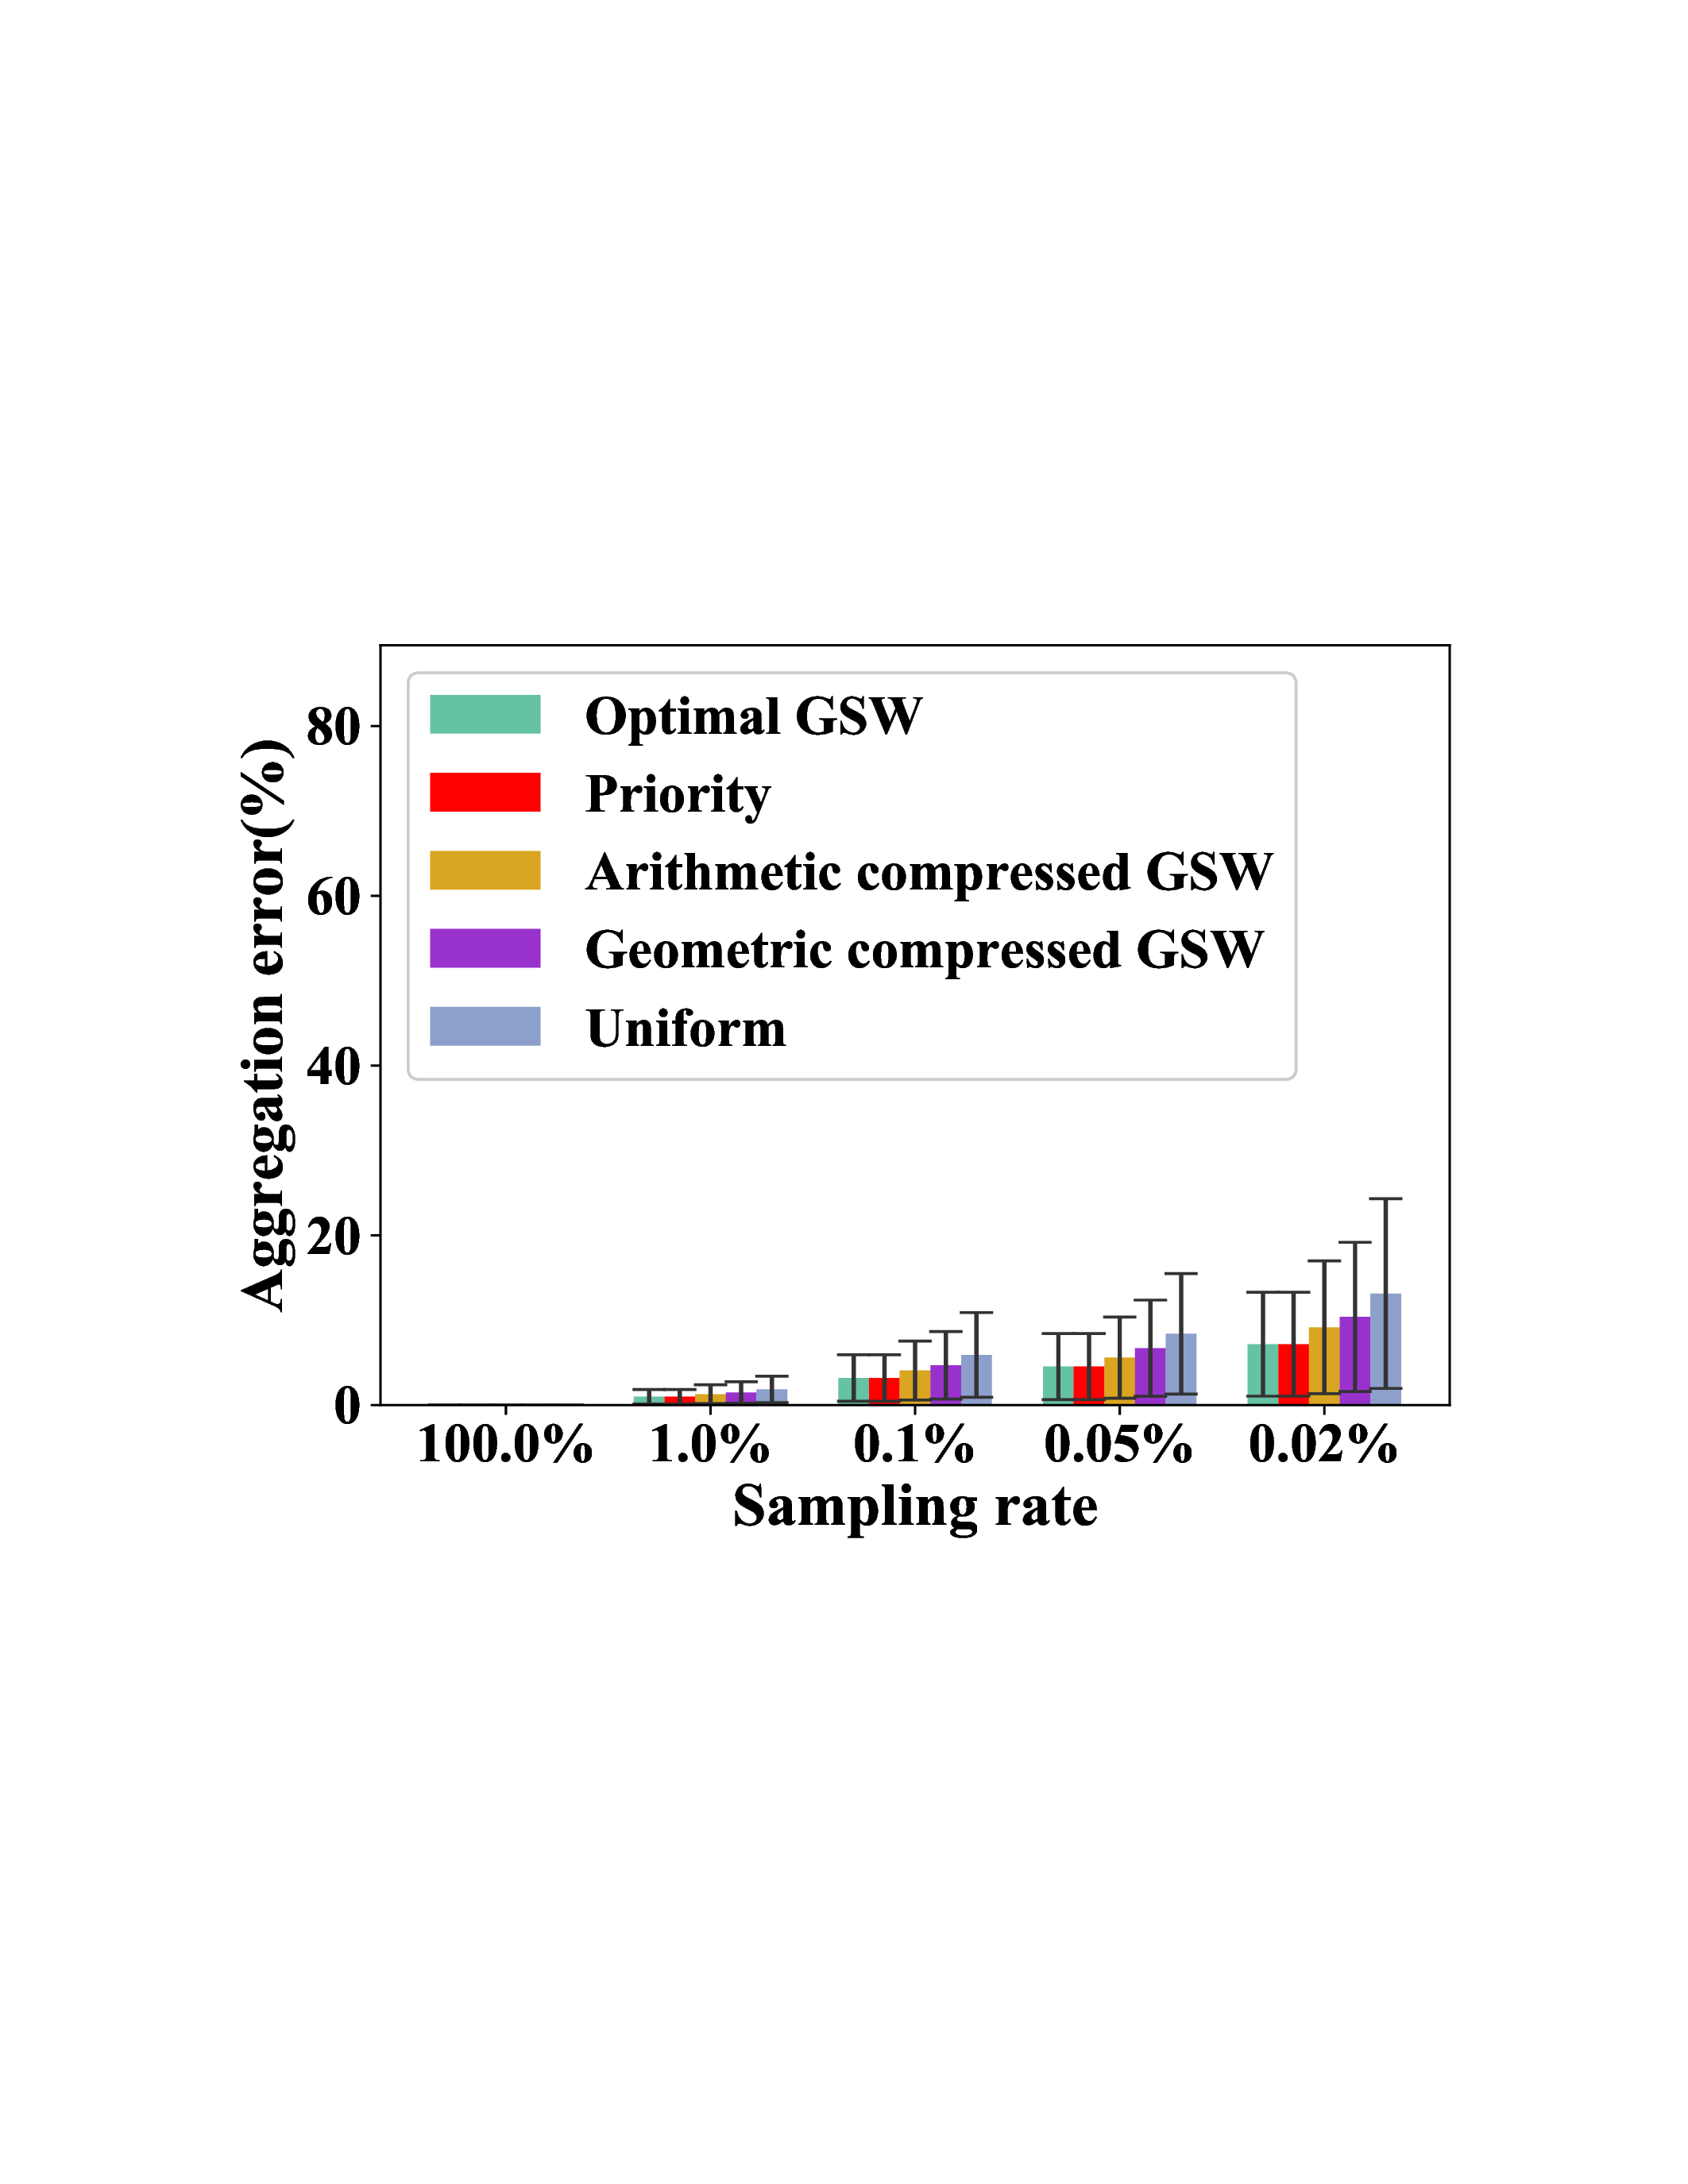}
\end{minipage}
}
\caption{AQP error at different selectivity on click via different sampling methods}
% \label{AQP and ARIMA Performance}
\end{figure*}

%-----Click不同抽样方法对ARIMA误差的影响----------
\begin{figure*}[hb]
\subfigure[Selectivity 0.5\%]{
\begin{minipage}[t]{0.33\linewidth}
\centering
\includegraphics[width=2.2in, height=2.0in]{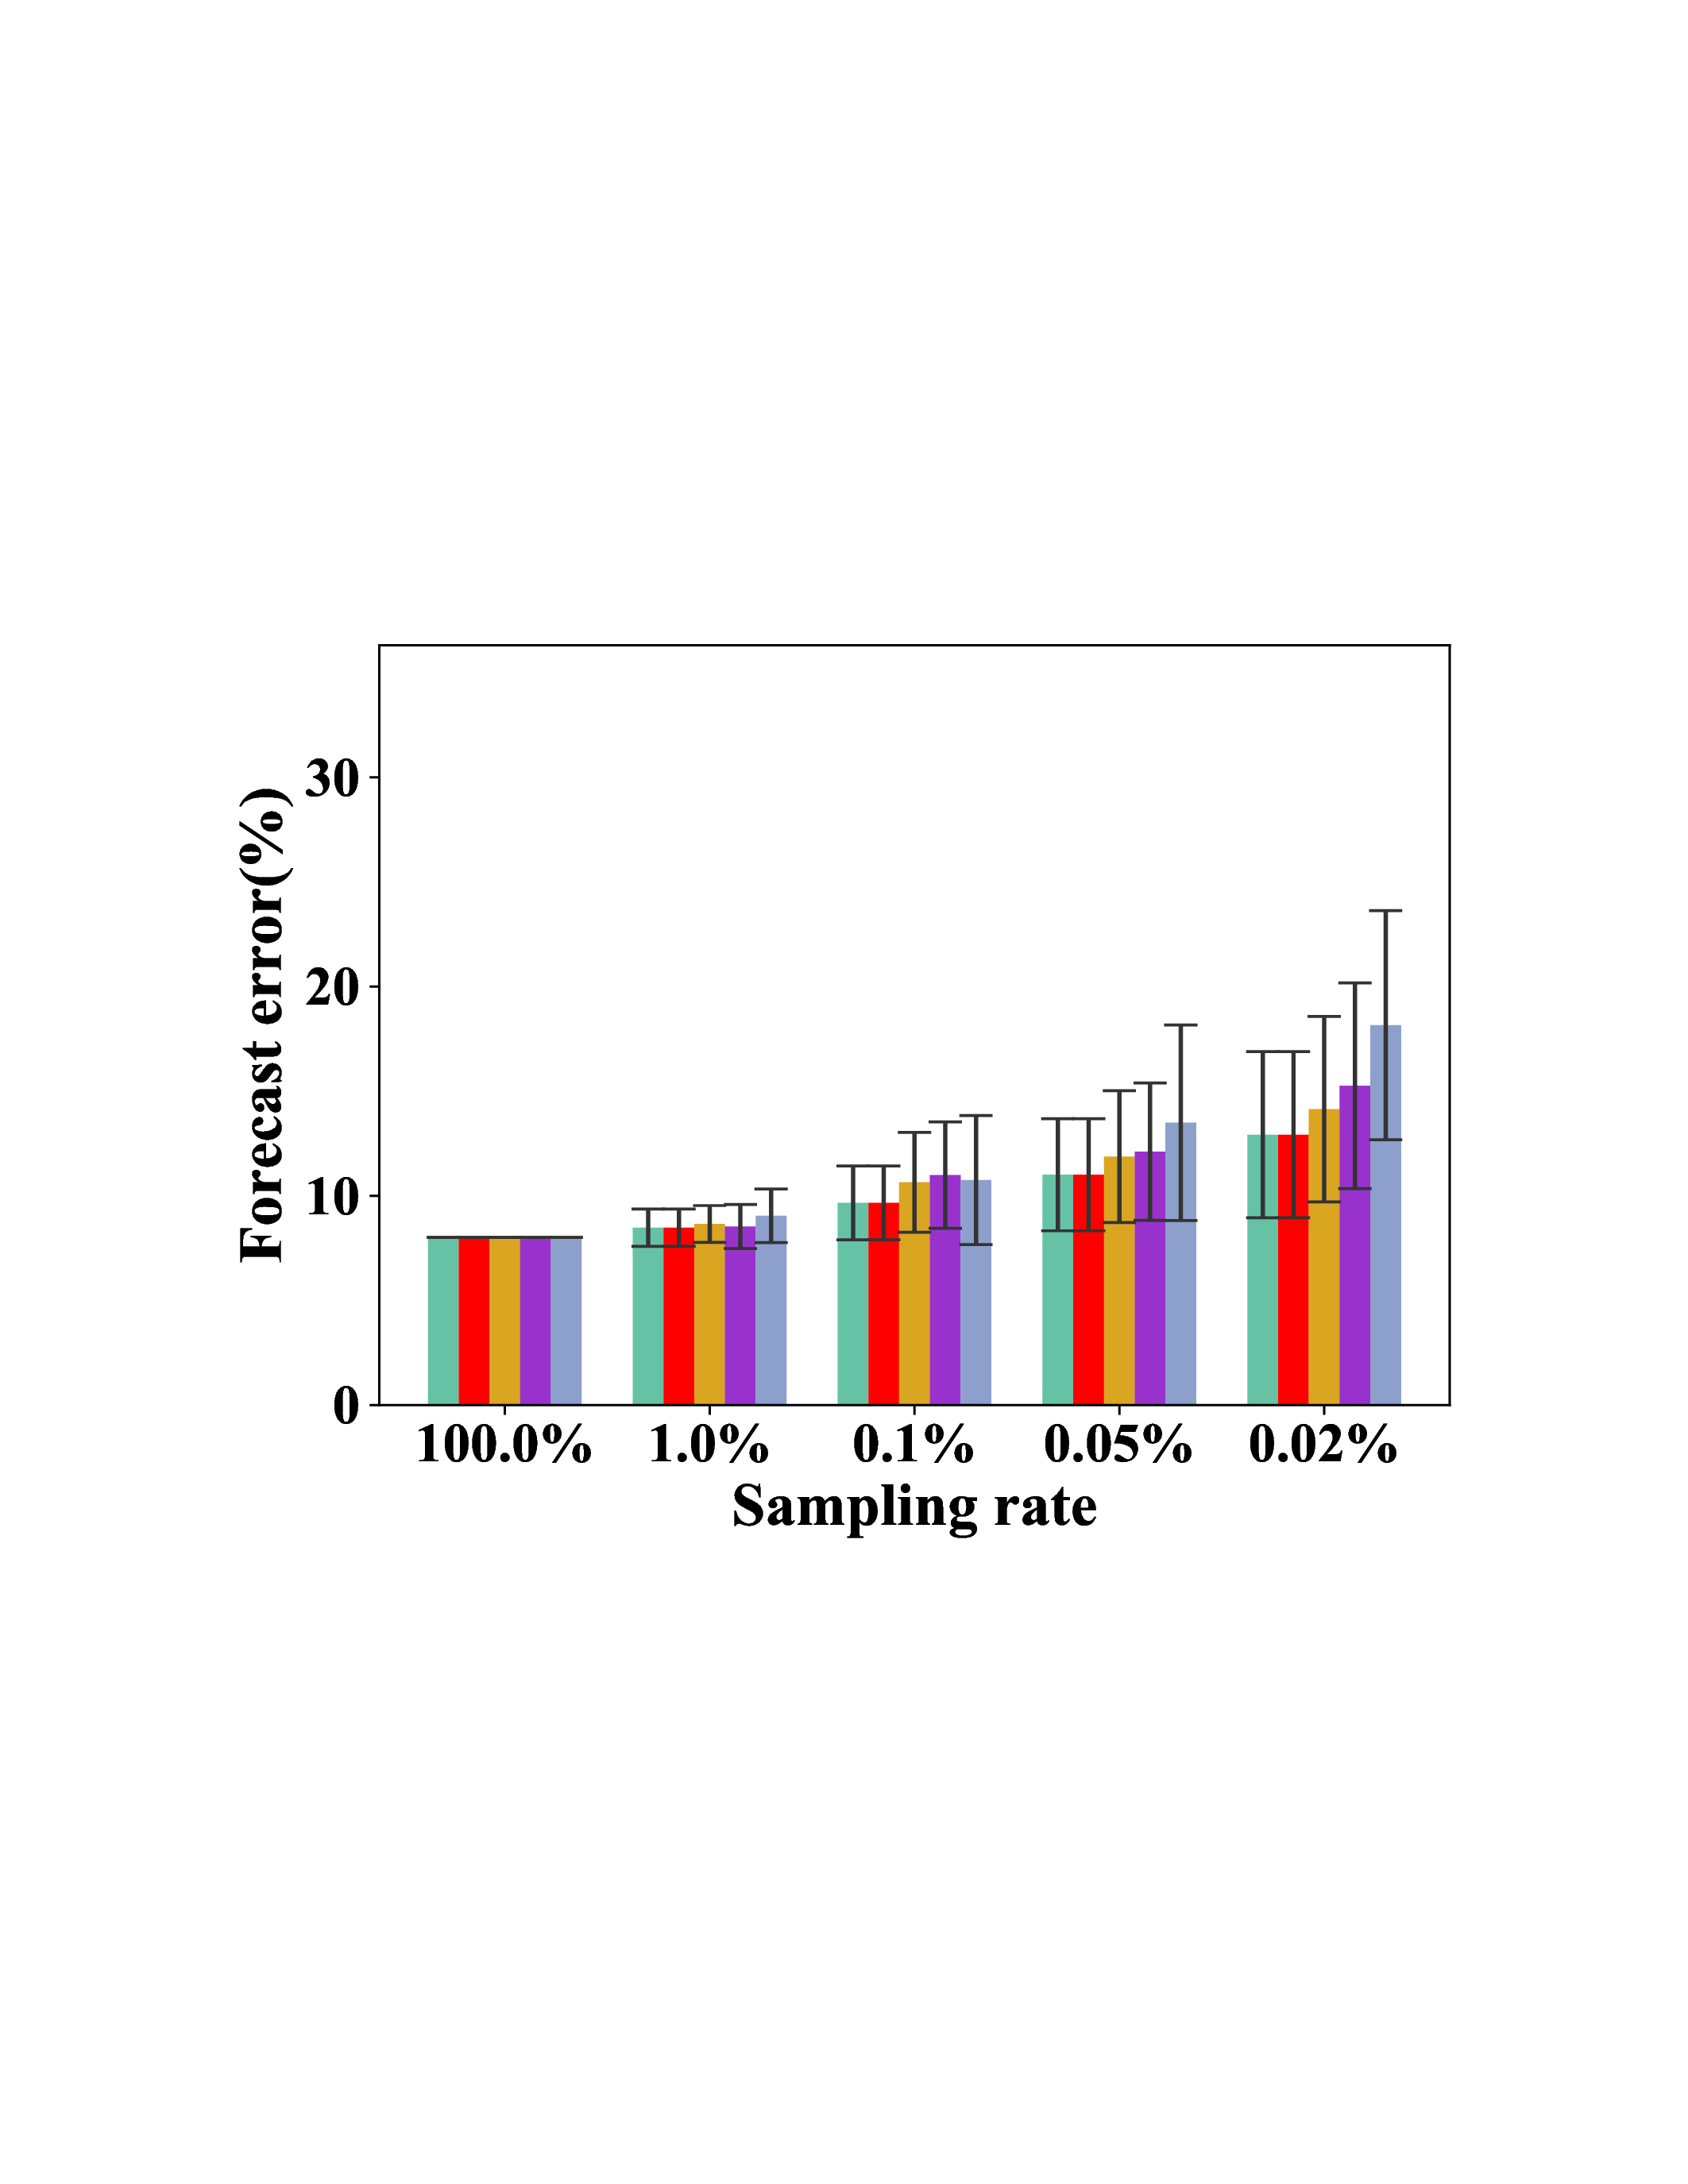}
% \label{fig:side:a}
\end{minipage}
}
\subfigure[Selectivity 1\%]{
\begin{minipage}[t]{0.33\linewidth}
\centering
\includegraphics[width=2.2in, height=2.0in]{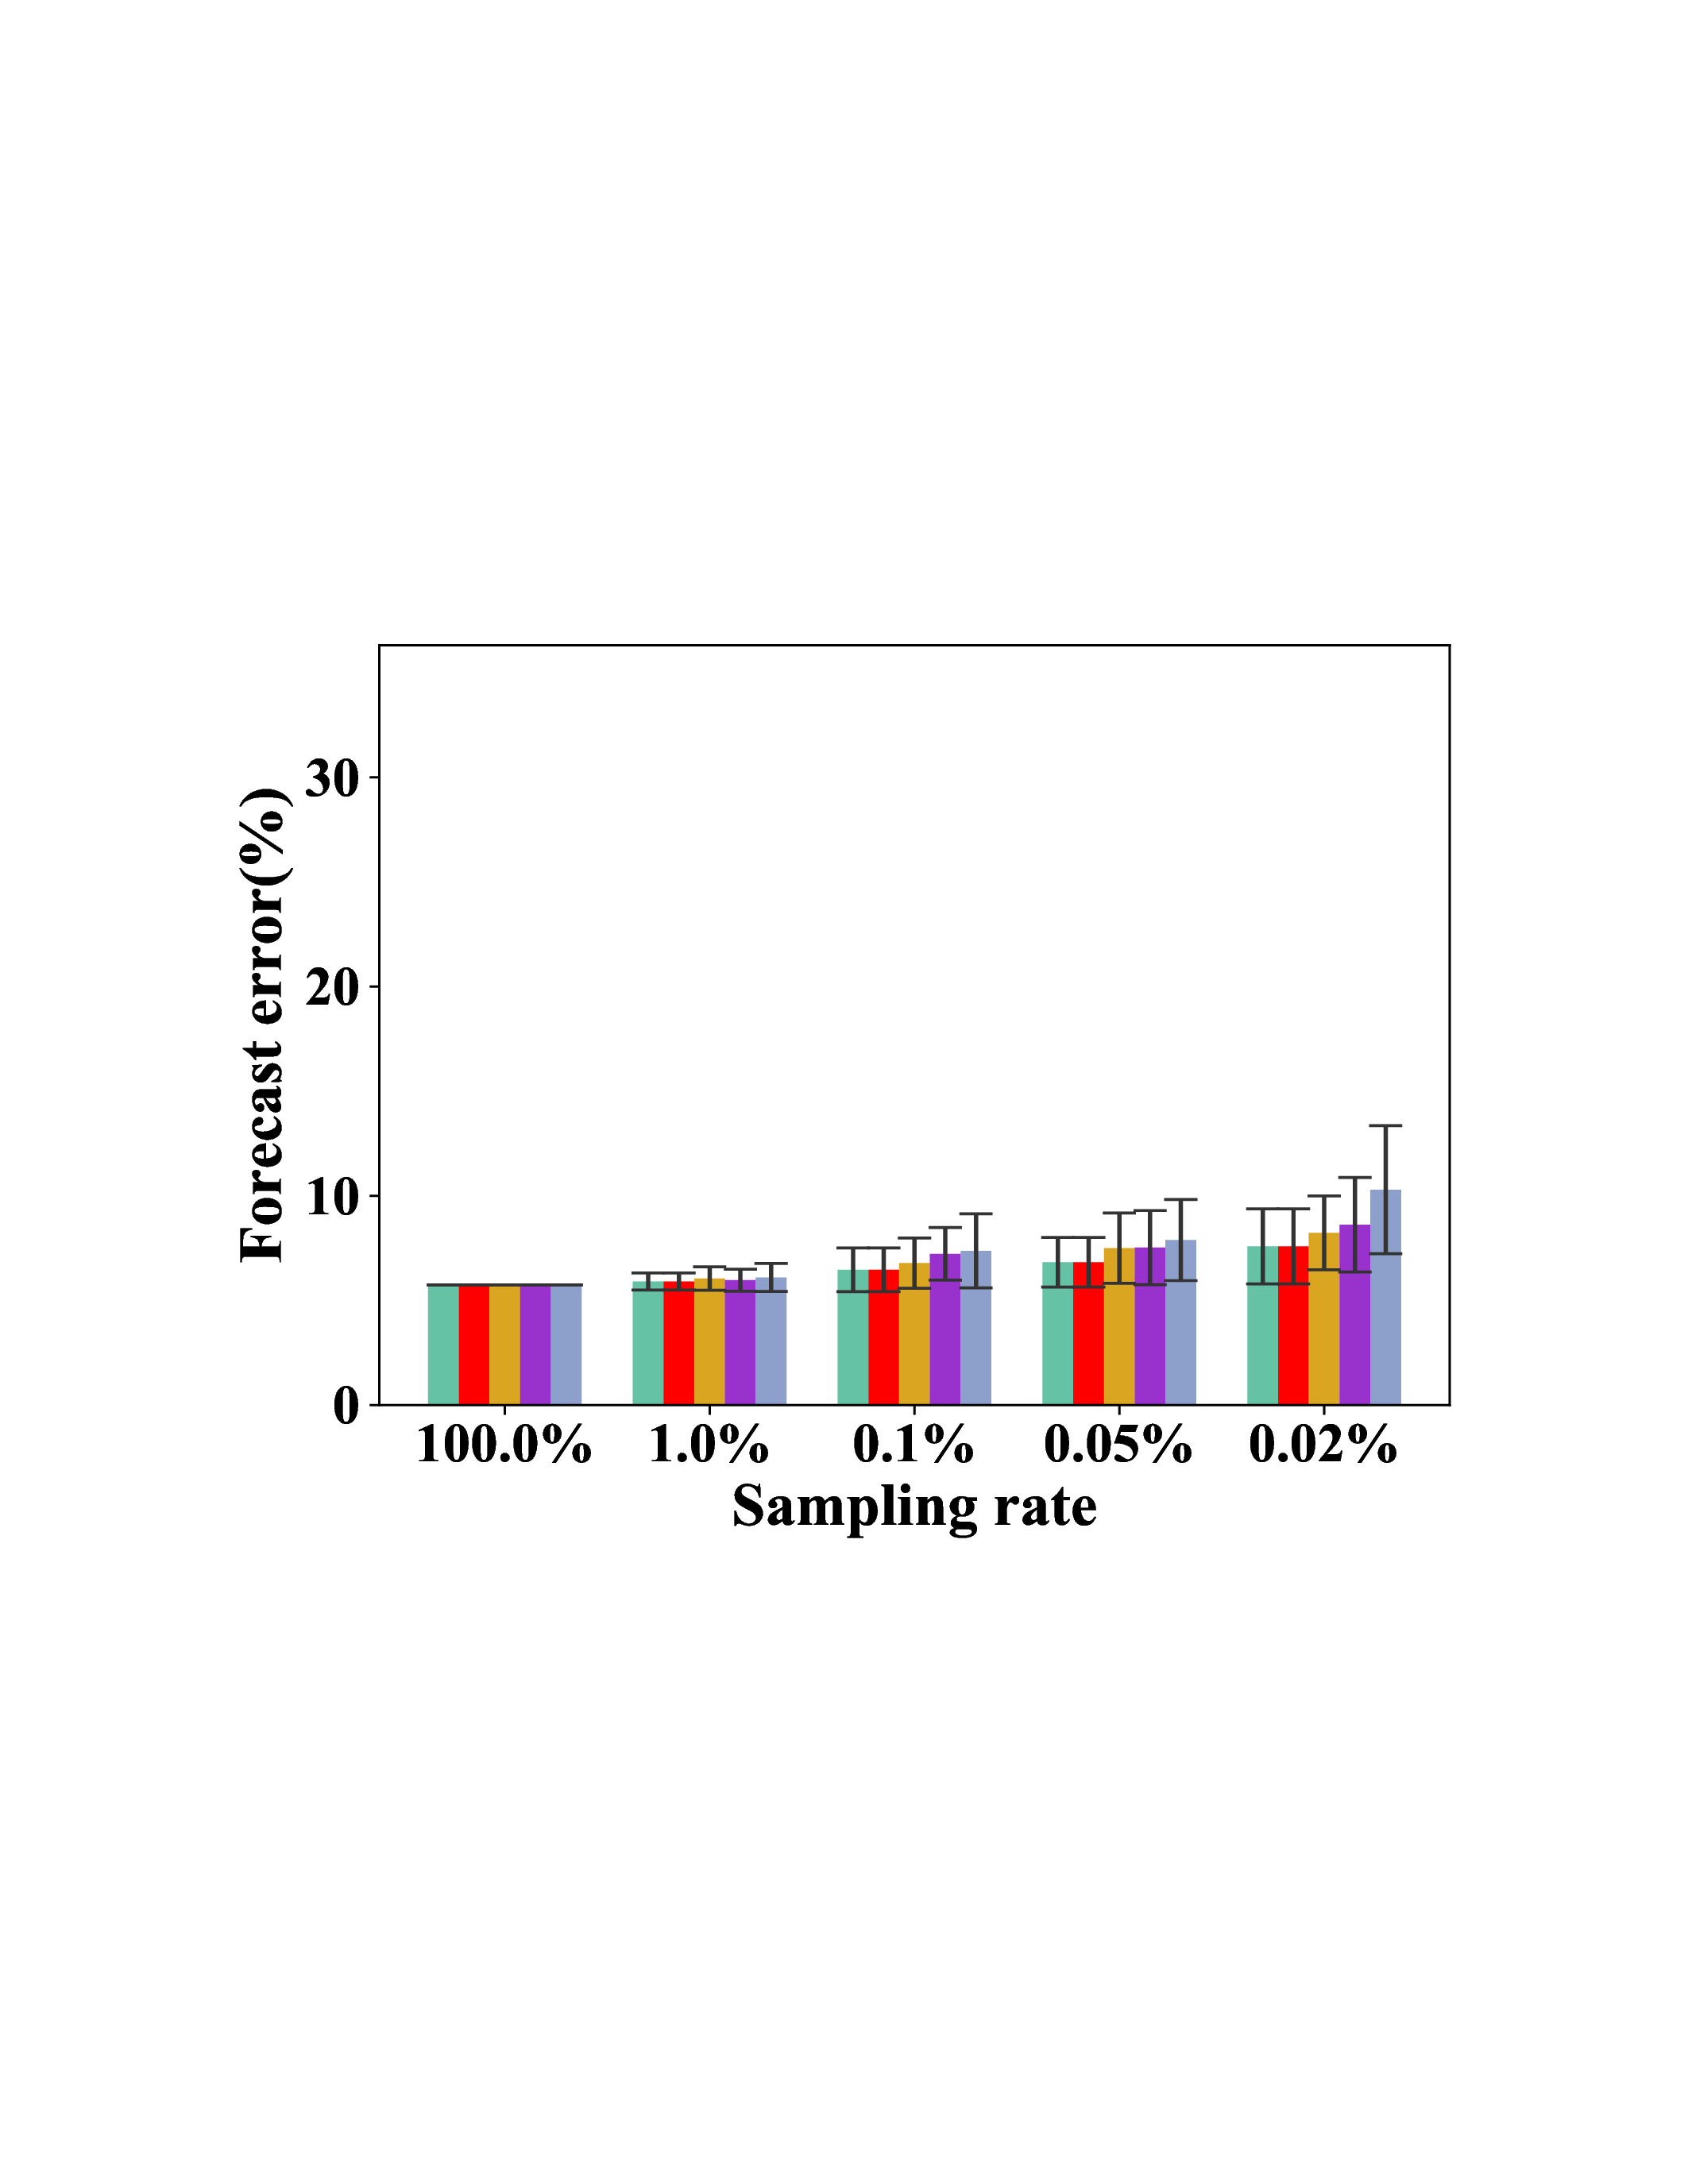}
\end{minipage}
}
\subfigure[Selectivity 5\%]{
\begin{minipage}[t]{0.33\linewidth}
\centering
\includegraphics[width=2.2in, height=2.0in]{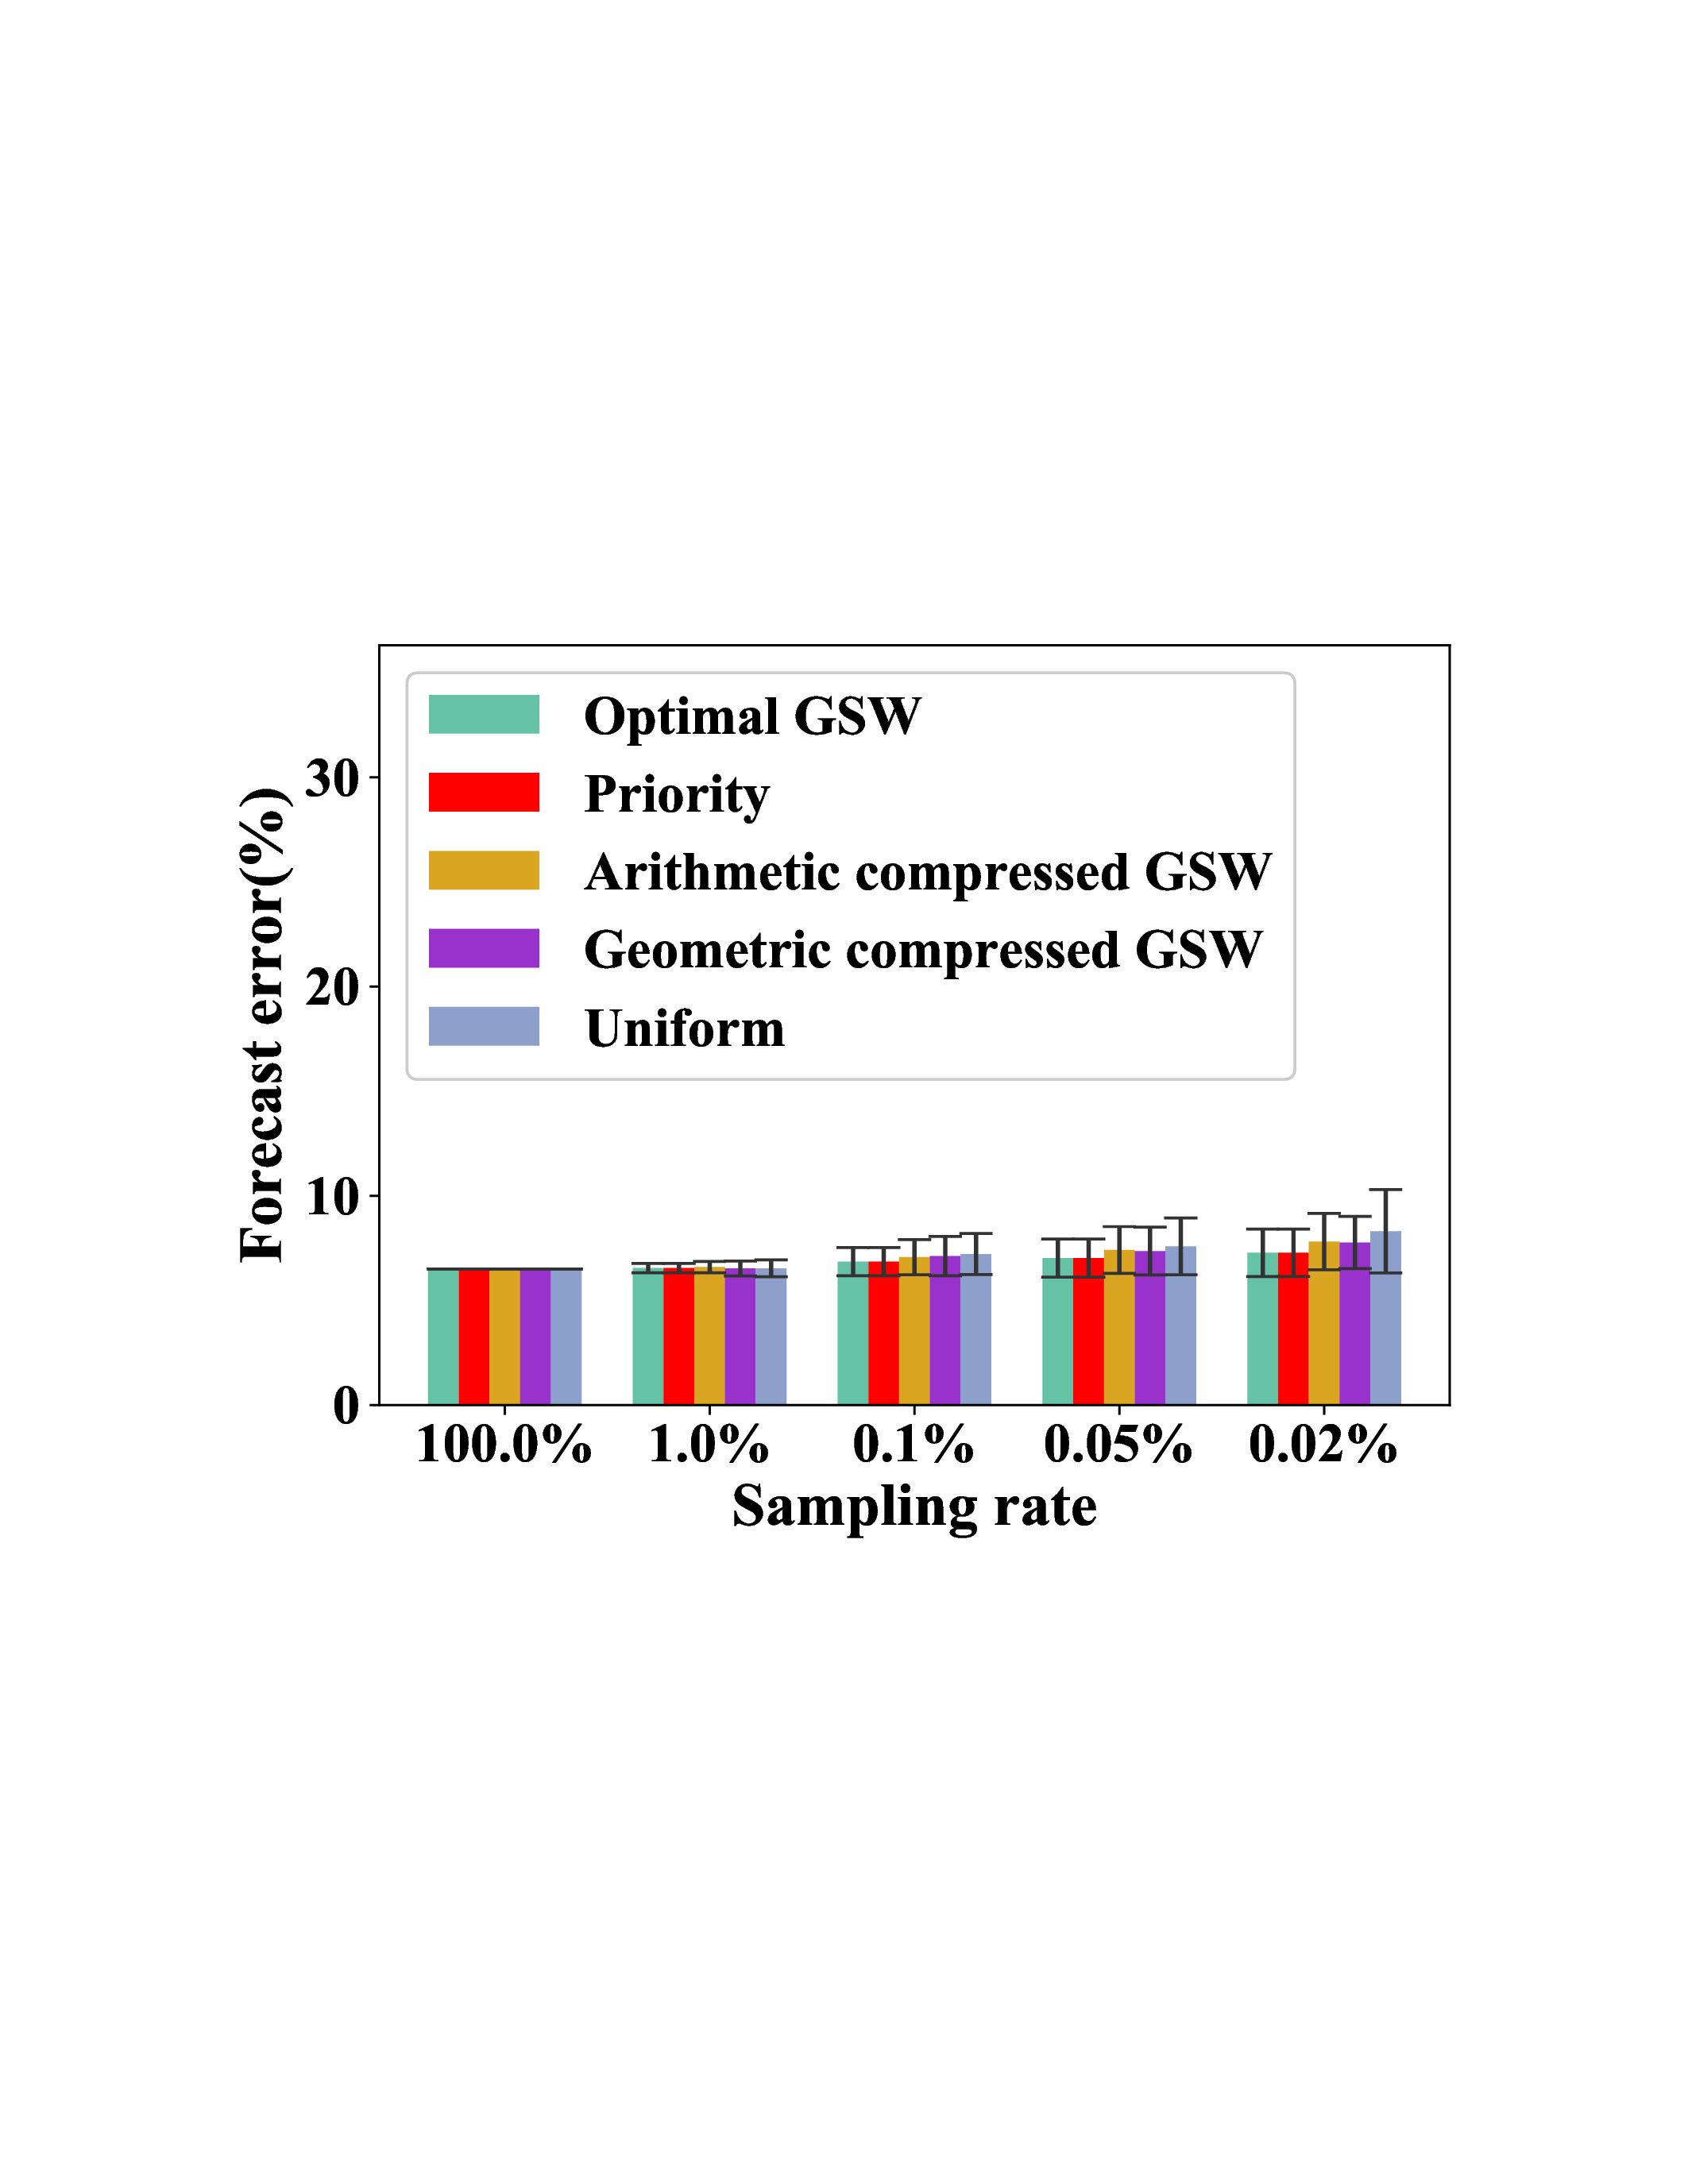}
\end{minipage}
}
\caption{ARIMA prediction error at different selectivity on click via different sampling methods}
% \label{AQP and ARIMA Performance}
\end{figure*}

%-----Click不同抽样方法对ARIMA Interval误差的影响----------
\begin{figure*}[hb]
\subfigure[Selectivity 0.5\%]{
\begin{minipage}[t]{0.33\linewidth}
\centering
\includegraphics[width=2.2in, height=2.0in]{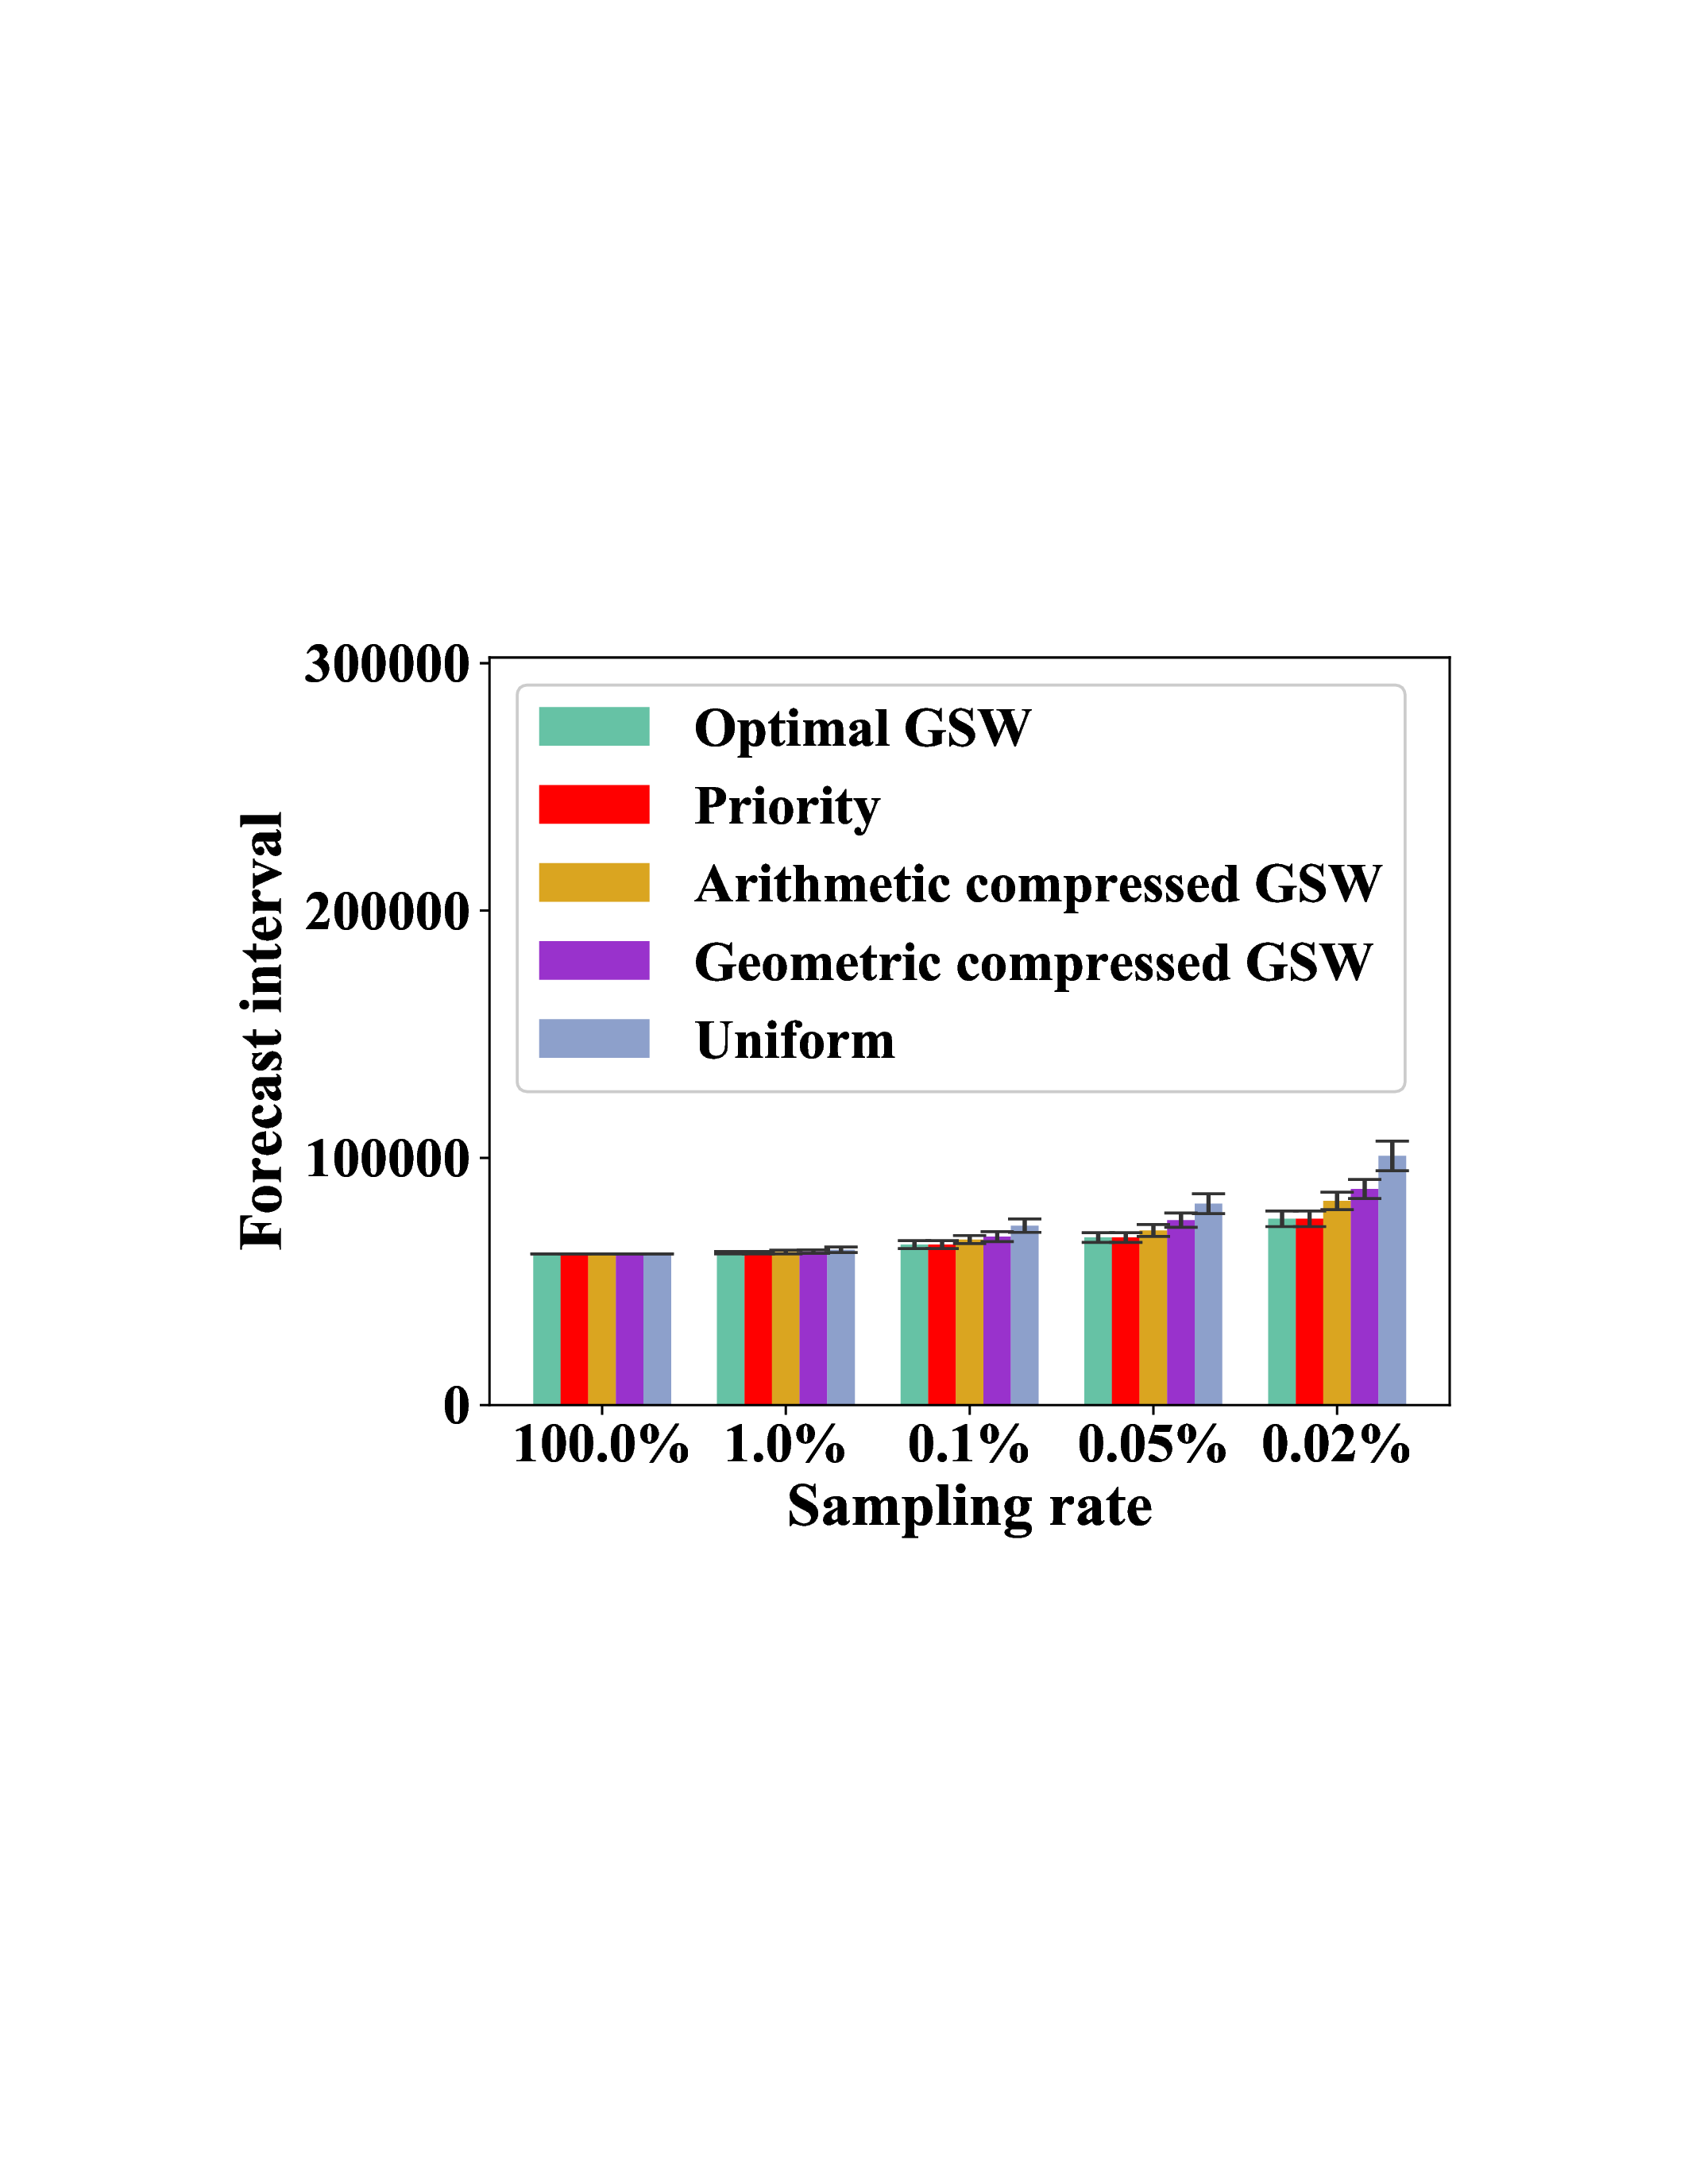}
% \label{fig:side:a}
\end{minipage}
}
\subfigure[Selectivity 1\%]{
\begin{minipage}[t]{0.33\linewidth}
\centering
\includegraphics[width=2.2in, height=2.0in]{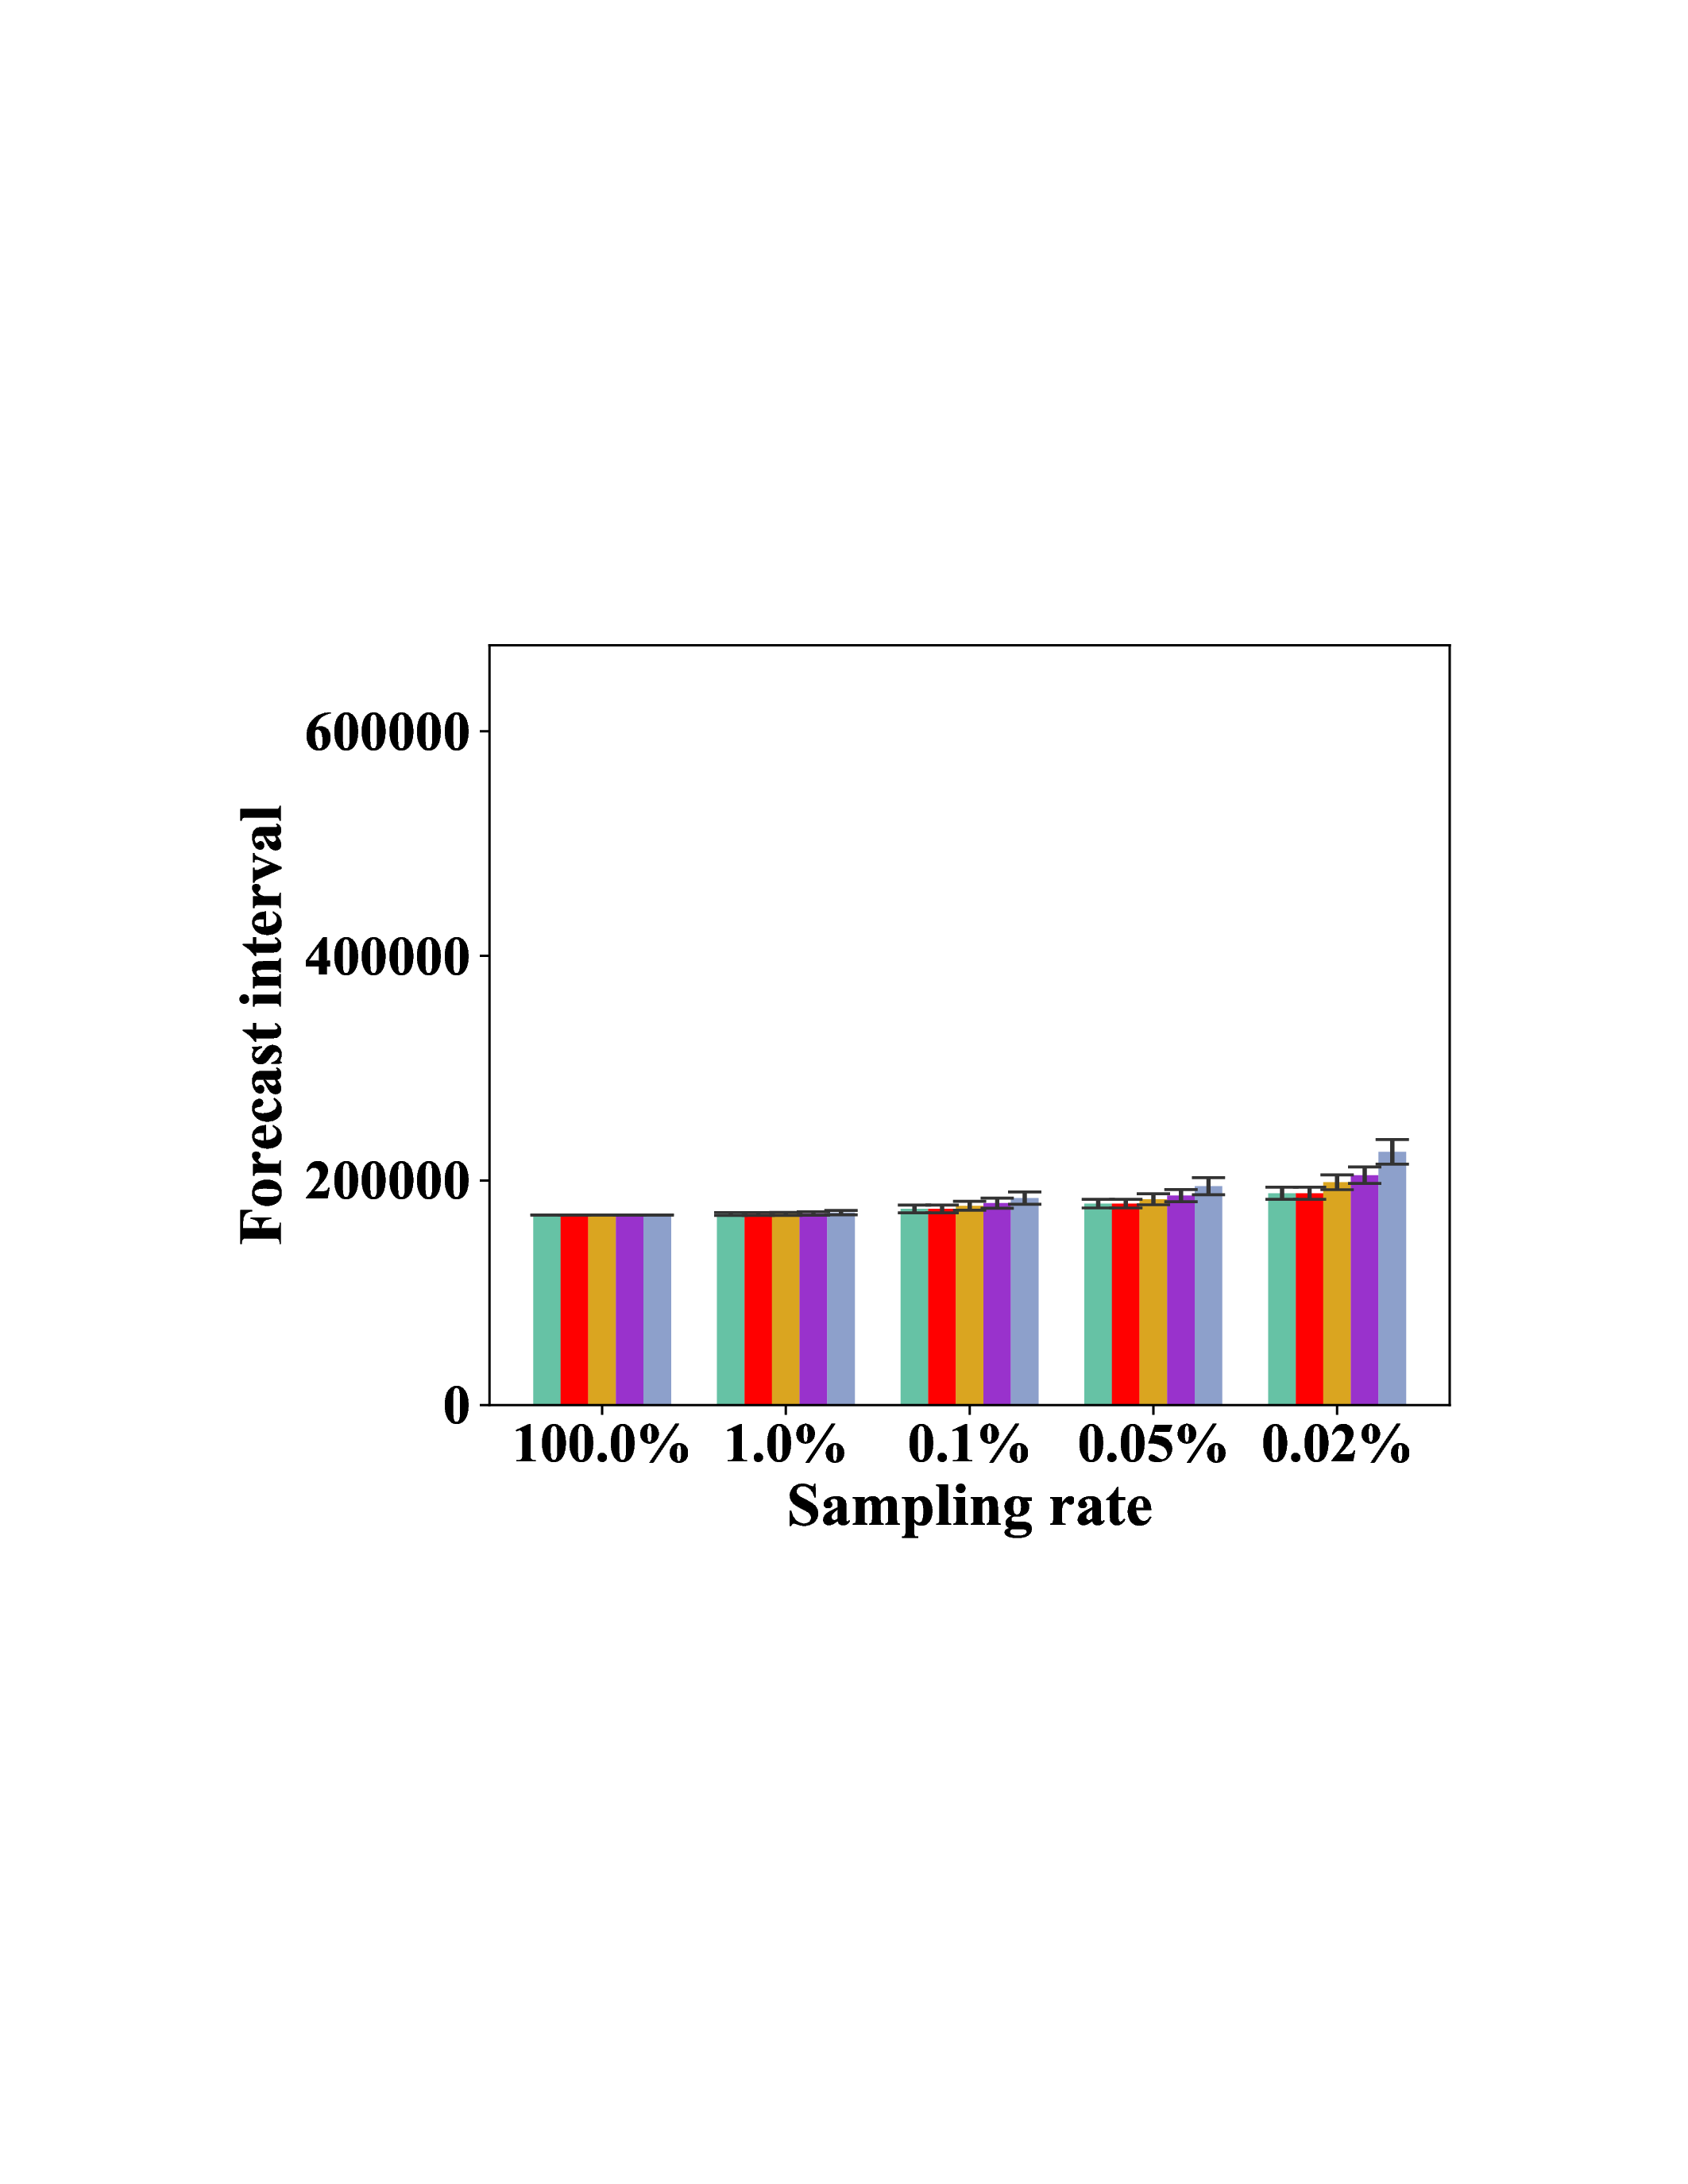}
\end{minipage}
}
\subfigure[Selectivity 5\%]{
\begin{minipage}[t]{0.33\linewidth}
\centering
\includegraphics[width=2.2in, height=2.0in]{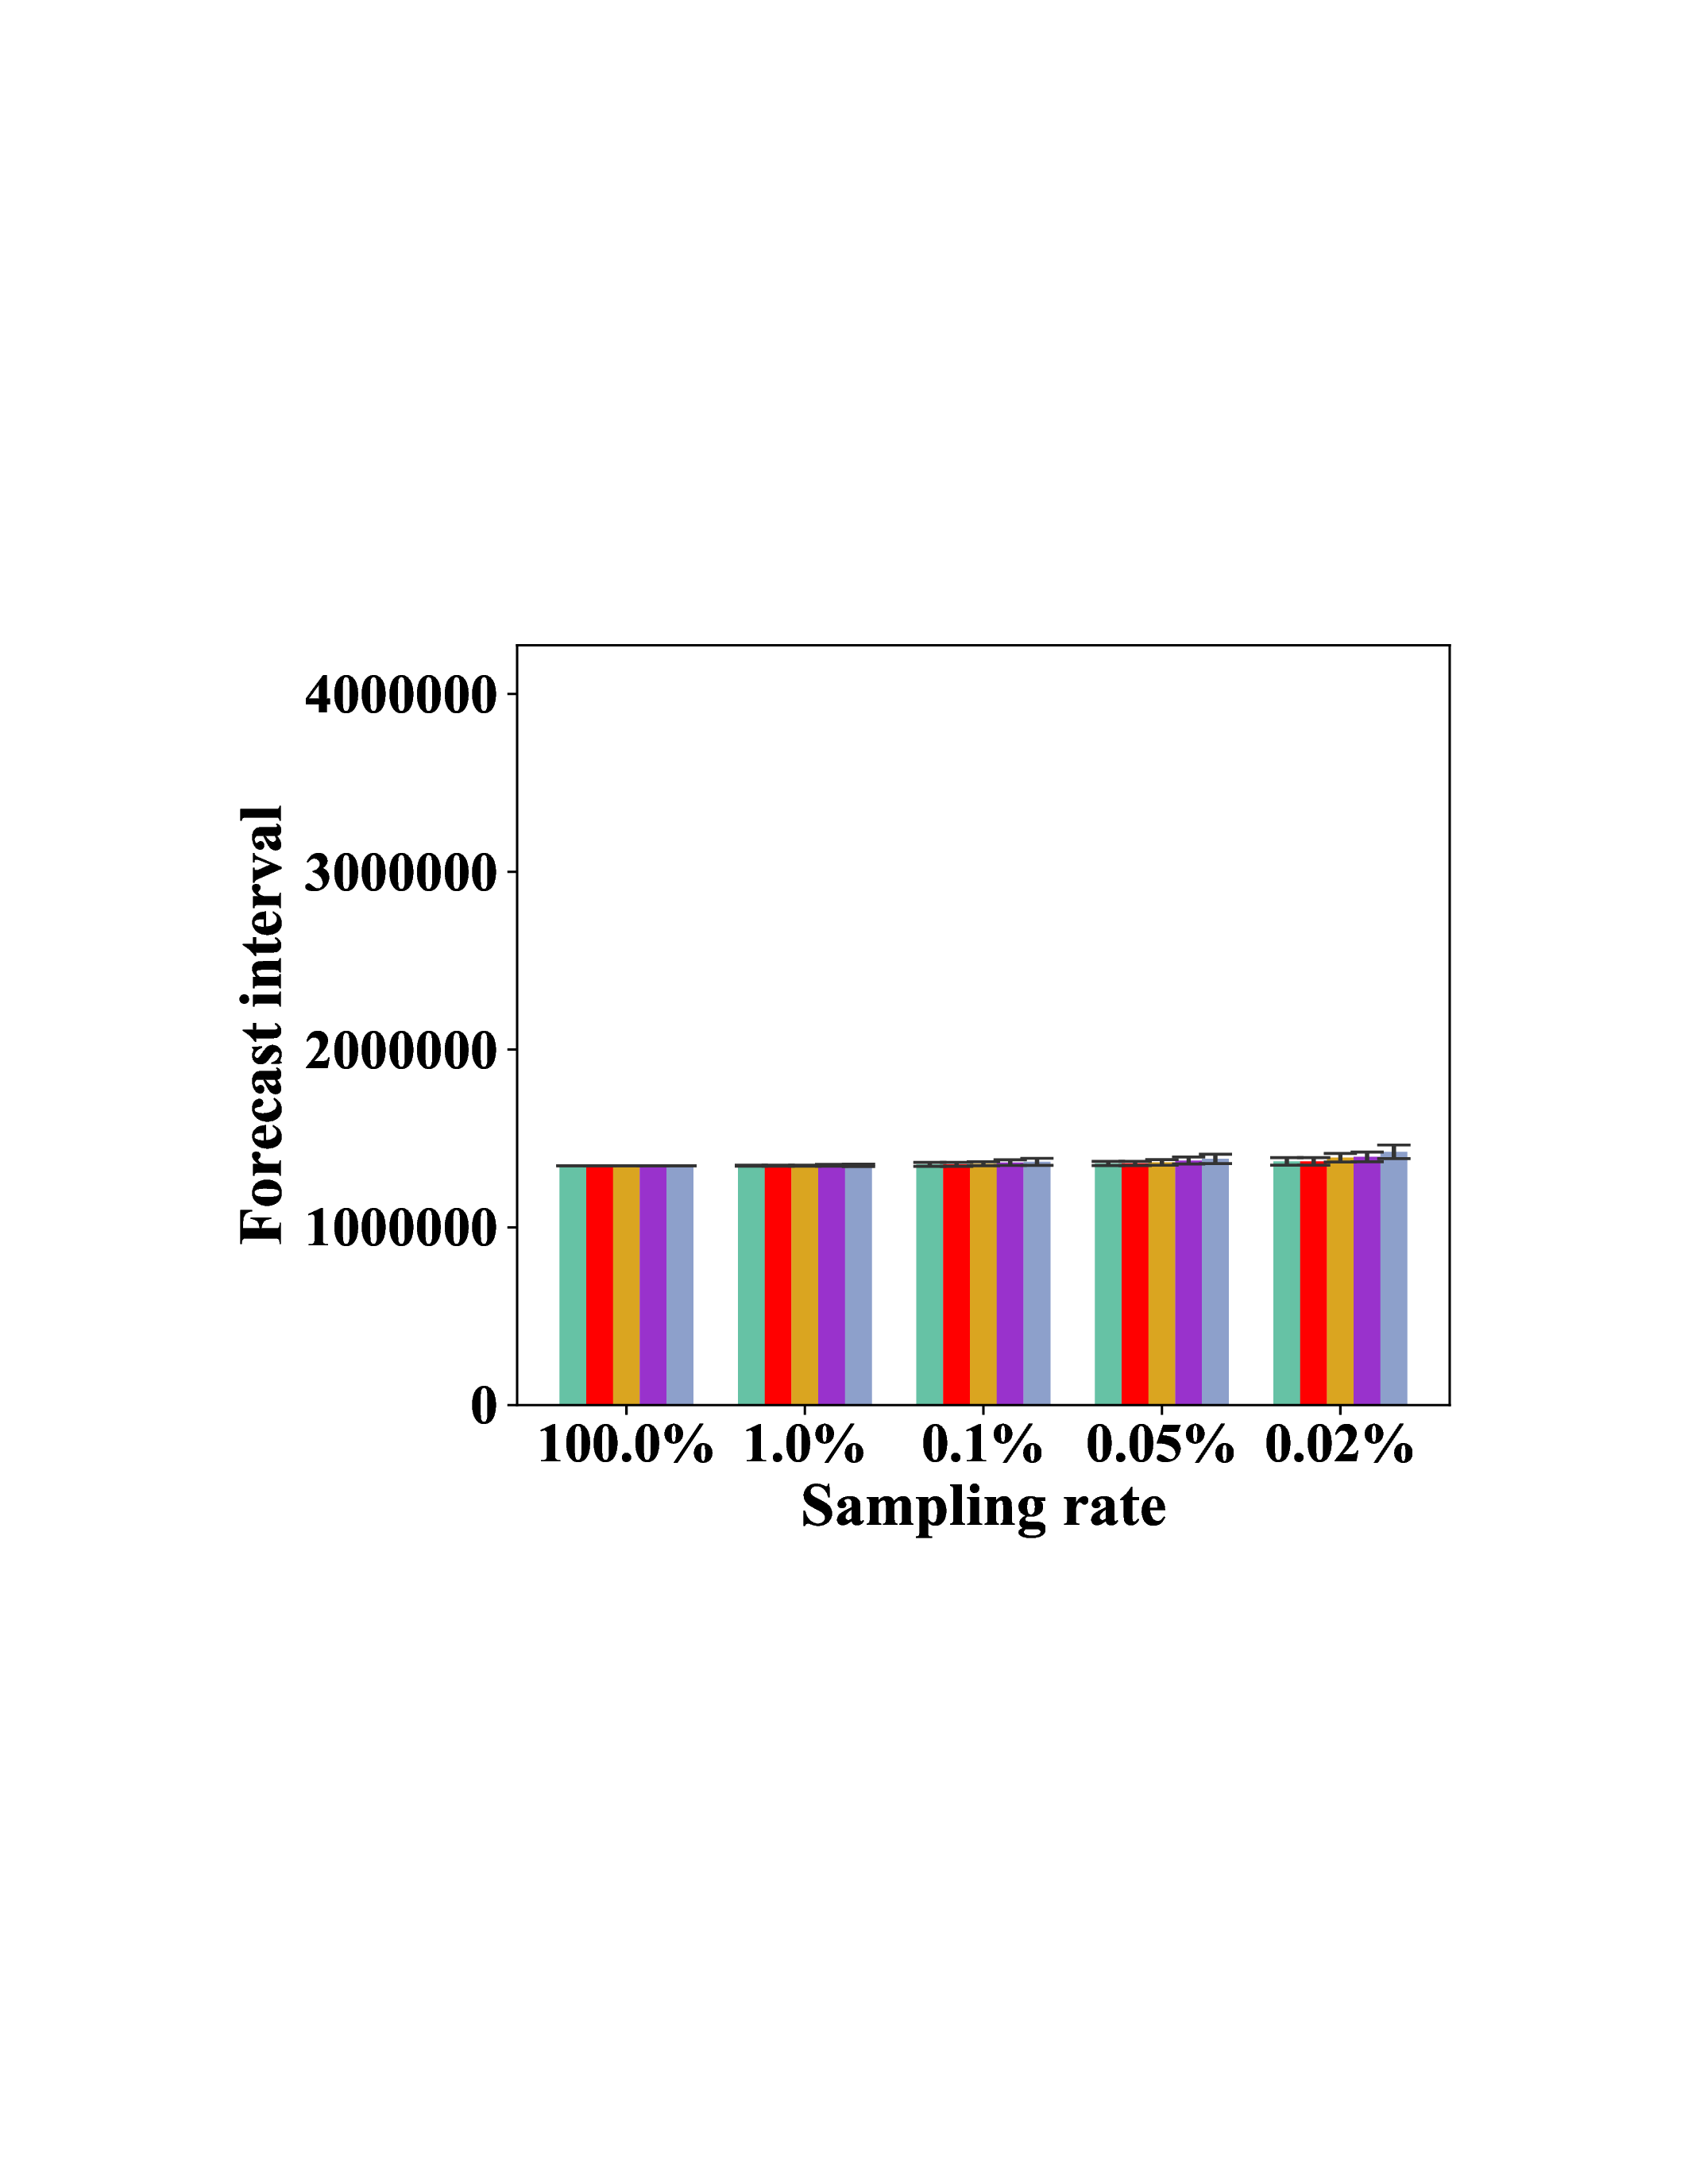}
\end{minipage}
}
\caption{ARIMA prediction interval at different selectivity on click via different sampling methods}
% \label{AQP and ARIMA Performance}
\end{figure*}

%============================

%-----Favorite不同抽样方法对AQP误差的影响----------
\begin{figure*}[hb]
\subfigure[Selectivity 0.5\%]{
\begin{minipage}[t]{0.33\linewidth}
\centering
\includegraphics[width=2.2in, height=2.0in]{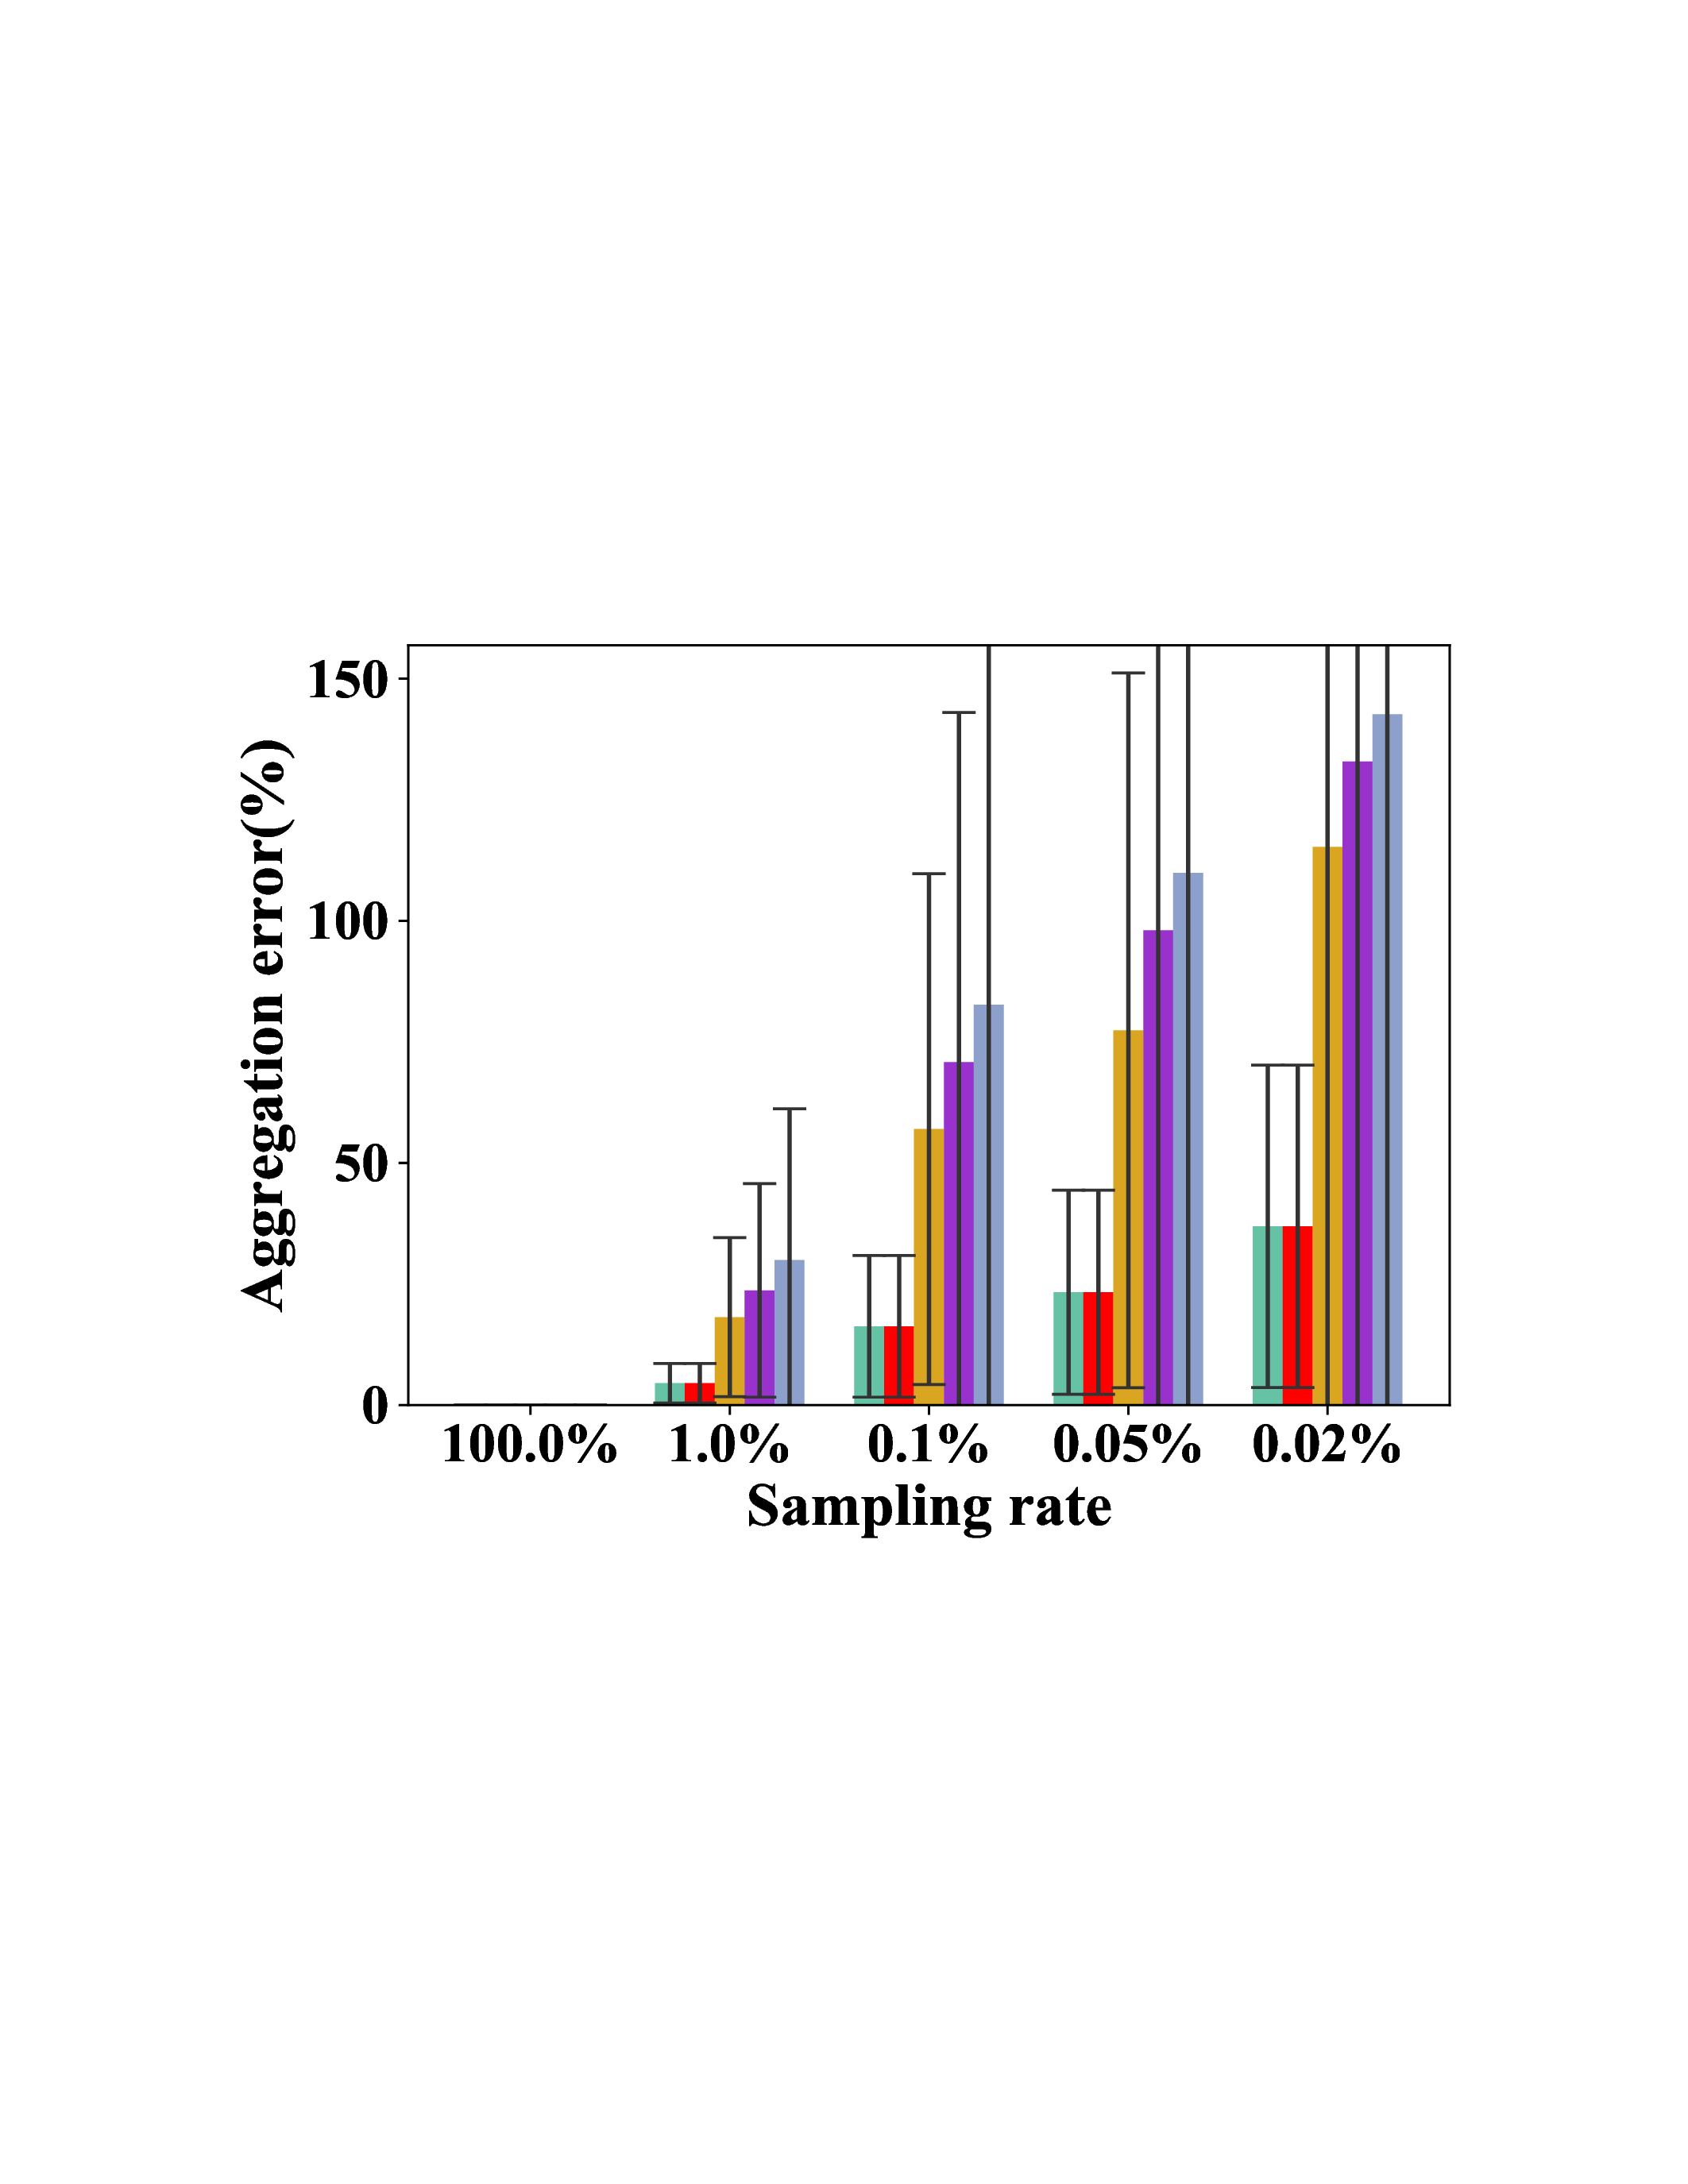}
% \label{fig:side:a}
\end{minipage}
}
\subfigure[Selectivity 1\%]{
\begin{minipage}[t]{0.33\linewidth}
\centering
\includegraphics[width=2.2in, height=2.0in]{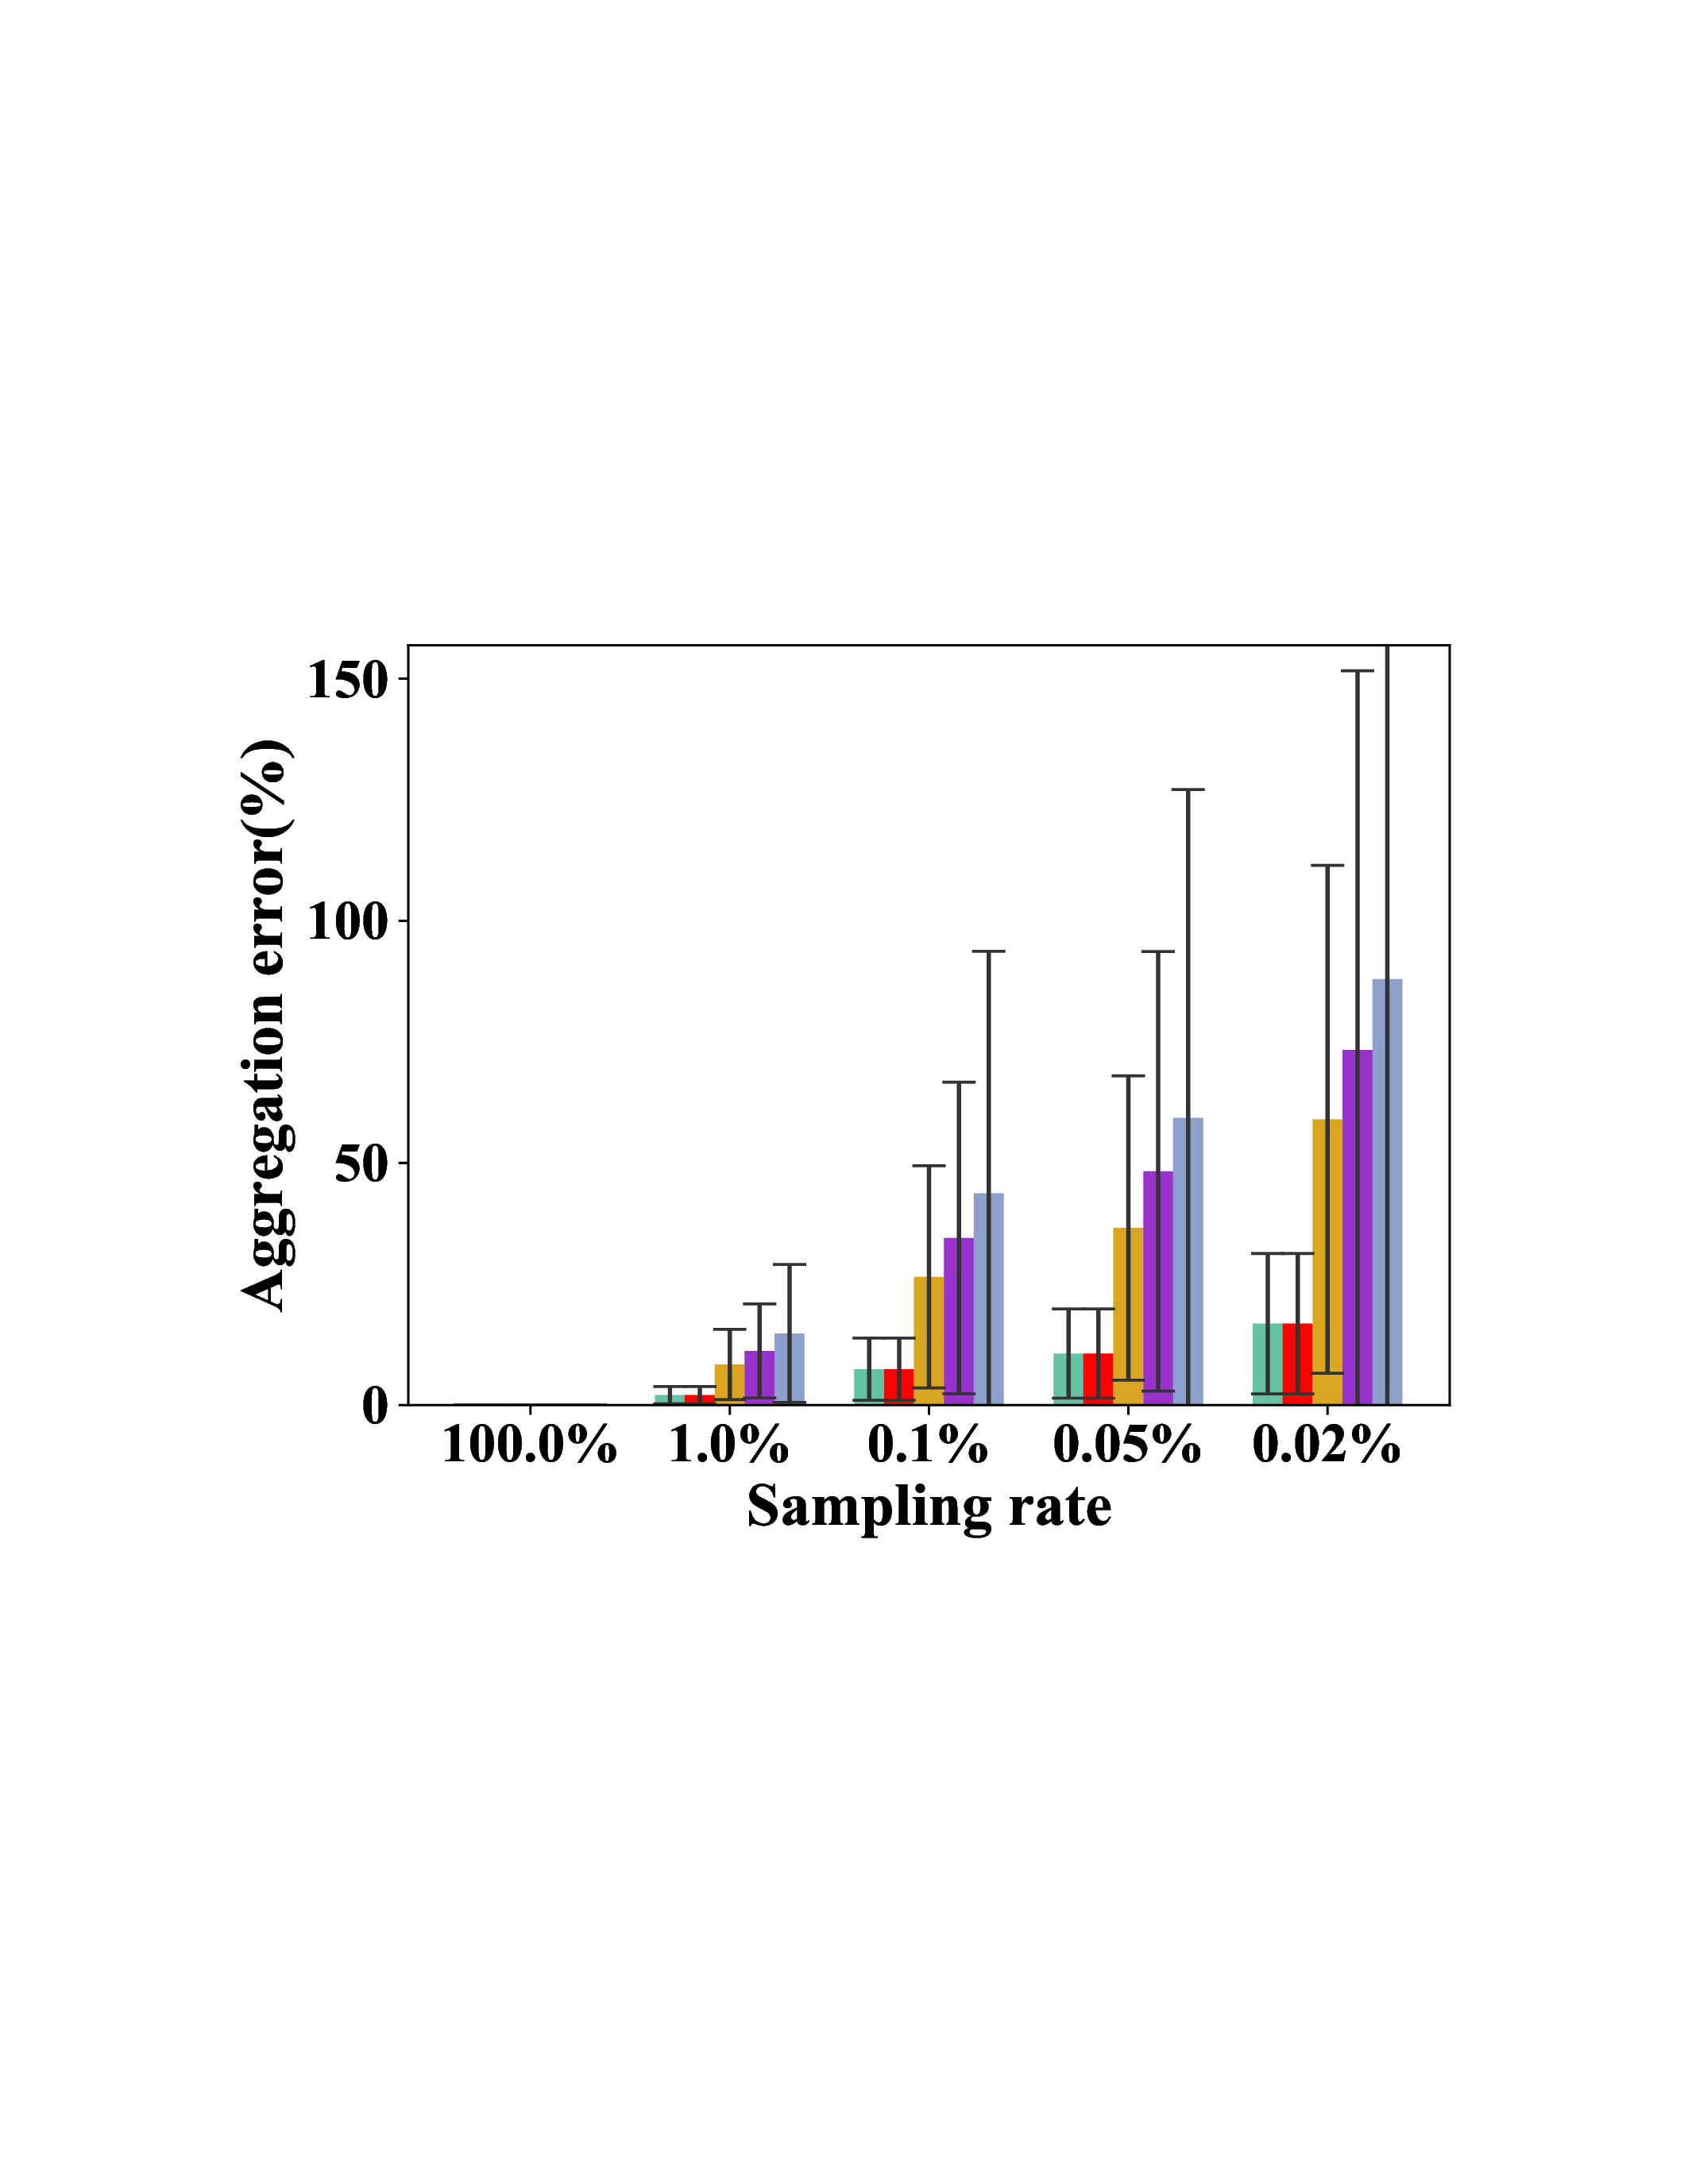}
\end{minipage}
}
\subfigure[Selectivity 5\%]{
\begin{minipage}[t]{0.33\linewidth}
\centering
\includegraphics[width=2.2in, height=2.0in]{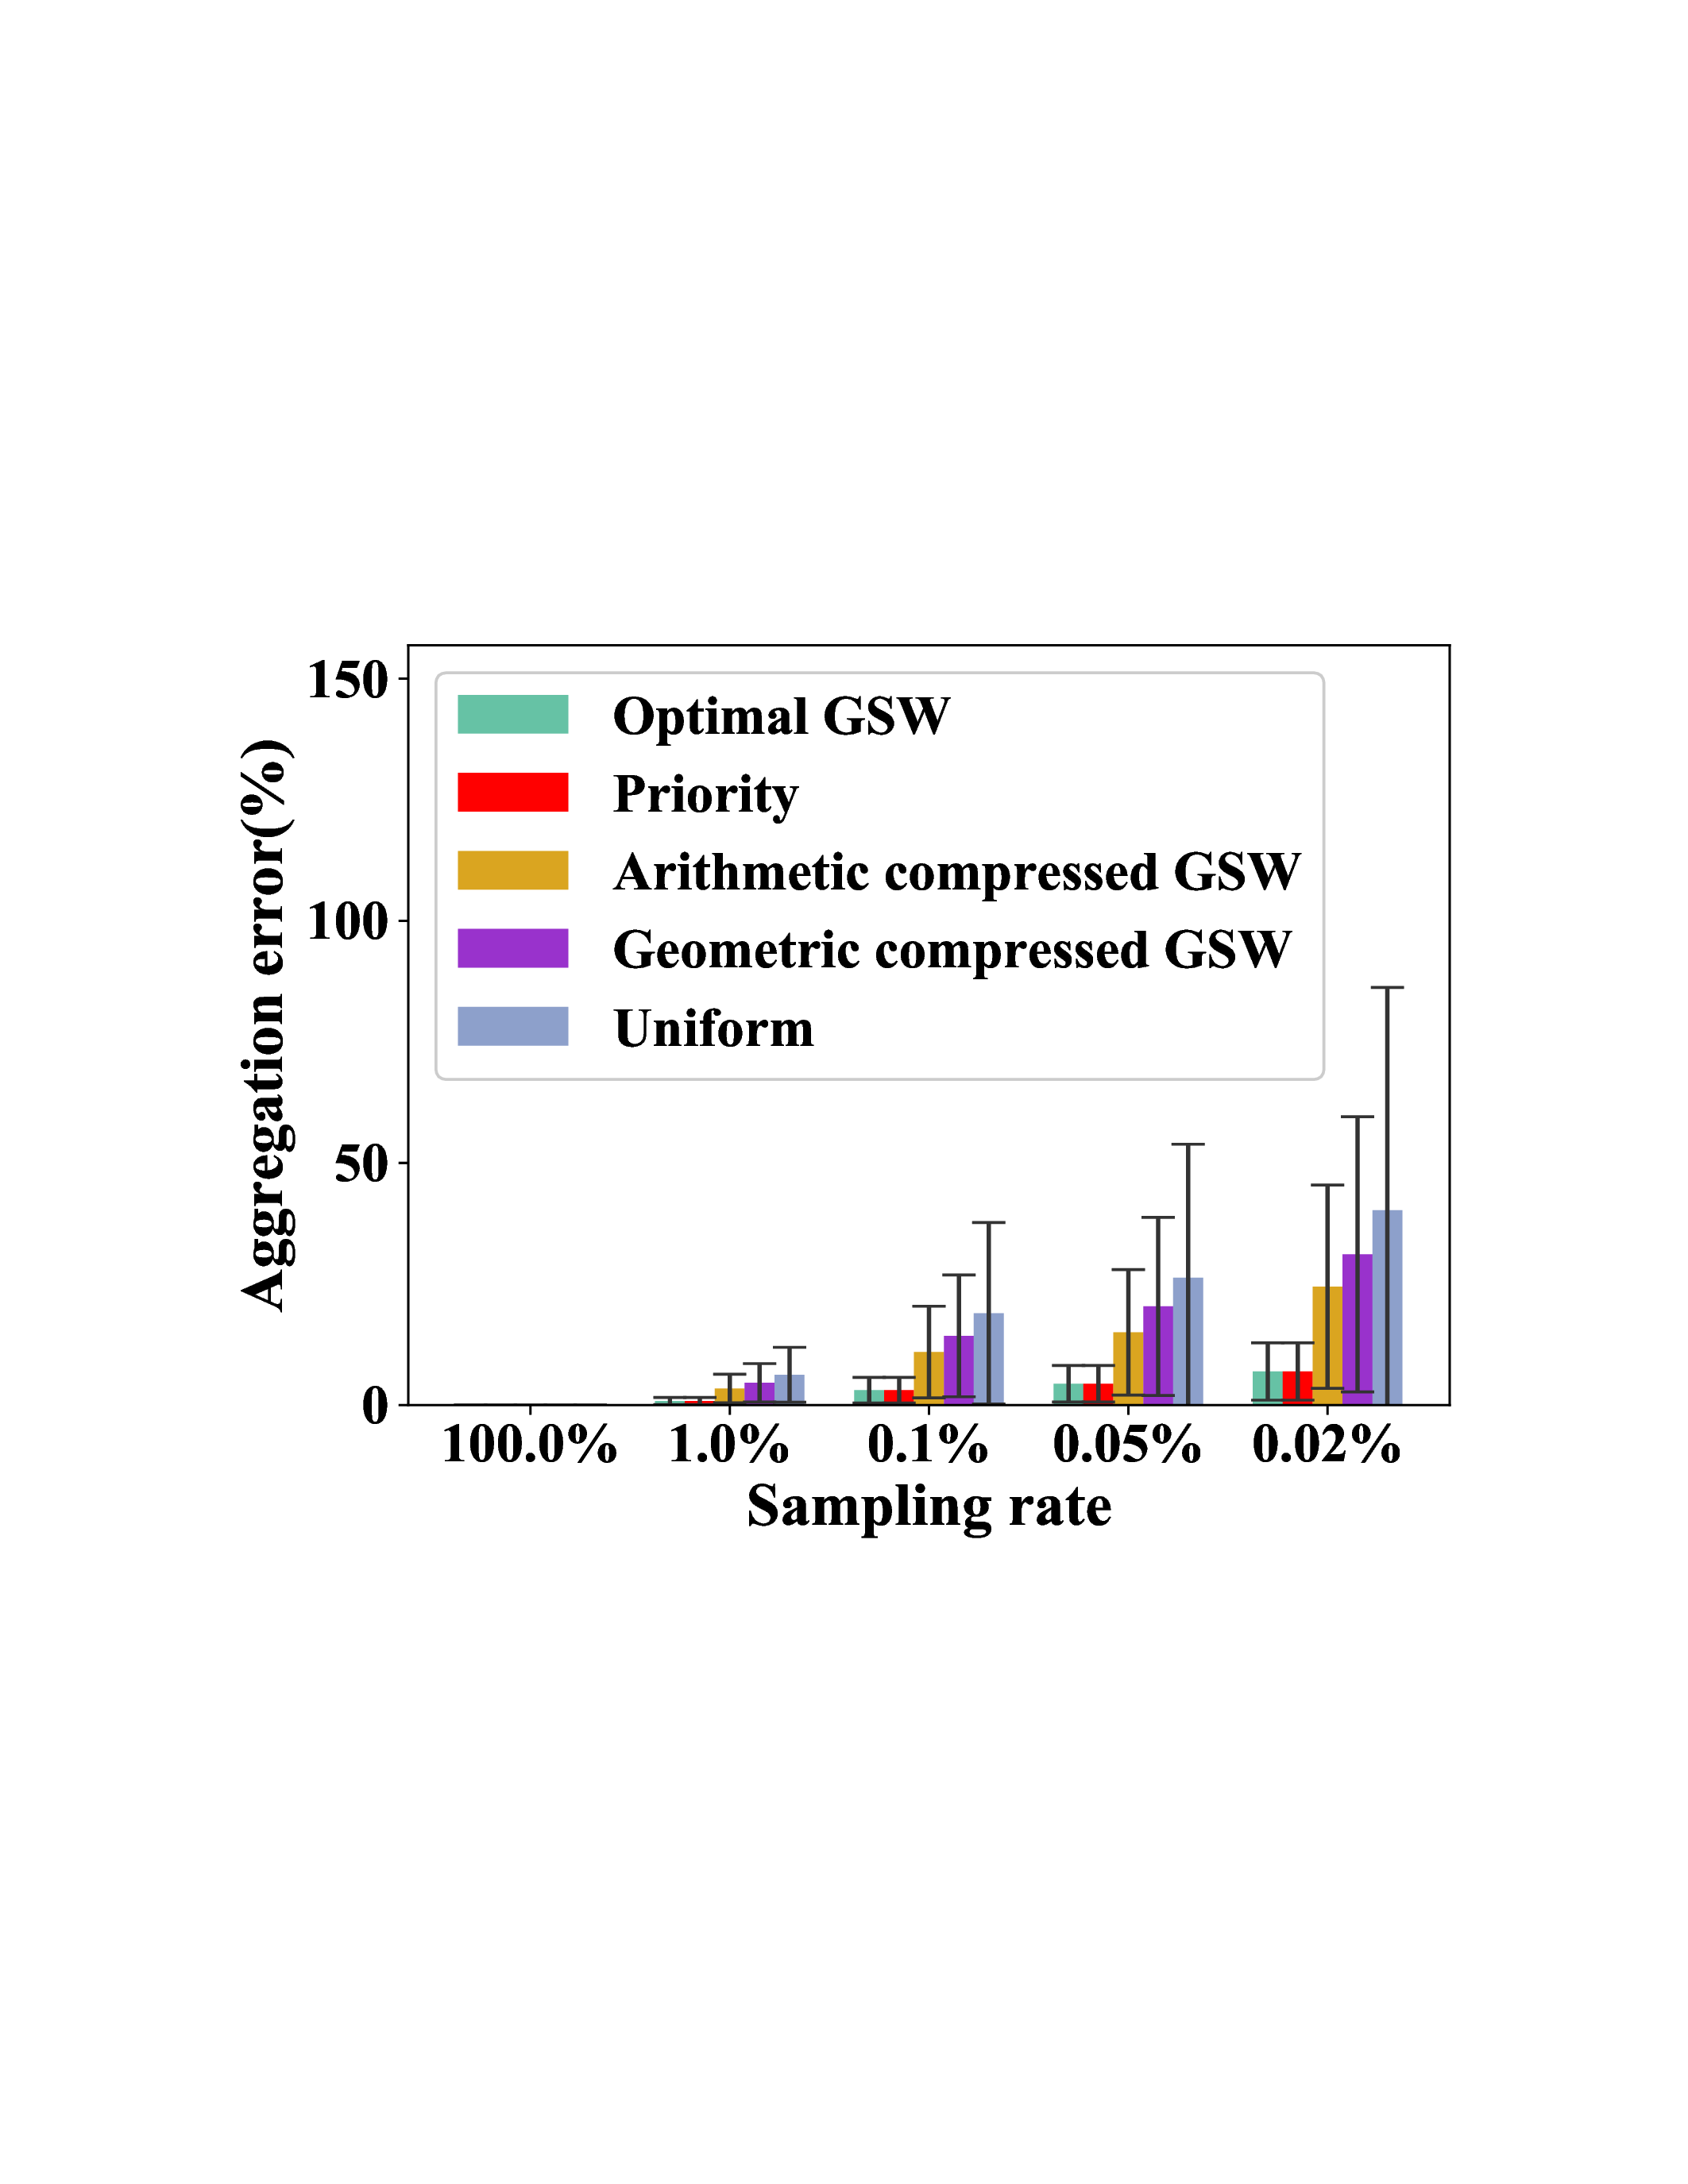}
\end{minipage}
}
\caption{AQP error at different selectivity on favorite via different sampling methods}
% \label{AQP and ARIMA Performance}
\end{figure*}

%-----Favorite不同抽样方法对ARIMA误差的影响----------
\begin{figure*}[hb]
\subfigure[Selectivity 0.5\%]{
\begin{minipage}[t]{0.33\linewidth}
\centering
\includegraphics[width=2.2in, height=2.0in]{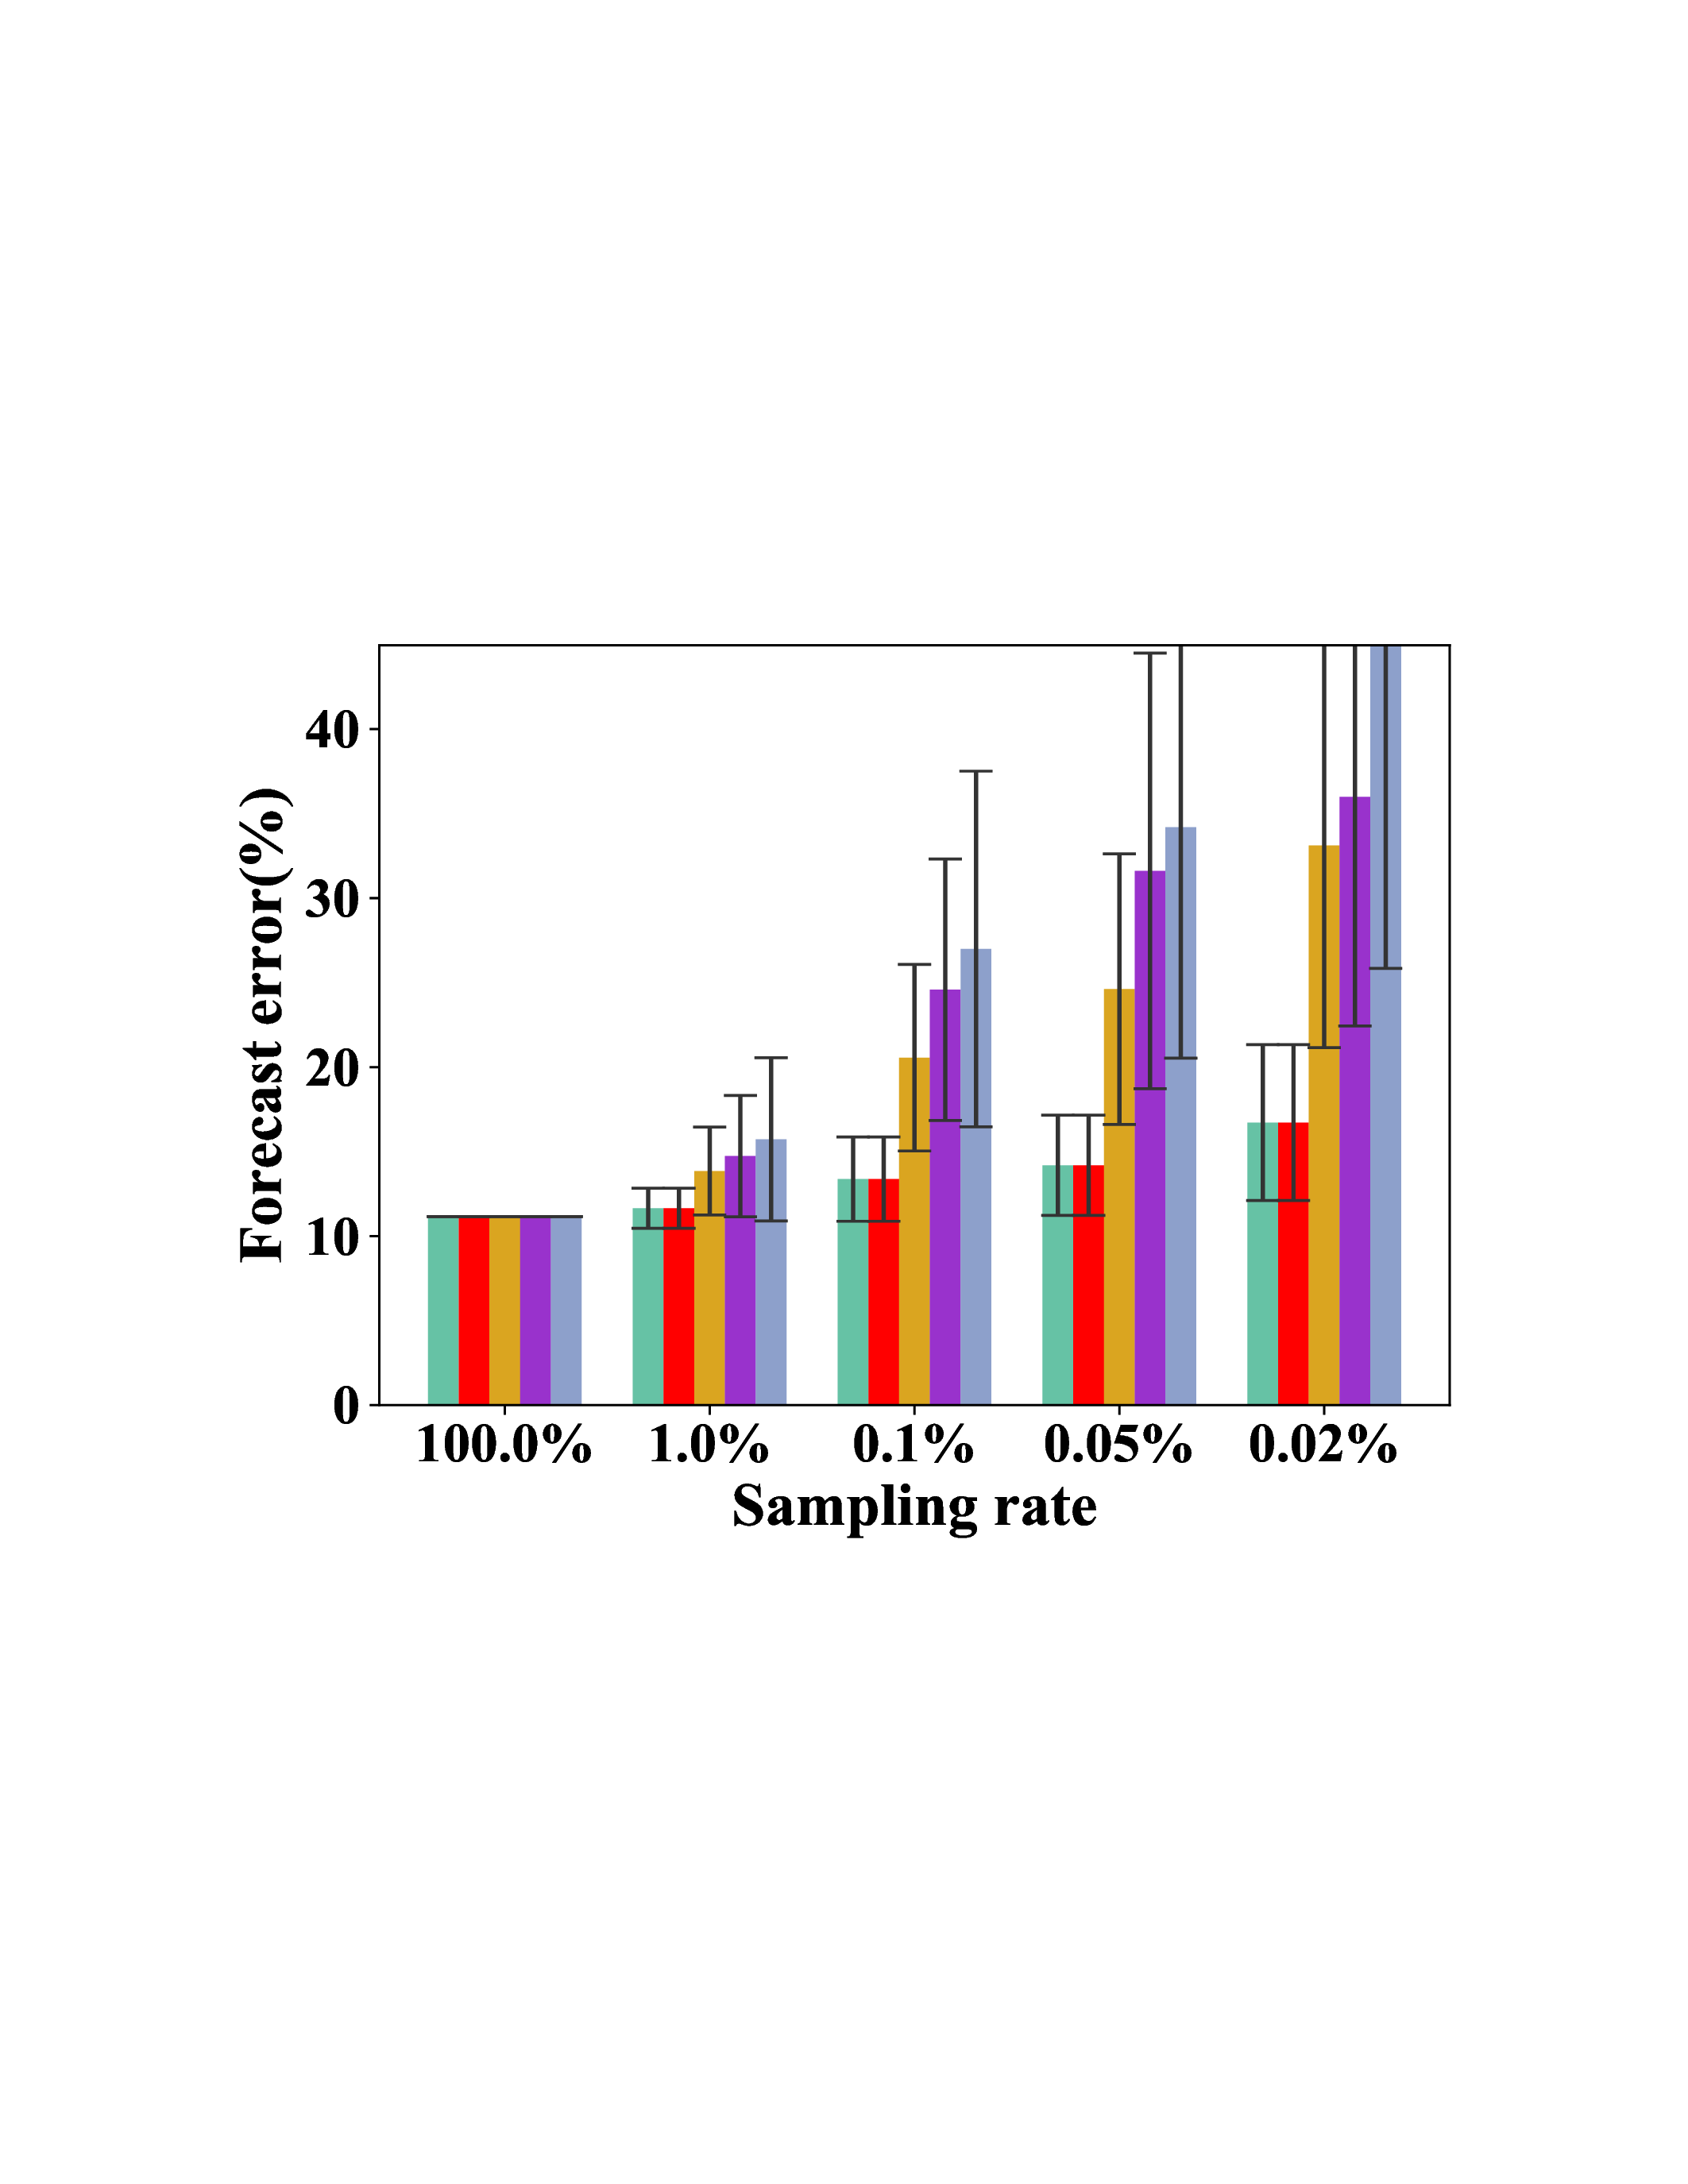}
% \label{fig:side:a}
\end{minipage}
}
\subfigure[Selectivity 1\%]{
\begin{minipage}[t]{0.33\linewidth}
\centering
\includegraphics[width=2.2in, height=2.0in]{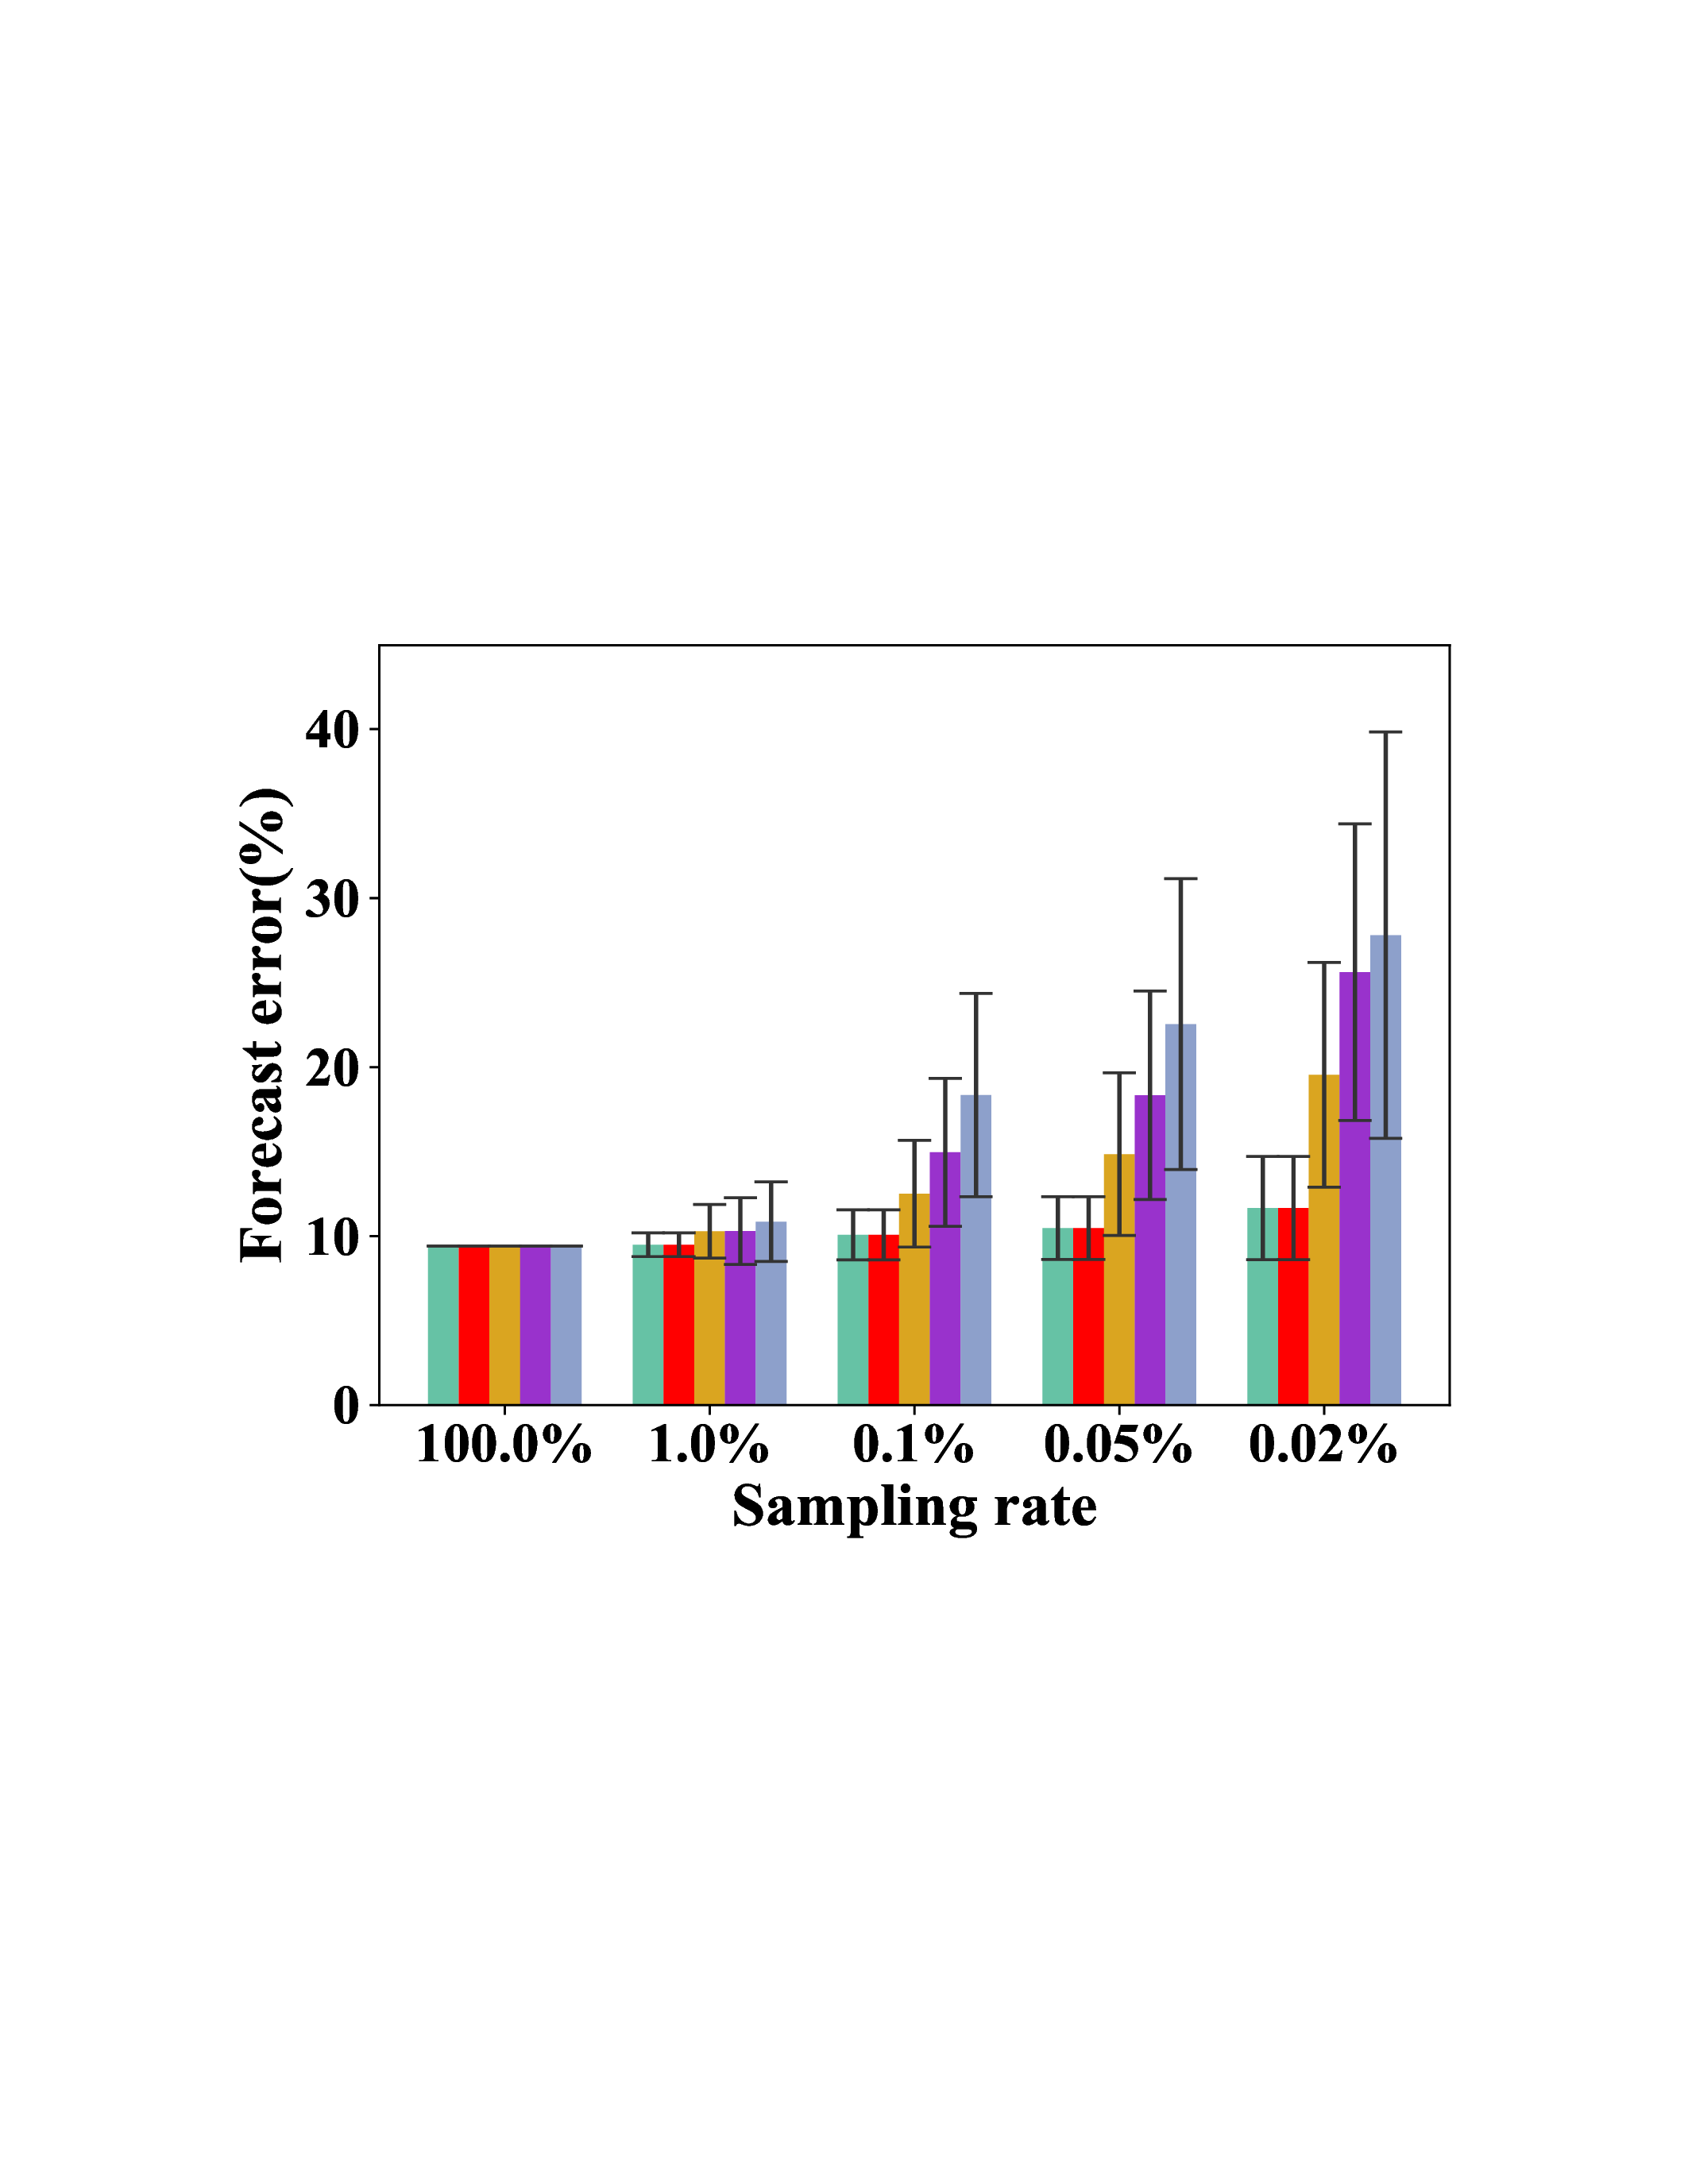}
\end{minipage}
}
\subfigure[Selectivity 5\%]{
\begin{minipage}[t]{0.33\linewidth}
\centering
\includegraphics[width=2.2in, height=2.0in]{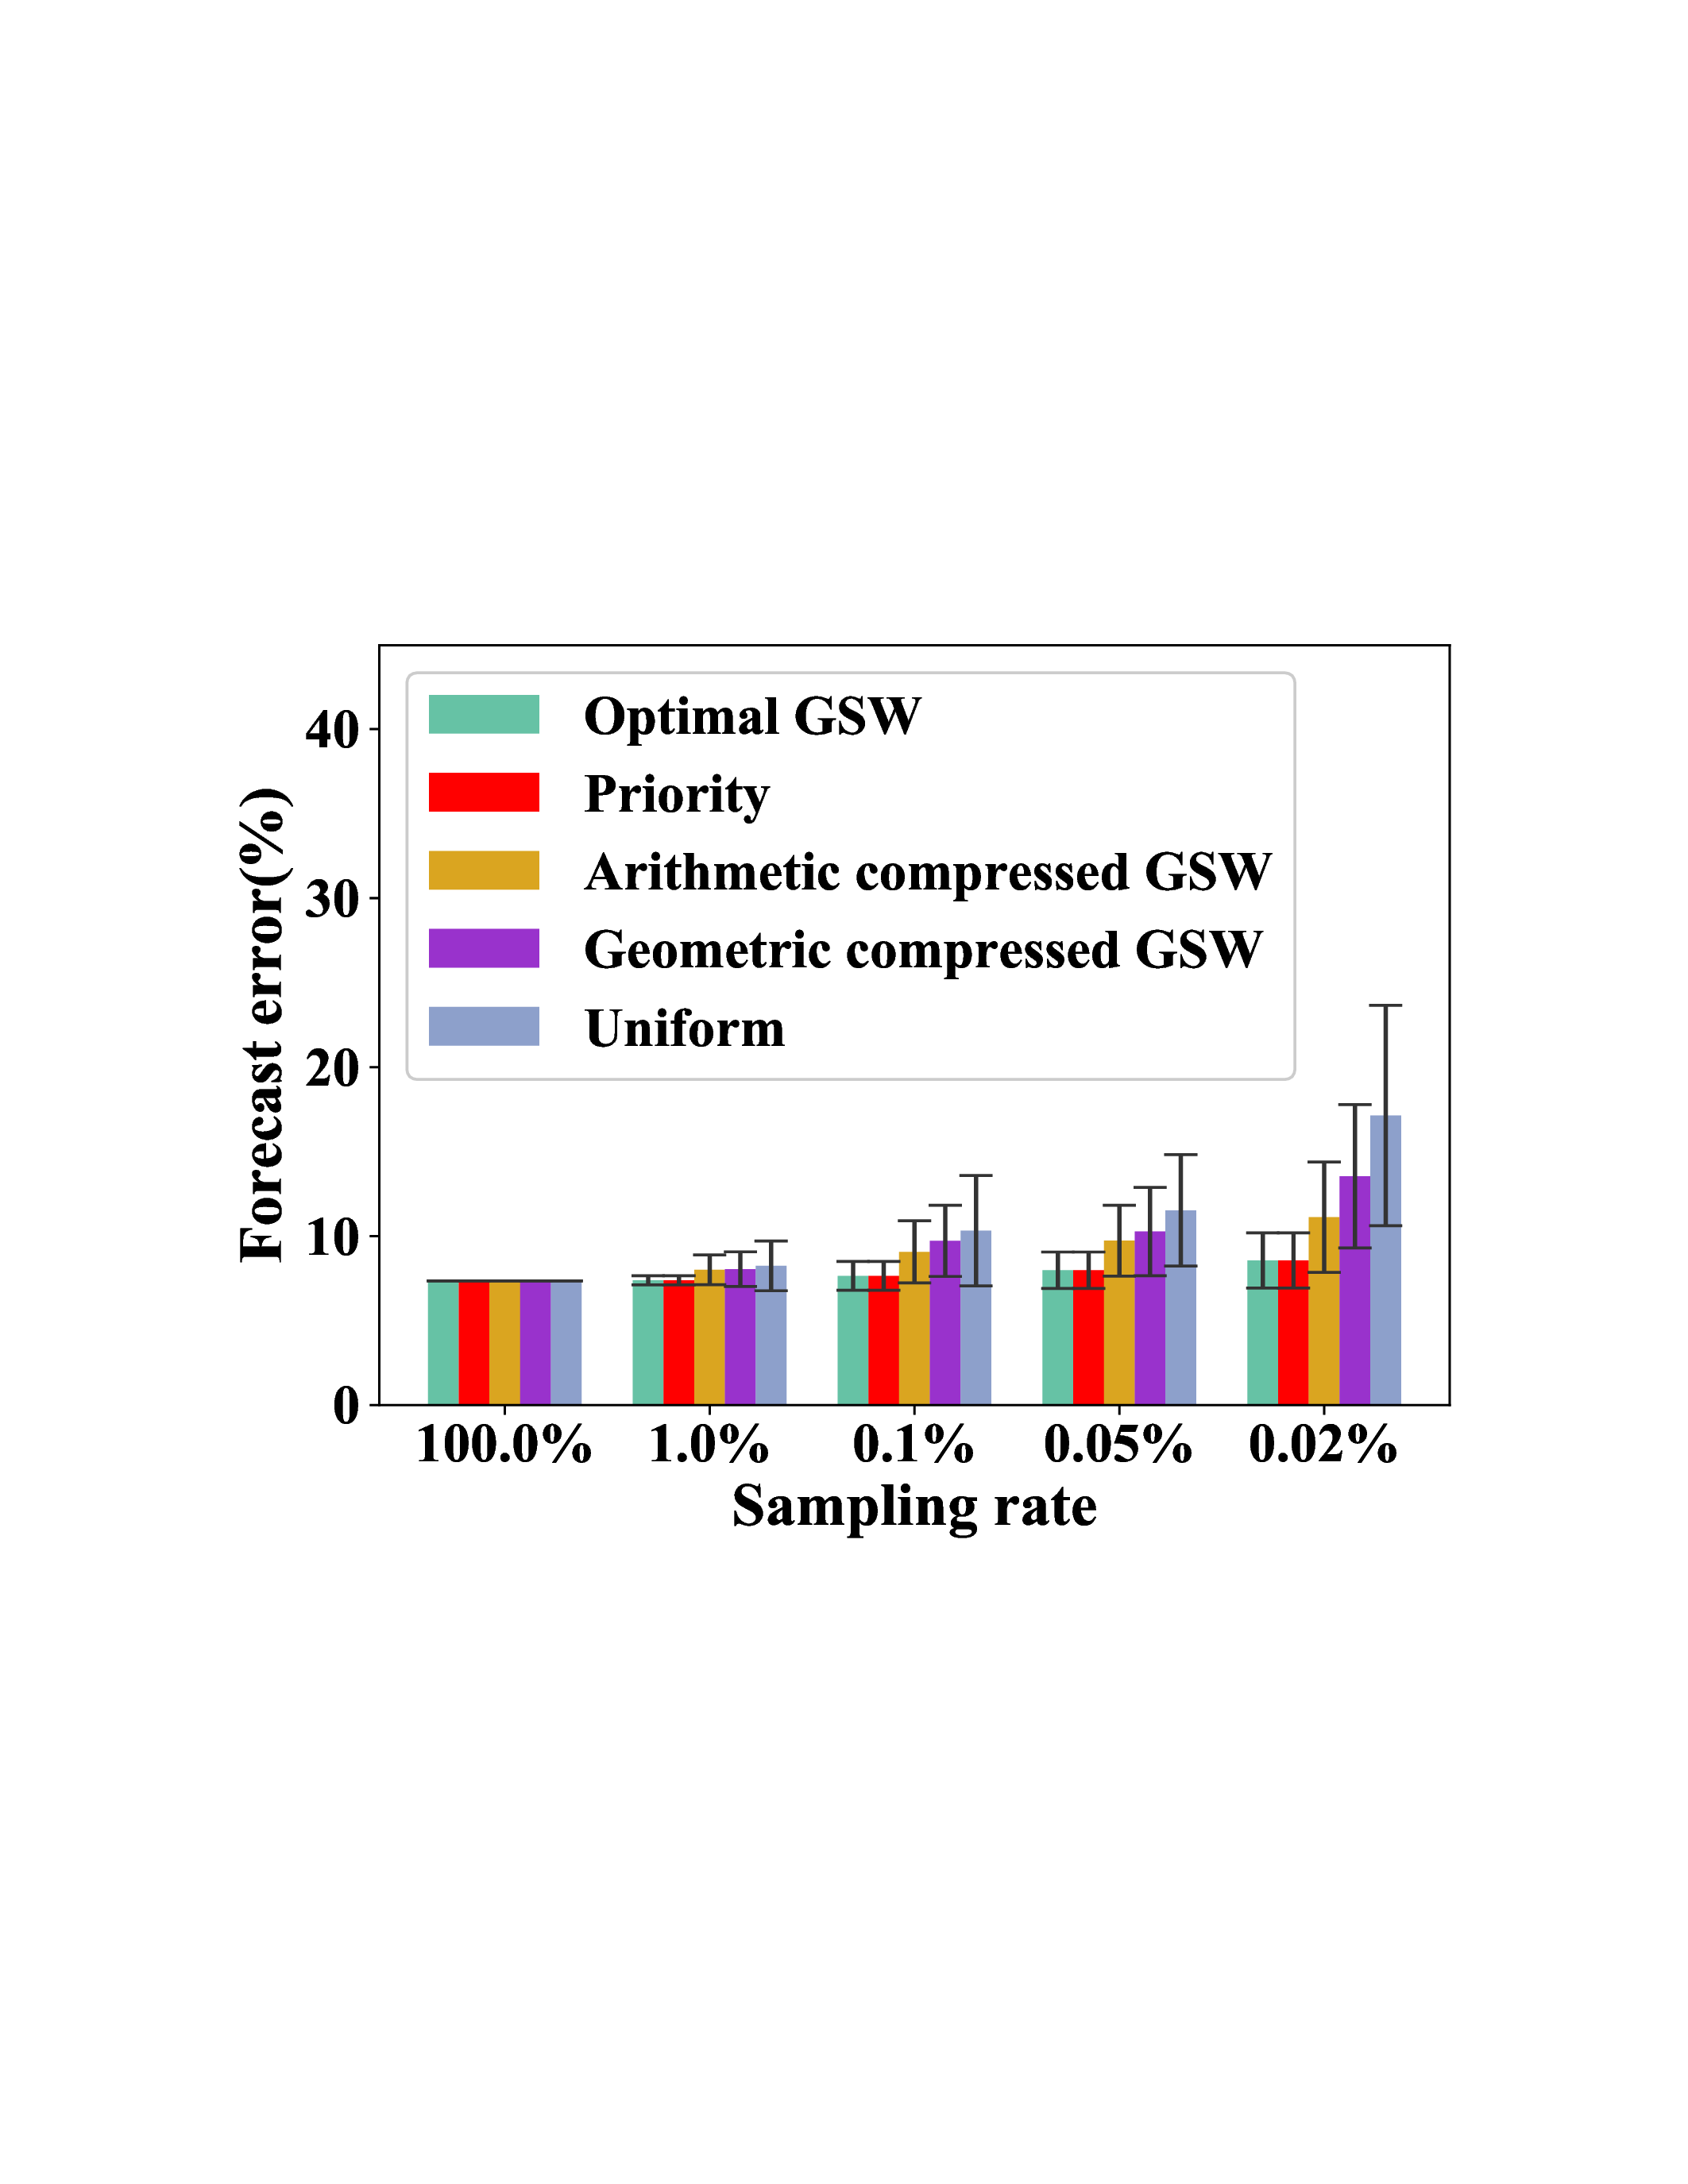}
\end{minipage}
}
\caption{ARIMA prediction error at different selectivity on favorite via different sampling methods}
% \label{AQP and ARIMA Performance}
\end{figure*}

%-----Favorite不同抽样方法对ARIMA Interval误差的影响----------
\begin{figure*}[hb]
\subfigure[Selectivity 0.5\%]{
\begin{minipage}[t]{0.33\linewidth}
\centering
\includegraphics[width=2.2in, height=2.0in]{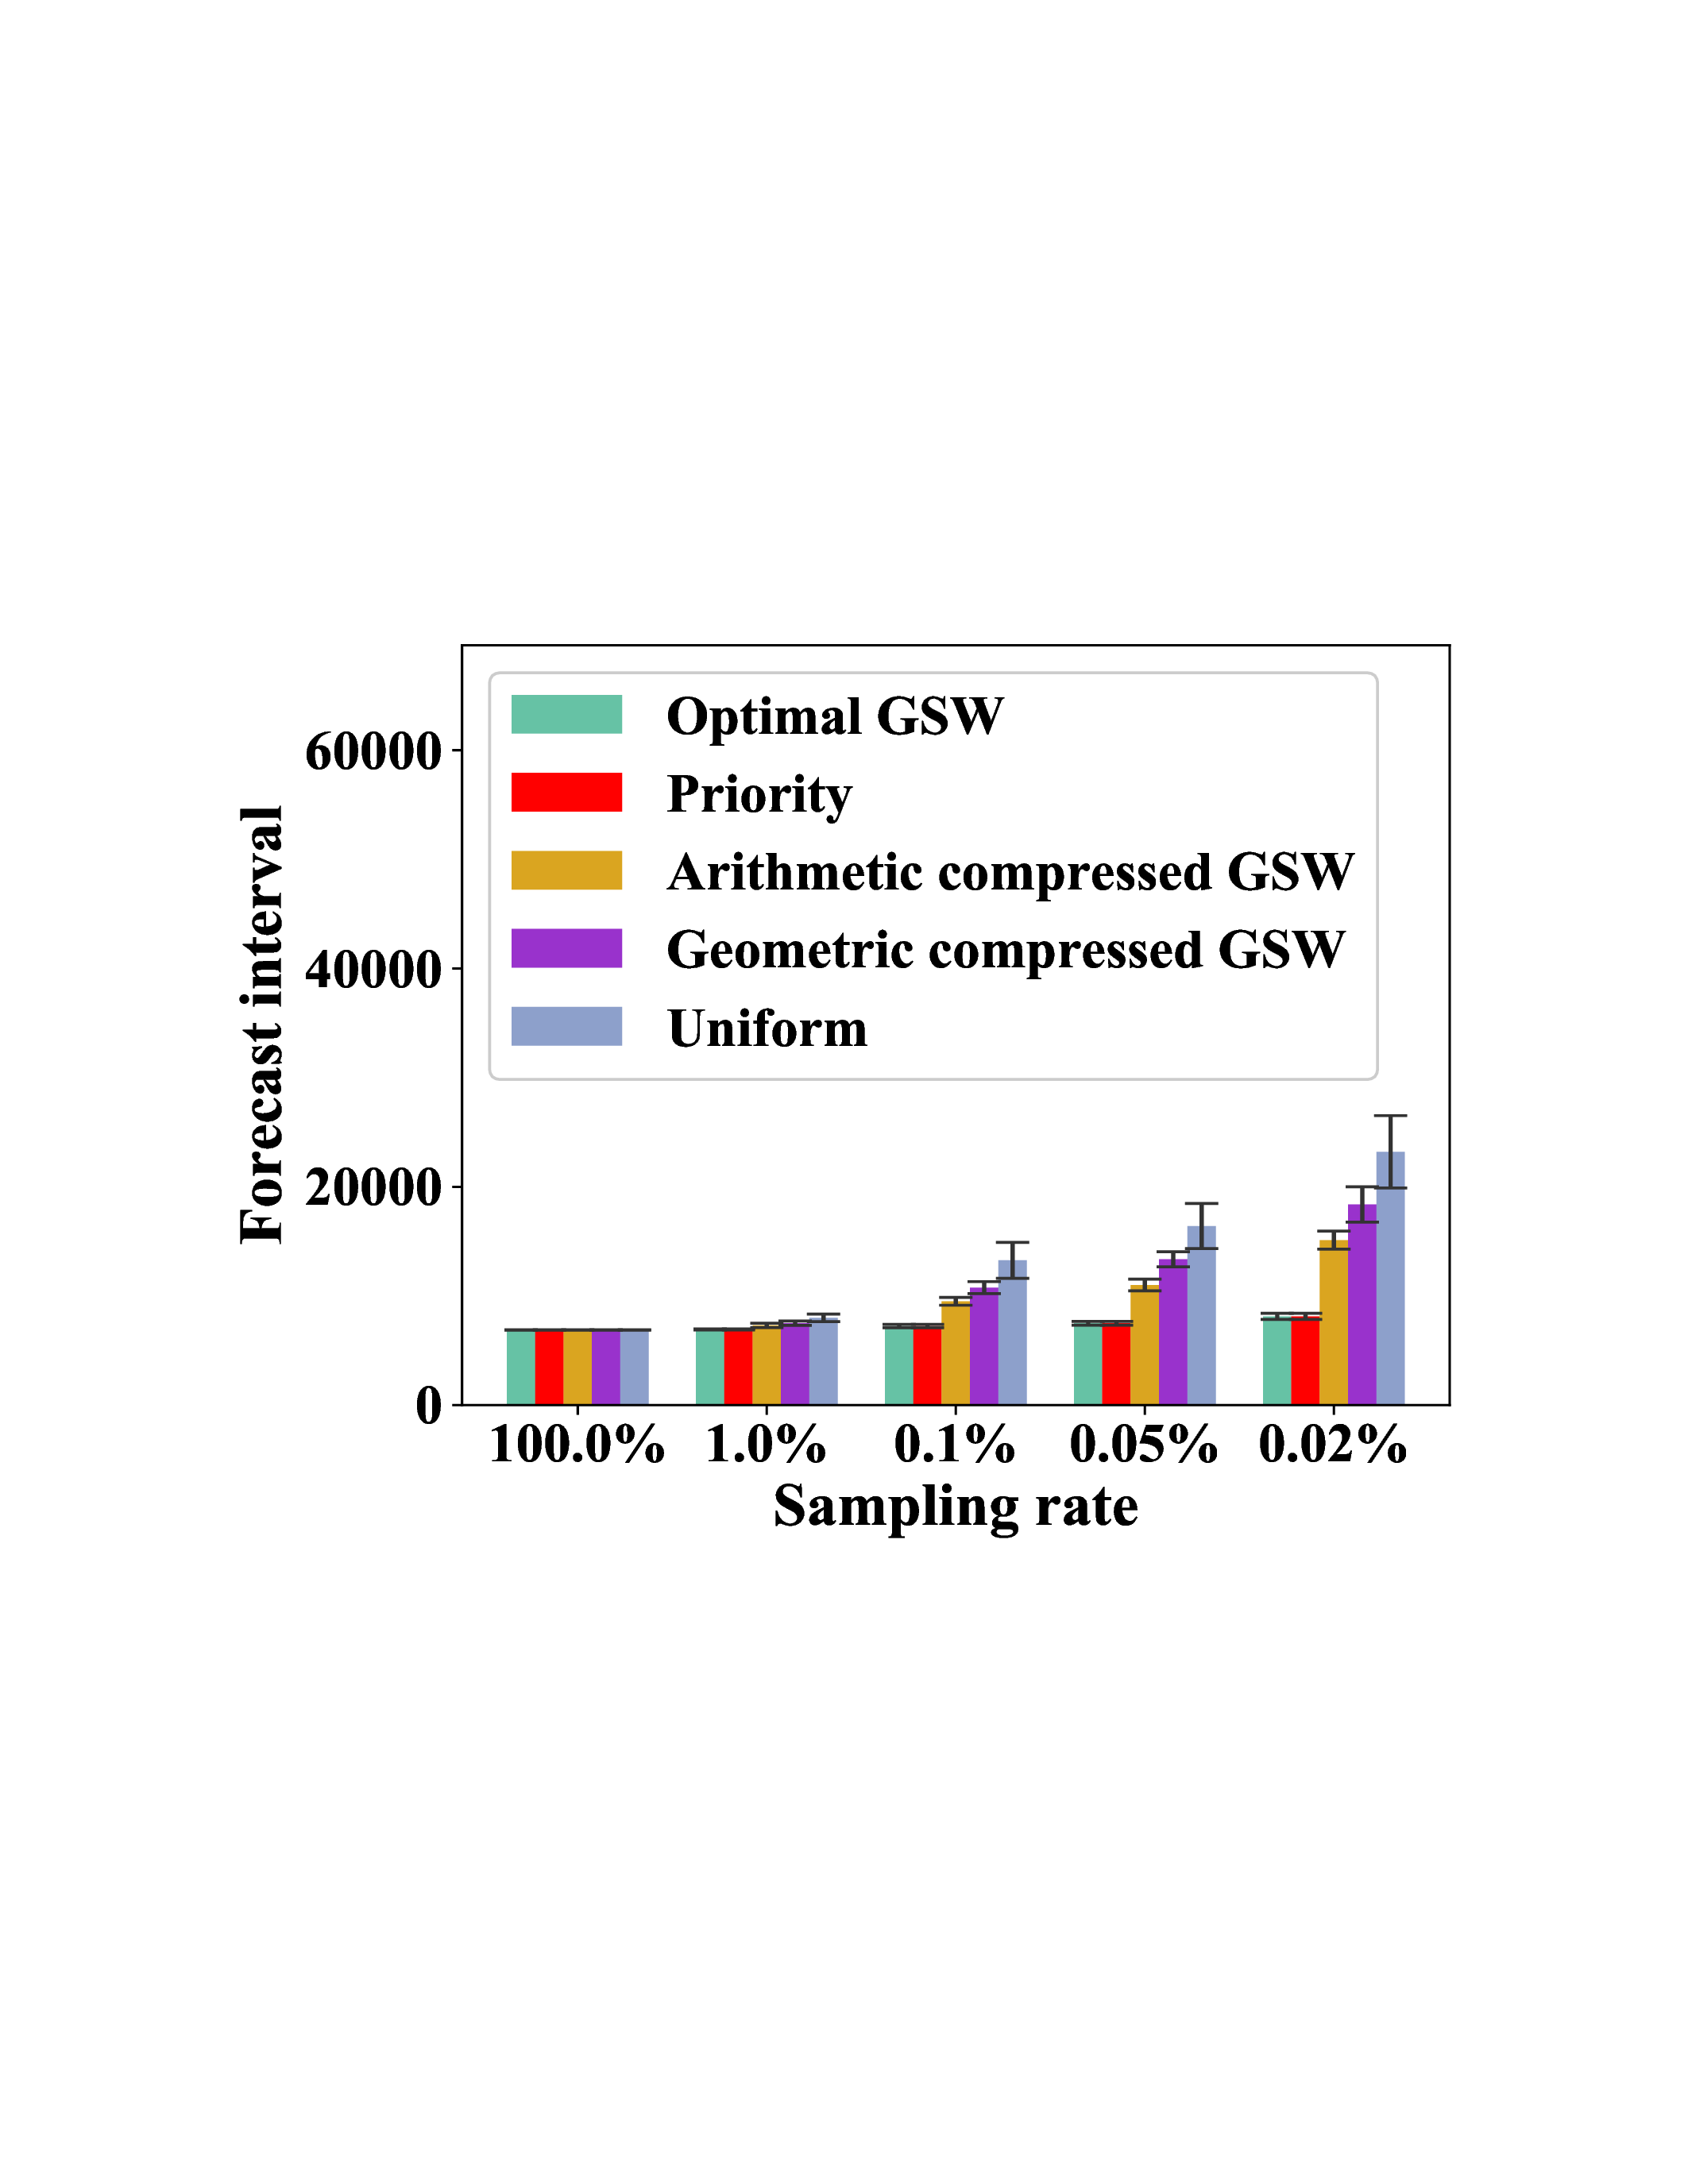}
% \label{fig:side:a}
\end{minipage}
}
\subfigure[Selectivity 1\%]{
\begin{minipage}[t]{0.33\linewidth}
\centering
\includegraphics[width=2.2in, height=2.0in]{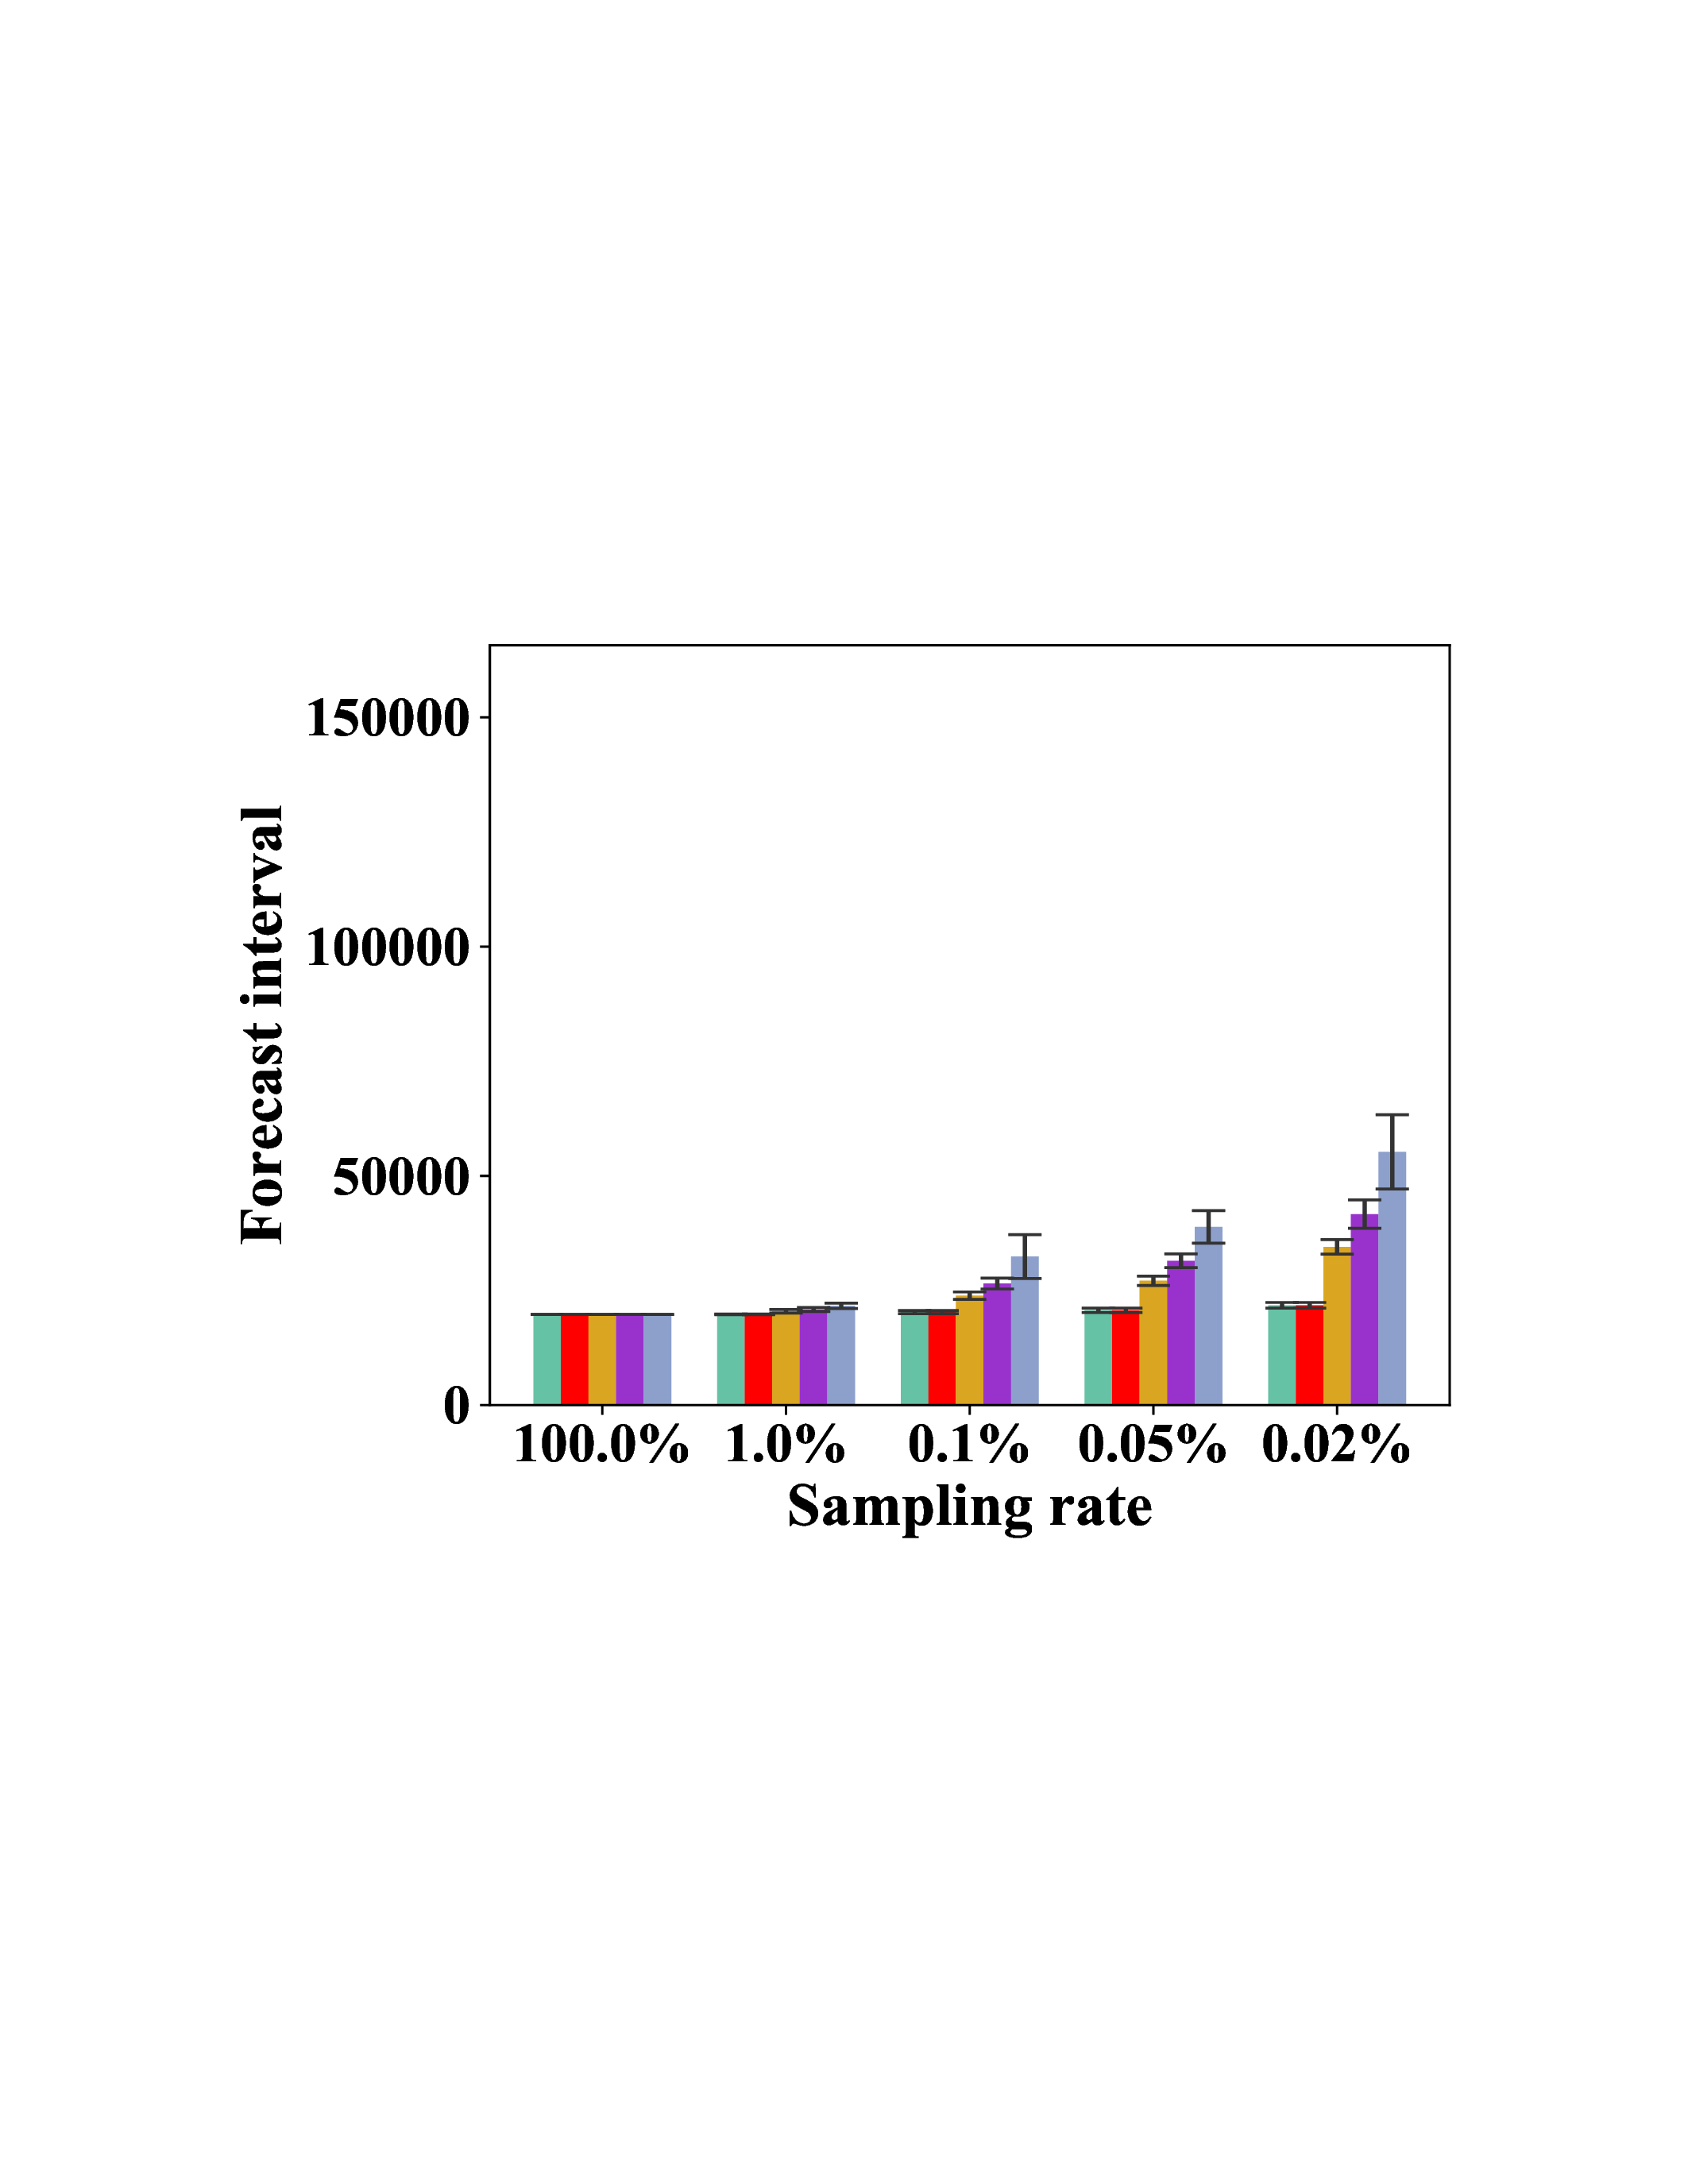}
\end{minipage}
}
\subfigure[Selectivity 5\%]{
\begin{minipage}[t]{0.33\linewidth}
\centering
\includegraphics[width=2.2in, height=2.0in]{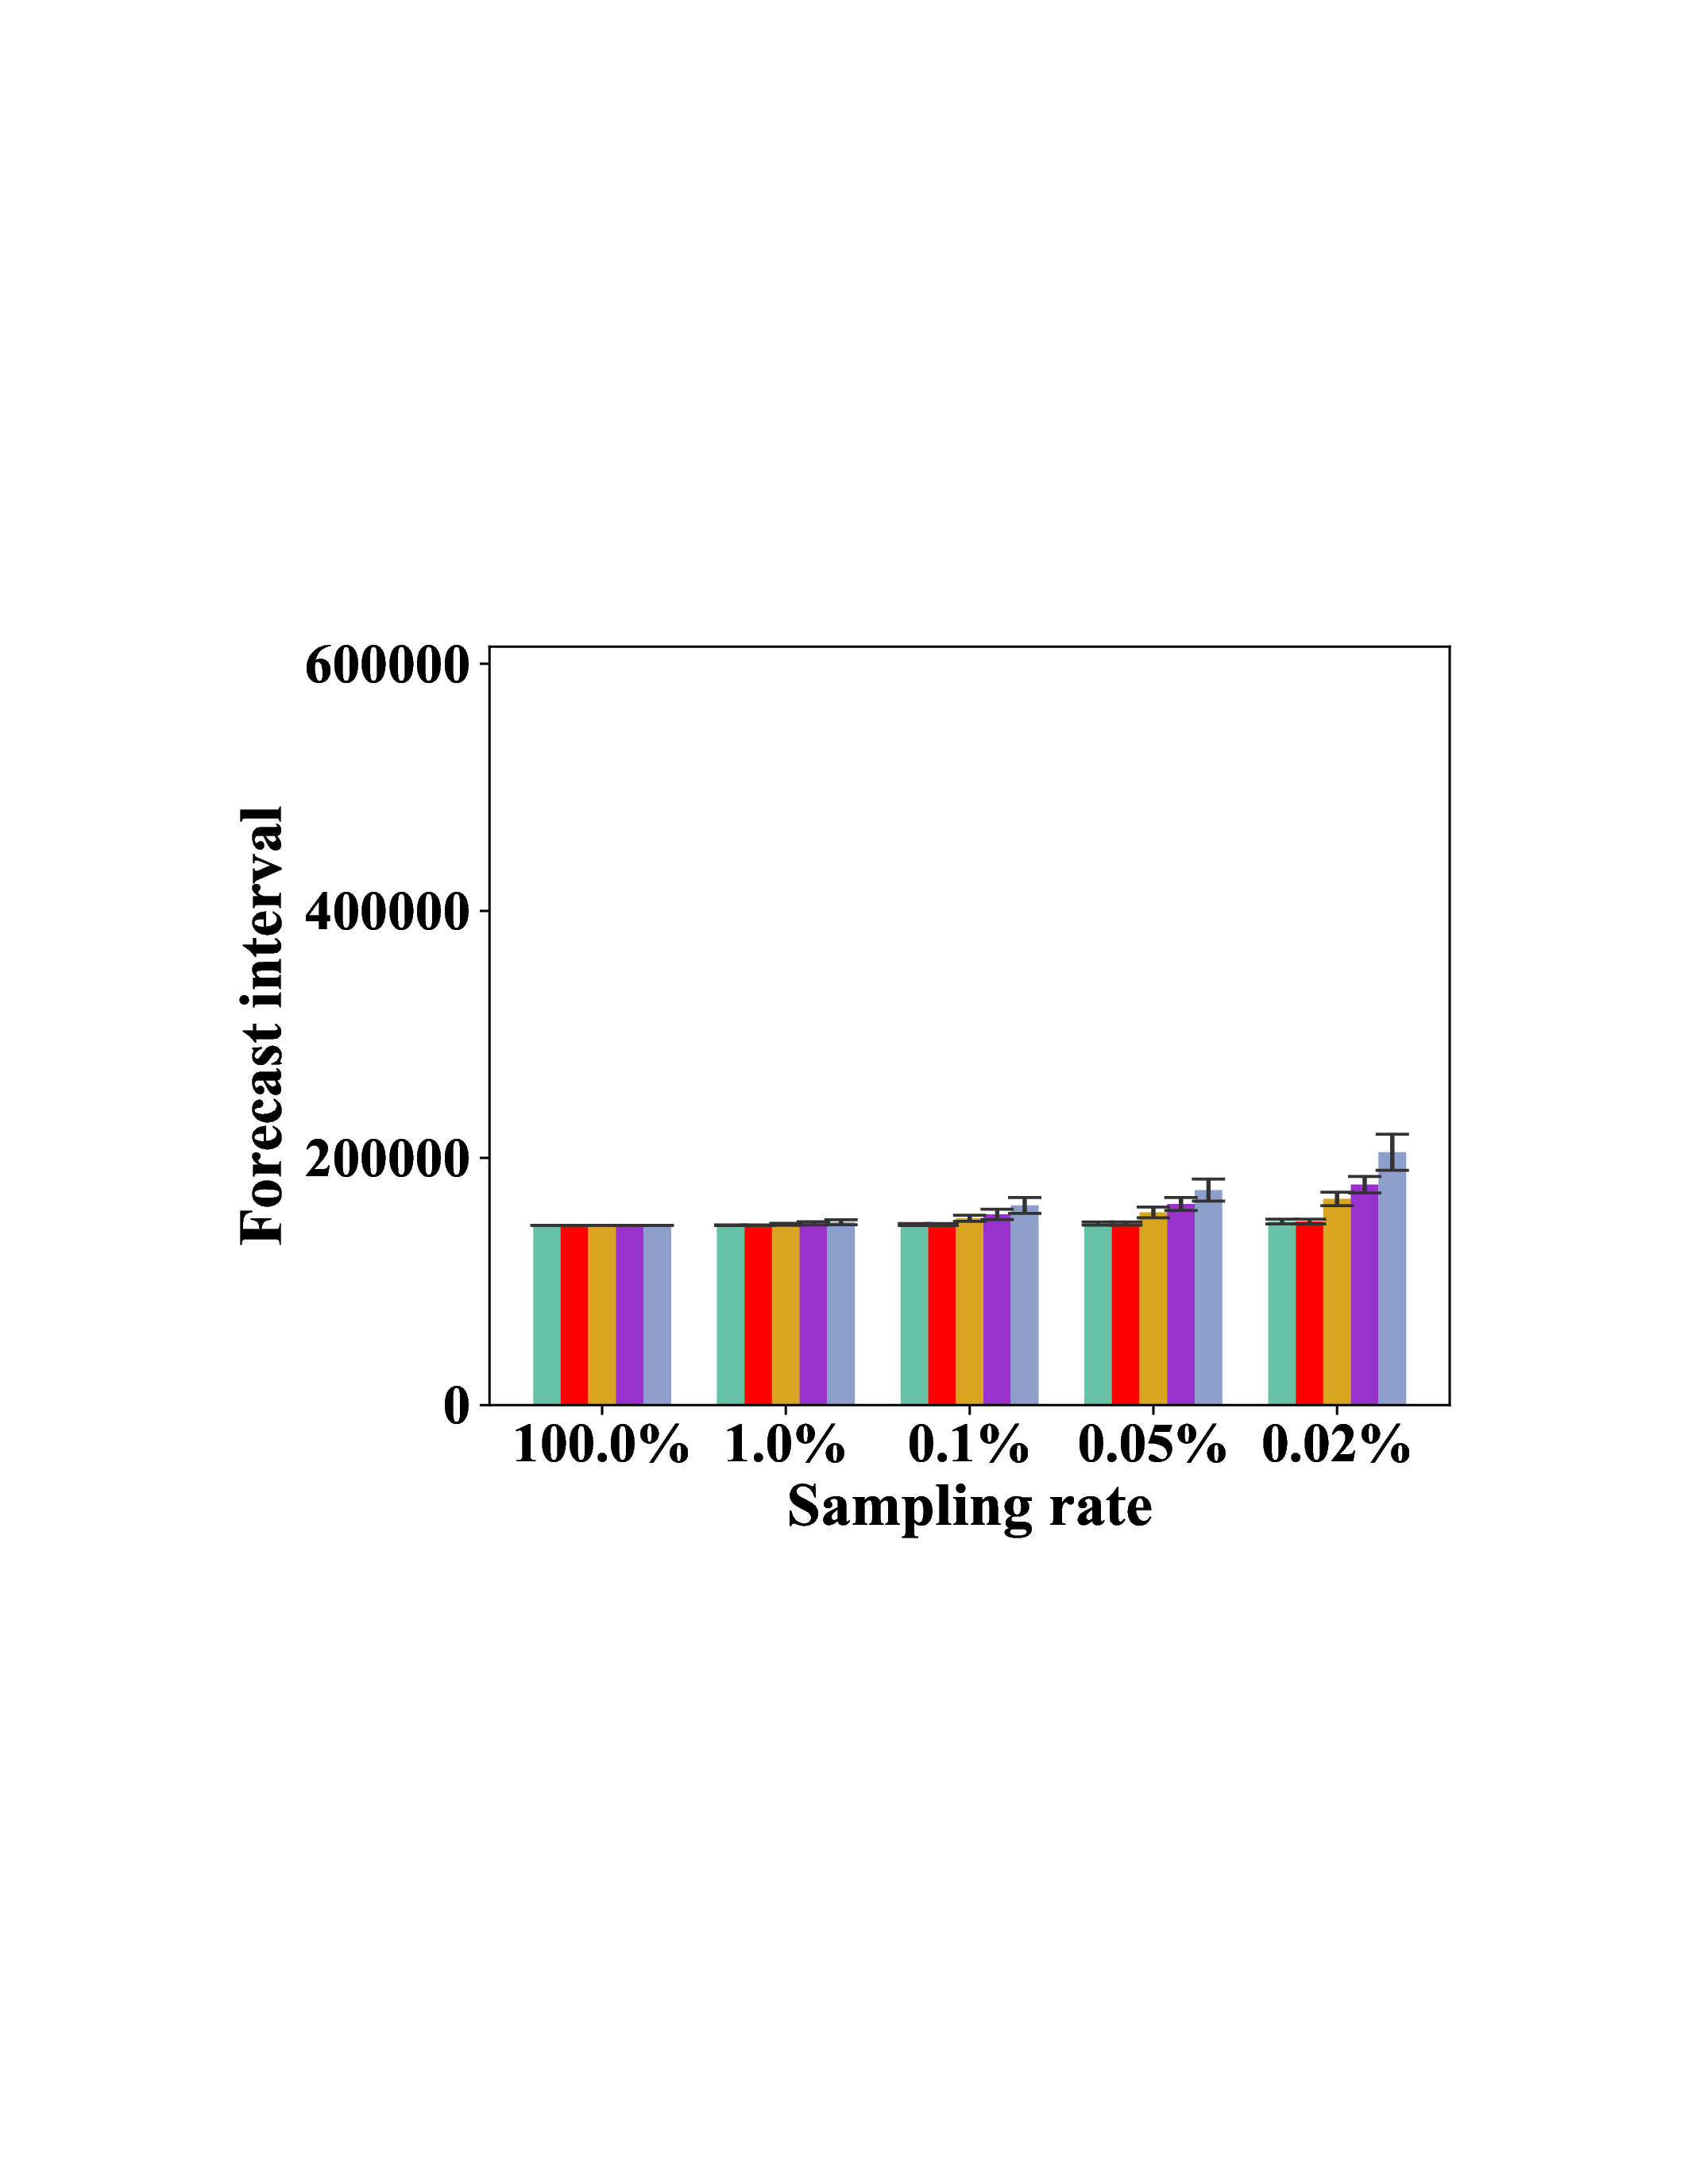}
\end{minipage}
}
\caption{ARIMA prediction interval at different selectivity on favorite via different sampling methods}
% \label{AQP and ARIMA Performance}
\end{figure*}

%============================

%-----Cart不同抽样方法对AQP误差的影响----------
\begin{figure*}[hb]
\subfigure[Selectivity 0.5\%]{
\begin{minipage}[t]{0.33\linewidth}
\centering
\includegraphics[width=2.2in, height=2.0in]{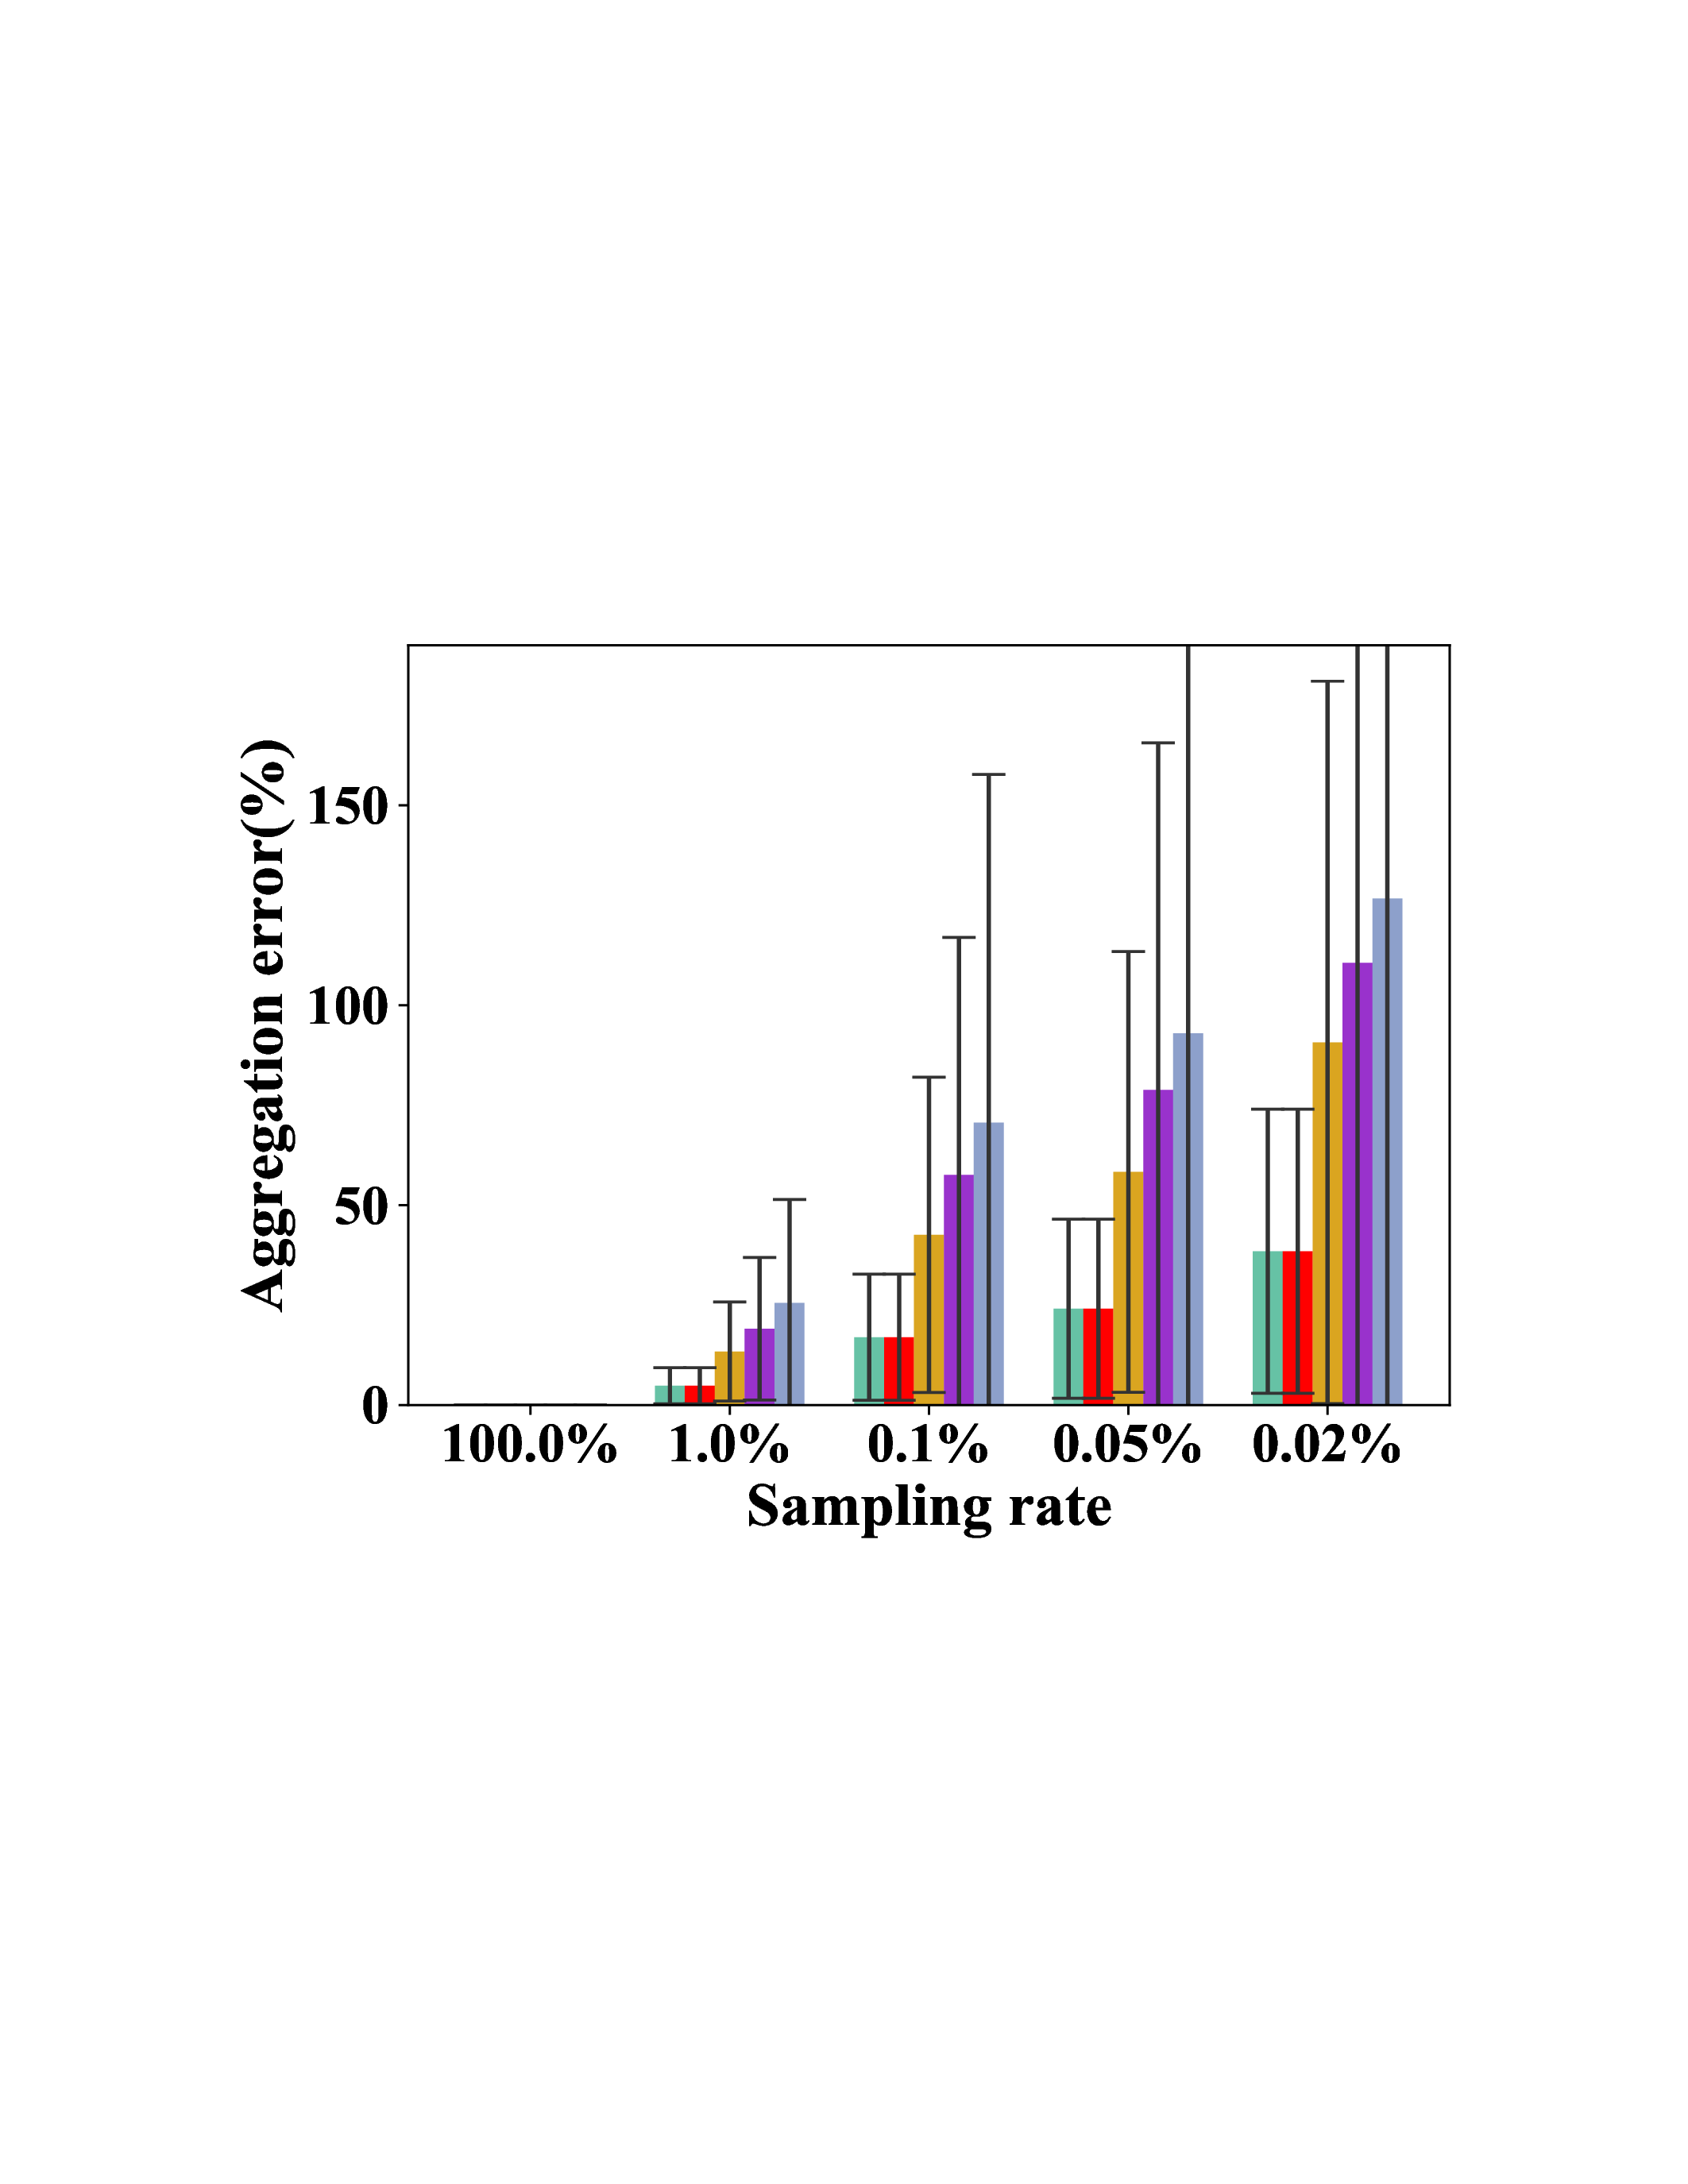}
% \label{fig:side:a}
\end{minipage}
}
\subfigure[Selectivity 1\%]{
\begin{minipage}[t]{0.33\linewidth}
\centering
\includegraphics[width=2.2in, height=2.0in]{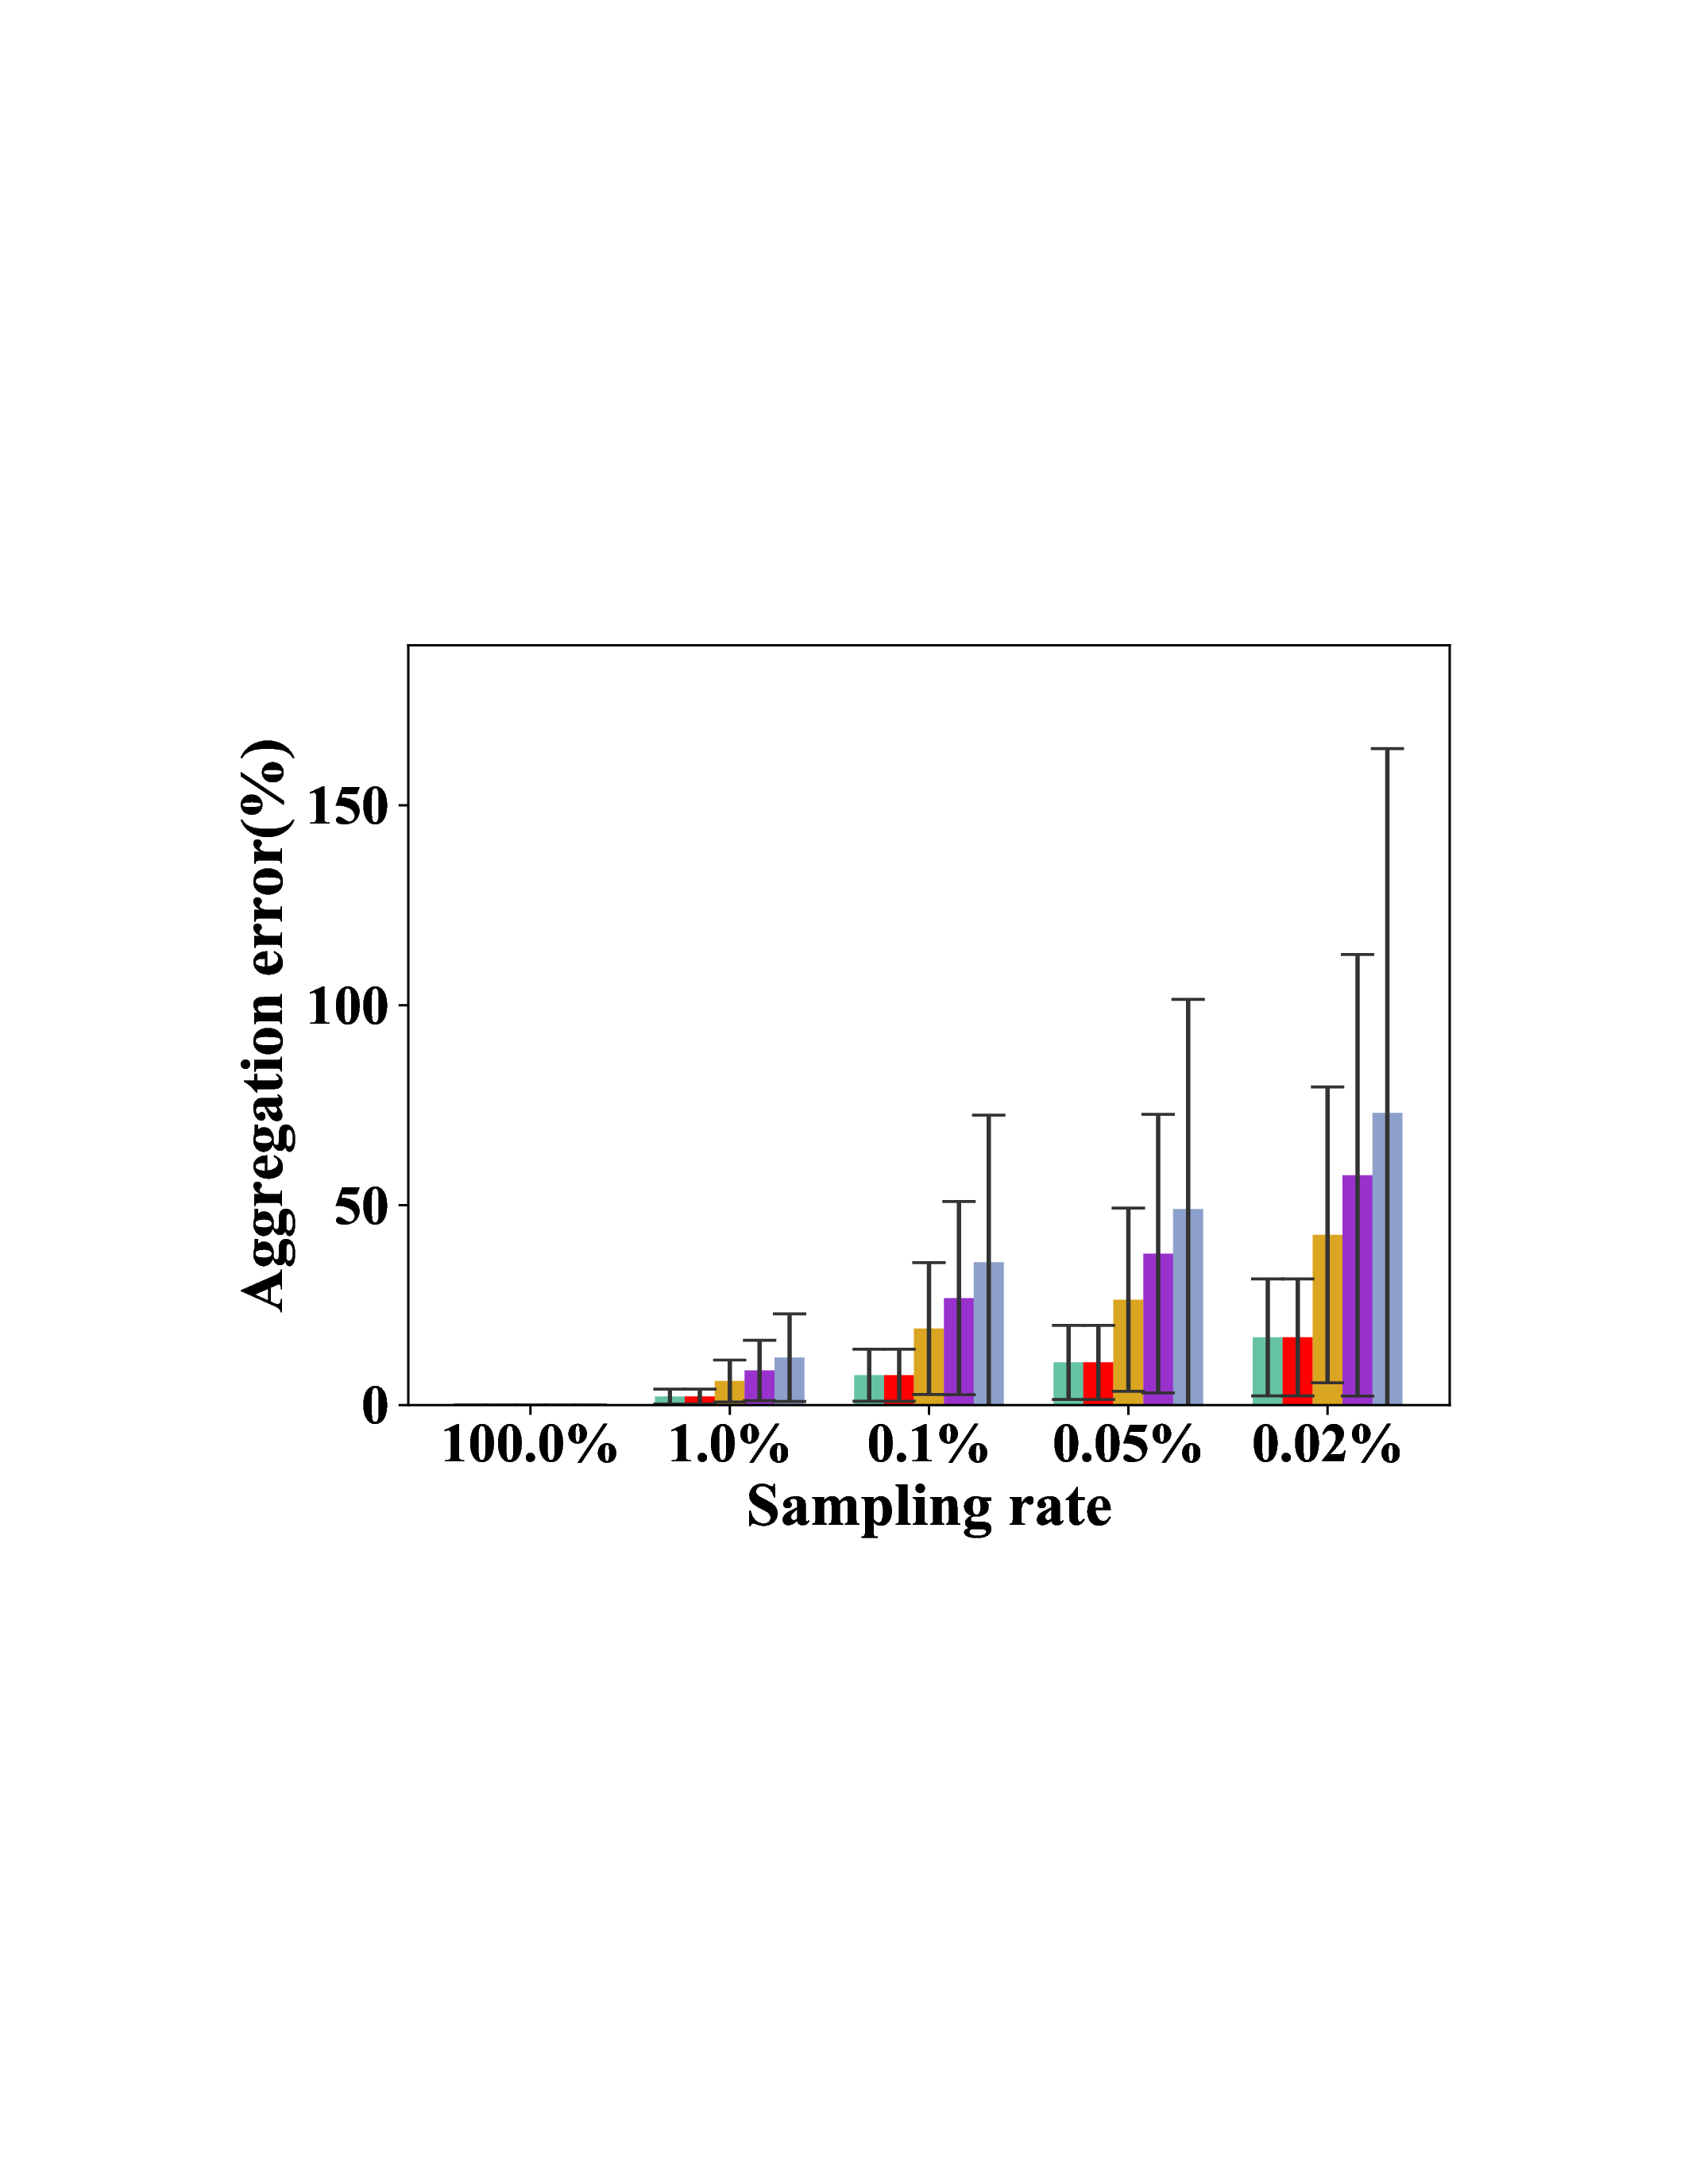}
\end{minipage}
}
\subfigure[Selectivity 5\%]{
\begin{minipage}[t]{0.33\linewidth}
\centering
\includegraphics[width=2.2in, height=2.0in]{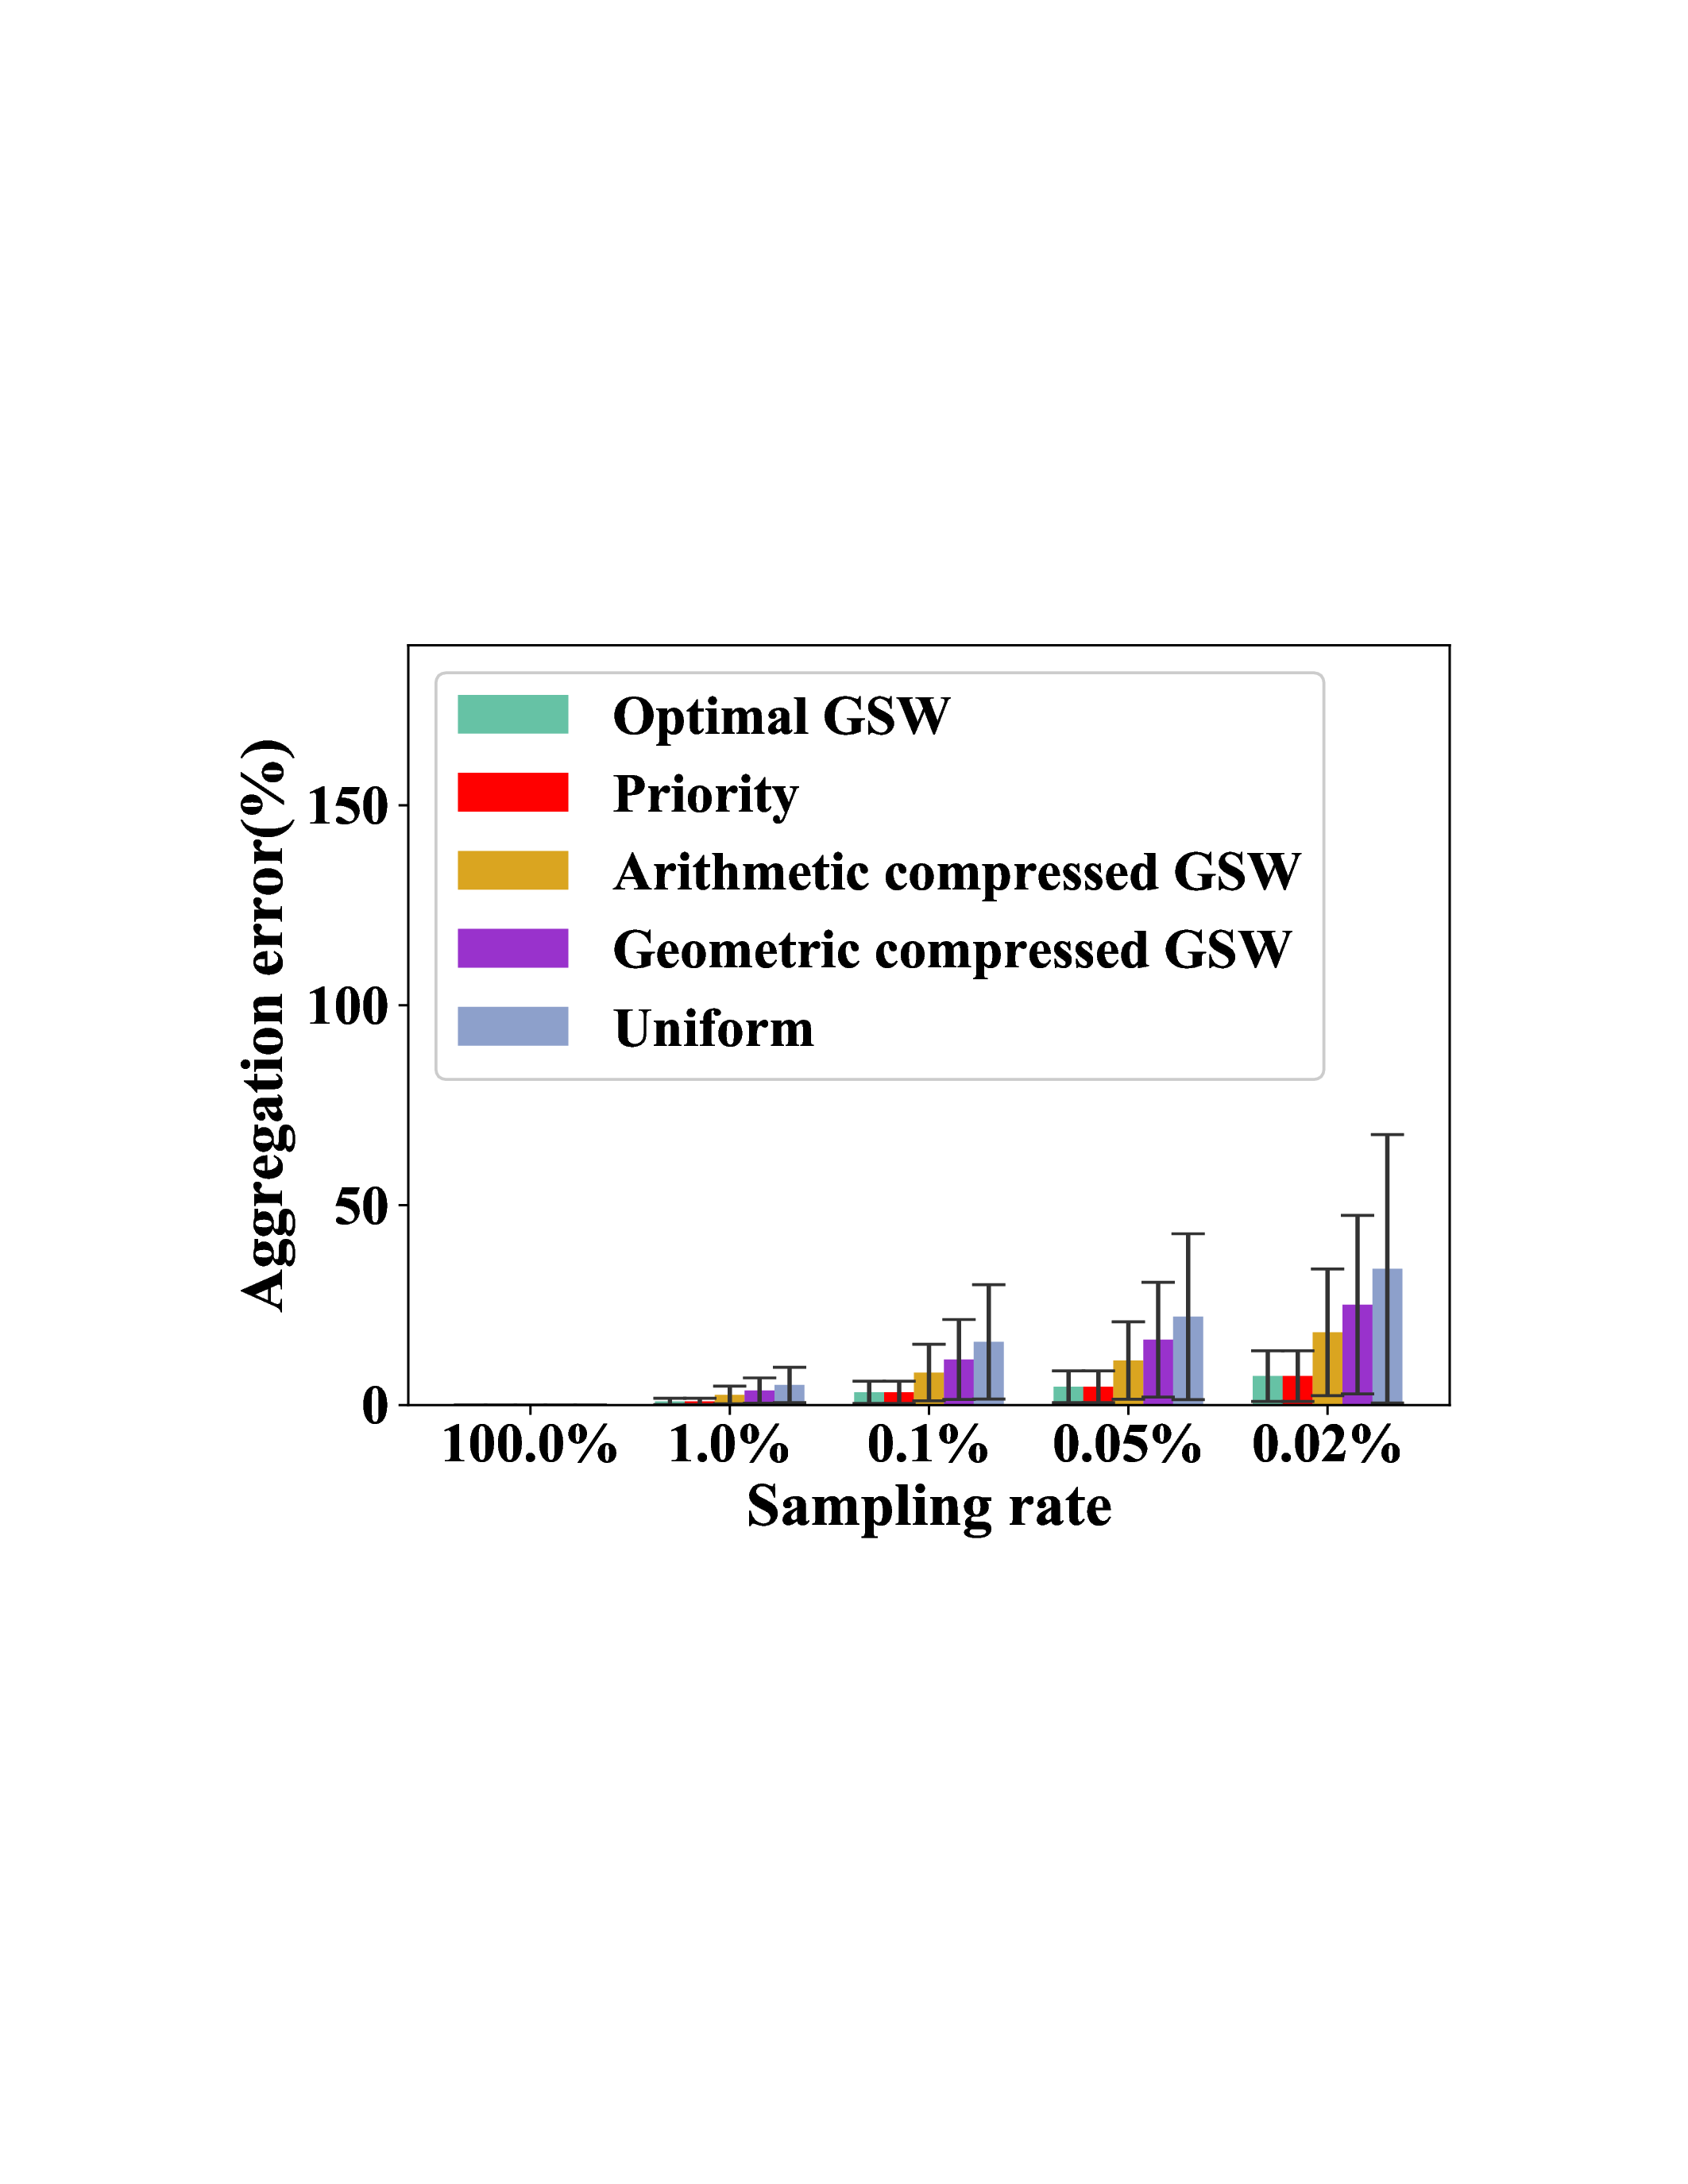}
\end{minipage}
}
\caption{AQP error at different selectivity on Cart via different sampling methods}
% \label{AQP and ARIMA Performance}
\end{figure*}

%-----Cart不同抽样方法对ARIMA误差的影响----------
\begin{figure*}[hb]
\subfigure[Selectivity 0.5\%]{
\begin{minipage}[t]{0.33\linewidth}
\centering
\includegraphics[width=2.2in,height=2.0in]{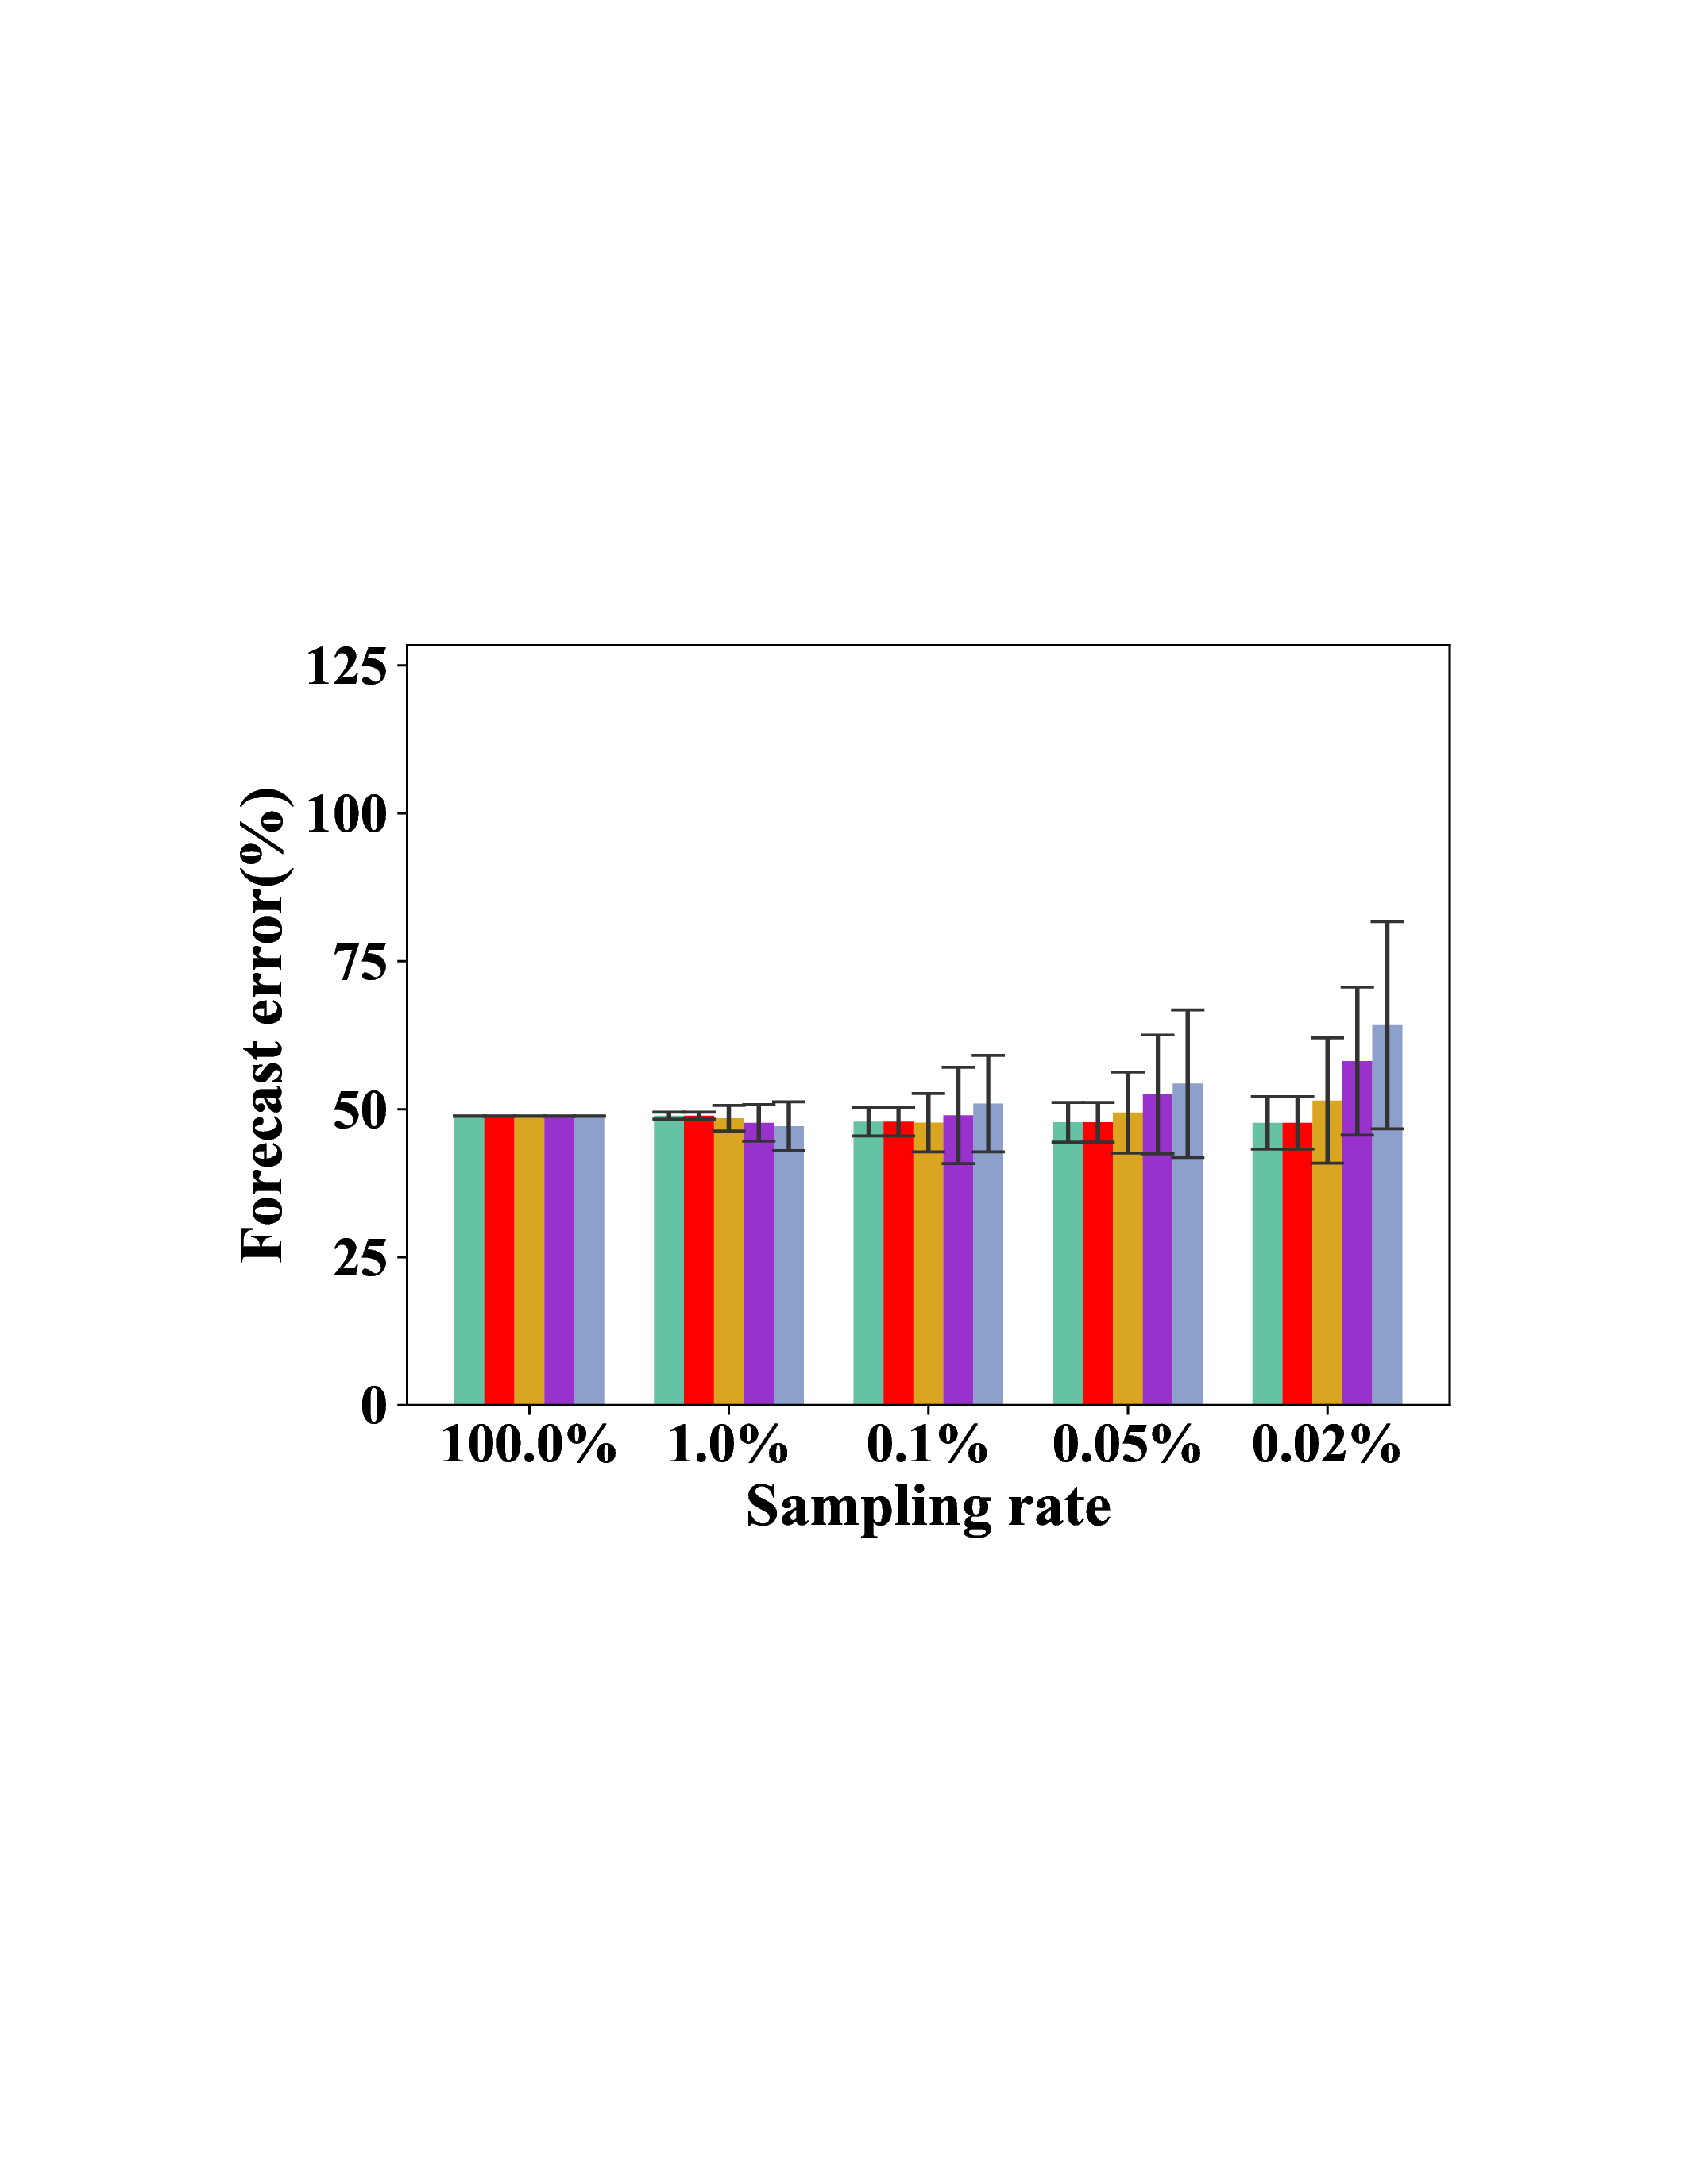}
% \label{fig:side:a}
\end{minipage}
}
\subfigure[Selectivity 1\%]{
\begin{minipage}[t]{0.33\linewidth}
\centering
\includegraphics[width=2.2in,height=2.0in]{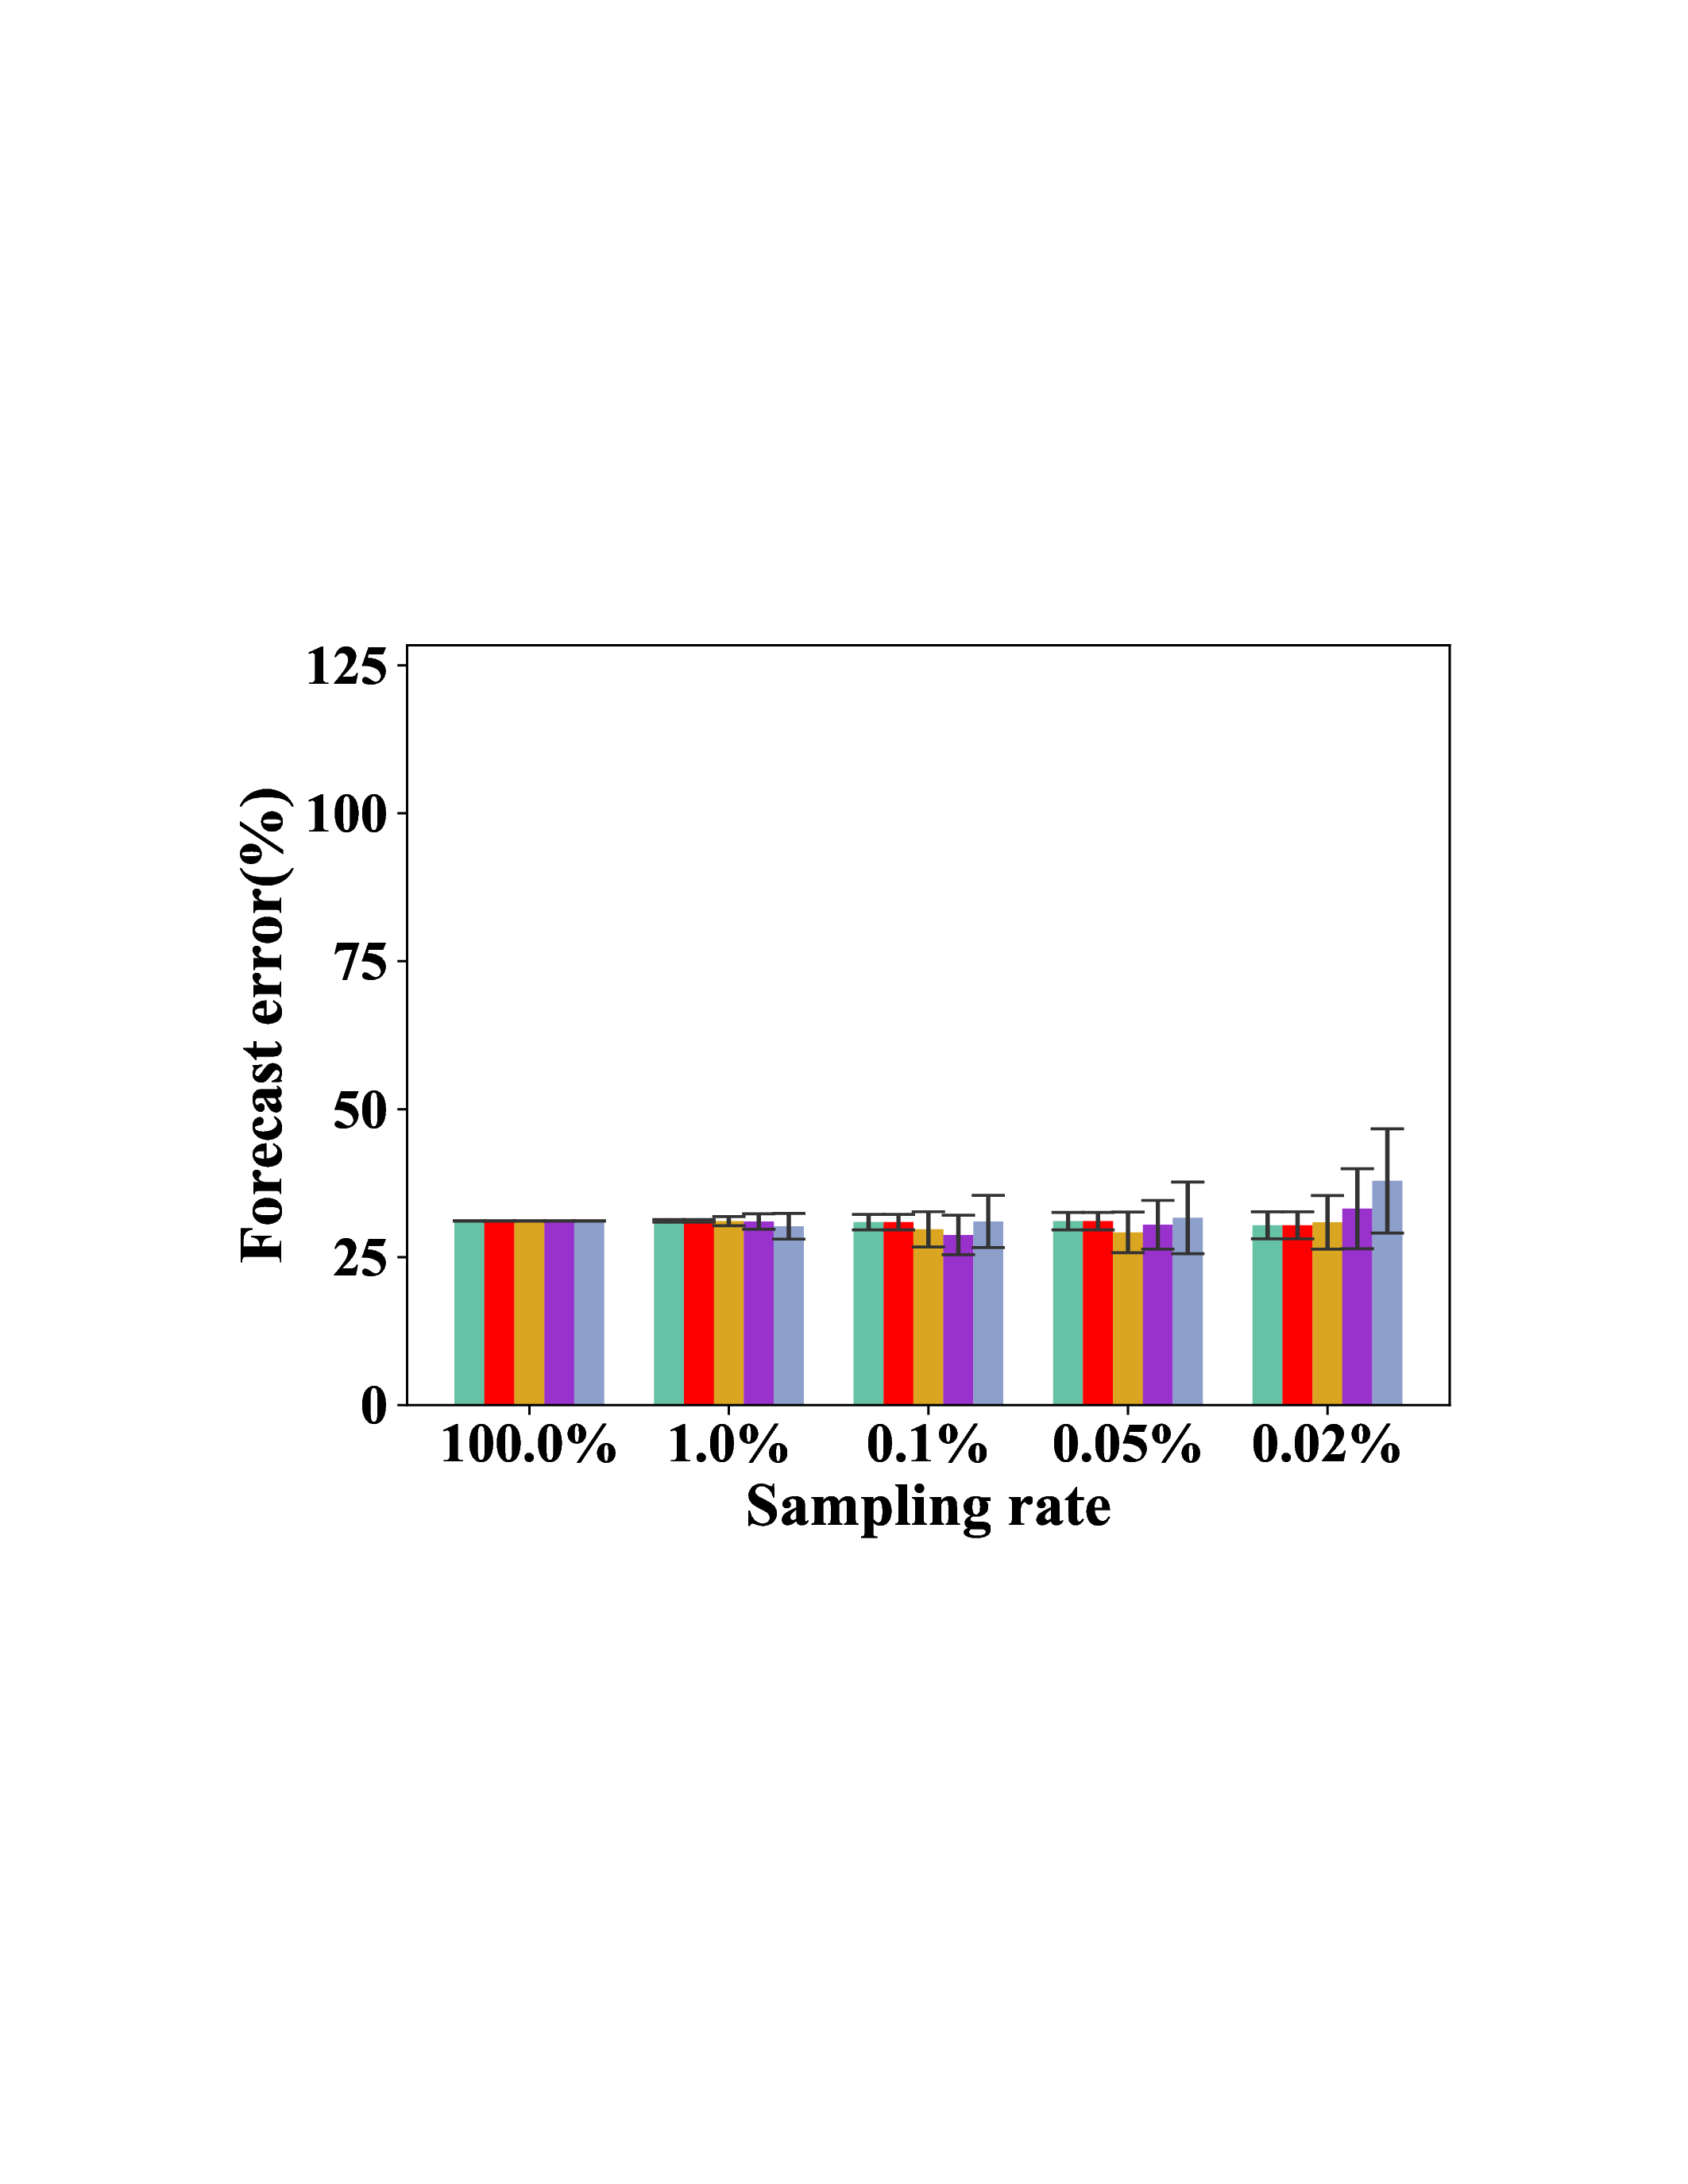}
\end{minipage}
}
\subfigure[Selectivity 5\%]{
\begin{minipage}[t]{0.33\linewidth}
\centering
\includegraphics[width=2.2in,height=2.0in]{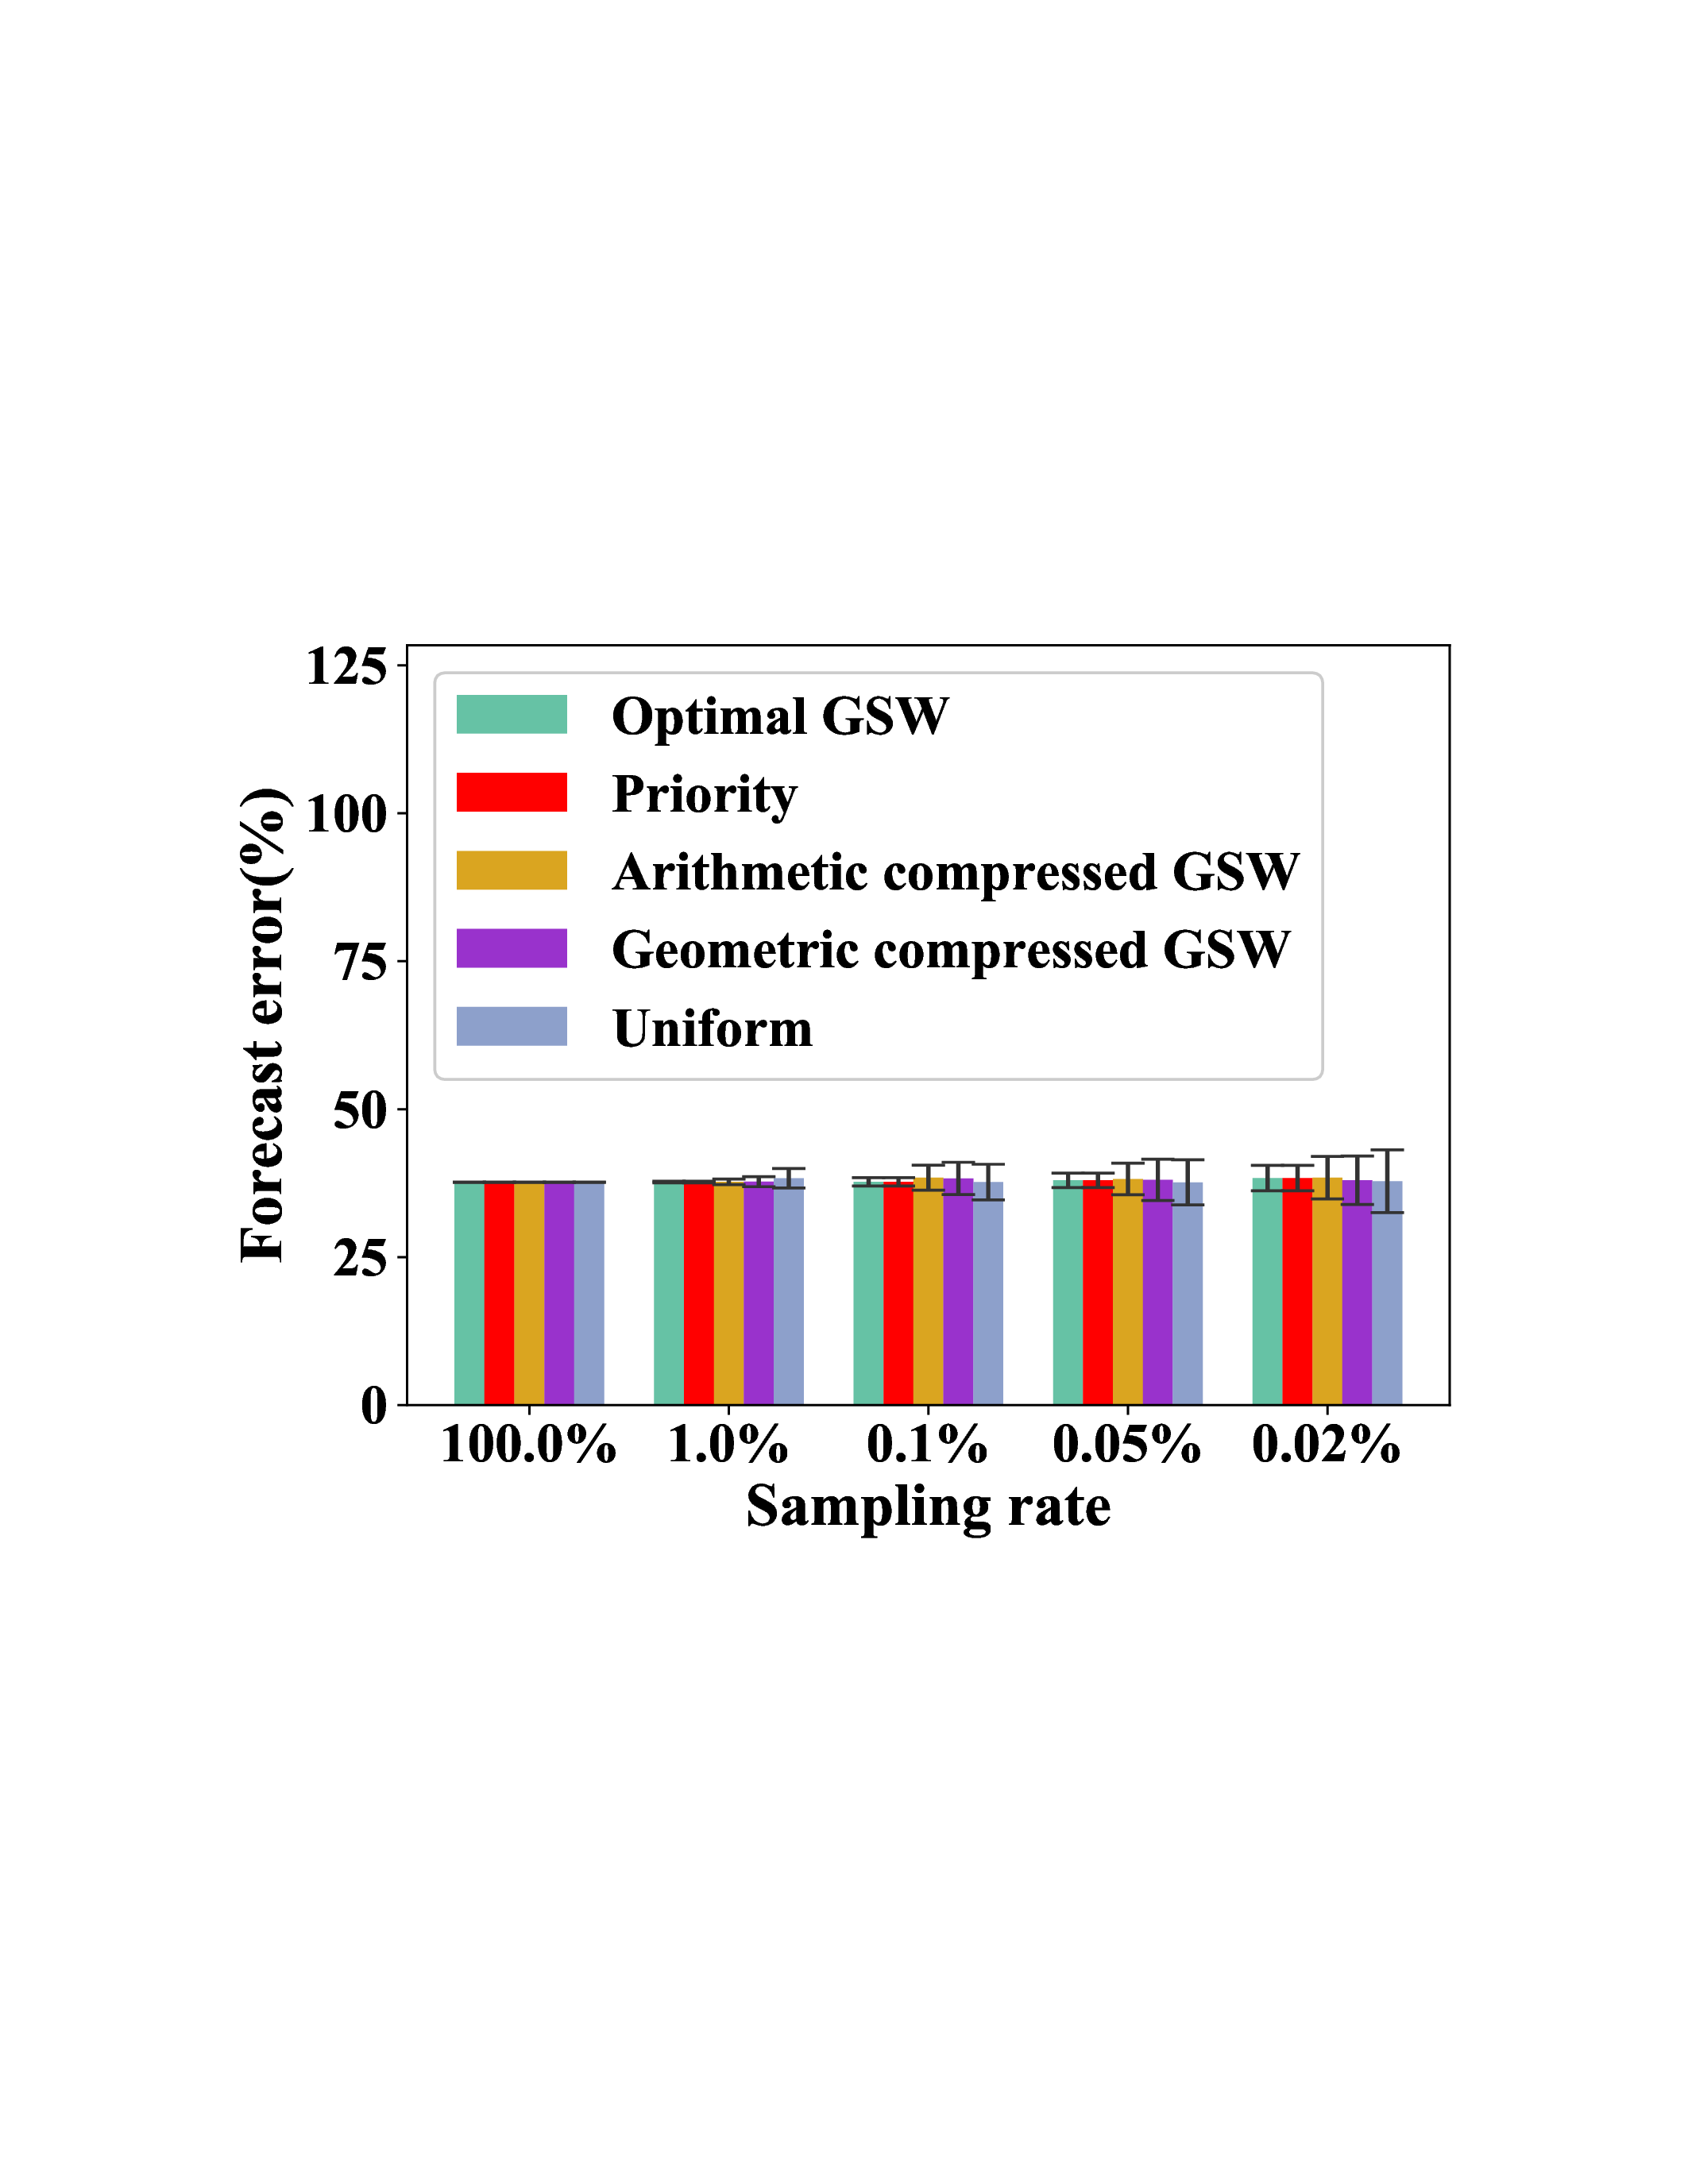}
\end{minipage}
}
\caption{ARIMA prediction error at different selectivity on Cart via different sampling methods}
% \label{AQP and ARIMA Performance}
\end{figure*}

%-----Cart不同抽样方法对ARIMA Interval误差的影响----------
\begin{figure*}[hb]
\subfigure[Selectivity 0.5\%]{
\begin{minipage}[t]{0.33\linewidth}
\centering
\includegraphics[width=2.2in, height=2.0in]{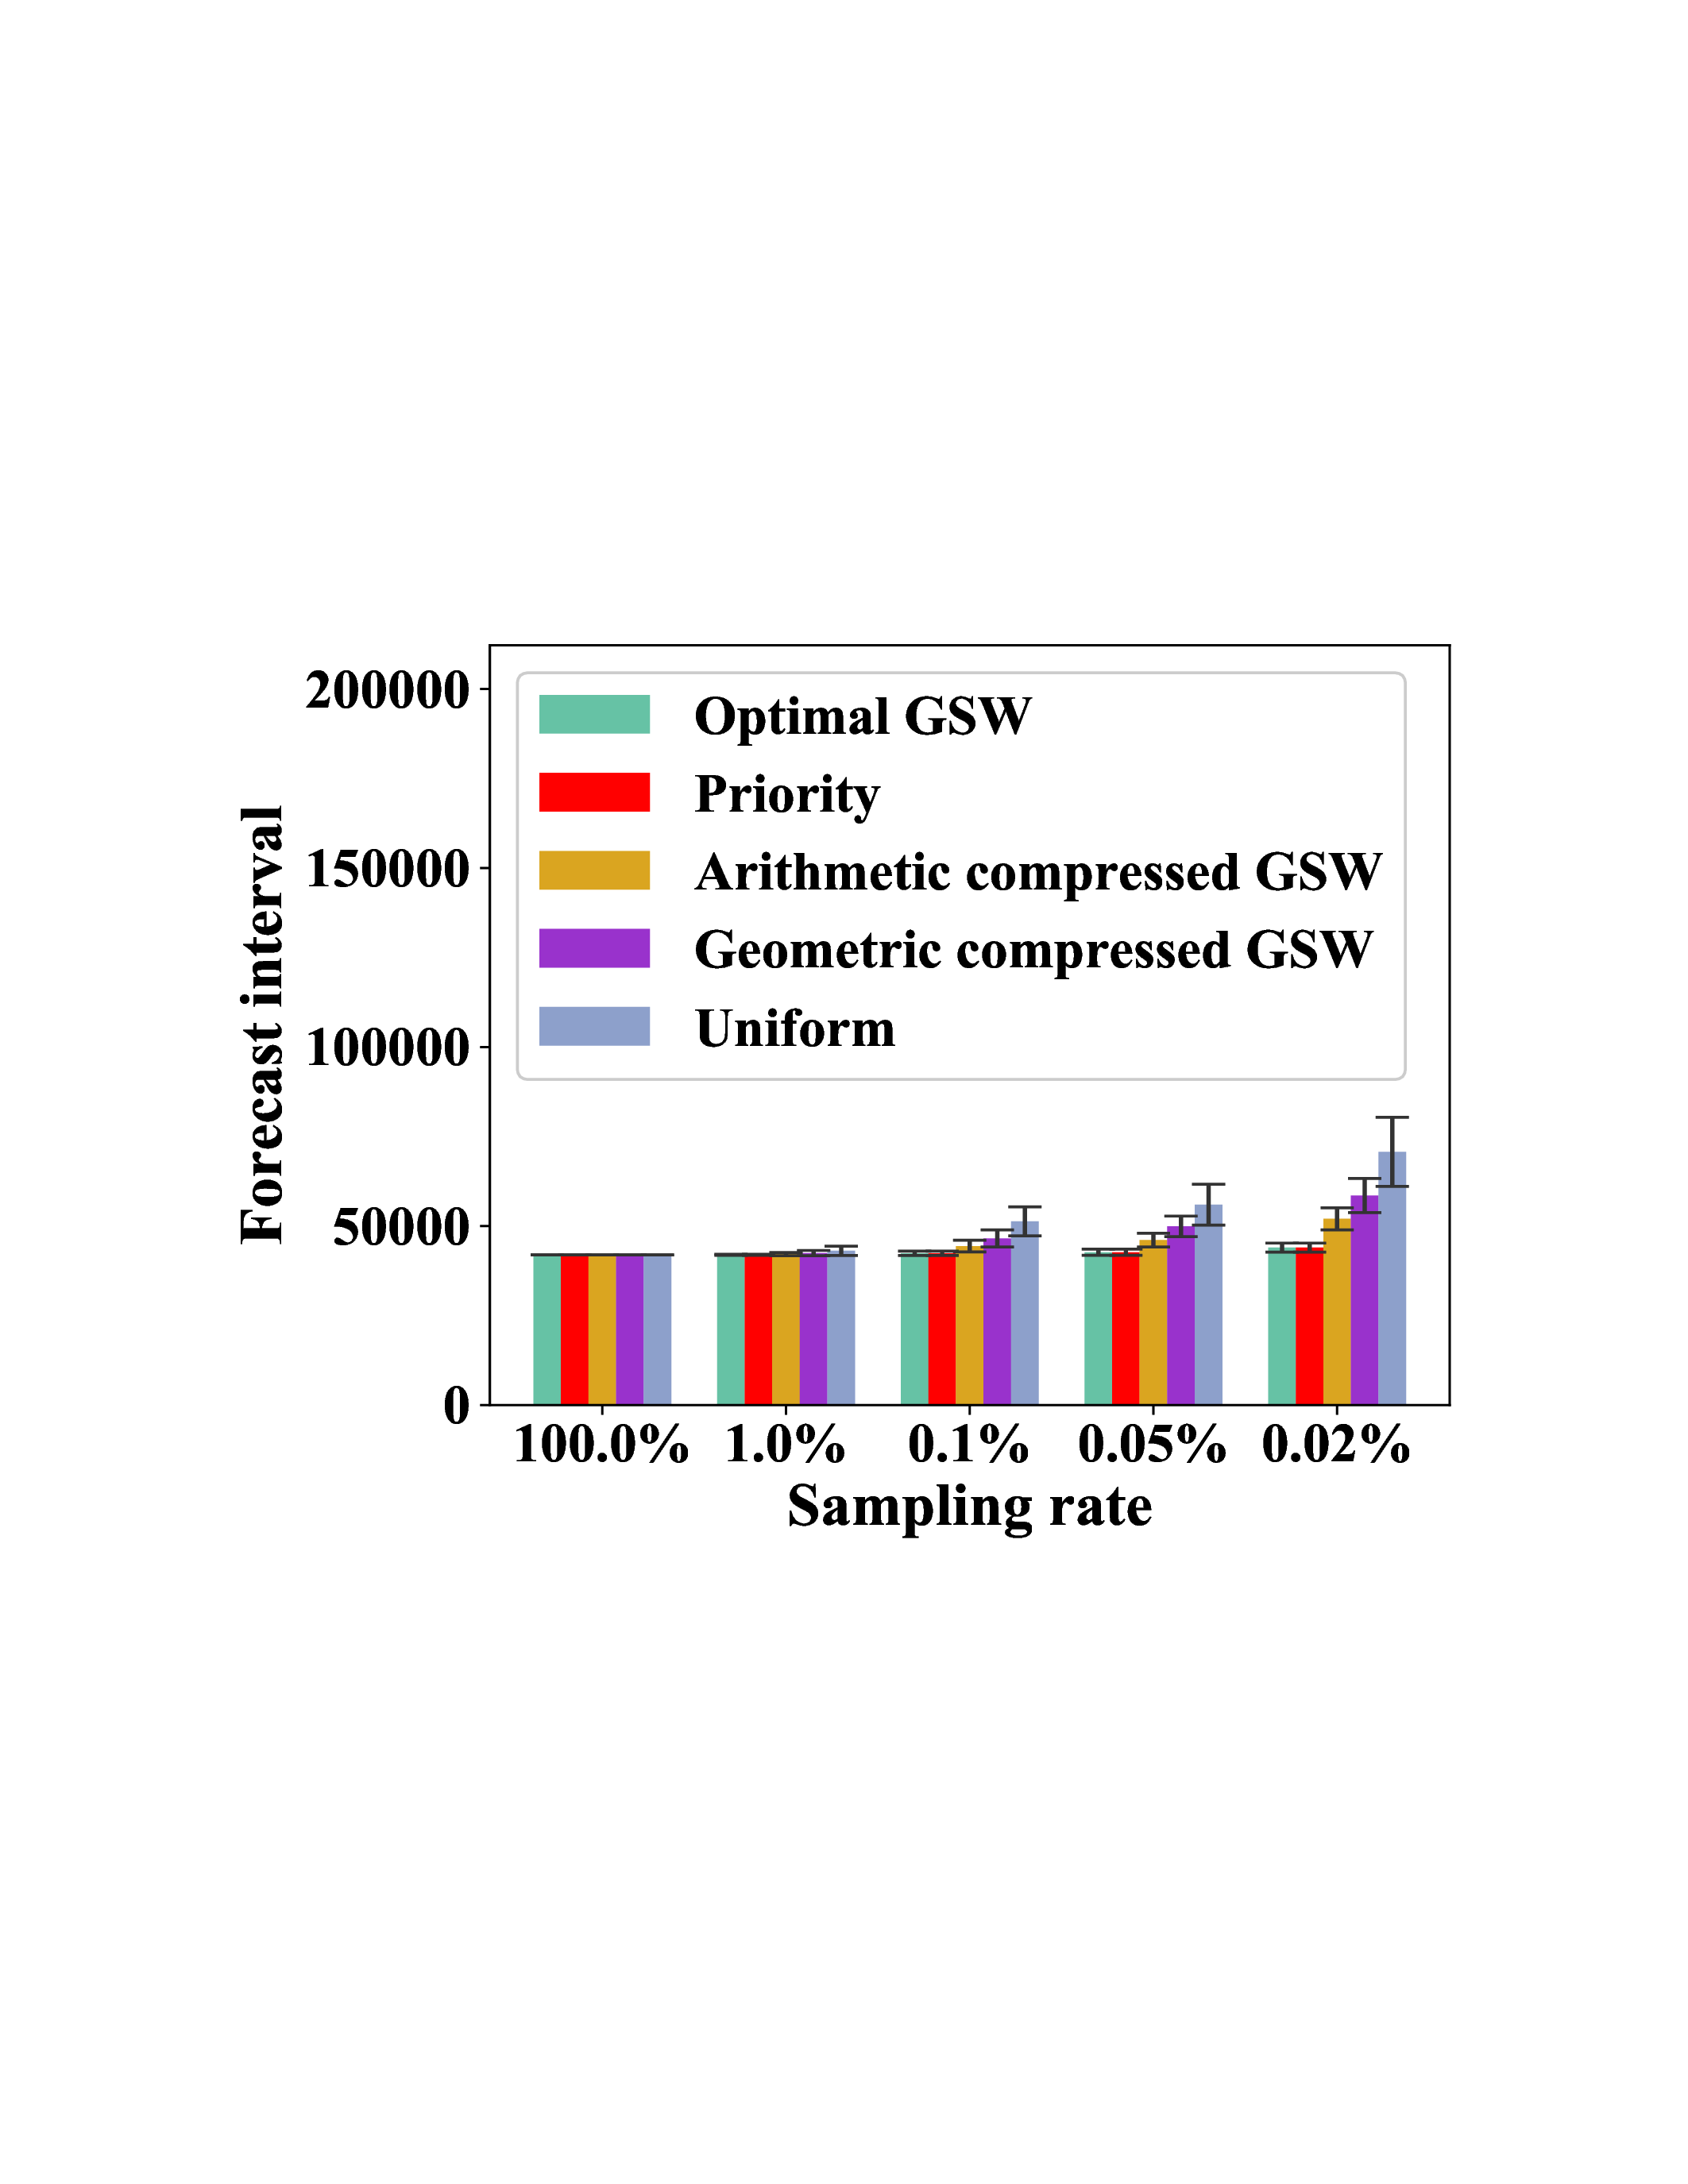}
% \label{fig:side:a}
\end{minipage}
}
\subfigure[Selectivity 1\%]{
\begin{minipage}[t]{0.33\linewidth}
\centering
\includegraphics[width=2.2in, height=2.0in]{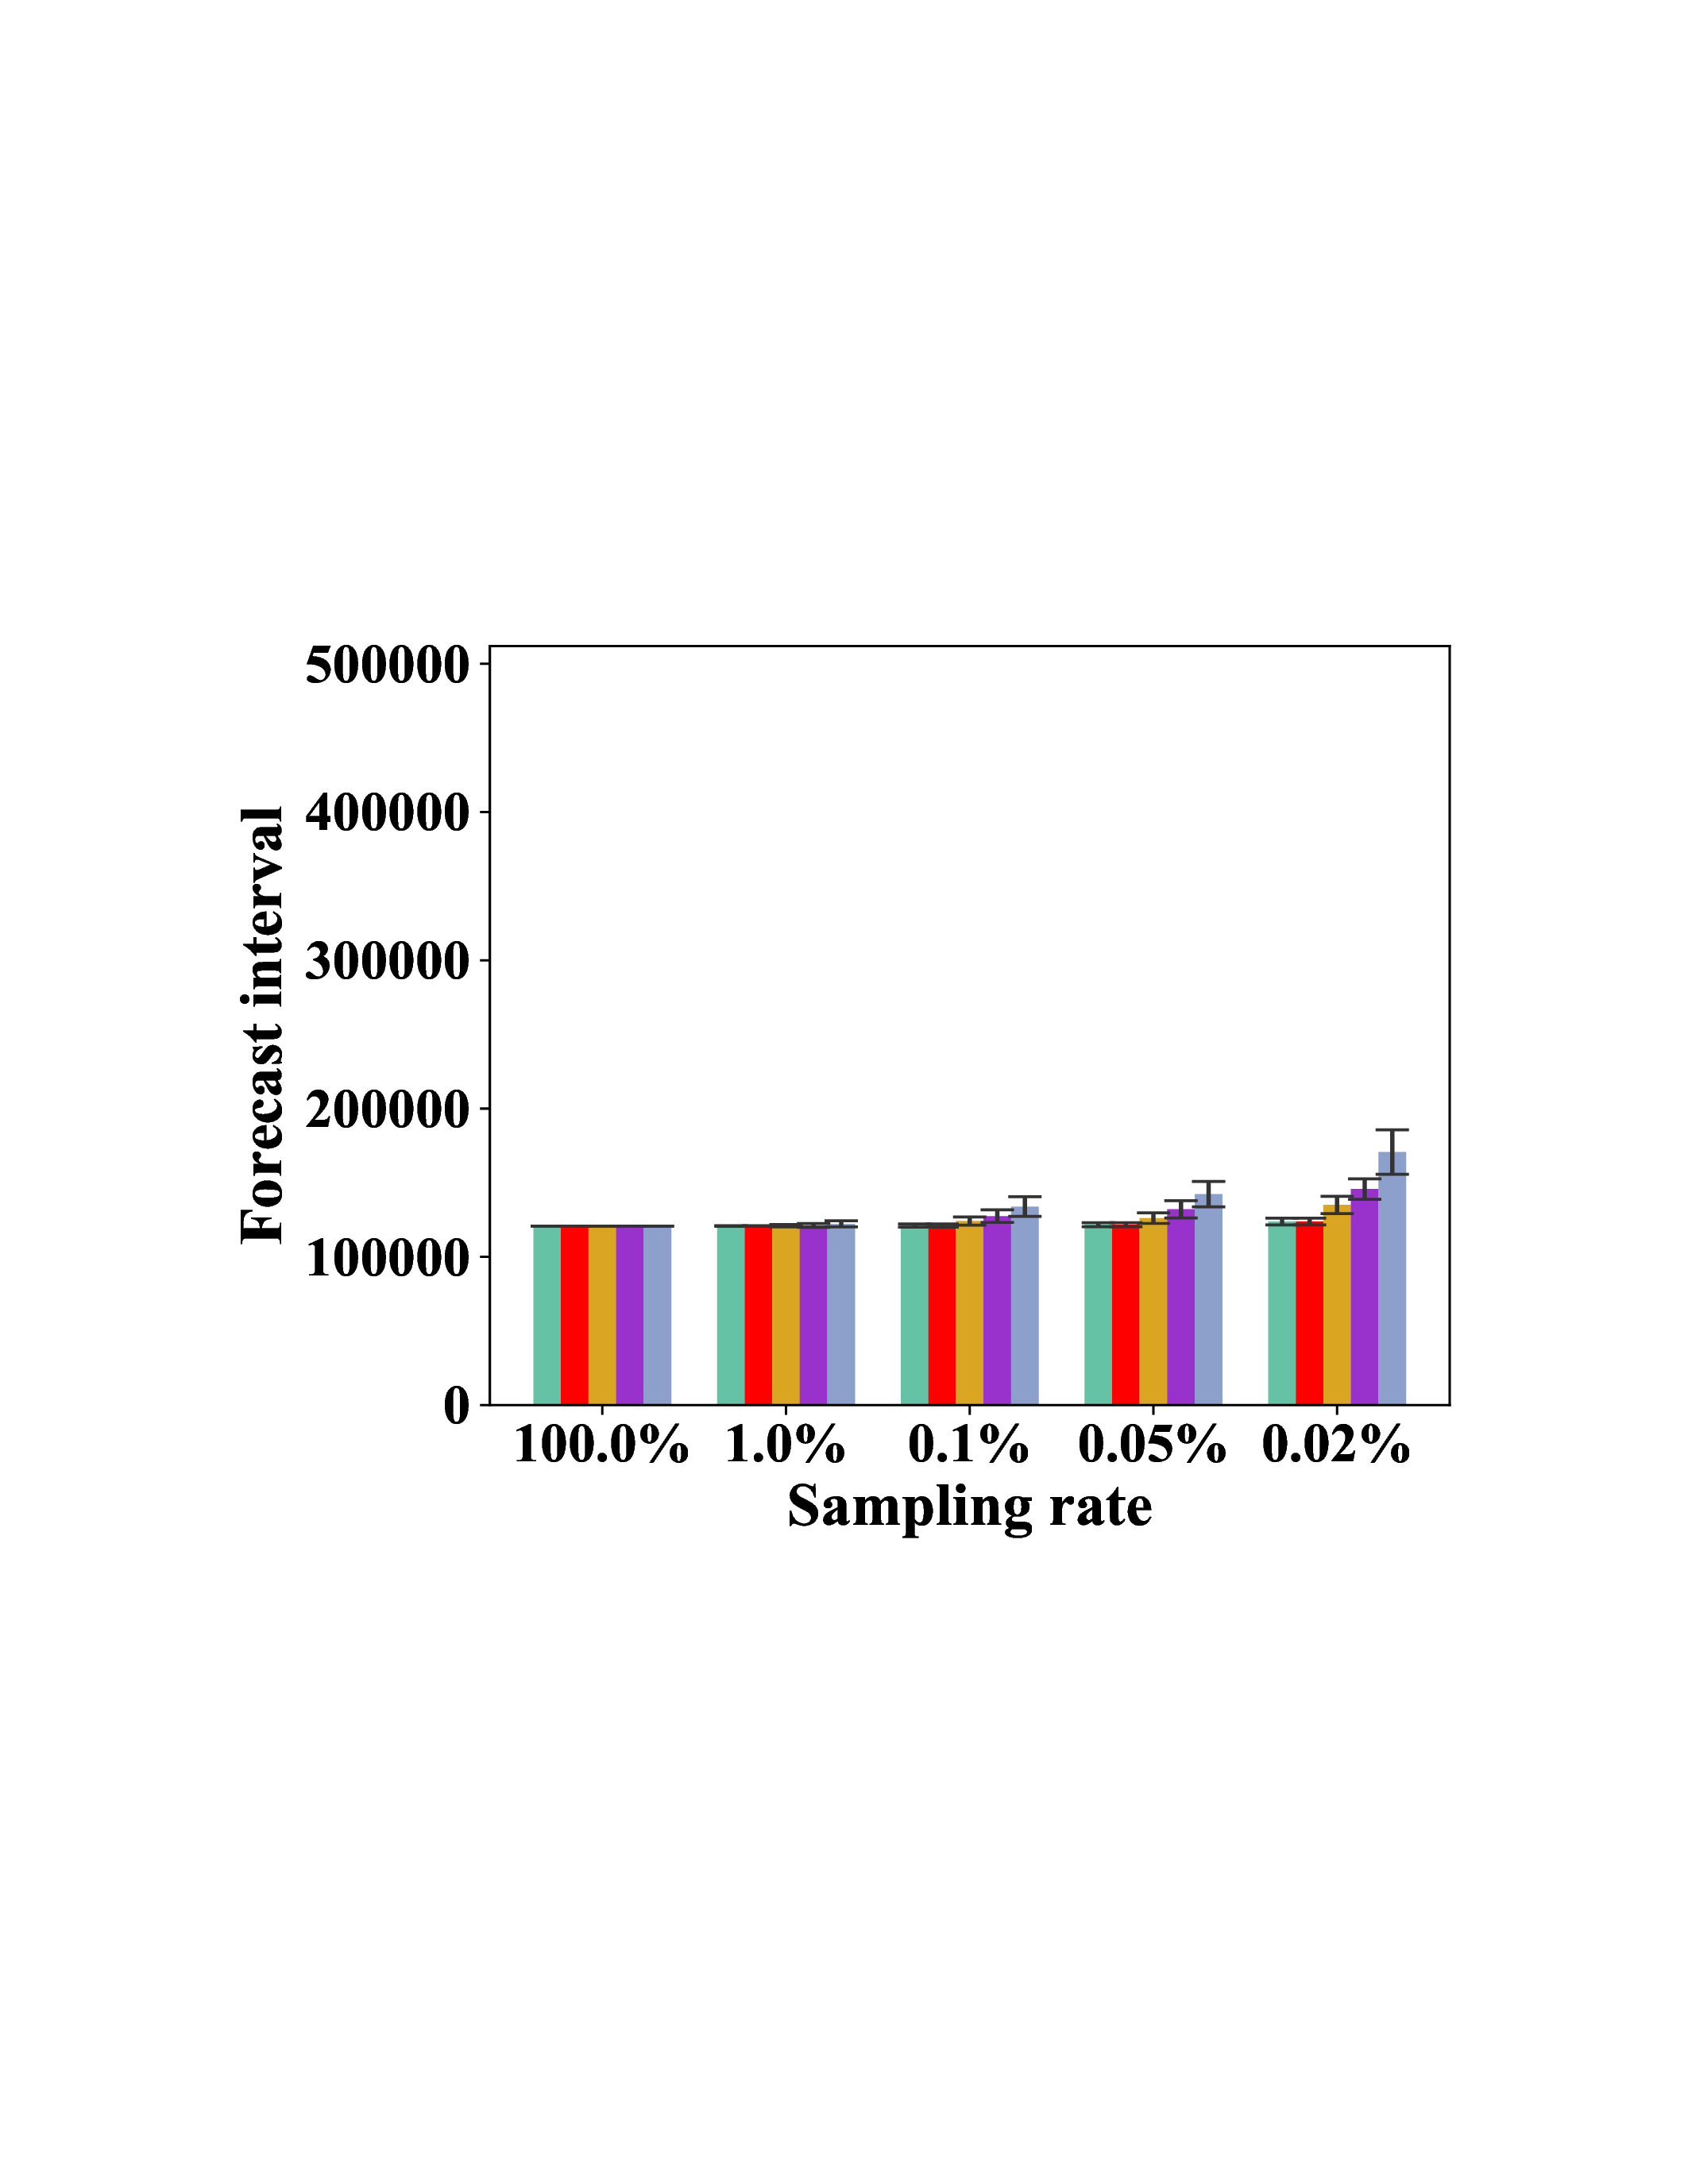}
\end{minipage}
}
\subfigure[Selectivity 5\%]{
\begin{minipage}[t]{0.33\linewidth}
\centering
\includegraphics[width=2.2in, height=2.0in]{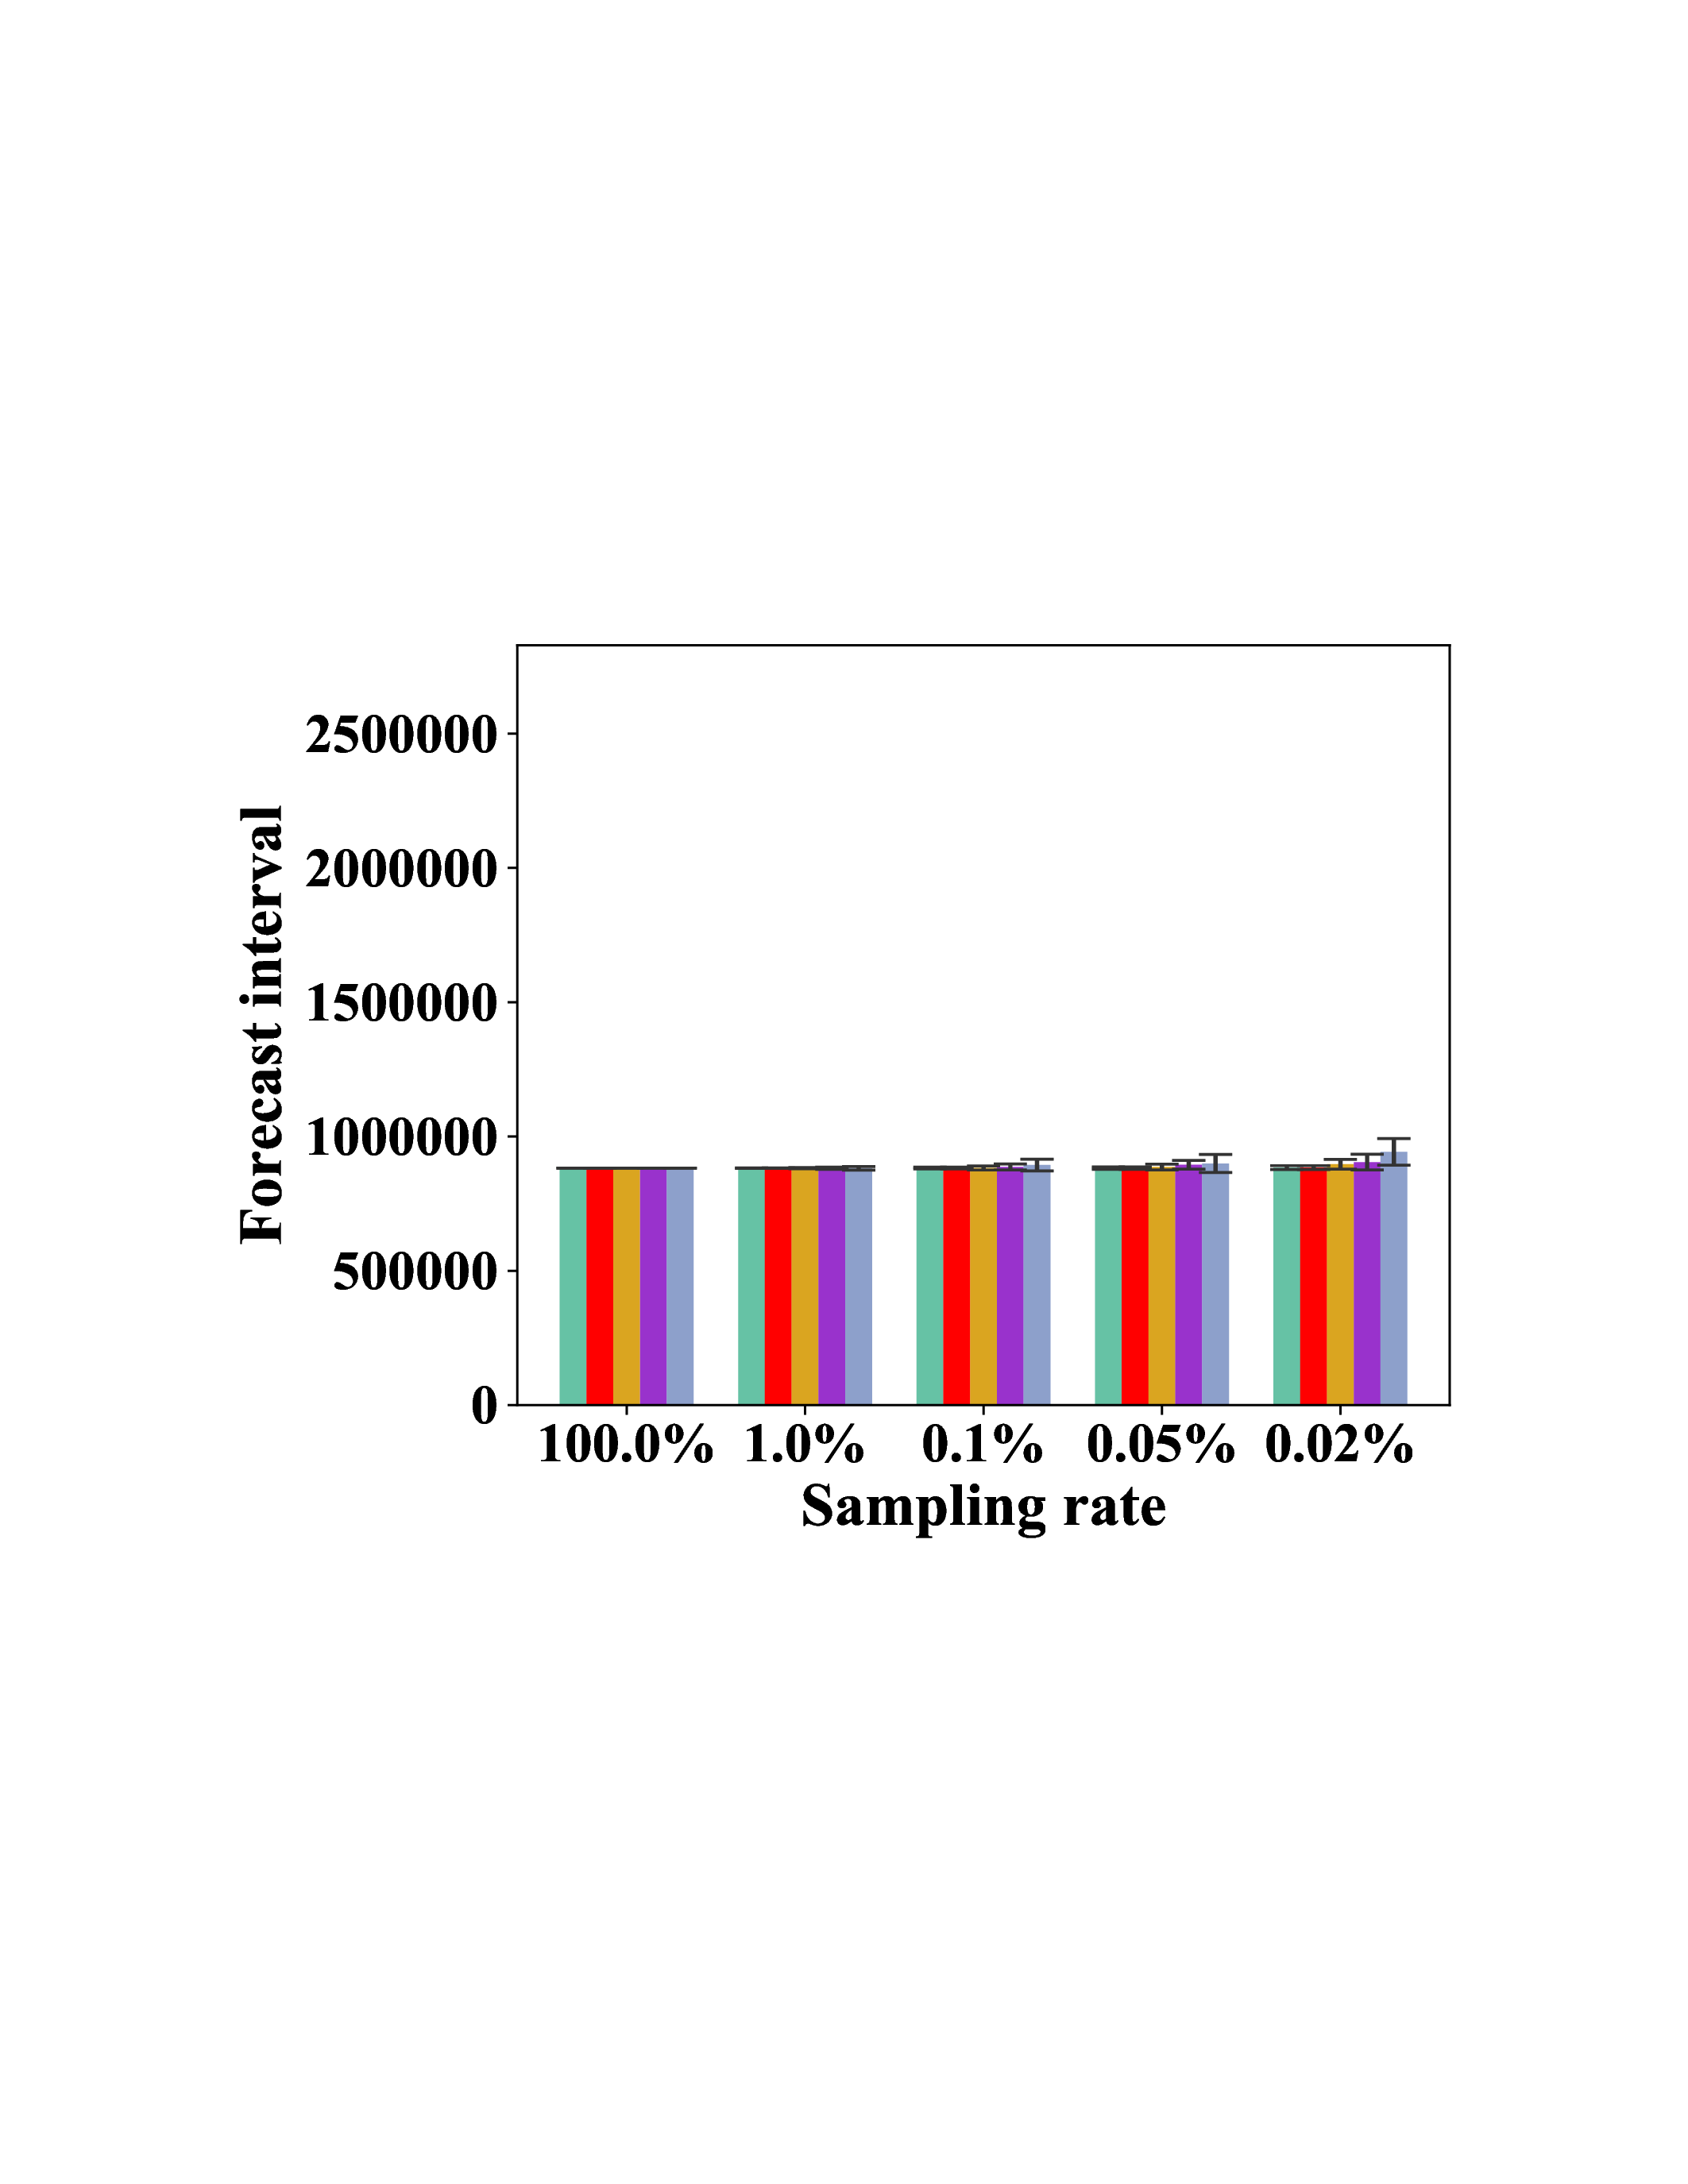}
\end{minipage}
}
\caption{ARIMA prediction interval at different selectivity on Cart via different sampling methods}
% \label{AQP and ARIMA Performance}
\end{figure*}

%============================

%========================CASE===================================
%==============Selectivity 0.5% on Impression Case===============

\begin{figure*}[hb]
\subfigure[Sampling rate 0.02\%]{
\begin{minipage}[t]{0.33\linewidth}
\centering
\includegraphics[width=2.2in, height=2.0in]{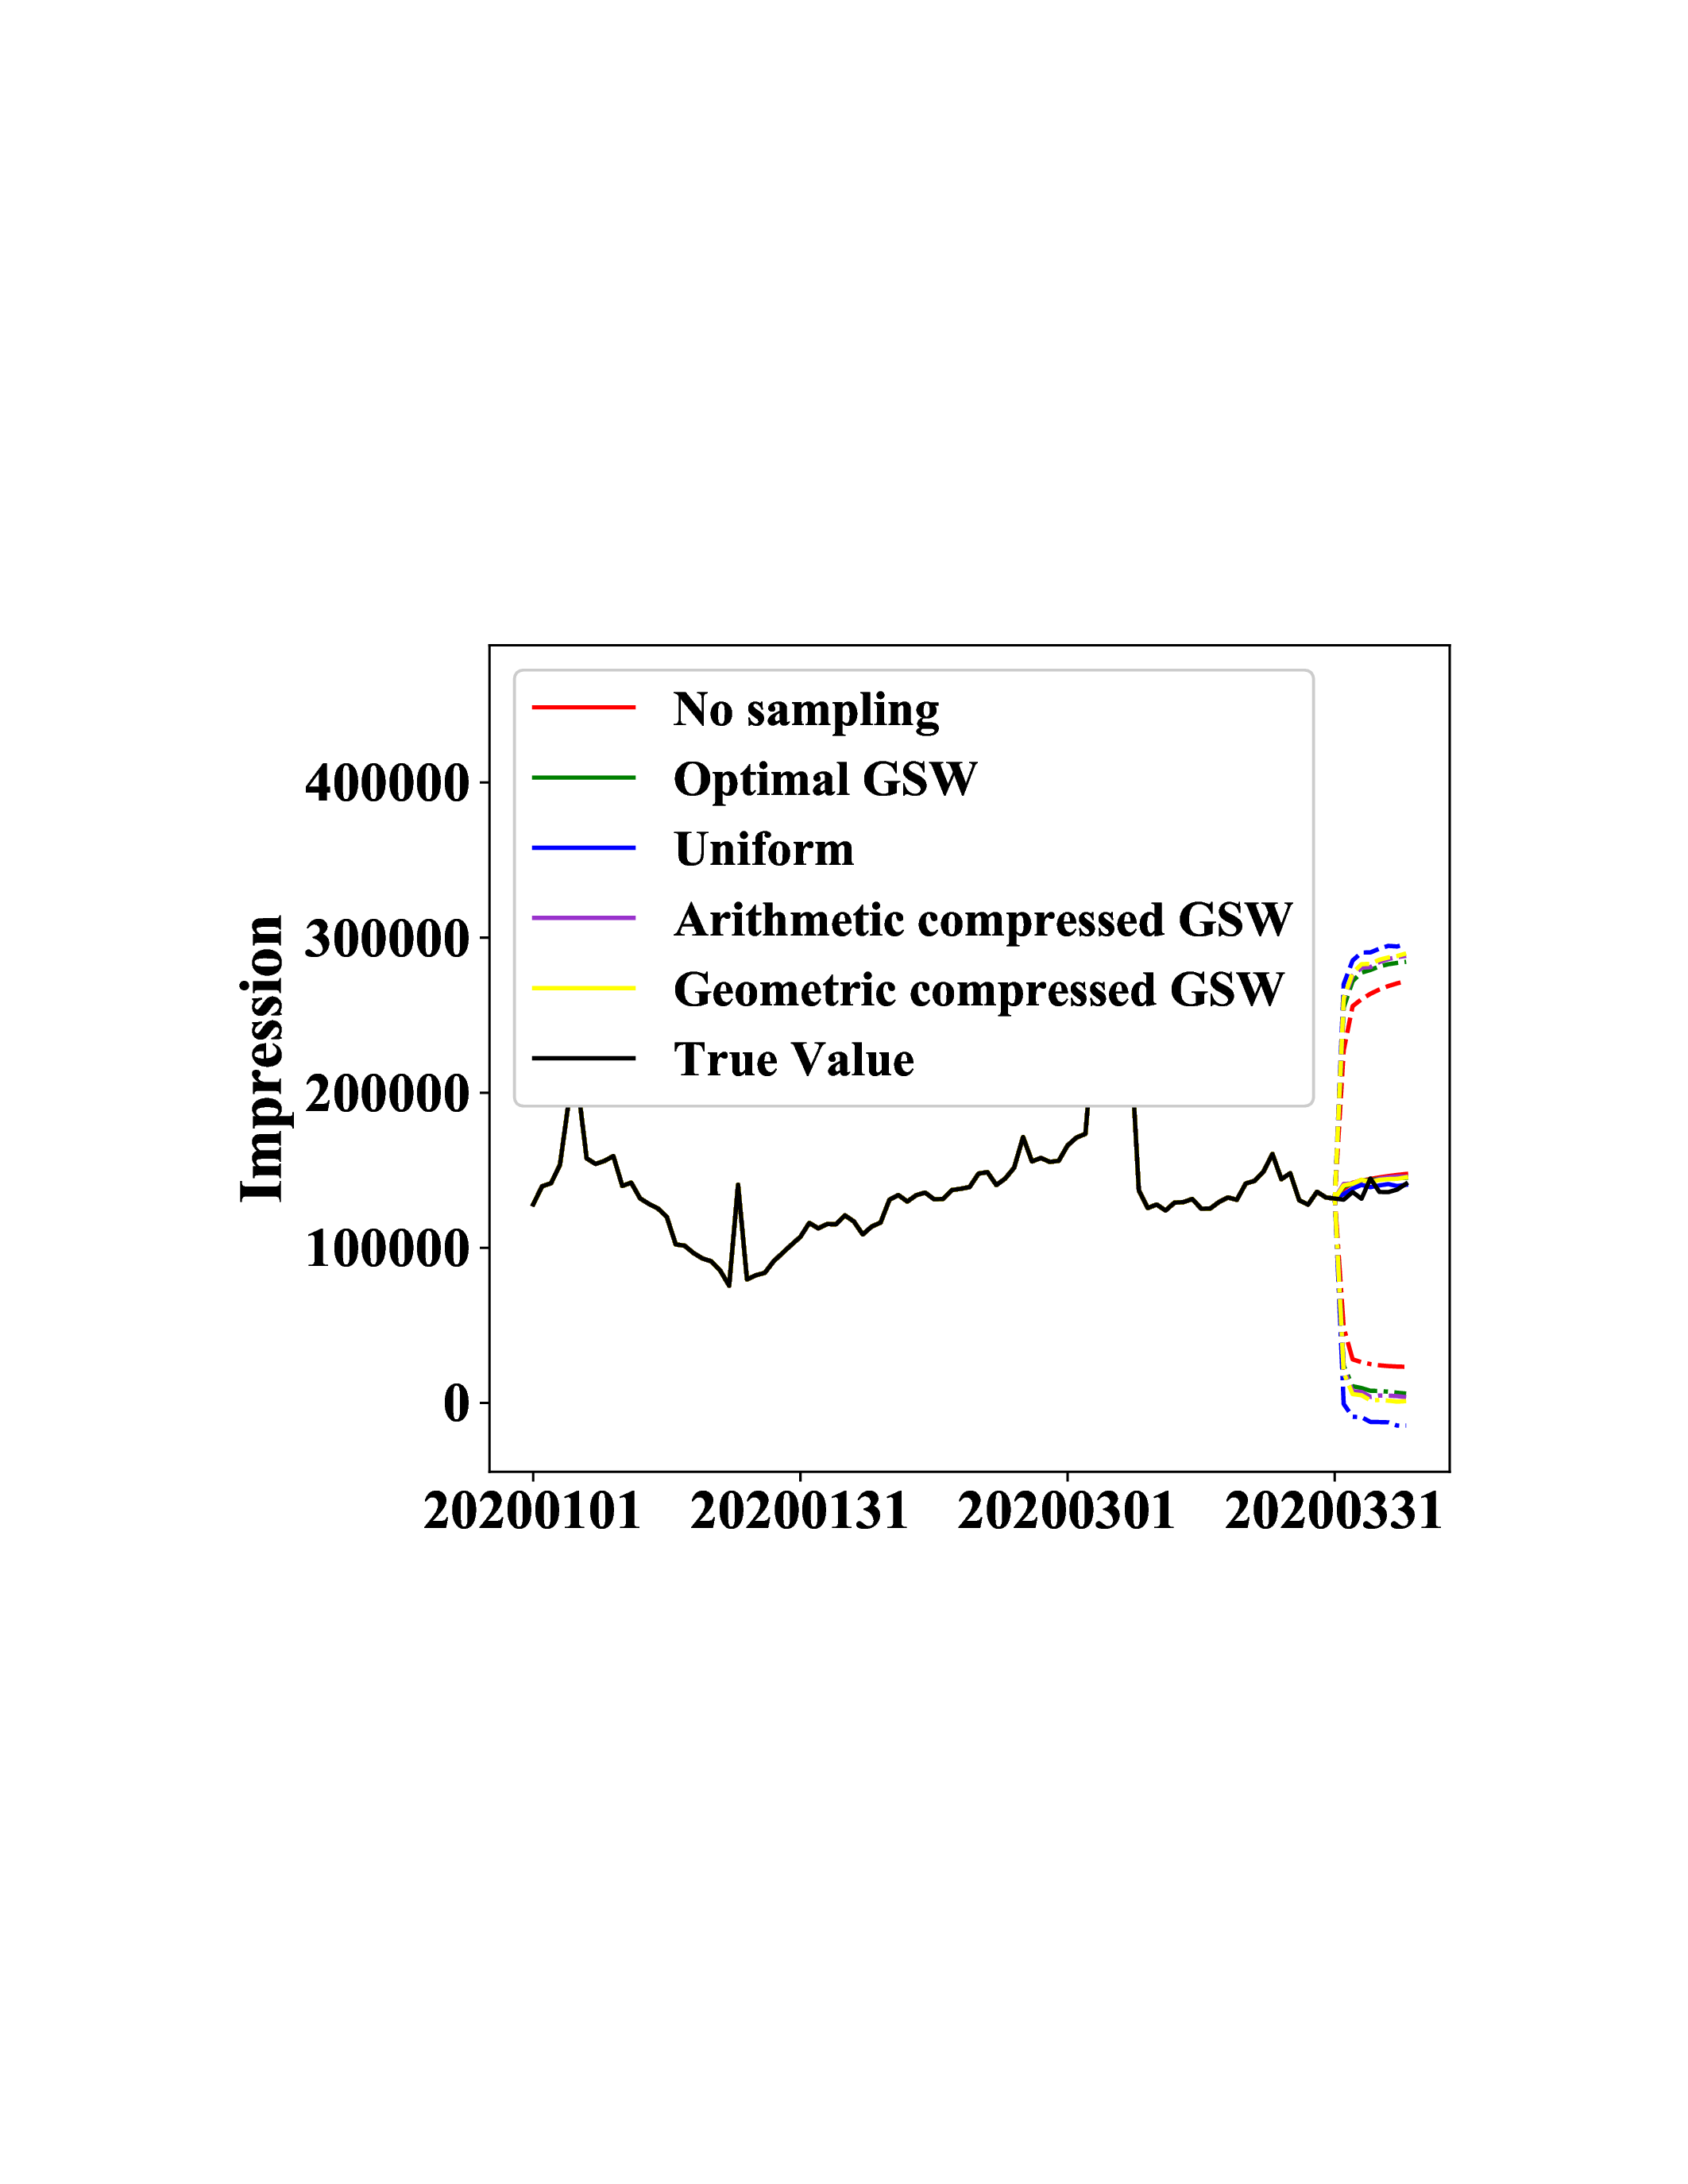}
% \label{fig:side:a}
\end{minipage}
}
\subfigure[Sampling rate 0.1\%]{
\begin{minipage}[t]{0.33\linewidth}
\centering
\includegraphics[width=2.2in, height=2.0in]{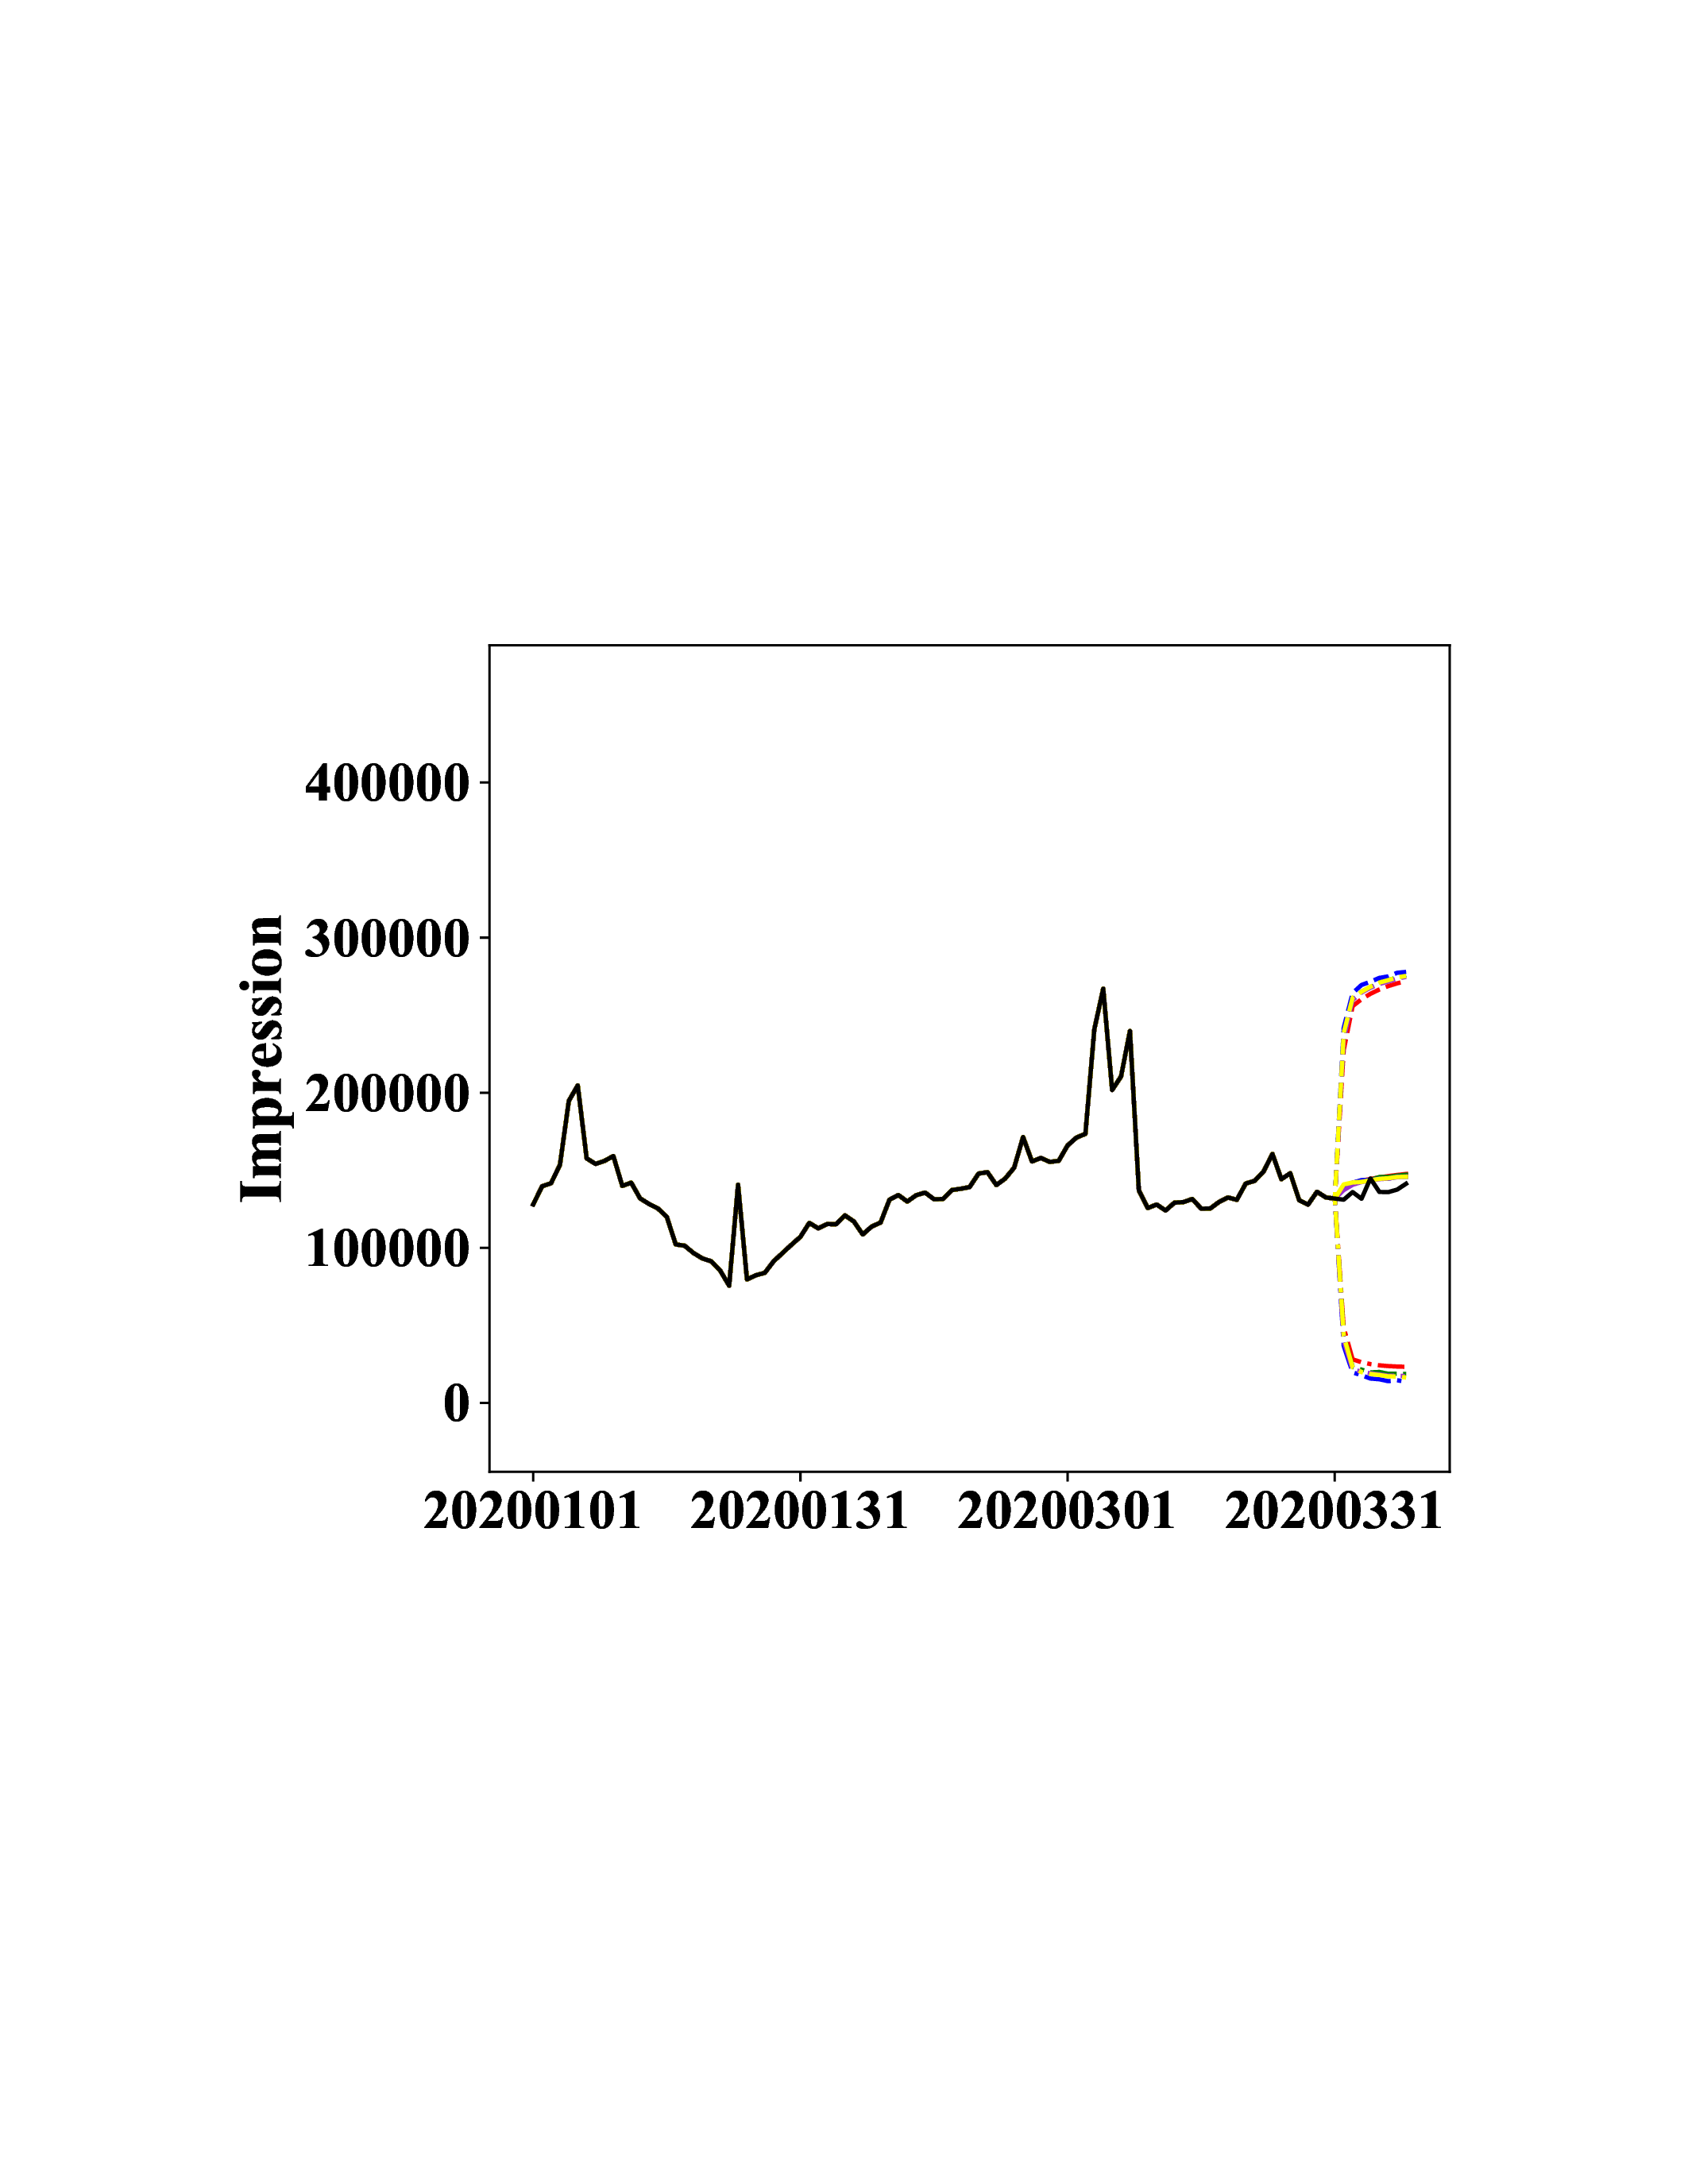}
\end{minipage}
}
\subfigure[Sampling rate 1\%]{
\begin{minipage}[t]{0.33\linewidth}
\centering
\includegraphics[width=2.2in, height=2.0in]{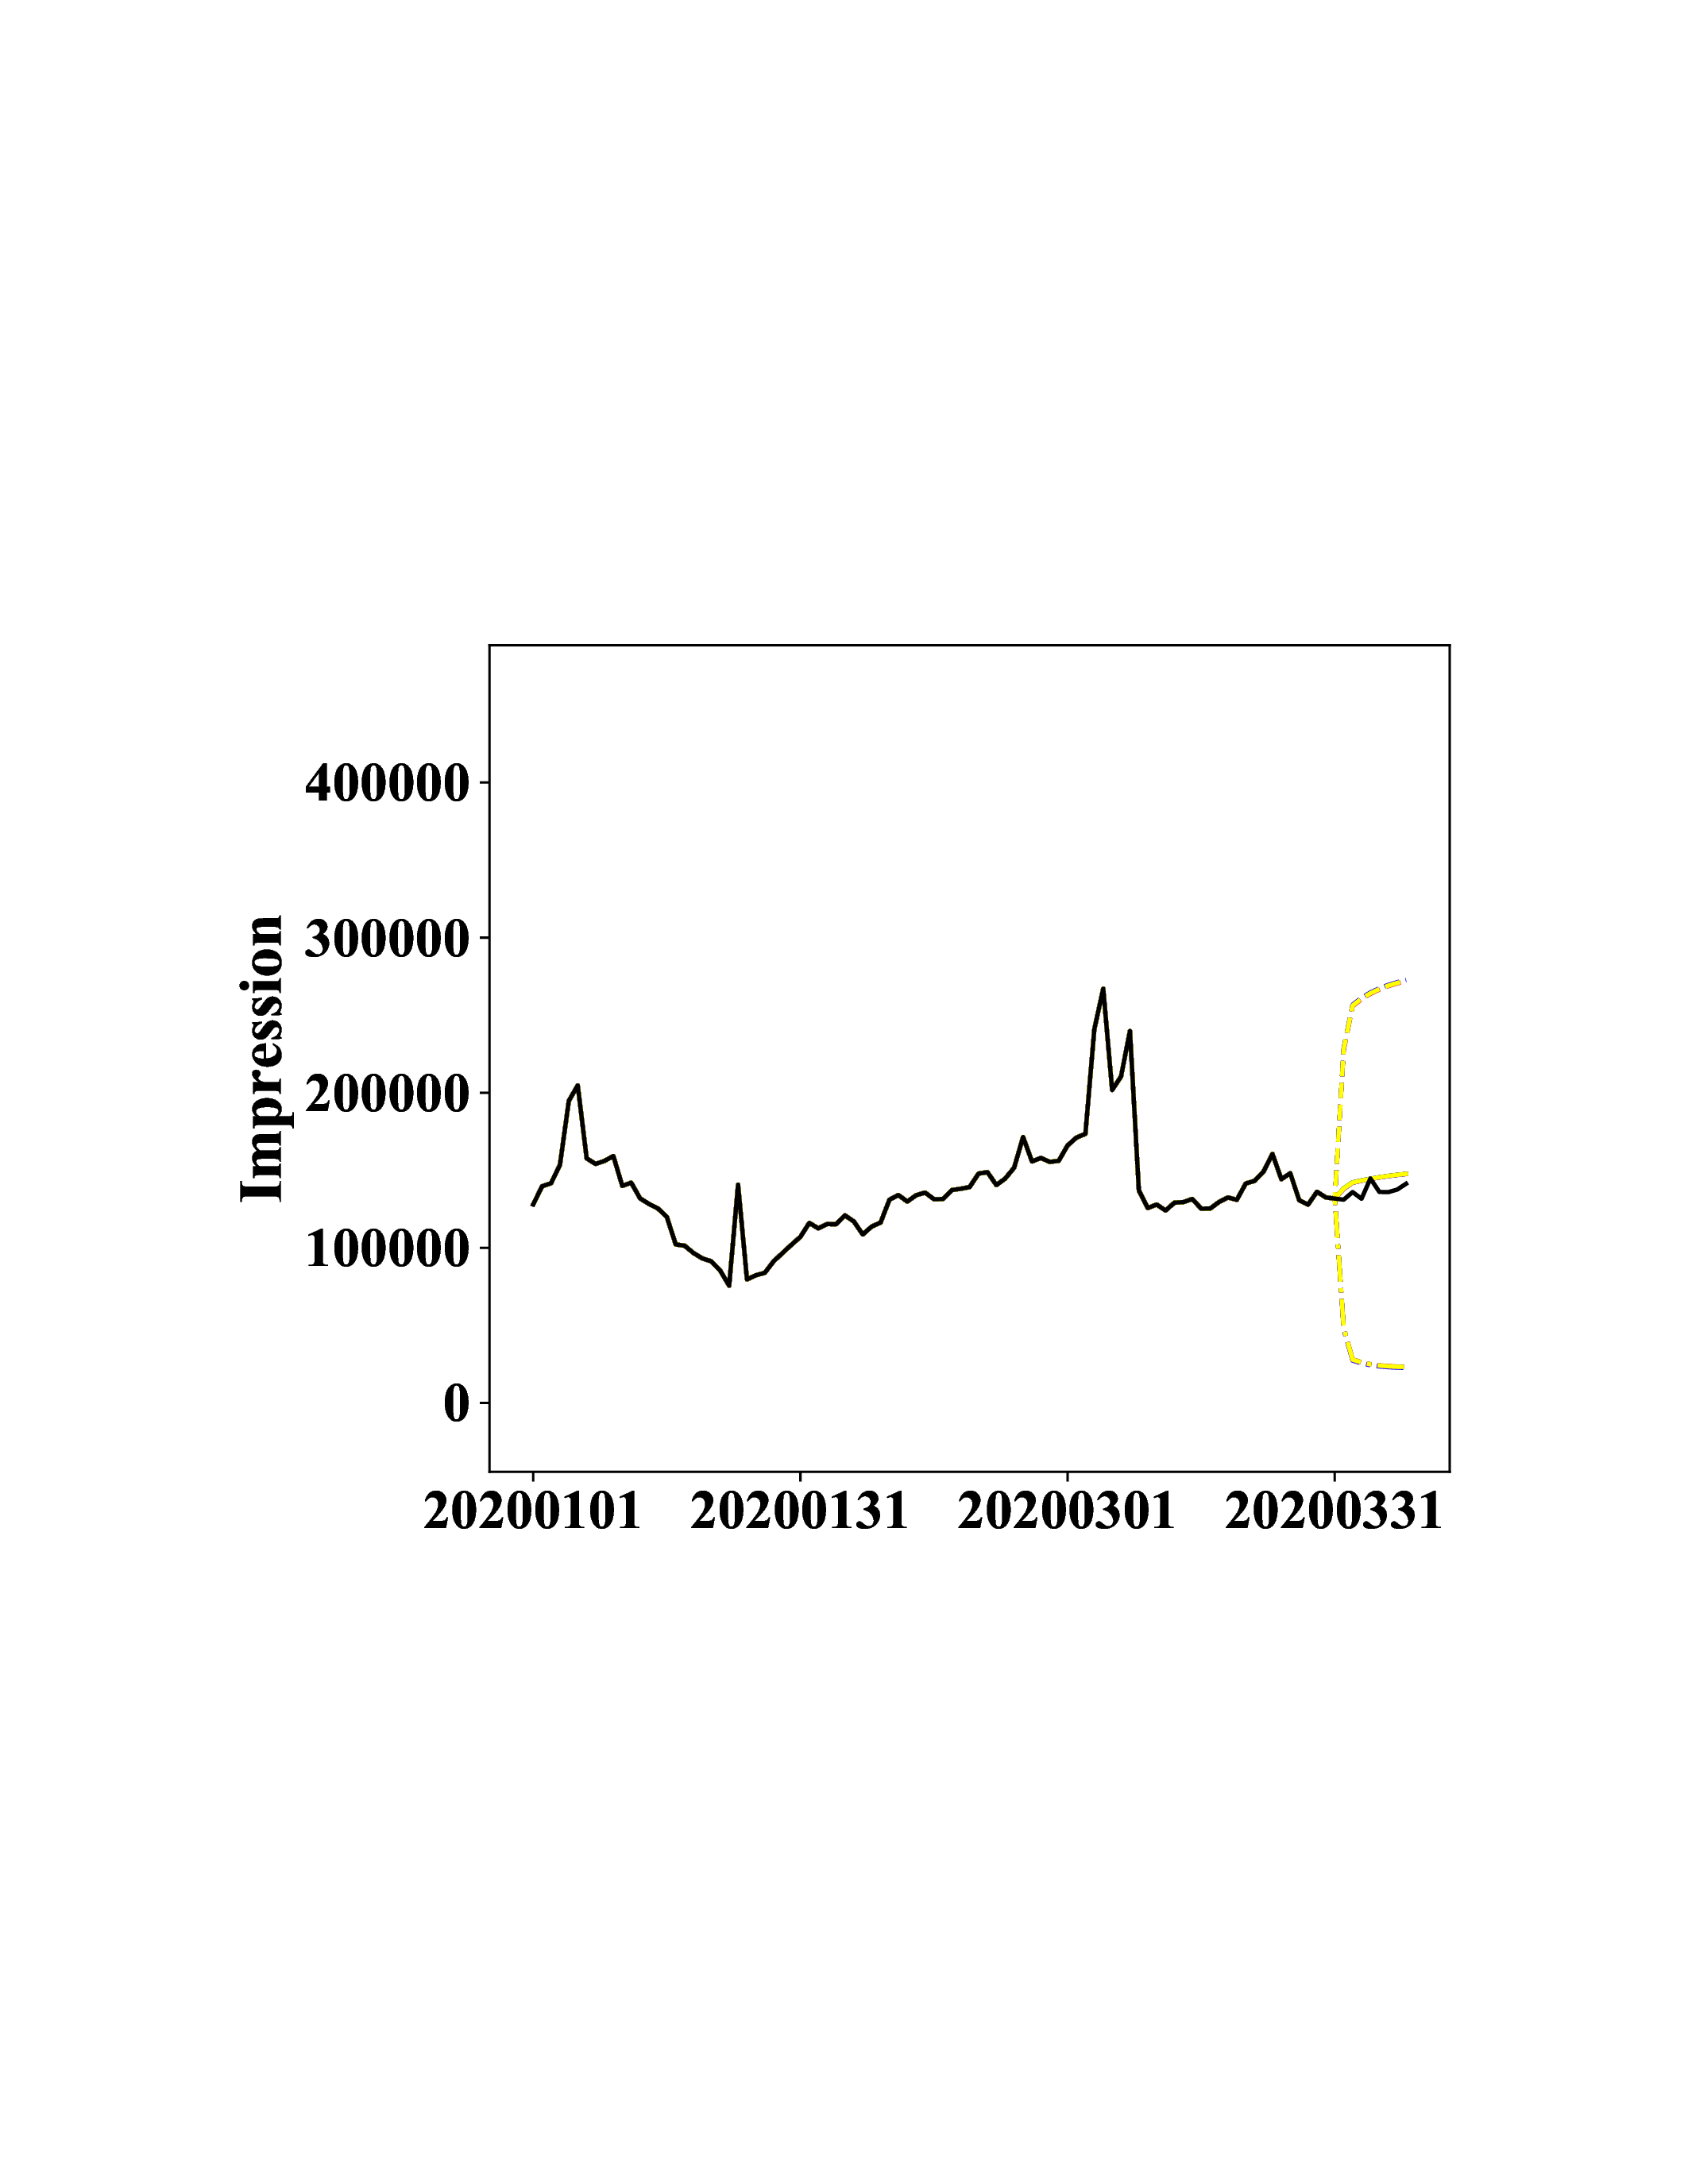}
\end{minipage}
}
\caption{ARIMA average predict error and interval at selectivity 0.5\% (why not 0.5\%? -- inconsistent with 0.5\% above) on impression via different sampling methods (so the predictions in different sampling methods are almost the same?)}
% \label{AQP and ARIMA Performance}
\end{figure*}
%---------end-------------

%==============Selectivity 5% on Impression Case===============

\begin{figure*}[hb]
\subfigure[Sampling rate 0.02\%]{
\begin{minipage}[t]{0.33\linewidth}
\centering
\includegraphics[width=2.2in, height=2.0in]{fig-new/vldb-fig9-fix-sample-9248224-5000-500w-pv-case.eps}
% \label{fig:side:a}
\end{minipage}
}
\subfigure[Sampling rate 0.1\%]{
\begin{minipage}[t]{0.33\linewidth}
\centering
\includegraphics[width=2.2in, height=2.0in]{fig-new/vldb-fig9-fix-sample-9248224-1000-500w-pv-case.eps}
\end{minipage}
}
\subfigure[Sampling rate 1\%]{
\begin{minipage}[t]{0.33\linewidth}
\centering
\includegraphics[width=2.2in, height=2.0in]{fig-new/vldb-fig9-fix-sample-9248224-100-500w-pv-case.eps}
\end{minipage}
}
\caption{ARIMA average predict error and interval at selectivity 5\% (why not 0.5\%? -- inconsistent with 0.5\% above) on impression via different sampling methods (so the predictions in different sampling methods are almost the same?)}
% \label{AQP and ARIMA Performance}
\end{figure*}
%---------end-------------

%==============Selectivity 0.5% on Click Case===============

\begin{figure*}[hb]
\subfigure[Sampling rate 0.02\%]{
\begin{minipage}[t]{0.33\linewidth}
\centering
\includegraphics[width=2.2in, height=2.0in]{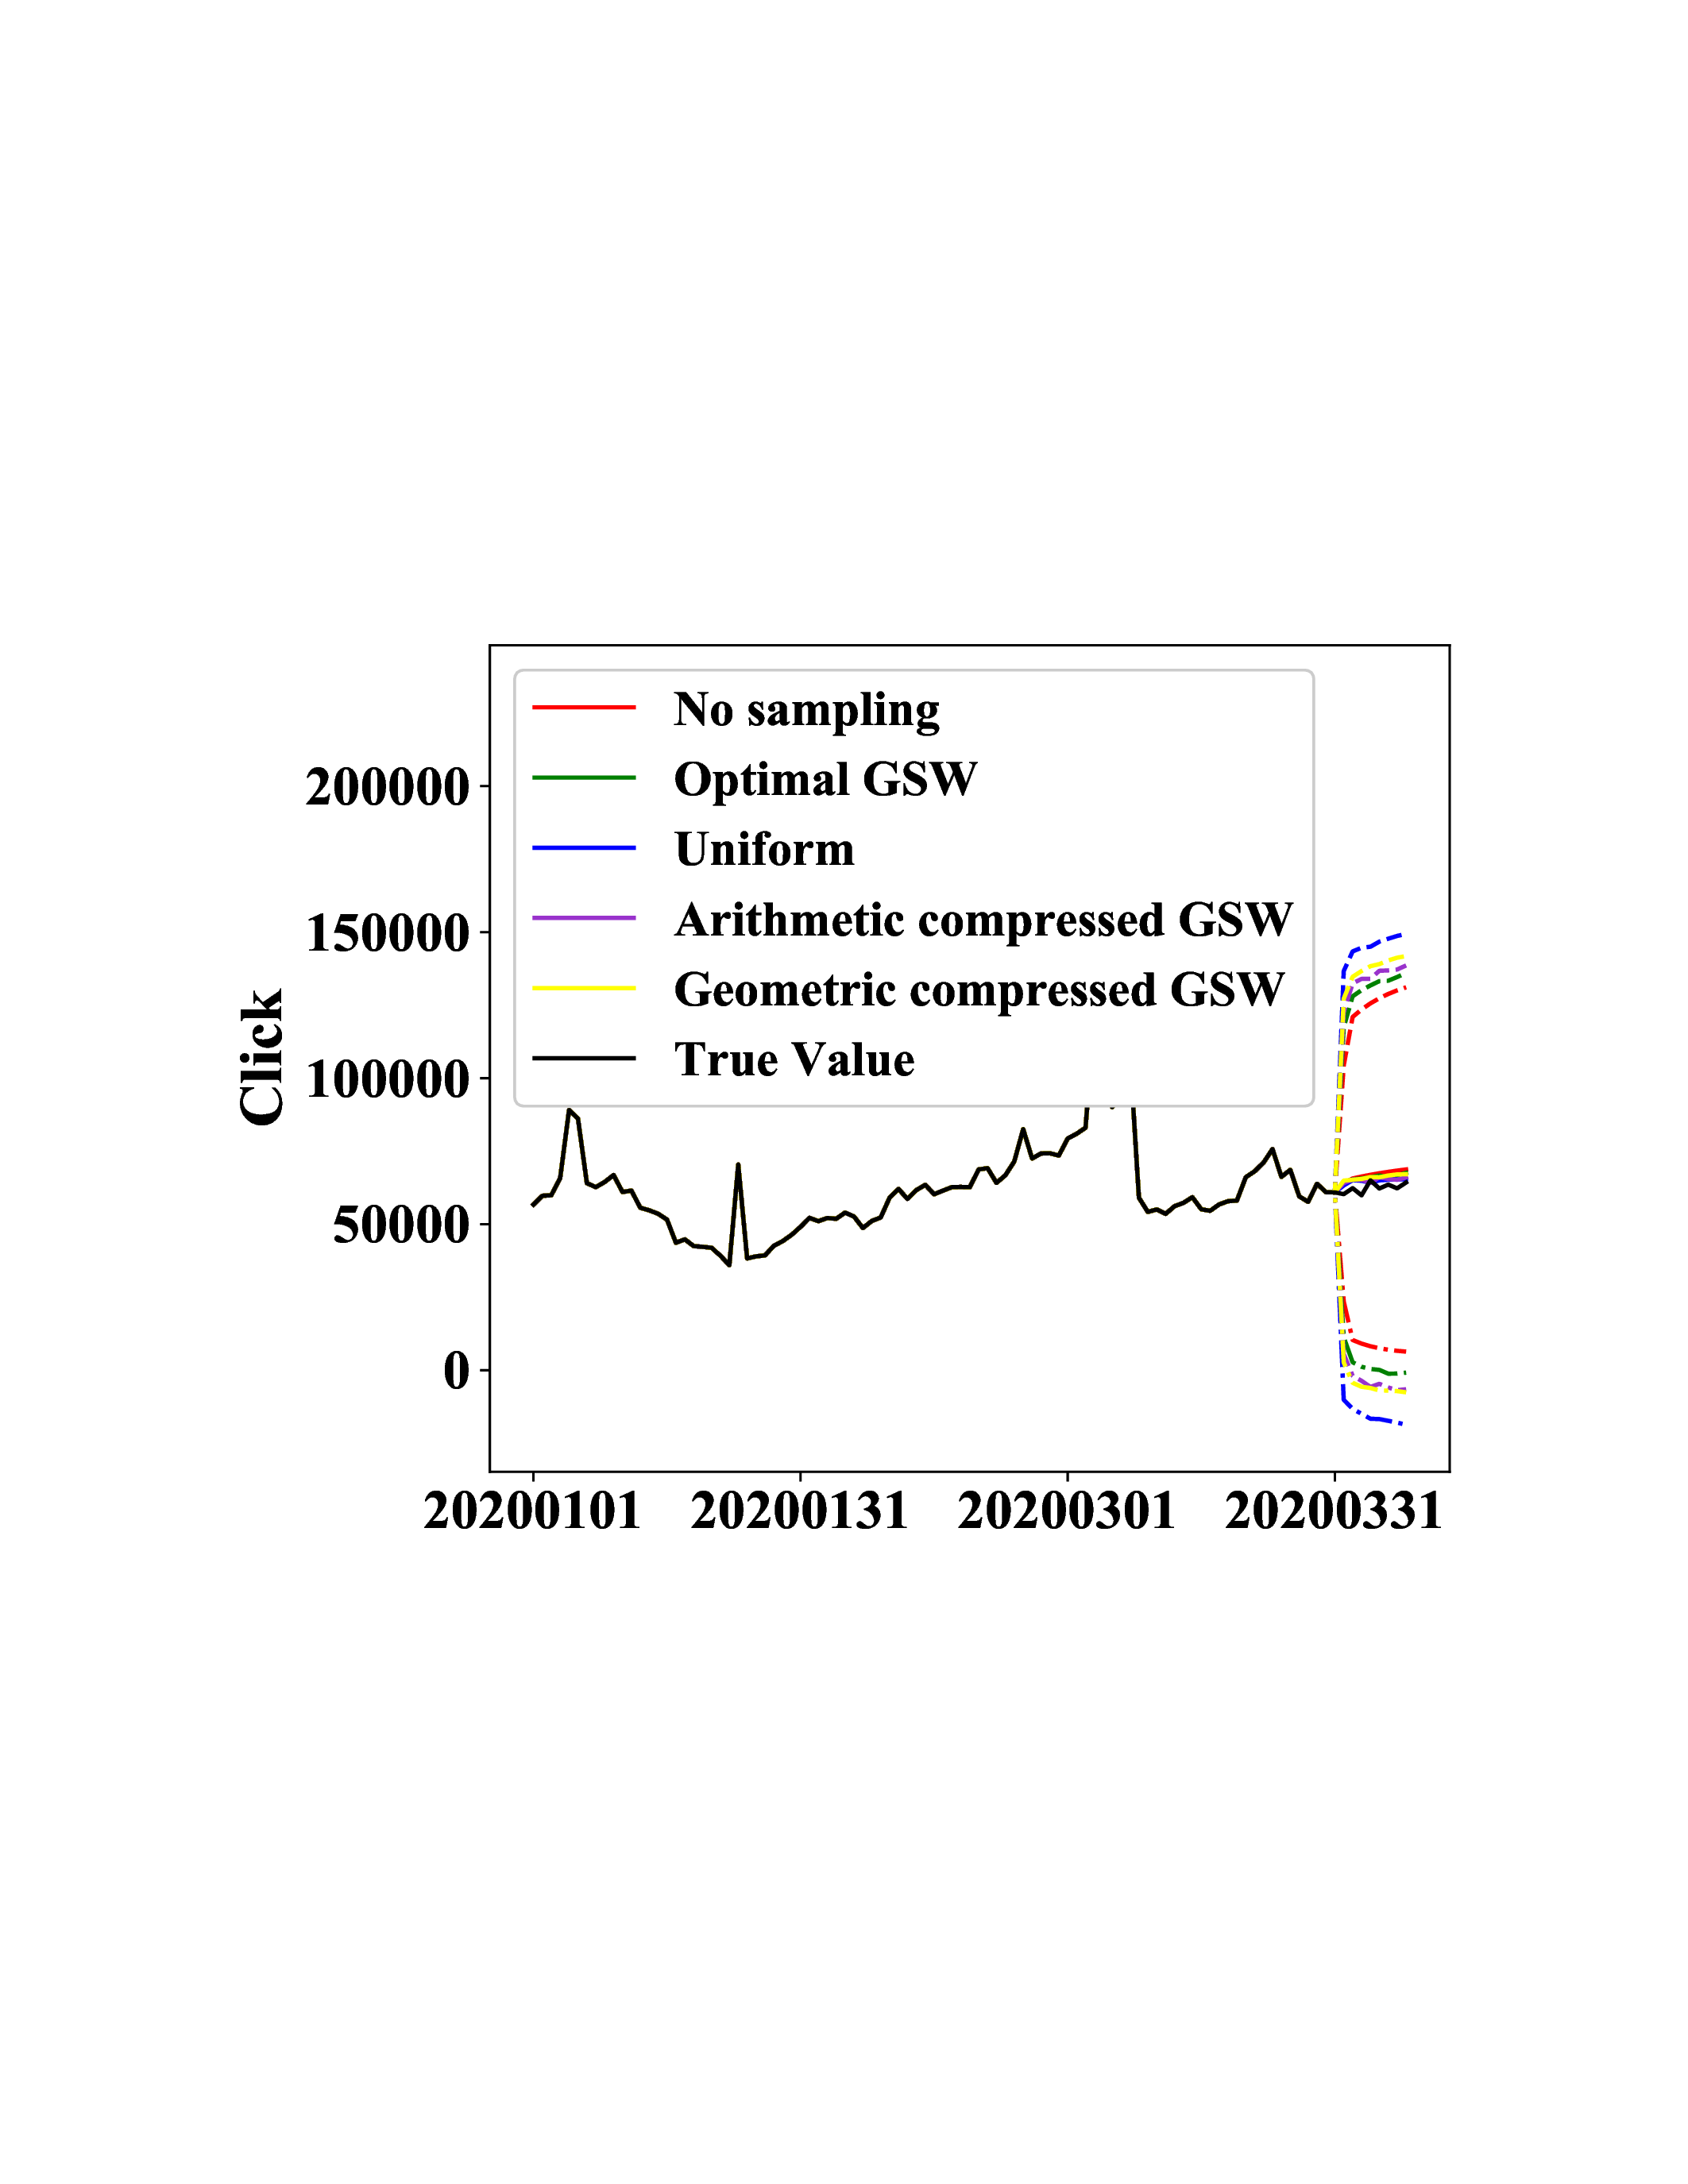}
% \label{fig:side:a}
\end{minipage}
}
\subfigure[Sampling rate 0.1\%]{
\begin{minipage}[t]{0.33\linewidth}
\centering
\includegraphics[width=2.2in, height=2.0in]{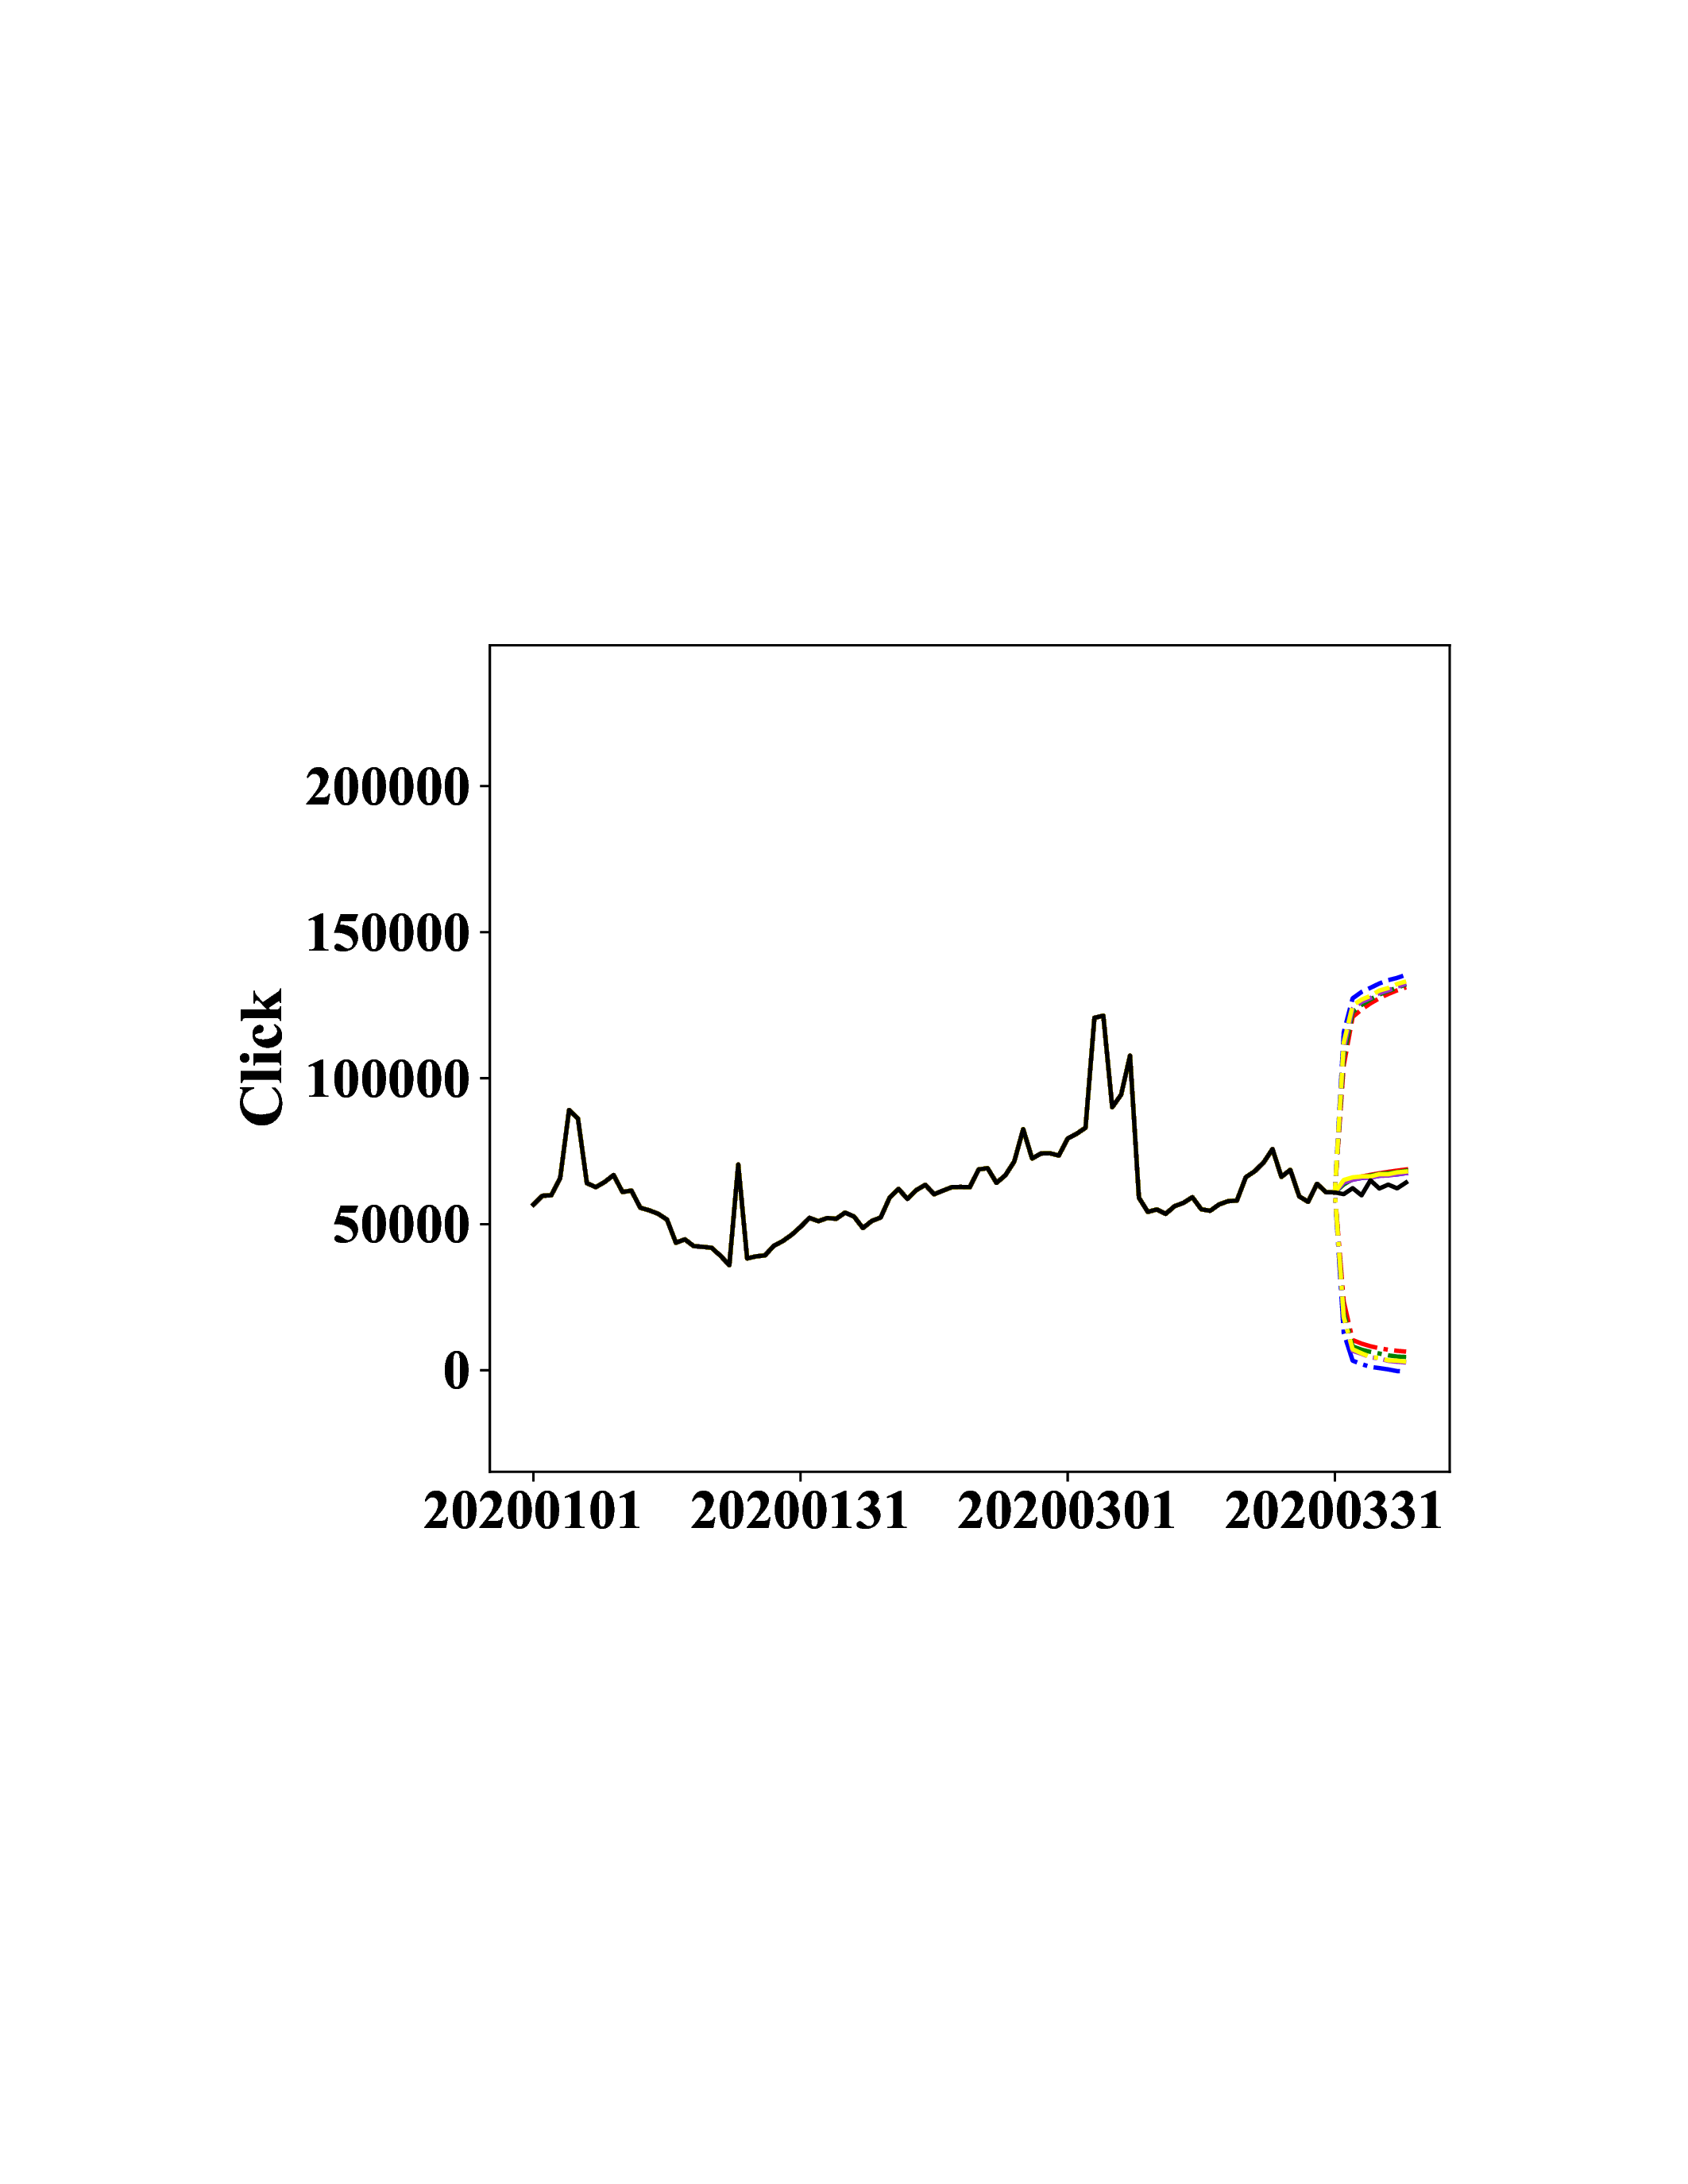}
\end{minipage}
}
\subfigure[Sampling rate 1\%]{
\begin{minipage}[t]{0.33\linewidth}
\centering
\includegraphics[width=2.2in, height=2.0in]{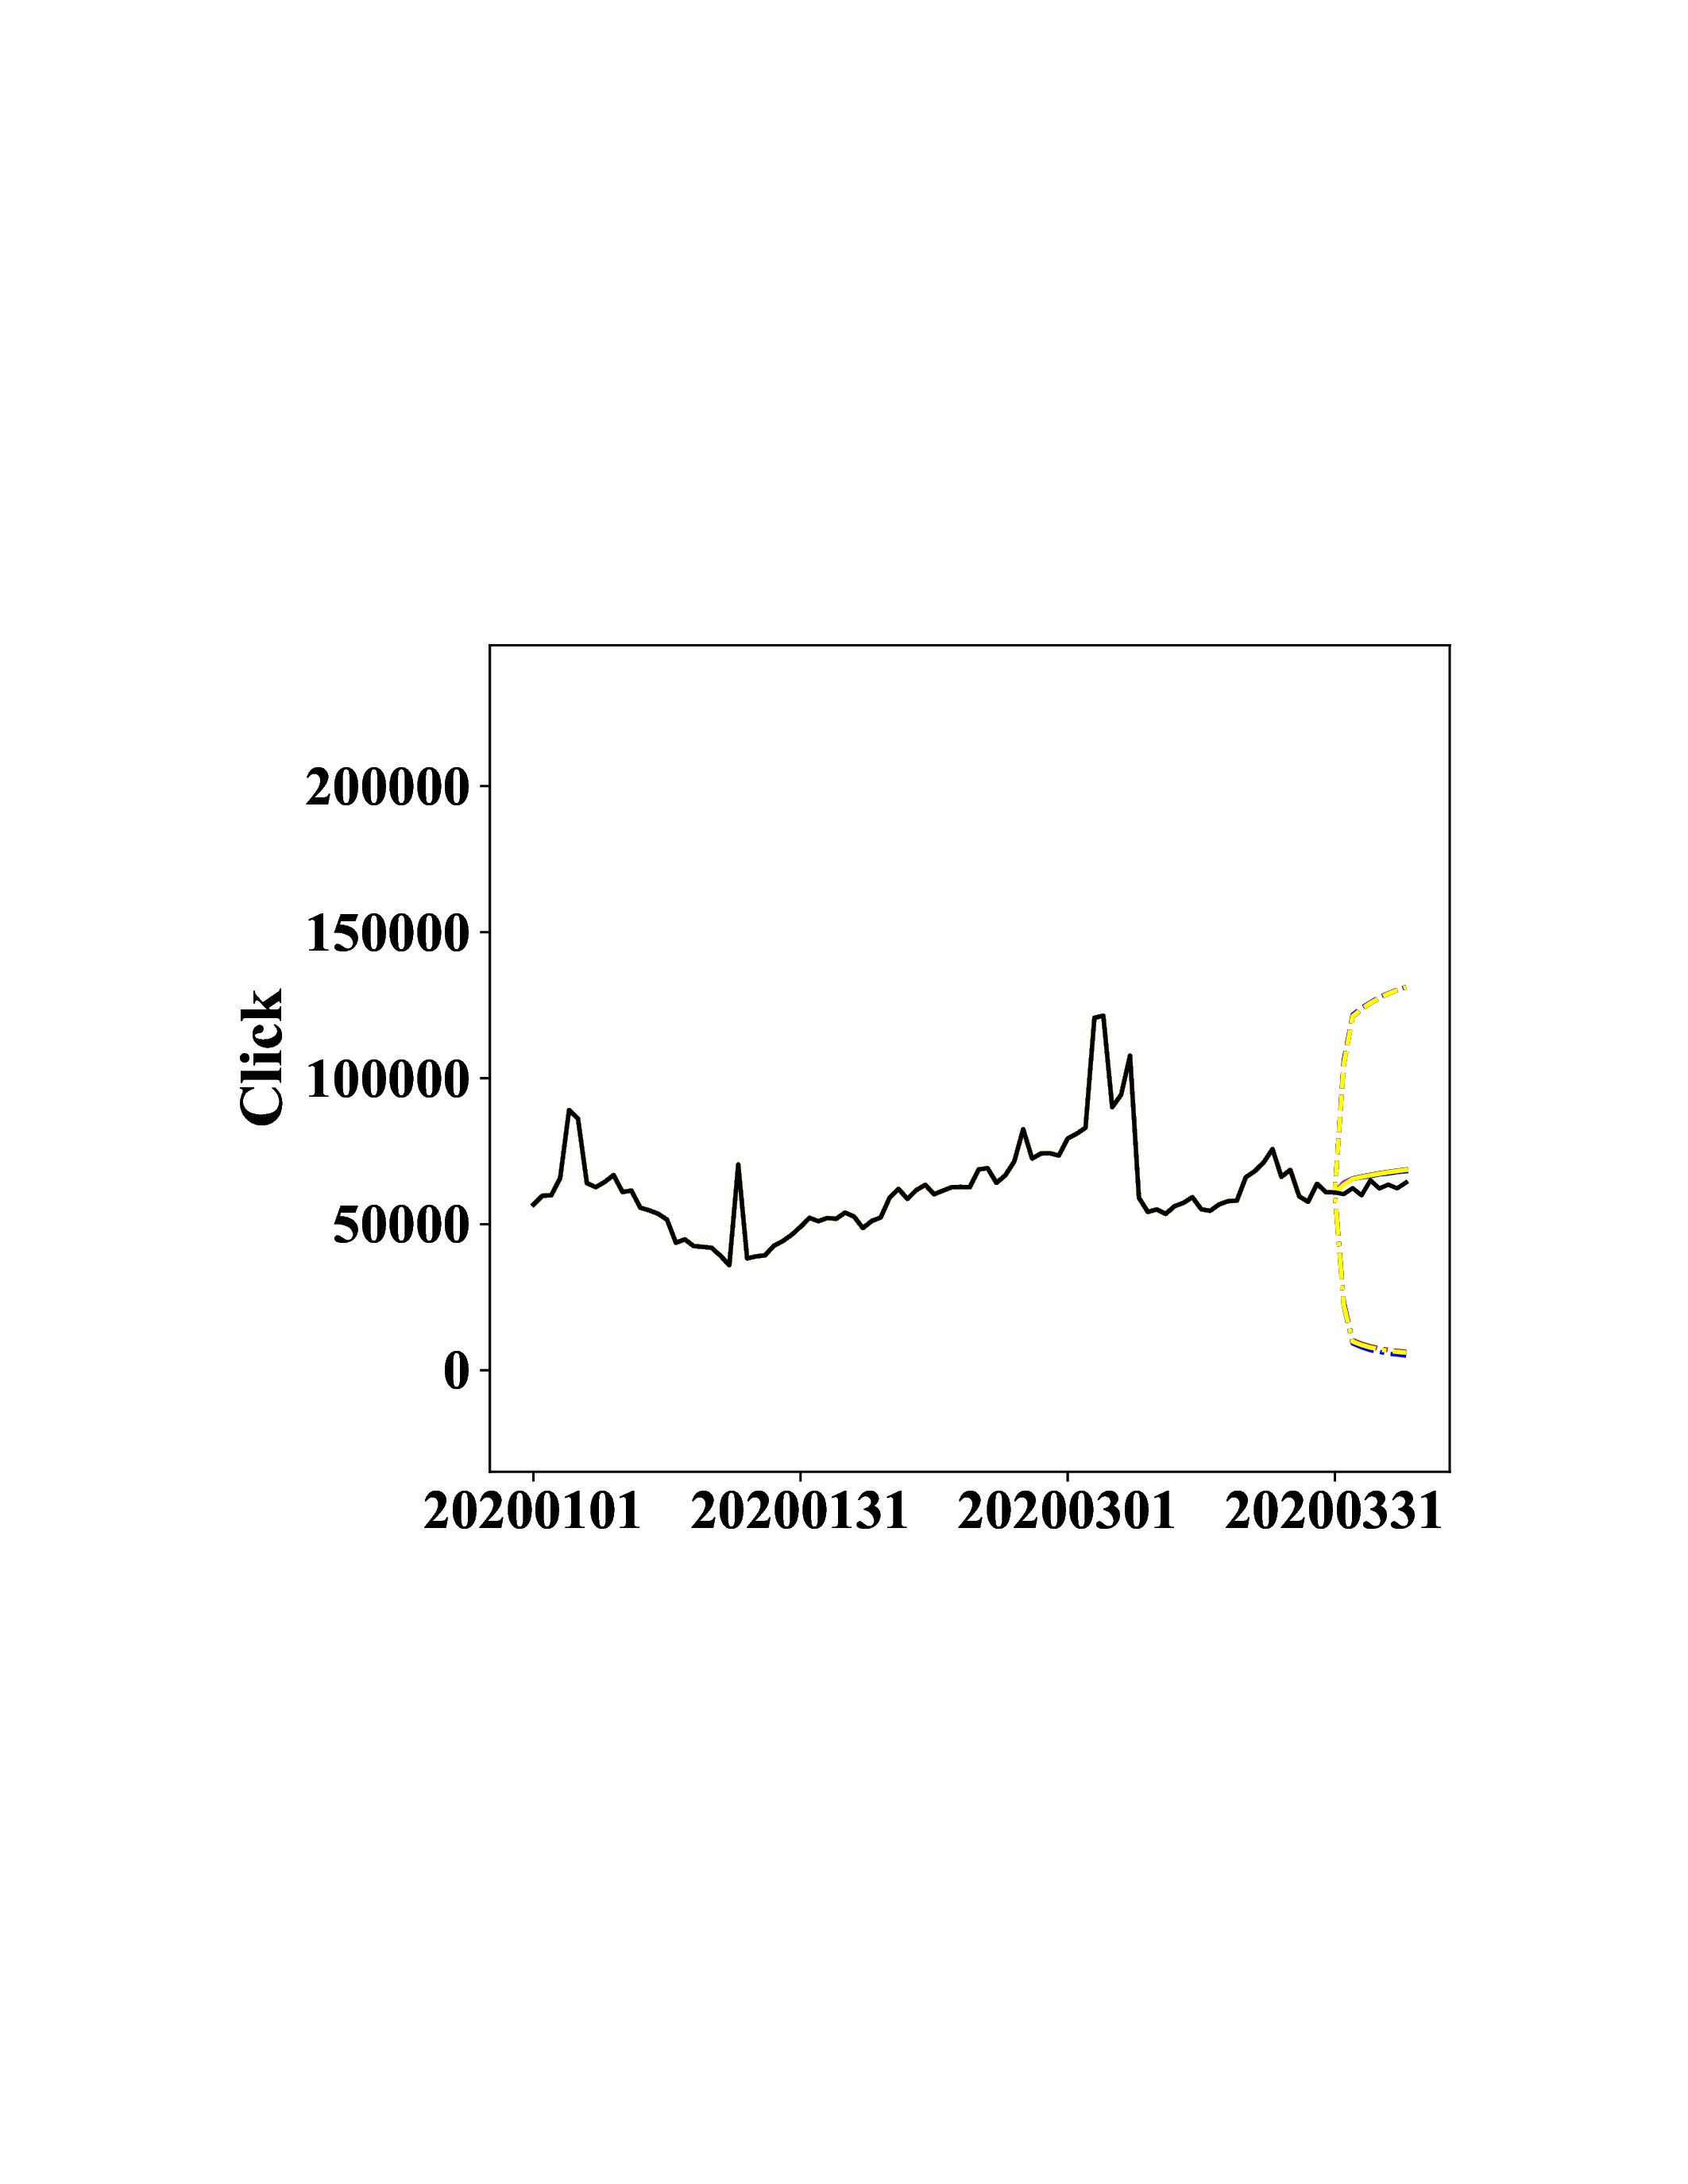}
\end{minipage}
}
\caption{ARIMA average predict error and interval at selectivity 0.5\% (why not 0.5\%? -- inconsistent with 0.5\% above) on click via different sampling methods (so the predictions in different sampling methods are almost the same?)}
% \label{AQP and ARIMA Performance}
\end{figure*}
%---------end-------------

%==============Selectivity 5% on Click Case===============

\begin{figure*}[hb]
\subfigure[Sampling rate 0.02\%]{
\begin{minipage}[t]{0.33\linewidth}
\centering
\includegraphics[width=2.2in, height=2.0in]{fig-new/vldb-fig9-fix-sample-9248224-5000-500w-clk-case.eps}
% \label{fig:side:a}
\end{minipage}
}
\subfigure[Sampling rate 0.1\%]{
\begin{minipage}[t]{0.33\linewidth}
\centering
\includegraphics[width=2.2in, height=2.0in]{fig-new/vldb-fig9-fix-sample-9248224-1000-500w-clk-case.eps}
\end{minipage}
}
\subfigure[Sampling rate 1\%]{
\begin{minipage}[t]{0.33\linewidth}
\centering
\includegraphics[width=2.2in, height=2.0in]{fig-new/vldb-fig9-fix-sample-9248224-100-500w-clk-case.eps}
\end{minipage}
}
\caption{ARIMA average predict error and interval at selectivity 5\% (why not 0.5\%? -- inconsistent with 0.5\% above) on click via different sampling methods (so the predictions in different sampling methods are almost the same?)}
% \label{AQP and ARIMA Performance}
\end{figure*}
%---------end-------------

%==============Selectivity 0.5% on Favorite Case===============

\begin{figure*}[hb]
\subfigure[Sampling rate 0.02\%]{
\begin{minipage}[t]{0.33\linewidth}
\centering
\includegraphics[width=2.2in, height=2.0in]{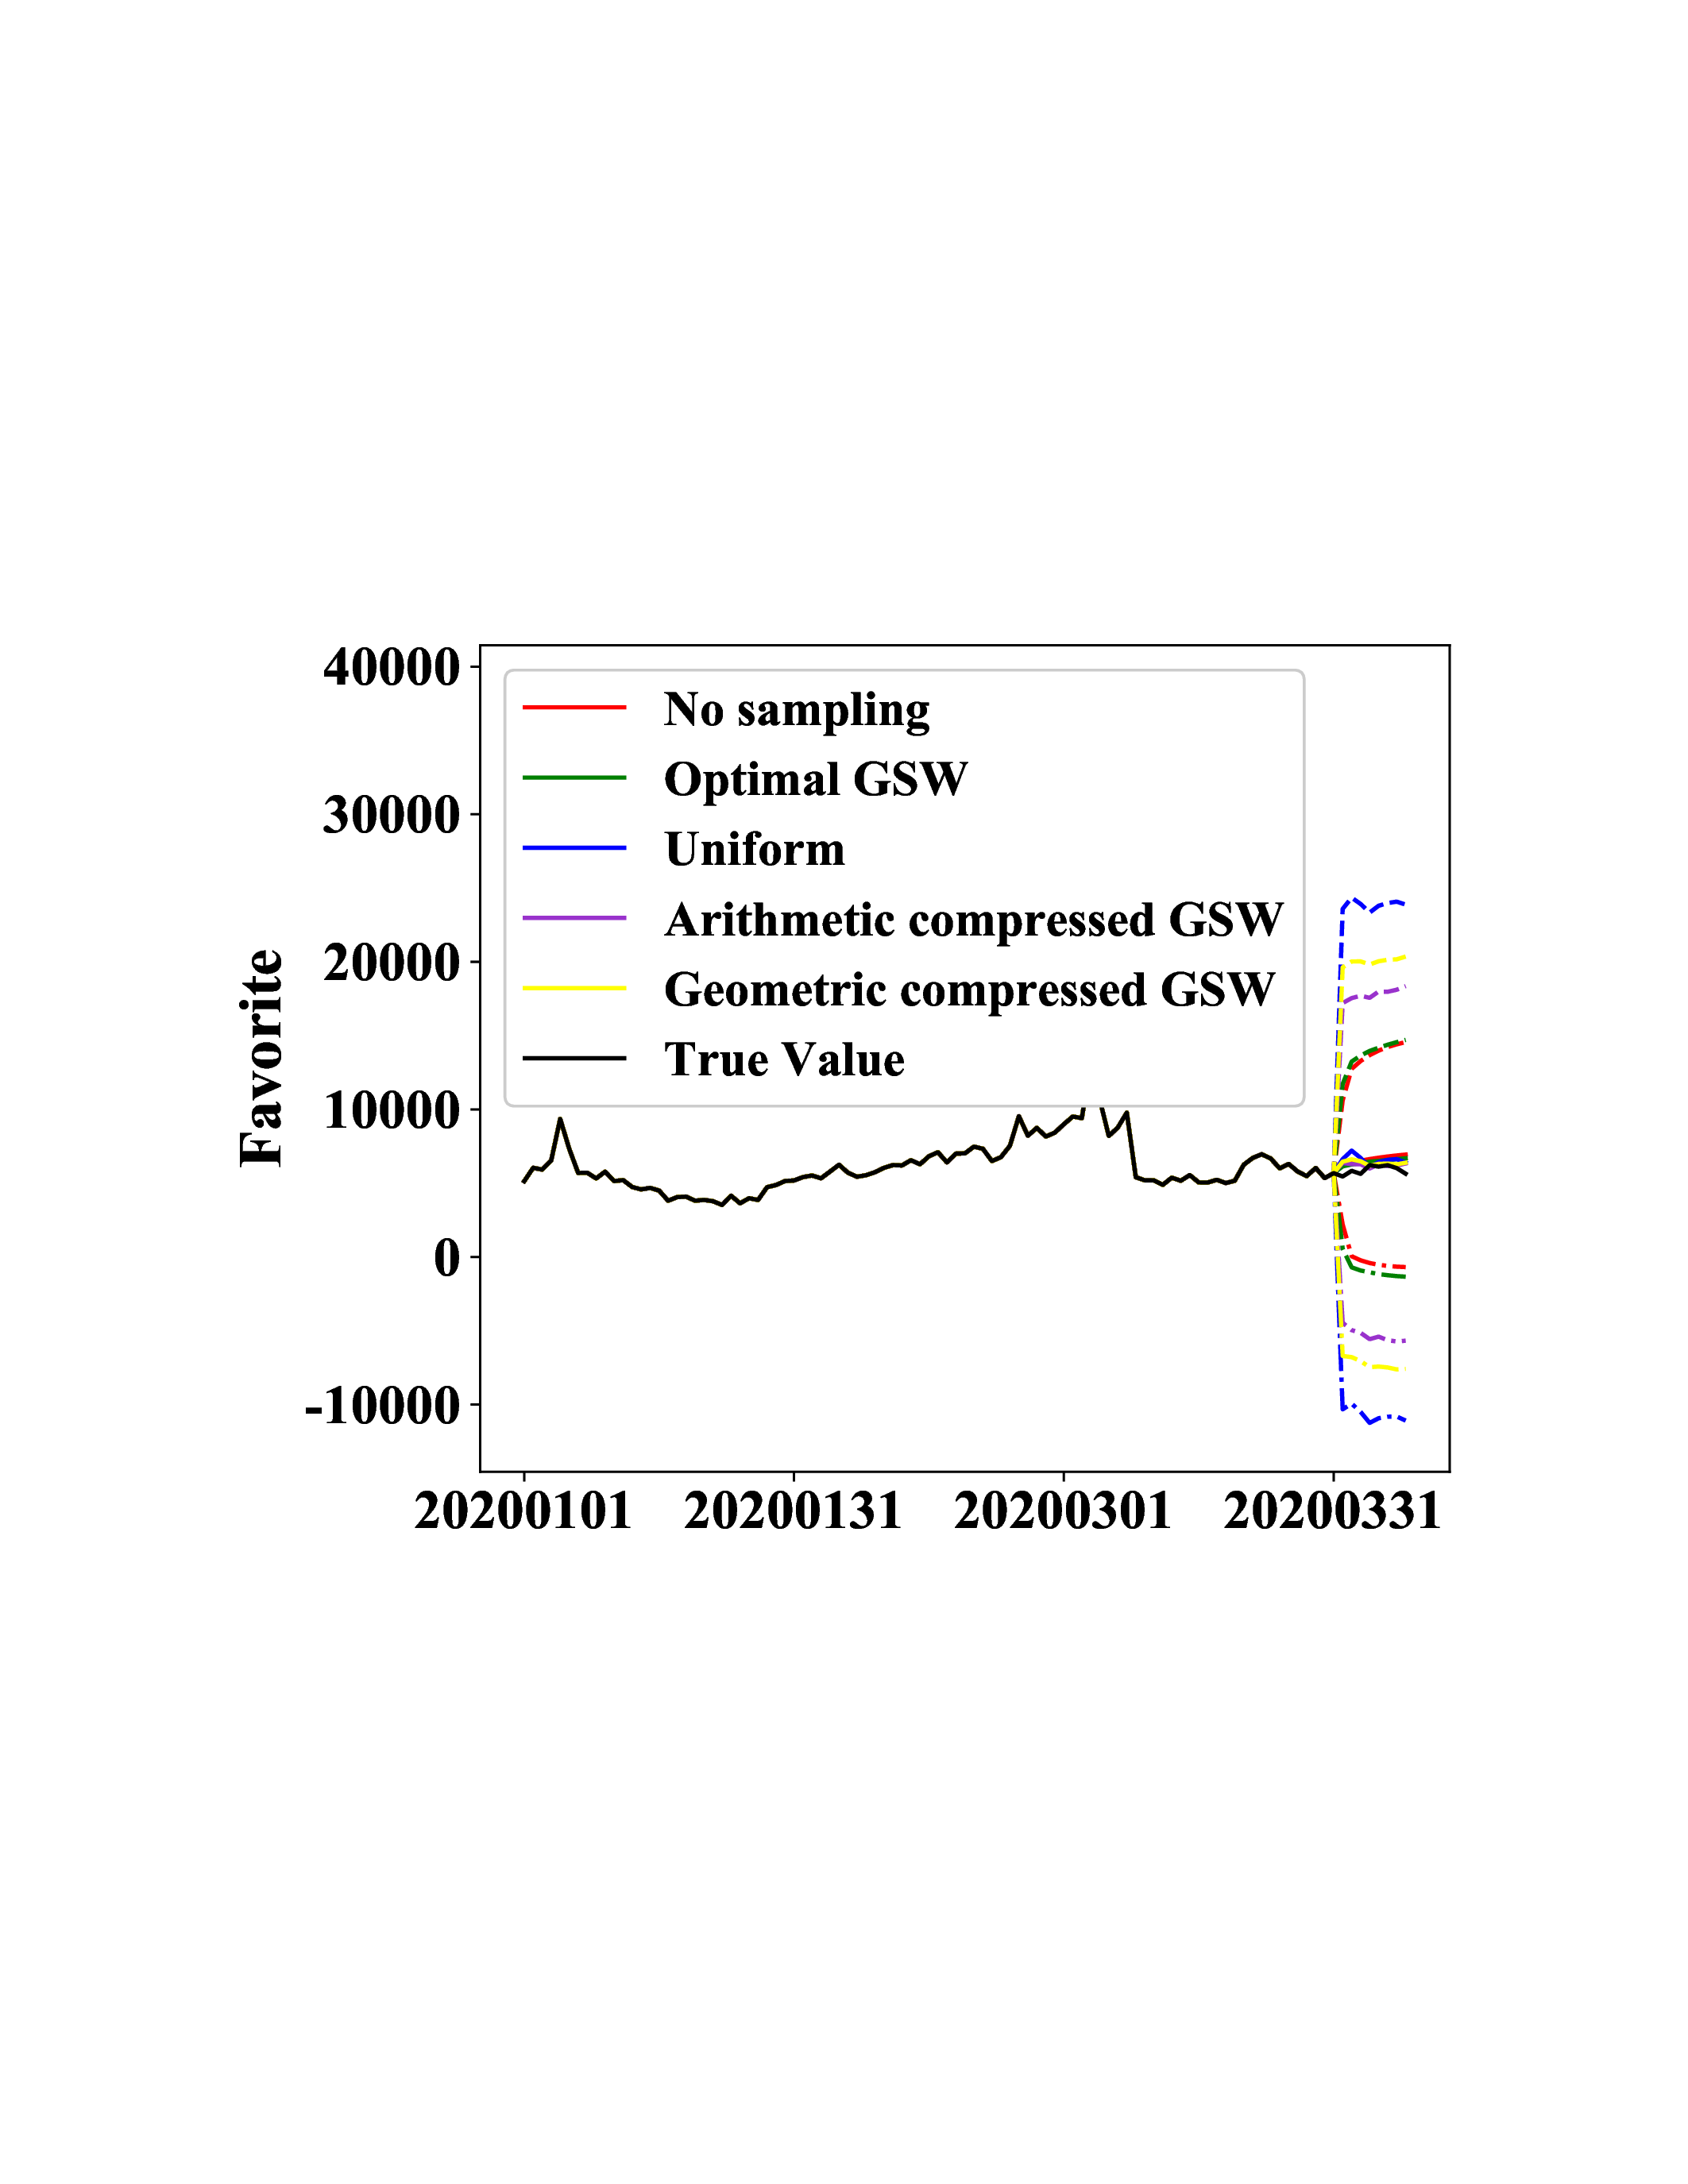}
% \label{fig:side:a}
\end{minipage}
}
\subfigure[Sampling rate 0.1\%]{
\begin{minipage}[t]{0.33\linewidth}
\centering
\includegraphics[width=2.2in, height=2.0in]{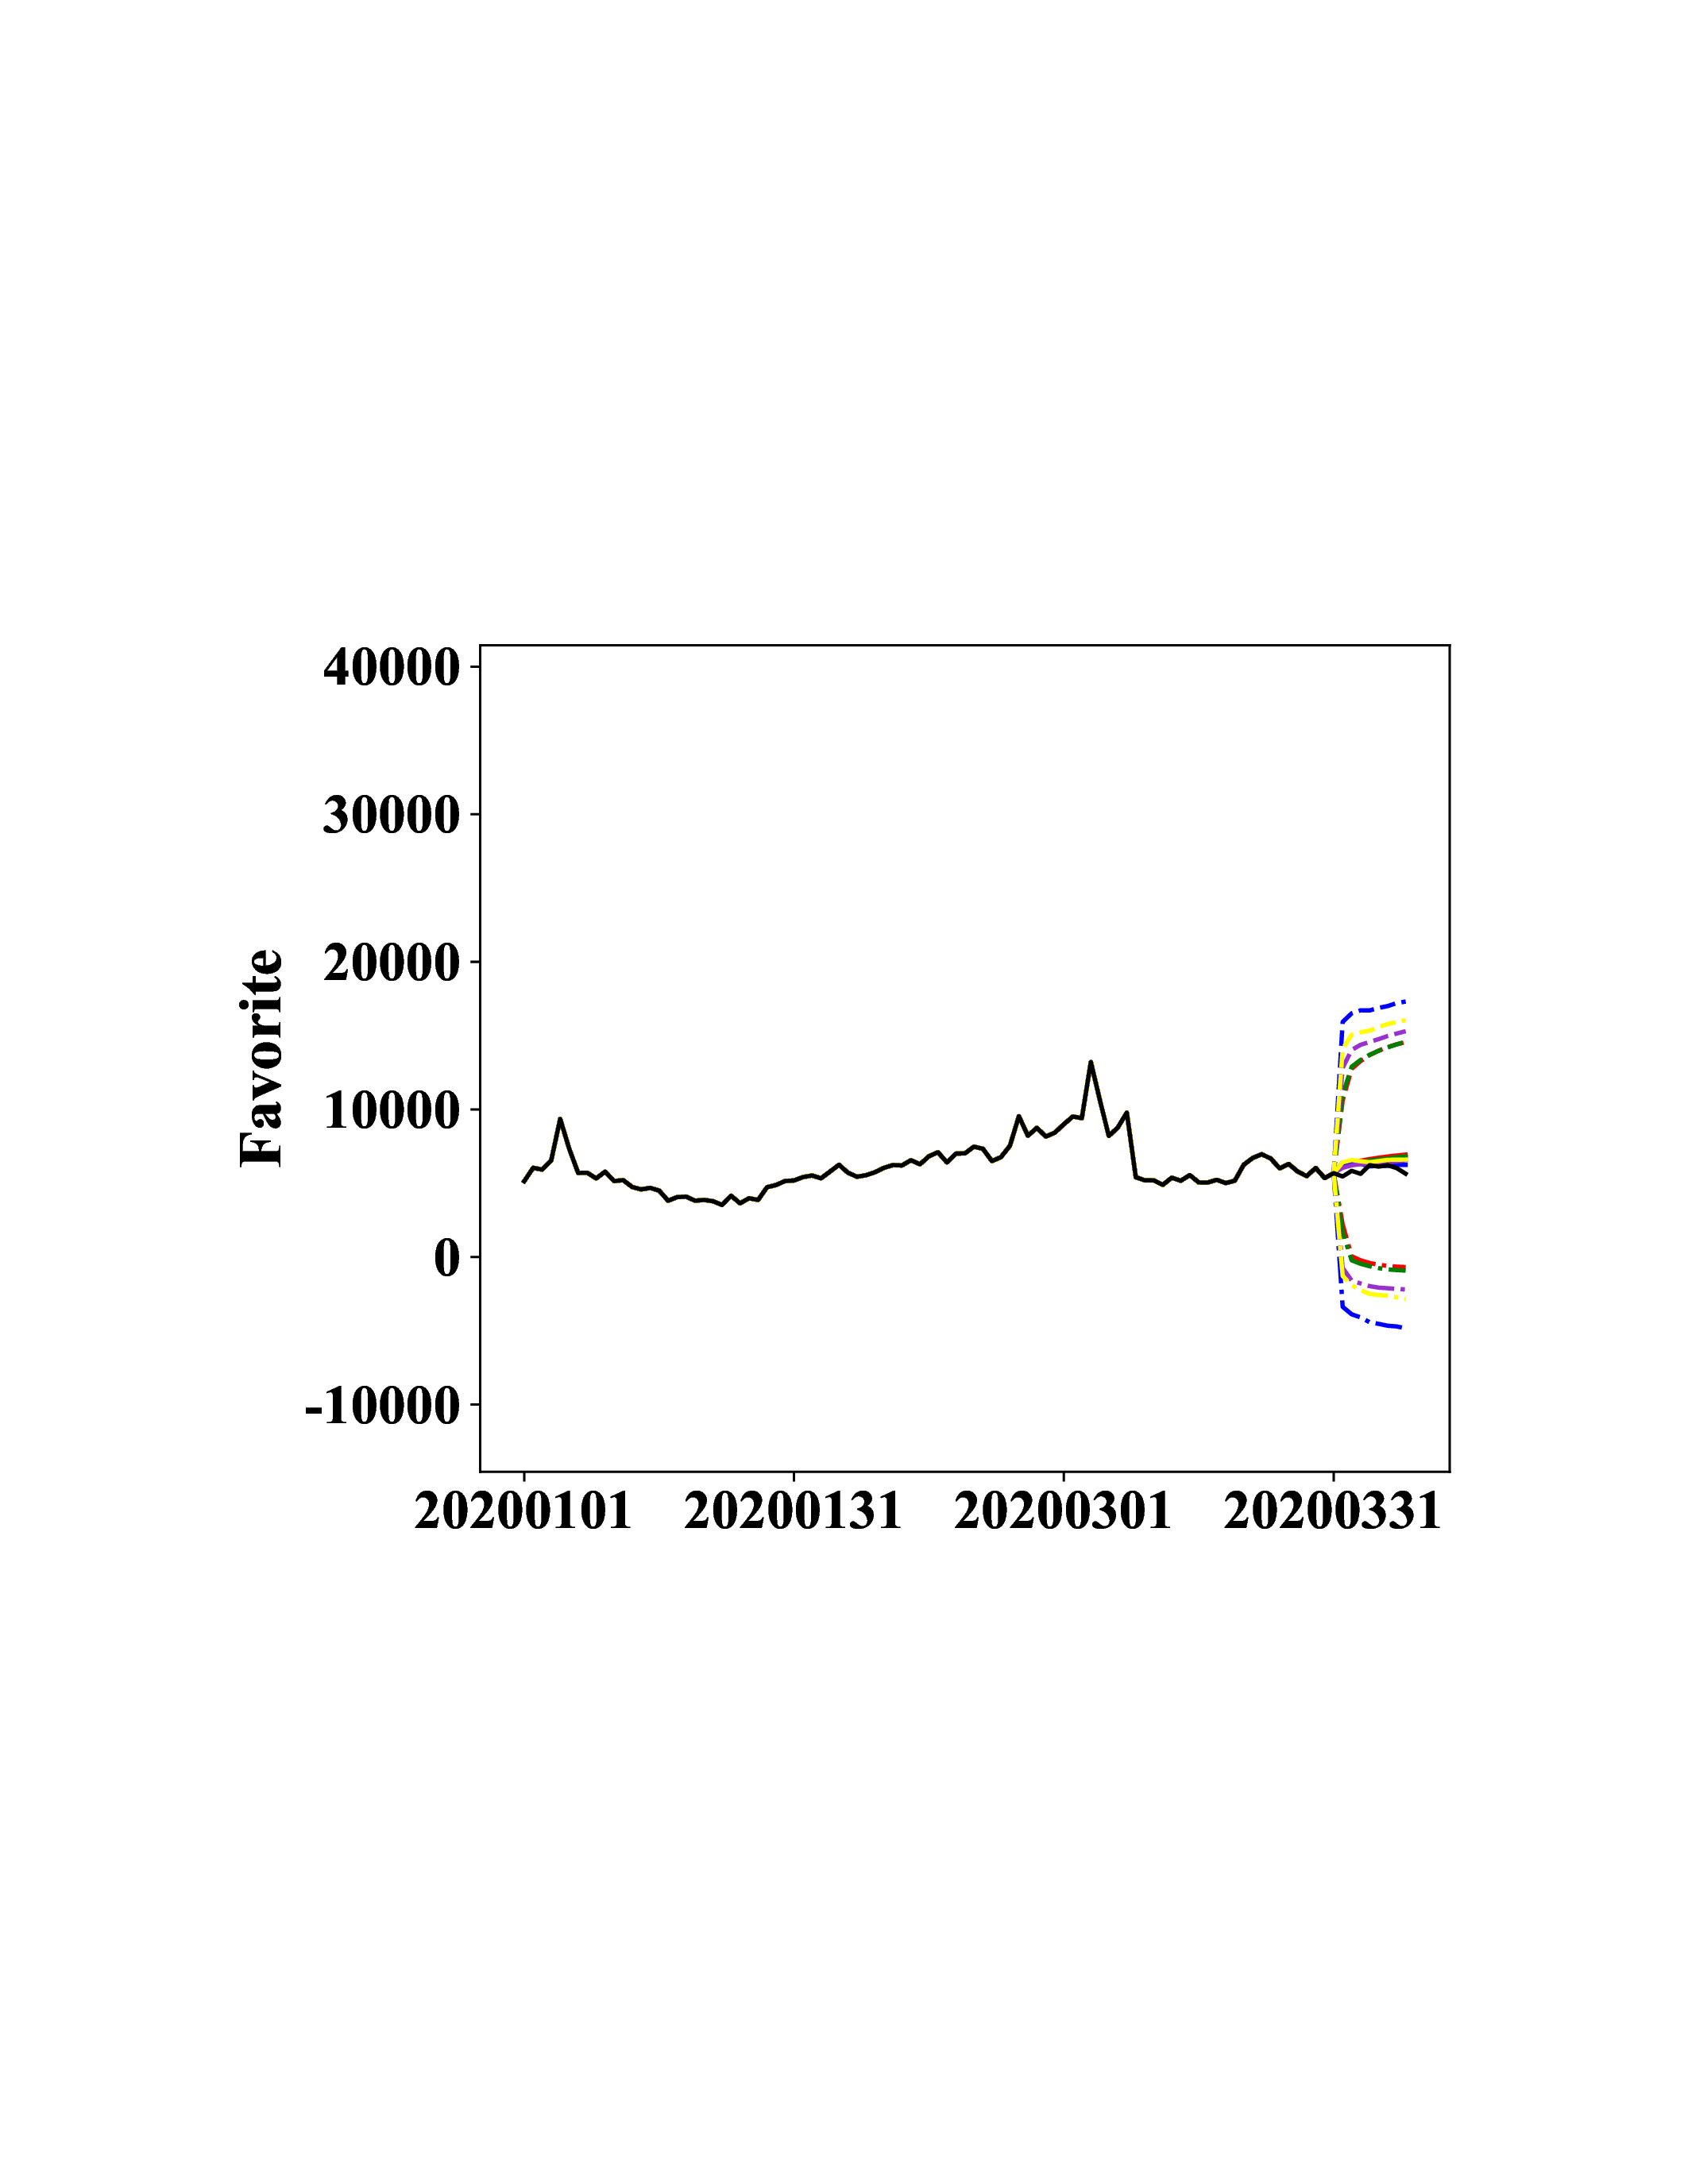}
\end{minipage}
}
\subfigure[Sampling rate 1\%]{
\begin{minipage}[t]{0.33\linewidth}
\centering
\includegraphics[width=2.2in, height=2.0in]{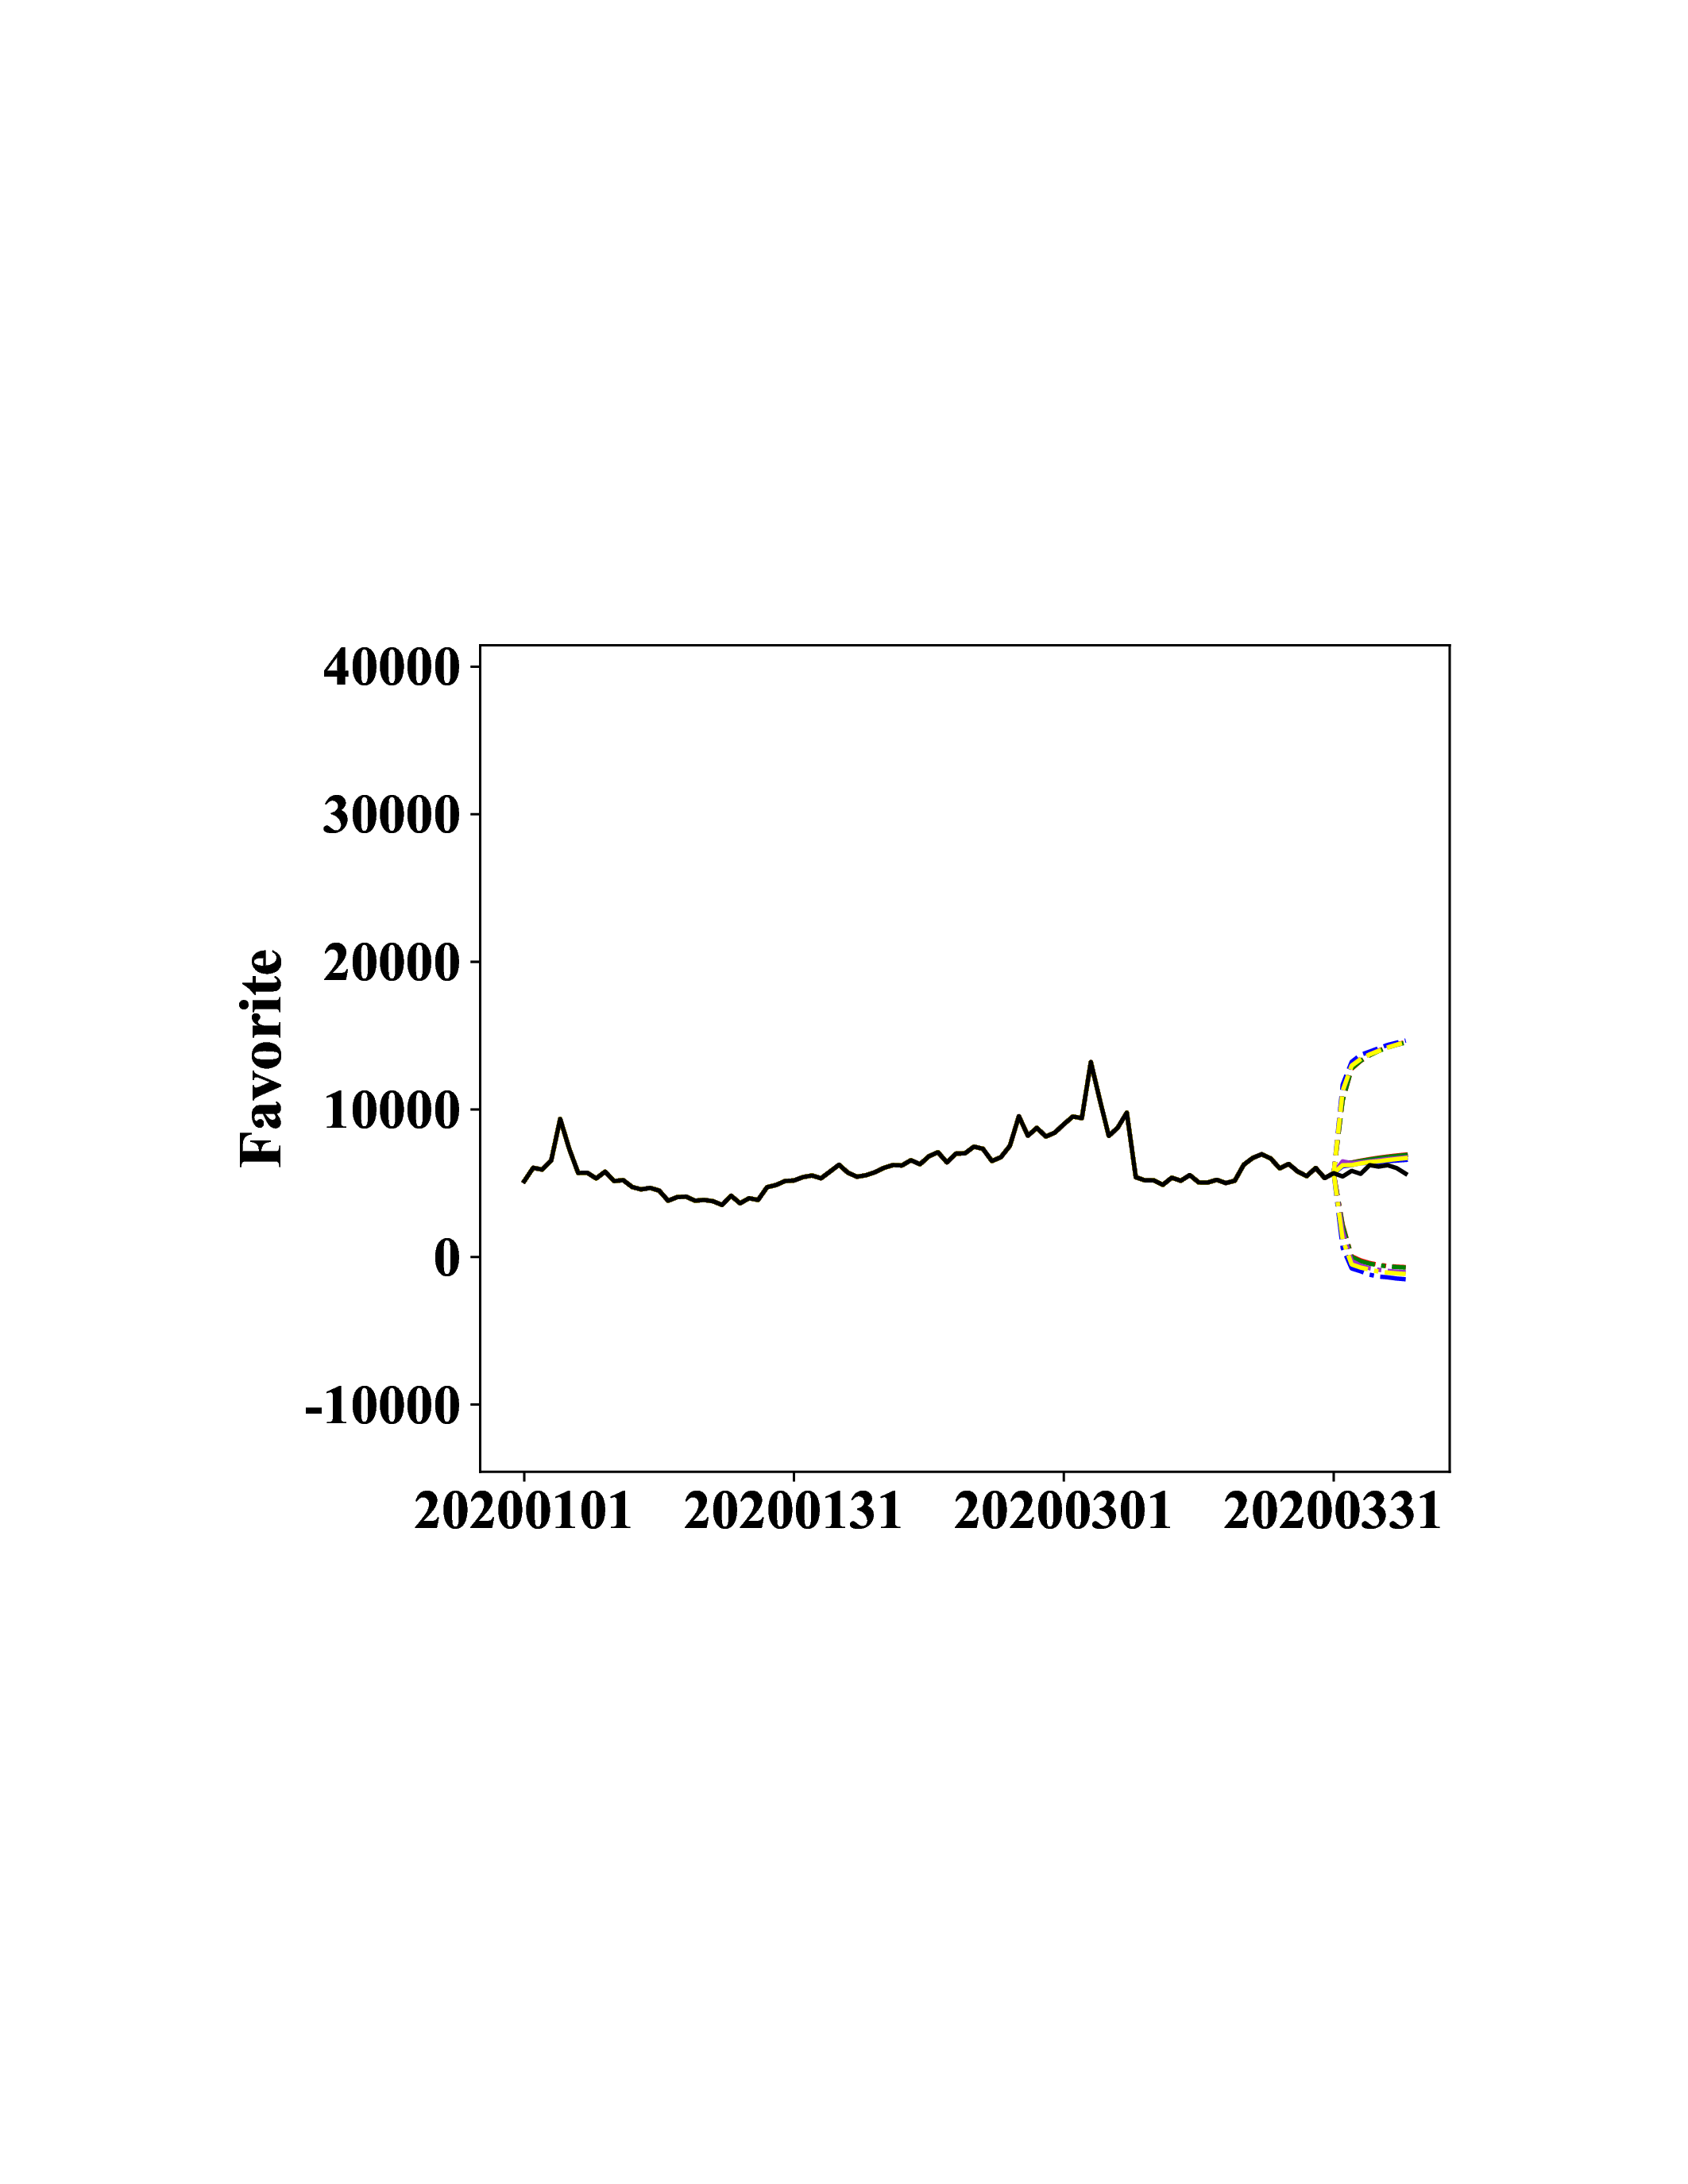}
\end{minipage}
}
\caption{ARIMA average predict error and interval at selectivity 0.5\% (why not 0.5\%? -- inconsistent with 0.5\% above) on favorite via different sampling methods (so the predictions in different sampling methods are almost the same?)}
% \label{AQP and ARIMA Performance}
\end{figure*}
%---------end-------------

%==============Selectivity 5% on Favorite Case===============

\begin{figure*}[hb]
\subfigure[Sampling rate 0.02\%]{
\begin{minipage}[t]{0.33\linewidth}
\centering
\includegraphics[width=2.2in, height=2.0in]{fig-new/vldb-fig9-fix-sample-9248224-5000-500w-col-case.eps}
% \label{fig:side:a}
\end{minipage}
}
\subfigure[Sampling rate 0.1\%]{
\begin{minipage}[t]{0.33\linewidth}
\centering
\includegraphics[width=2.2in, height=2.0in]{fig-new/vldb-fig9-fix-sample-9248224-1000-500w-col-case.eps}
\end{minipage}
}
\subfigure[Sampling rate 1\%]{
\begin{minipage}[t]{0.33\linewidth}
\centering
\includegraphics[width=2.2in, height=2.0in]{fig-new/vldb-fig9-fix-sample-9248224-100-500w-col-case.eps}
\end{minipage}
}
\caption{ARIMA average predict error and interval at selectivity 5\% (why not 0.5\%? -- inconsistent with 0.5\% above) on favorite via different sampling methods (so the predictions in different sampling methods are almost the same?)}
% \label{AQP and ARIMA Performance}
\end{figure*}
%---------end-------------

%==============Selectivity 0.5% on Cart Case===============

\begin{figure*}[hb]
\subfigure[Sampling rate 0.02\%]{
\begin{minipage}[t]{0.33\linewidth}
\centering
\includegraphics[width=2.2in, height=2.0in]{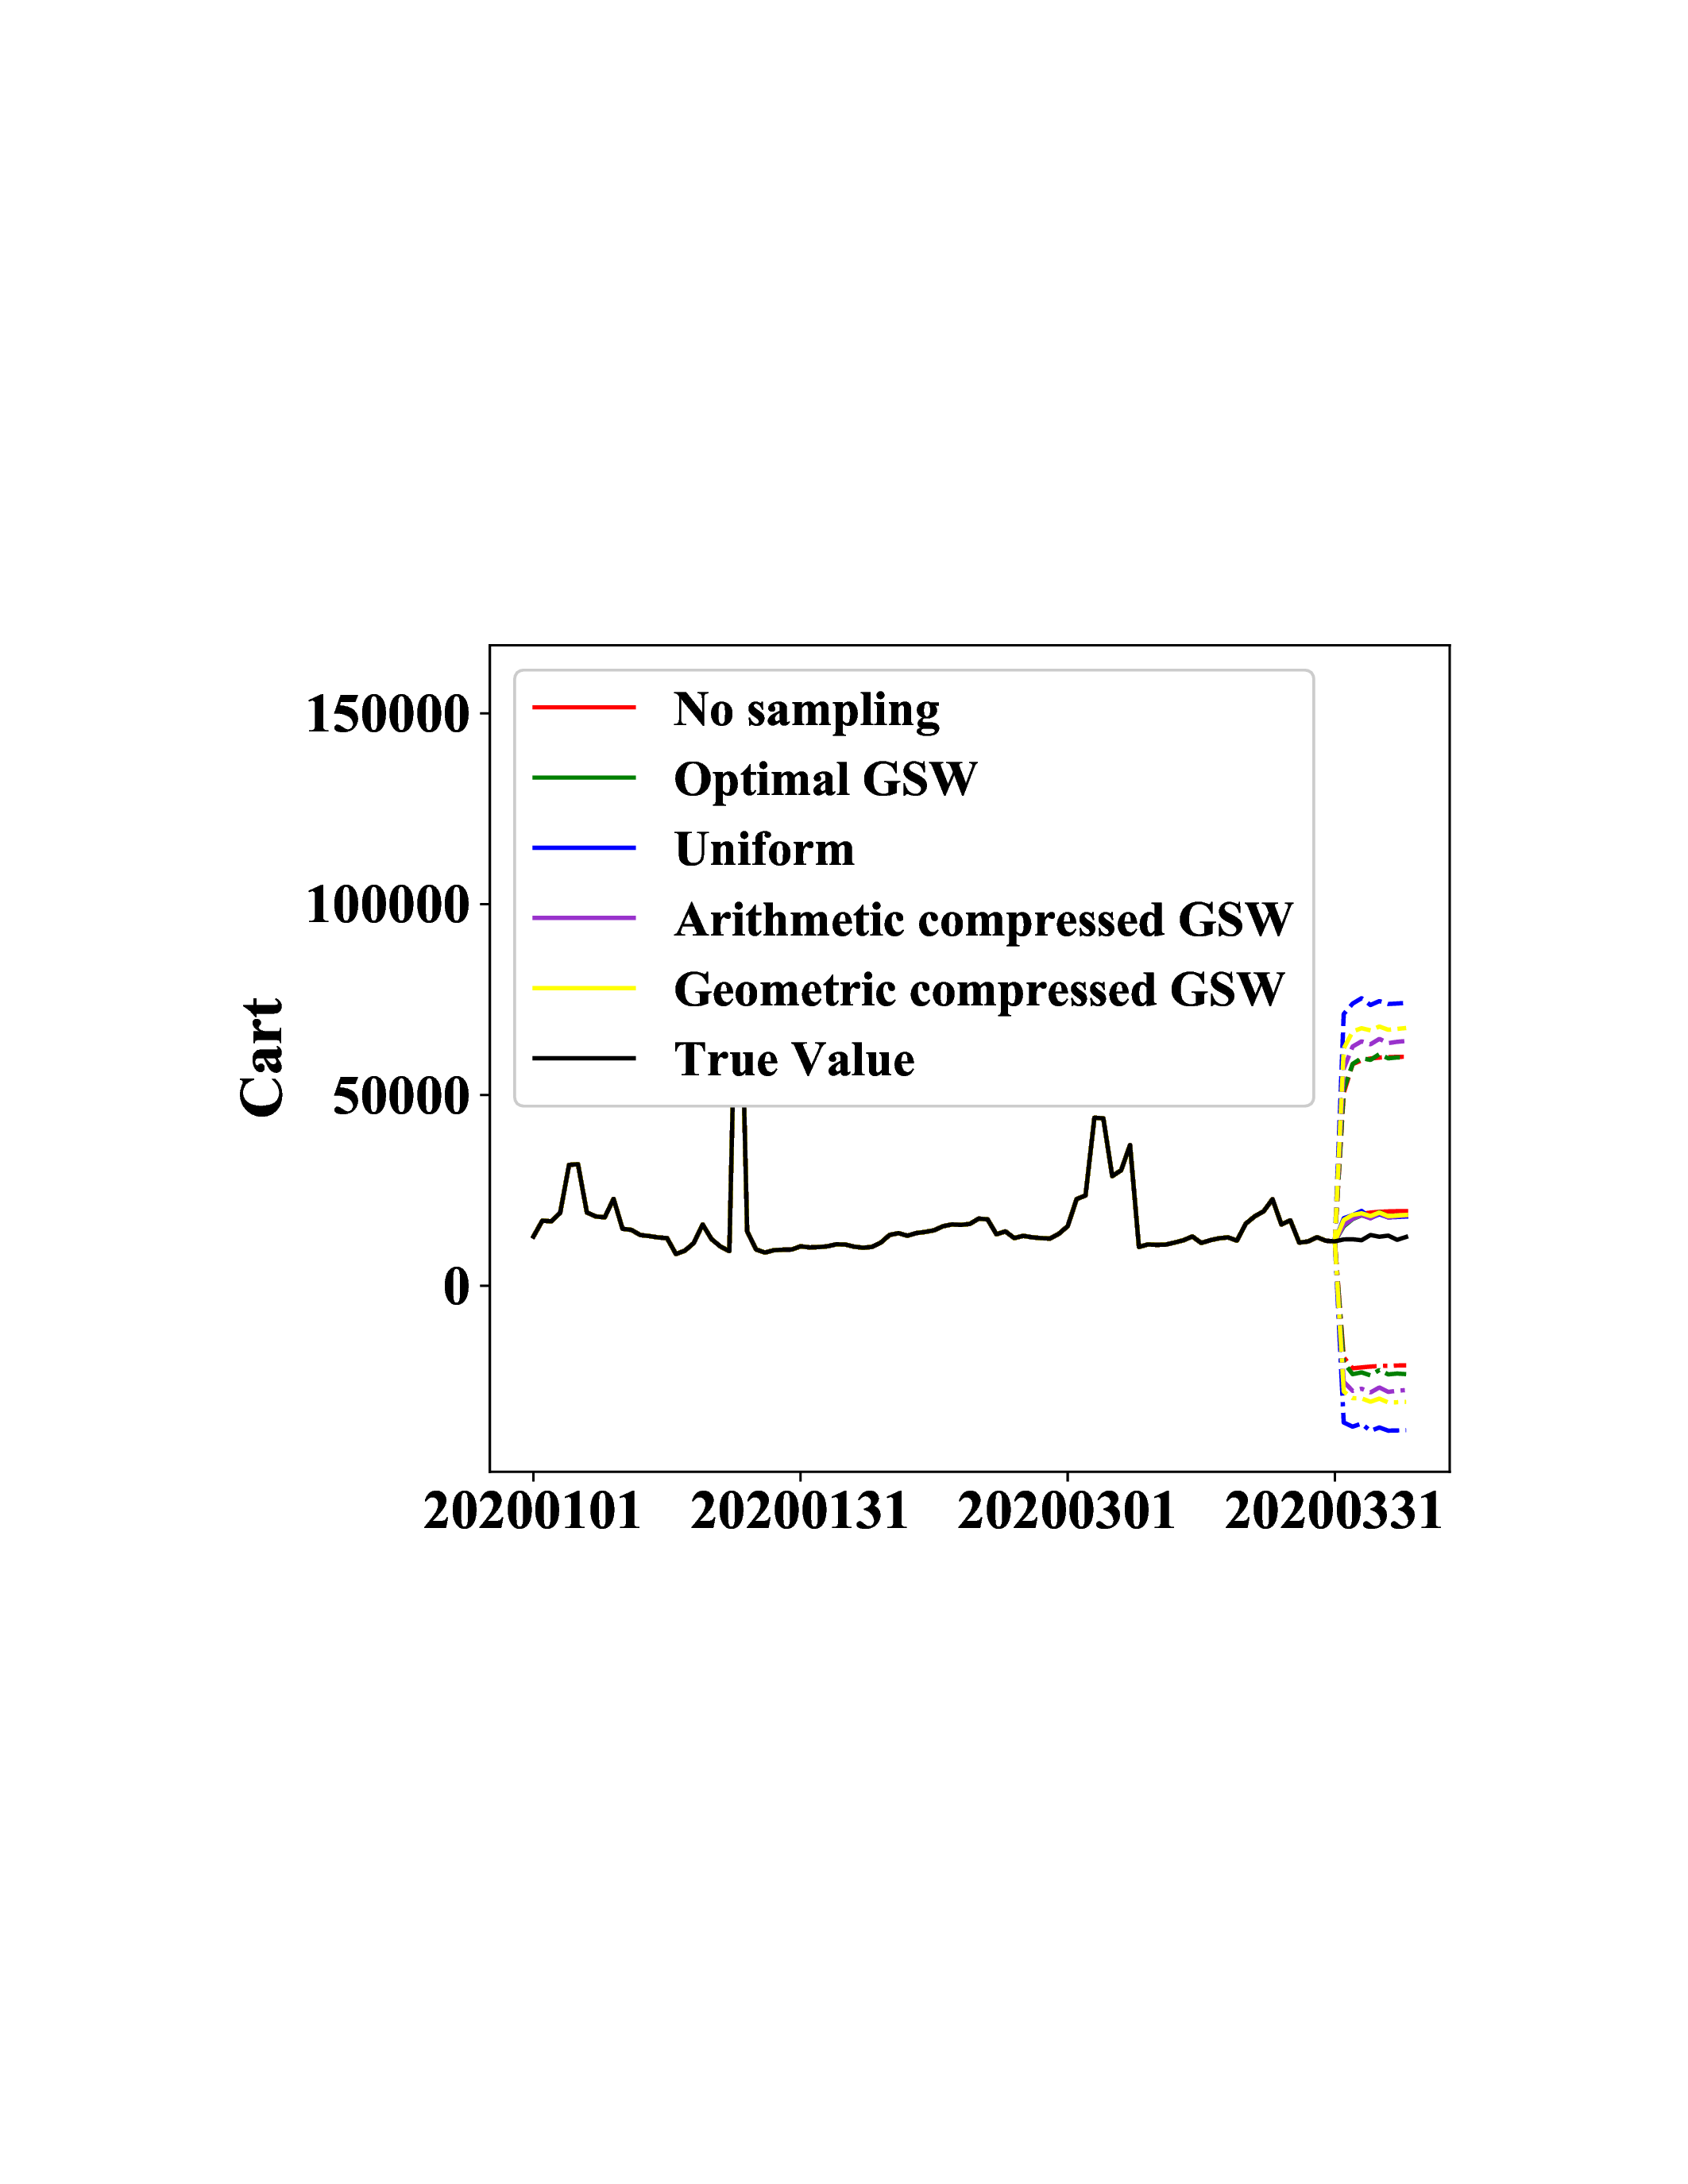}
% \label{fig:side:a}
\end{minipage}
}
\subfigure[Sampling rate 0.1\%]{
\begin{minipage}[t]{0.33\linewidth}
\centering
\includegraphics[width=2.2in, height=2.0in]{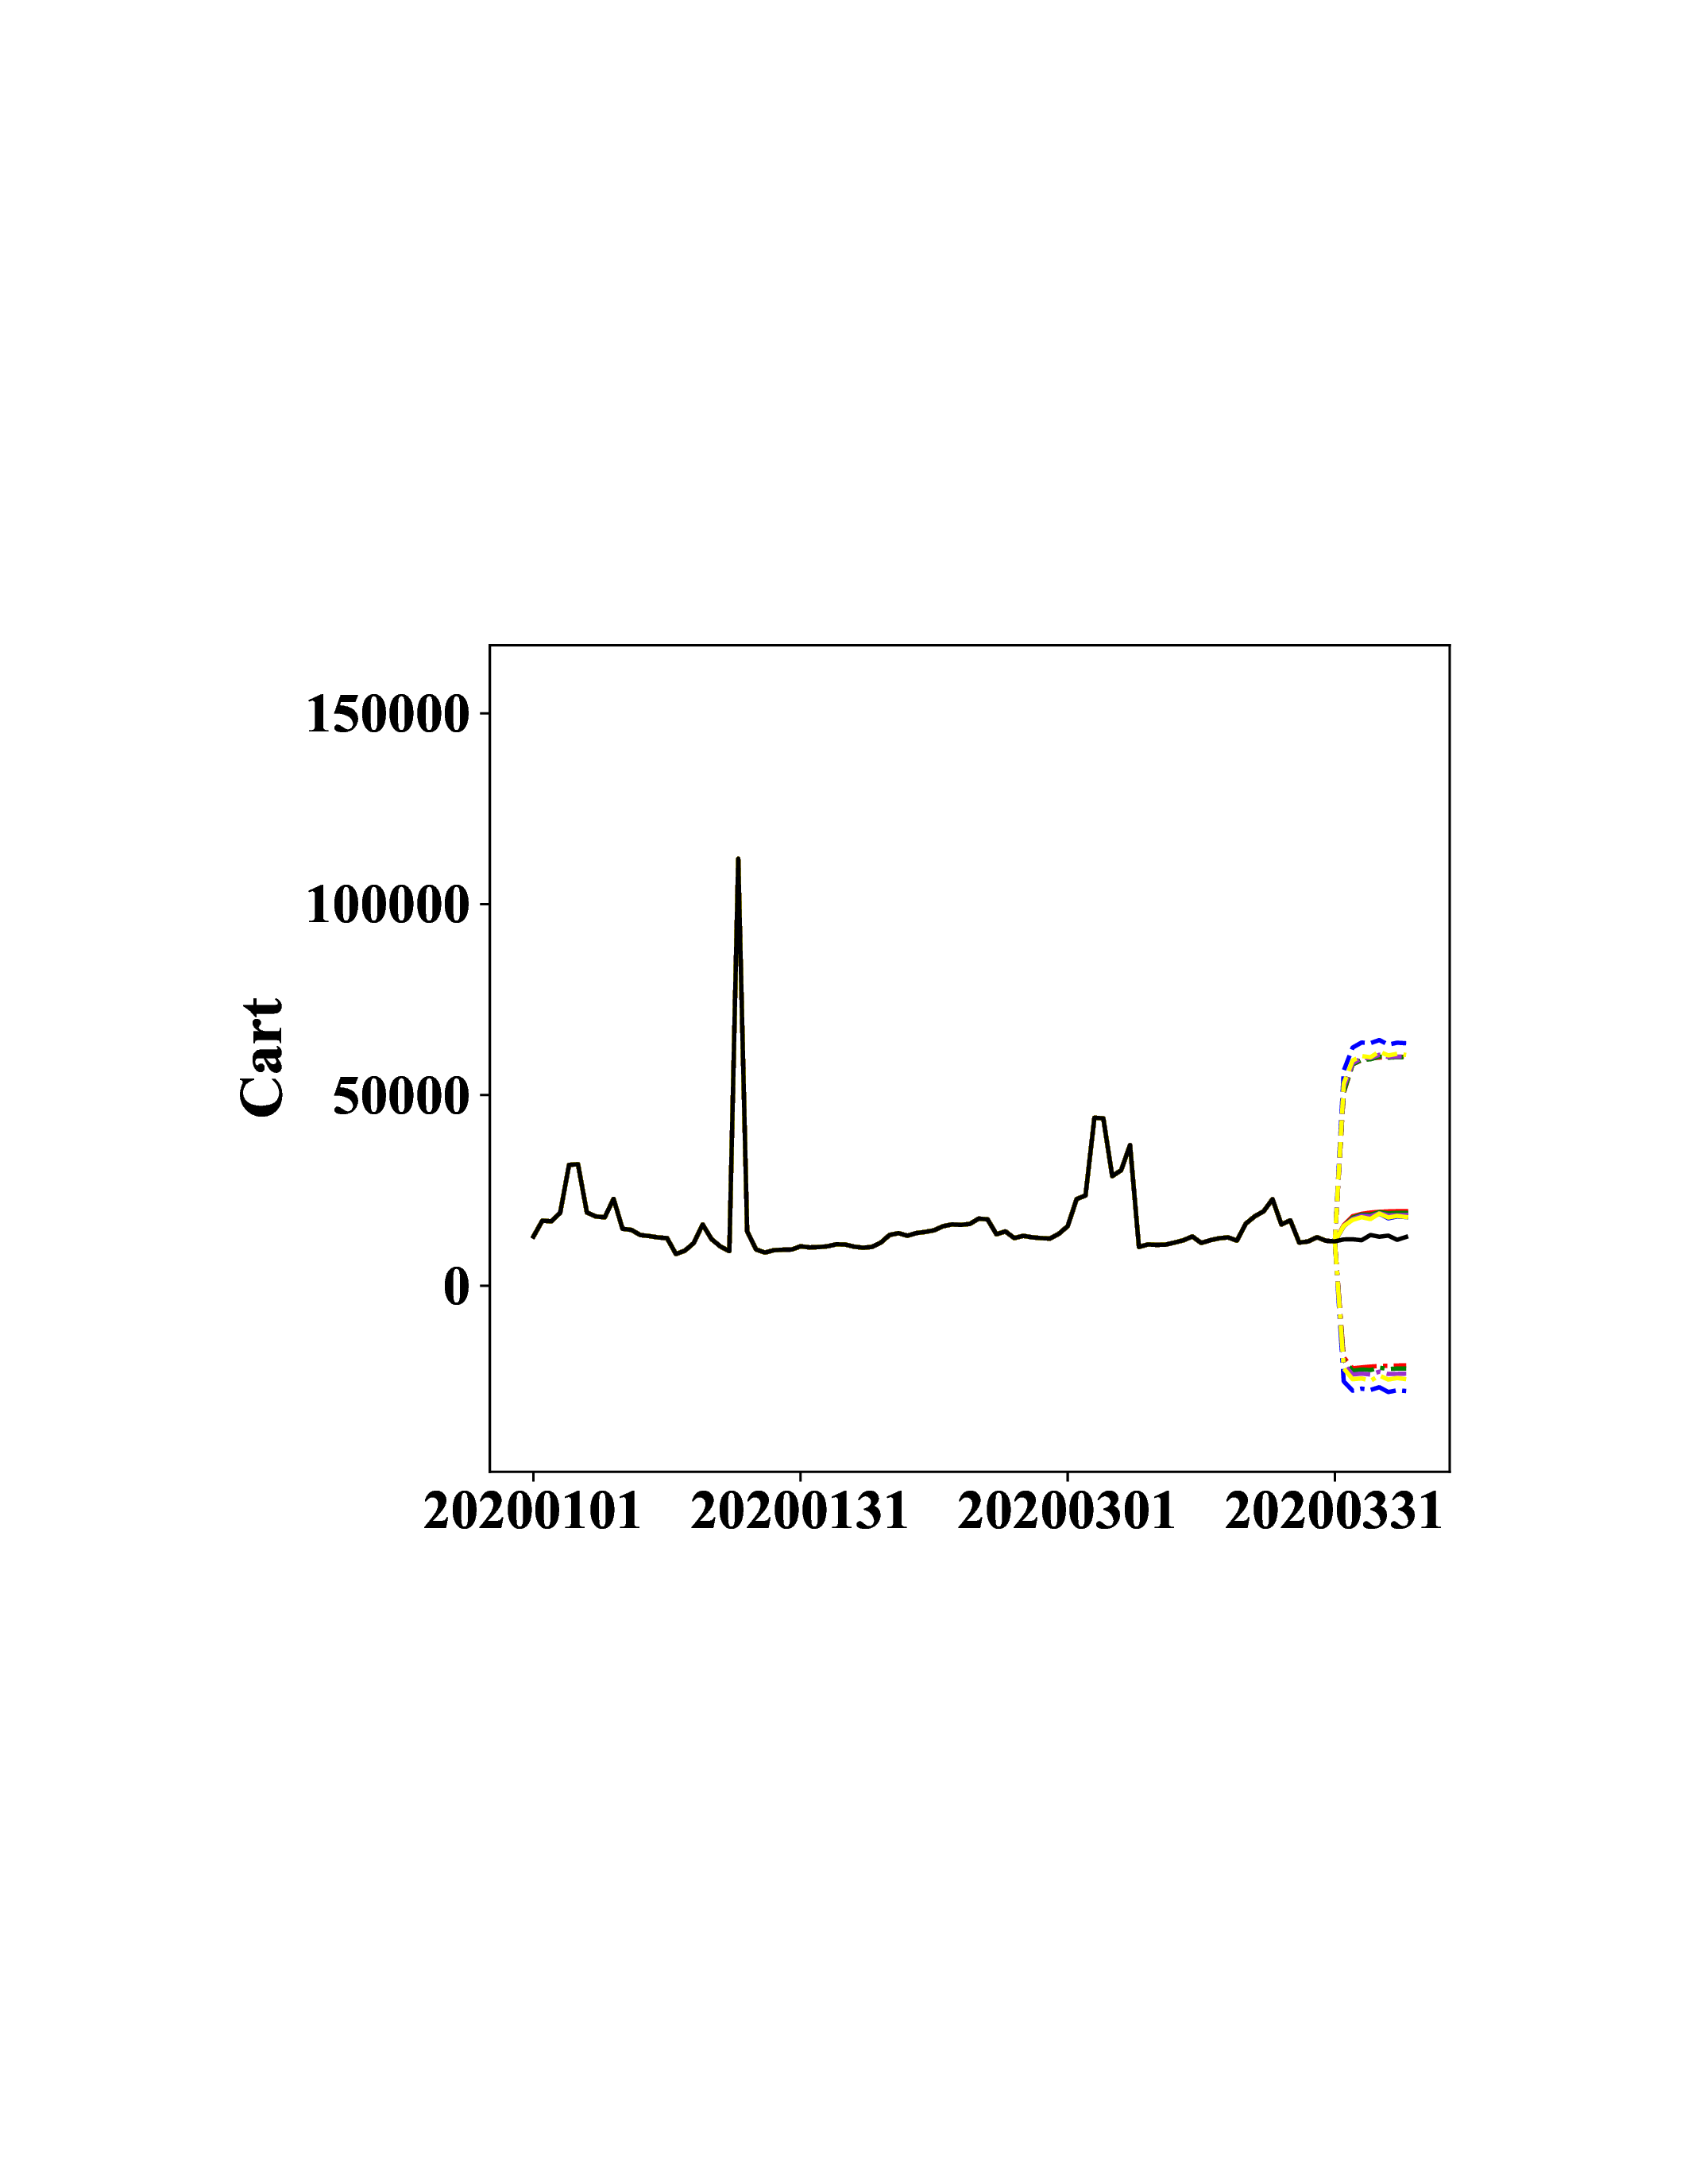}
\end{minipage}
}
\subfigure[Sampling rate 1\%]{
\begin{minipage}[t]{0.33\linewidth}
\centering
\includegraphics[width=2.2in, height=2.0in]{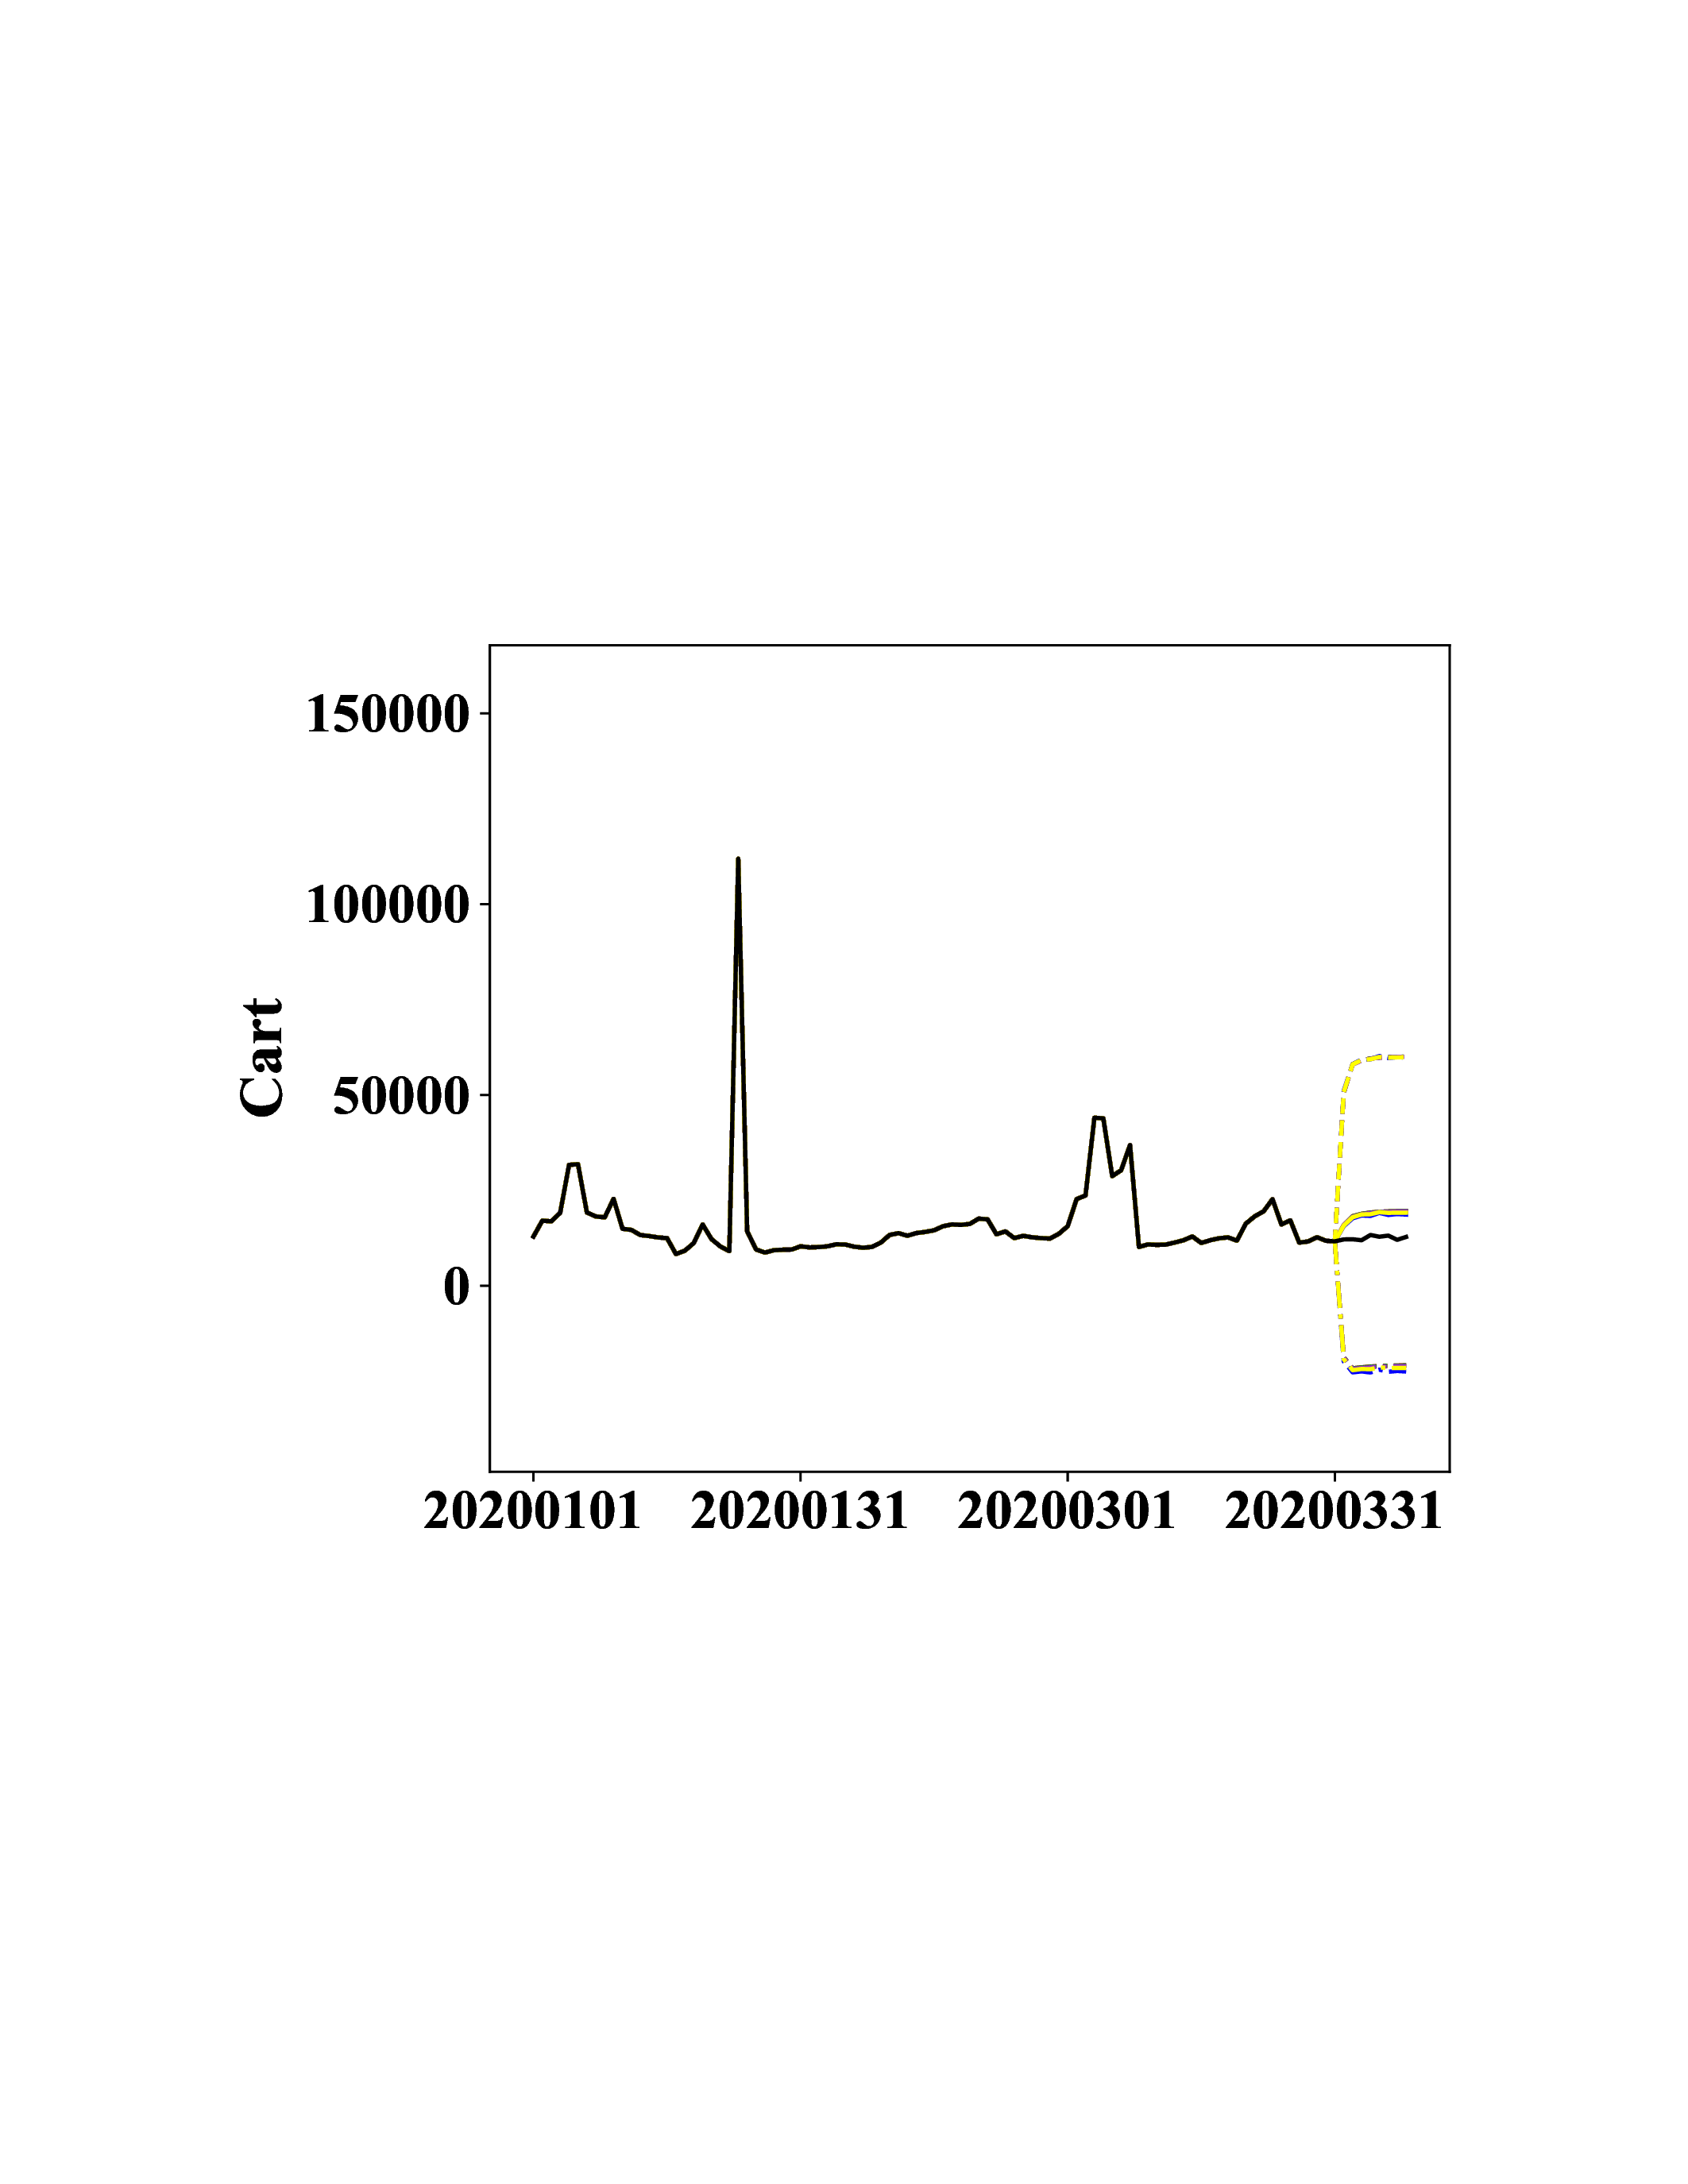}
\end{minipage}
}
\caption{ARIMA average predict error and interval at selectivity 0.5\% (why not 0.5\%? -- inconsistent with 0.5\% above) on cart via different sampling methods (so the predictions in different sampling methods are almost the same?)}
% \label{AQP and ARIMA Performance}
\end{figure*}
%---------end-------------

%==============Selectivity 5% on Cart Case===============

\begin{figure*}[hb]
\subfigure[Sampling rate 0.02\%]{
\begin{minipage}[t]{0.33\linewidth}
\centering
\includegraphics[width=2.2in, height=2.0in]{fig-new/vldb-fig9-fix-sample-9248224-5000-500w-cart-case.eps}
% \label{fig:side:a}
\end{minipage}
}
\subfigure[Sampling rate 0.1\%]{
\begin{minipage}[t]{0.33\linewidth}
\centering
\includegraphics[width=2.2in, height=2.0in]{fig-new/vldb-fig9-fix-sample-9248224-1000-500w-cart-case.eps}
\end{minipage}
}
\subfigure[Sampling rate 1\%]{
\begin{minipage}[t]{0.33\linewidth}
\centering
\includegraphics[width=2.2in, height=2.0in]{fig-new/vldb-fig9-fix-sample-9248224-100-500w-cart-case.eps}
\end{minipage}
}
\caption{ARIMA average predict error and interval at selectivity 5\% (why not 0.5\%? -- inconsistent with 0.5\% above) on cart via different sampling methods (so the predictions in different sampling methods are almost the same?)}
% \label{AQP and ARIMA Performance}
\end{figure*}
%---------end-------------

%=========================

%%图13展示了对于固定的数据集，binomial sampling和compressed-arithmetic-mean sampling保证在没有任何筛选条件下
%%对每一天的impression, click, favorite以及cart四个指标求sum，一共有30天，每一组sample可以获得30个[sum_imp, sum_clk, sum_fav,sum_cart]，每一天共100组
%%对每一天的100组样本求平均，可以每天100组的平均误差，共有30天，再对30天求平均误差，将得到的平均误差来代表样本总体平均AQP误差。
%%实验使得binomial sampling和compressed-arithmetic-mean sampling四个指标参照上面方法，使得总体平均AQP误差接近
%%图13给出了样本的sampling rate和AQP总体平均误差，图14,15分别展示了在上述的样本中，取一个固定selectivity的人群
%%看这个人群在各个指标上的ARIMA predict error and interval
%%16,17,18,19是给出了具体case

%-----fig13. binomial sampling aqp error bound nearly to compressed-arithmetic-mean ----------
\begin{figure*}[hb]
\subfigure[Sampling rate (what is x-axis? AQP error?)]{
\begin{minipage}[t]{0.49\linewidth}
\centering
\includegraphics[width=2.2in, height=2.0in]{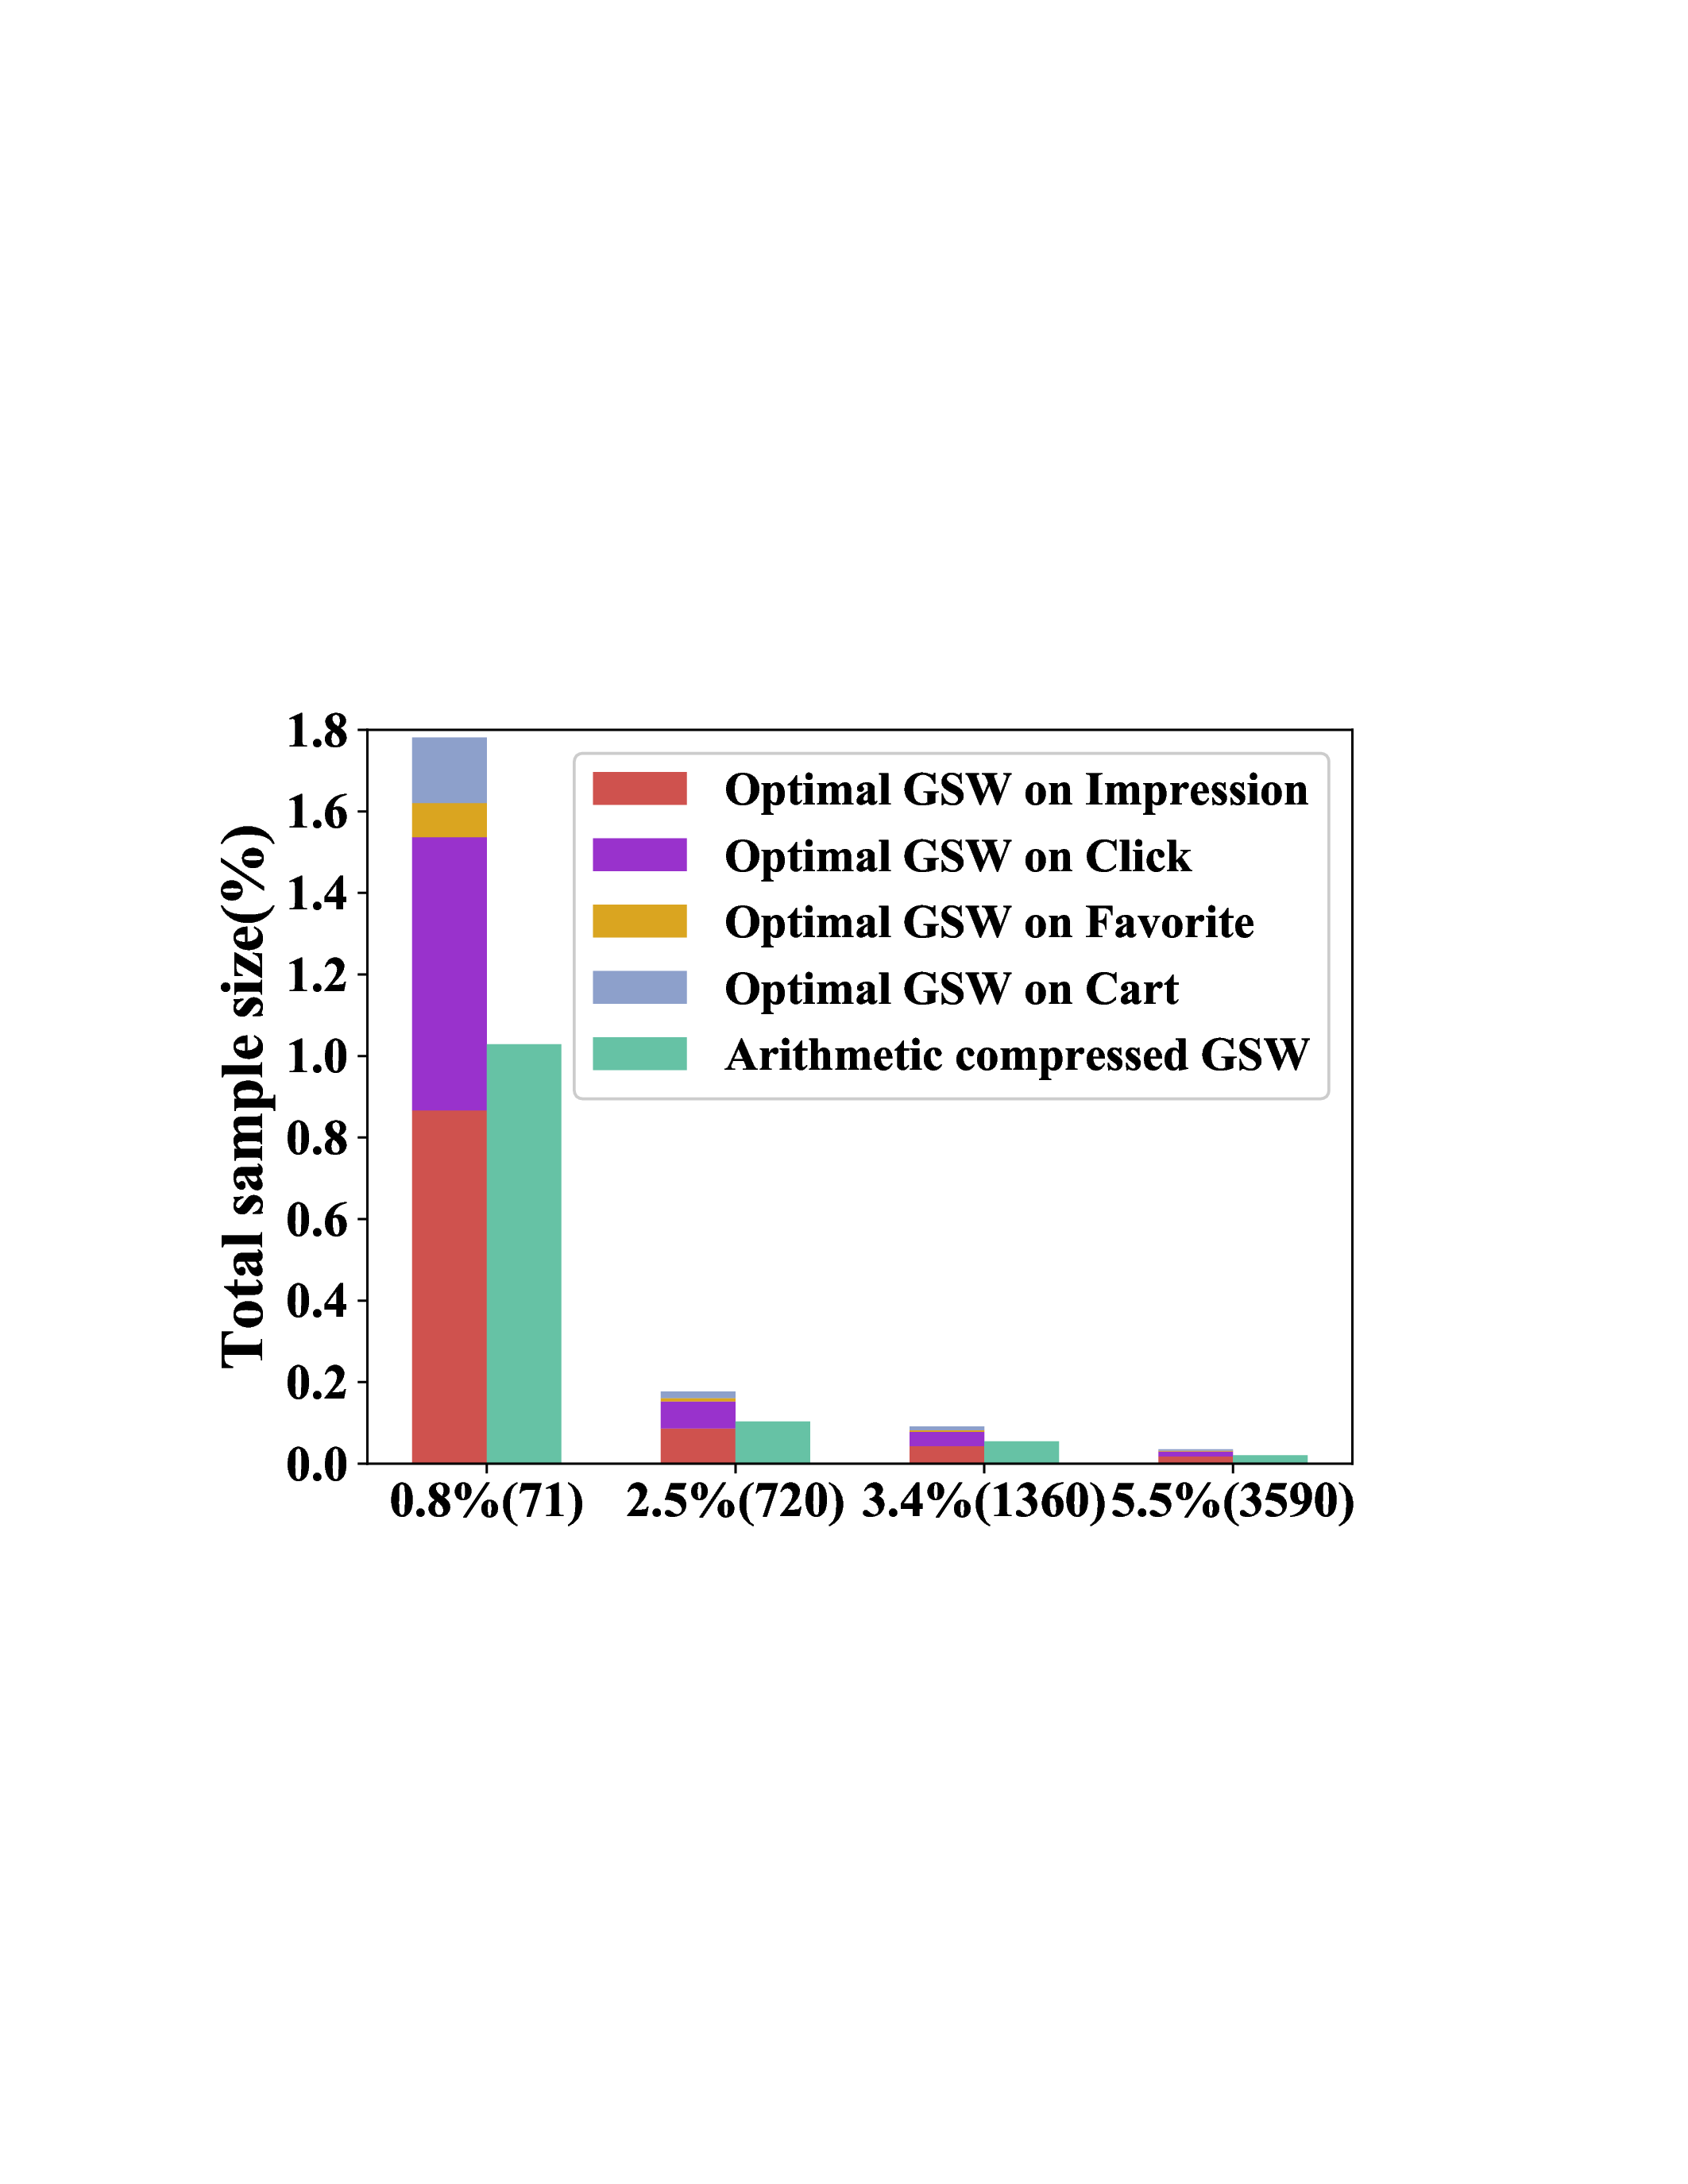}
% \label{fig:side:a}
\end{minipage}
}
\subfigure[AQP Error]{
\begin{minipage}[t]{0.49\linewidth}
\centering
\includegraphics[width=2.2in, height=2.0in]{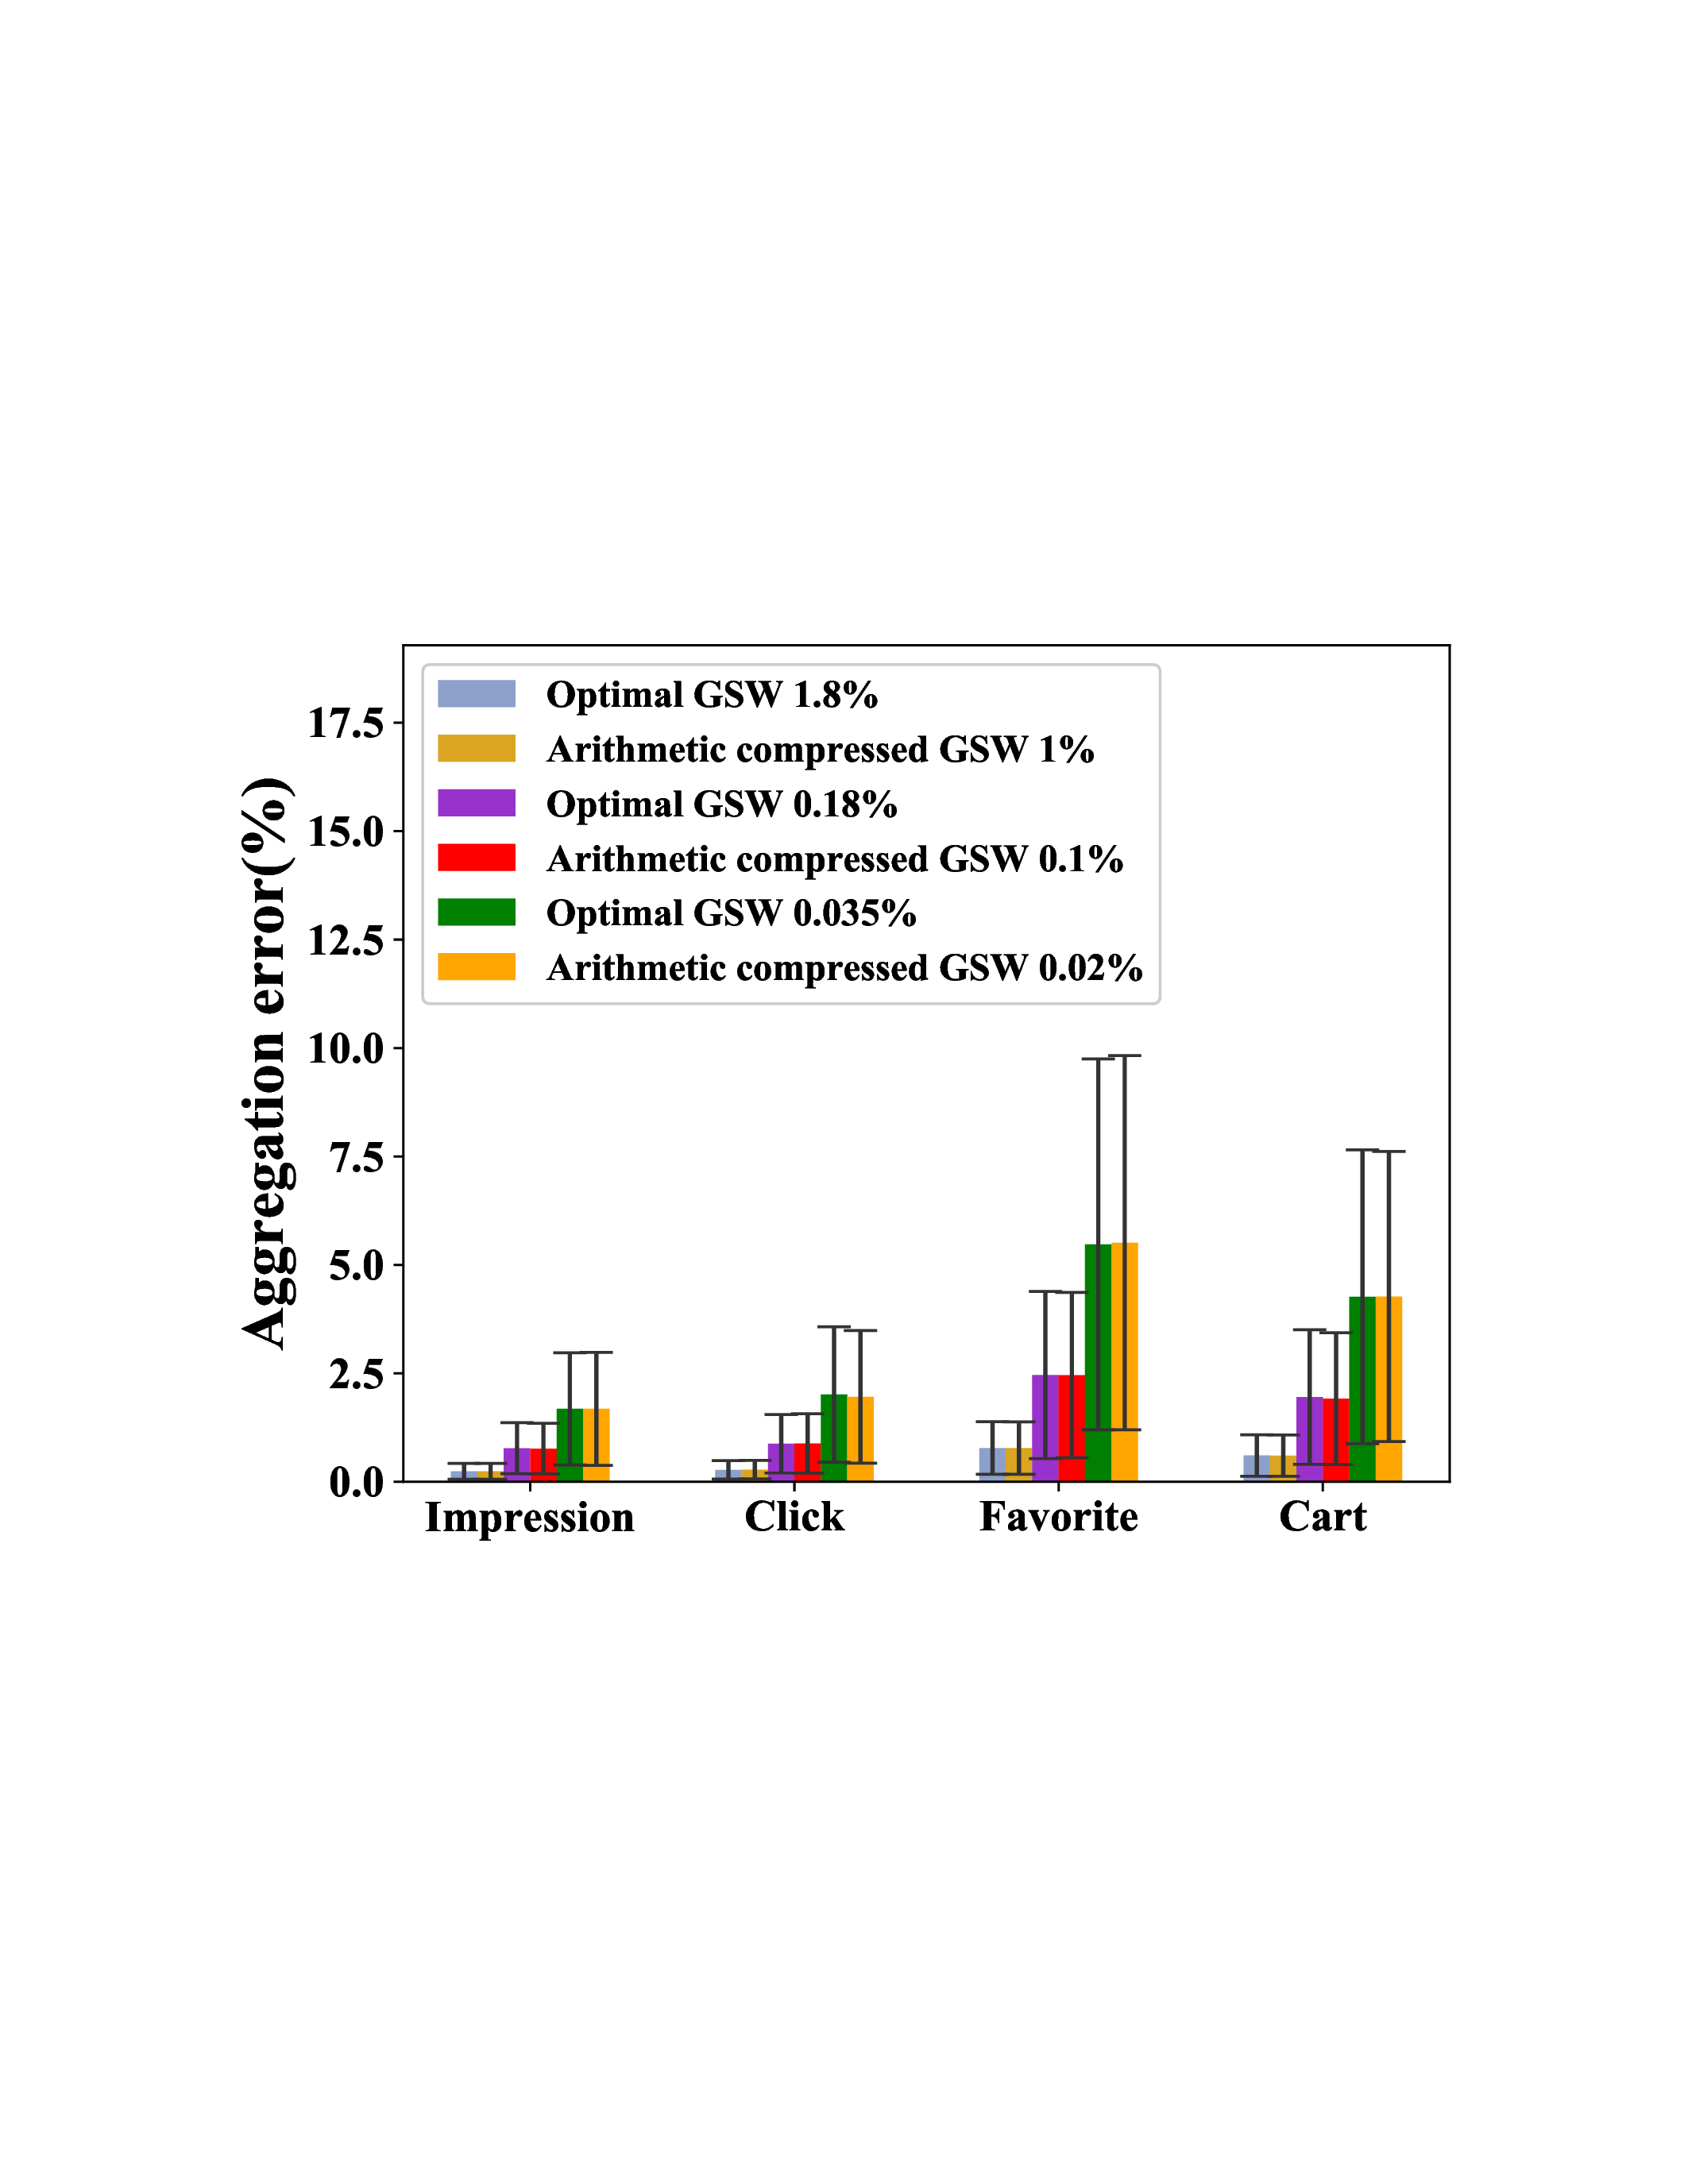}
\end{minipage}
}
\caption{Sampling rate via different sampling methods with nearly aqp error bound (can we add uniform and geometric-mean here?)}
% \label{AQP and ARIMA Performance}
\end{figure*}
%---------end-------------

%%

%-----fig14. predict relative error when binomial sampling aqp error bound close to compressed-arithmetic-mean sampling----------
\eat{
\begin{figure*}[ht]
\subfigure[Selectivity 0.5\%]{
\begin{minipage}[t]{0.33\linewidth}
\centering
\includegraphics[width=2.2in, height=2in]{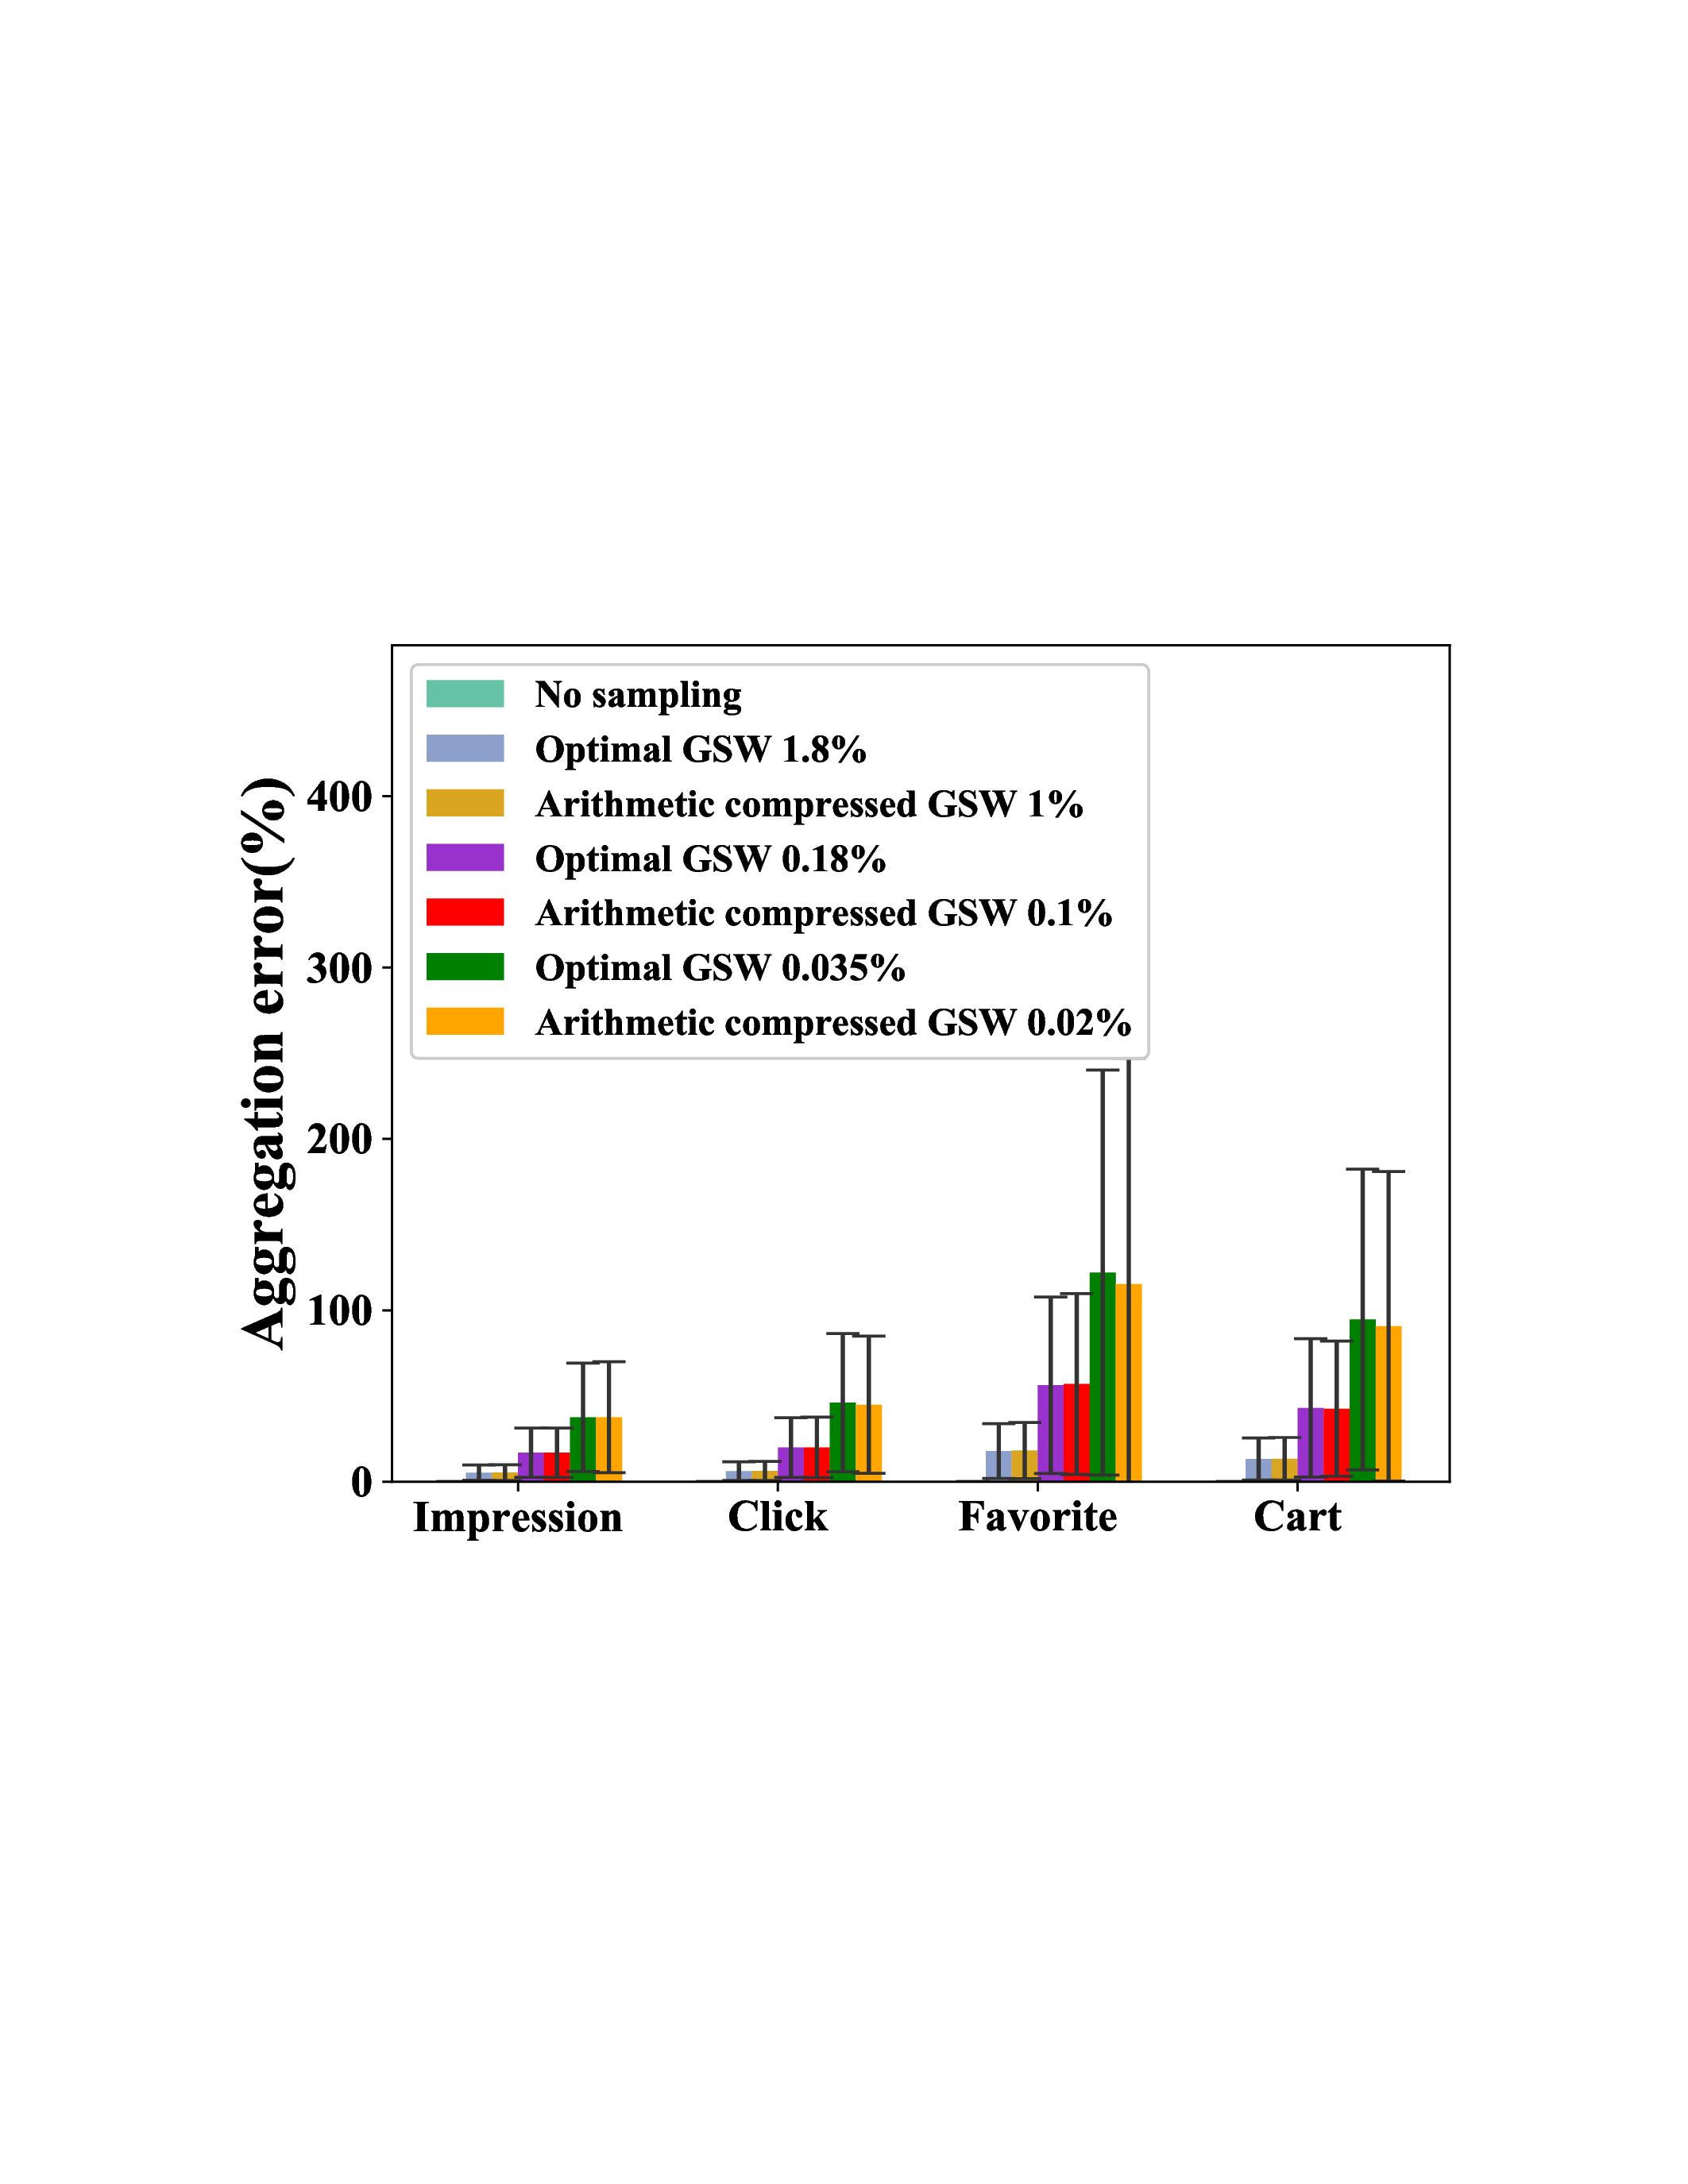}
% \label{fig:side:a}
\end{minipage}
}
\subfigure[Selectivity 1\%]{
\begin{minipage}[t]{0.33\linewidth}
\centering
\includegraphics[width=2.2in, height=2in]{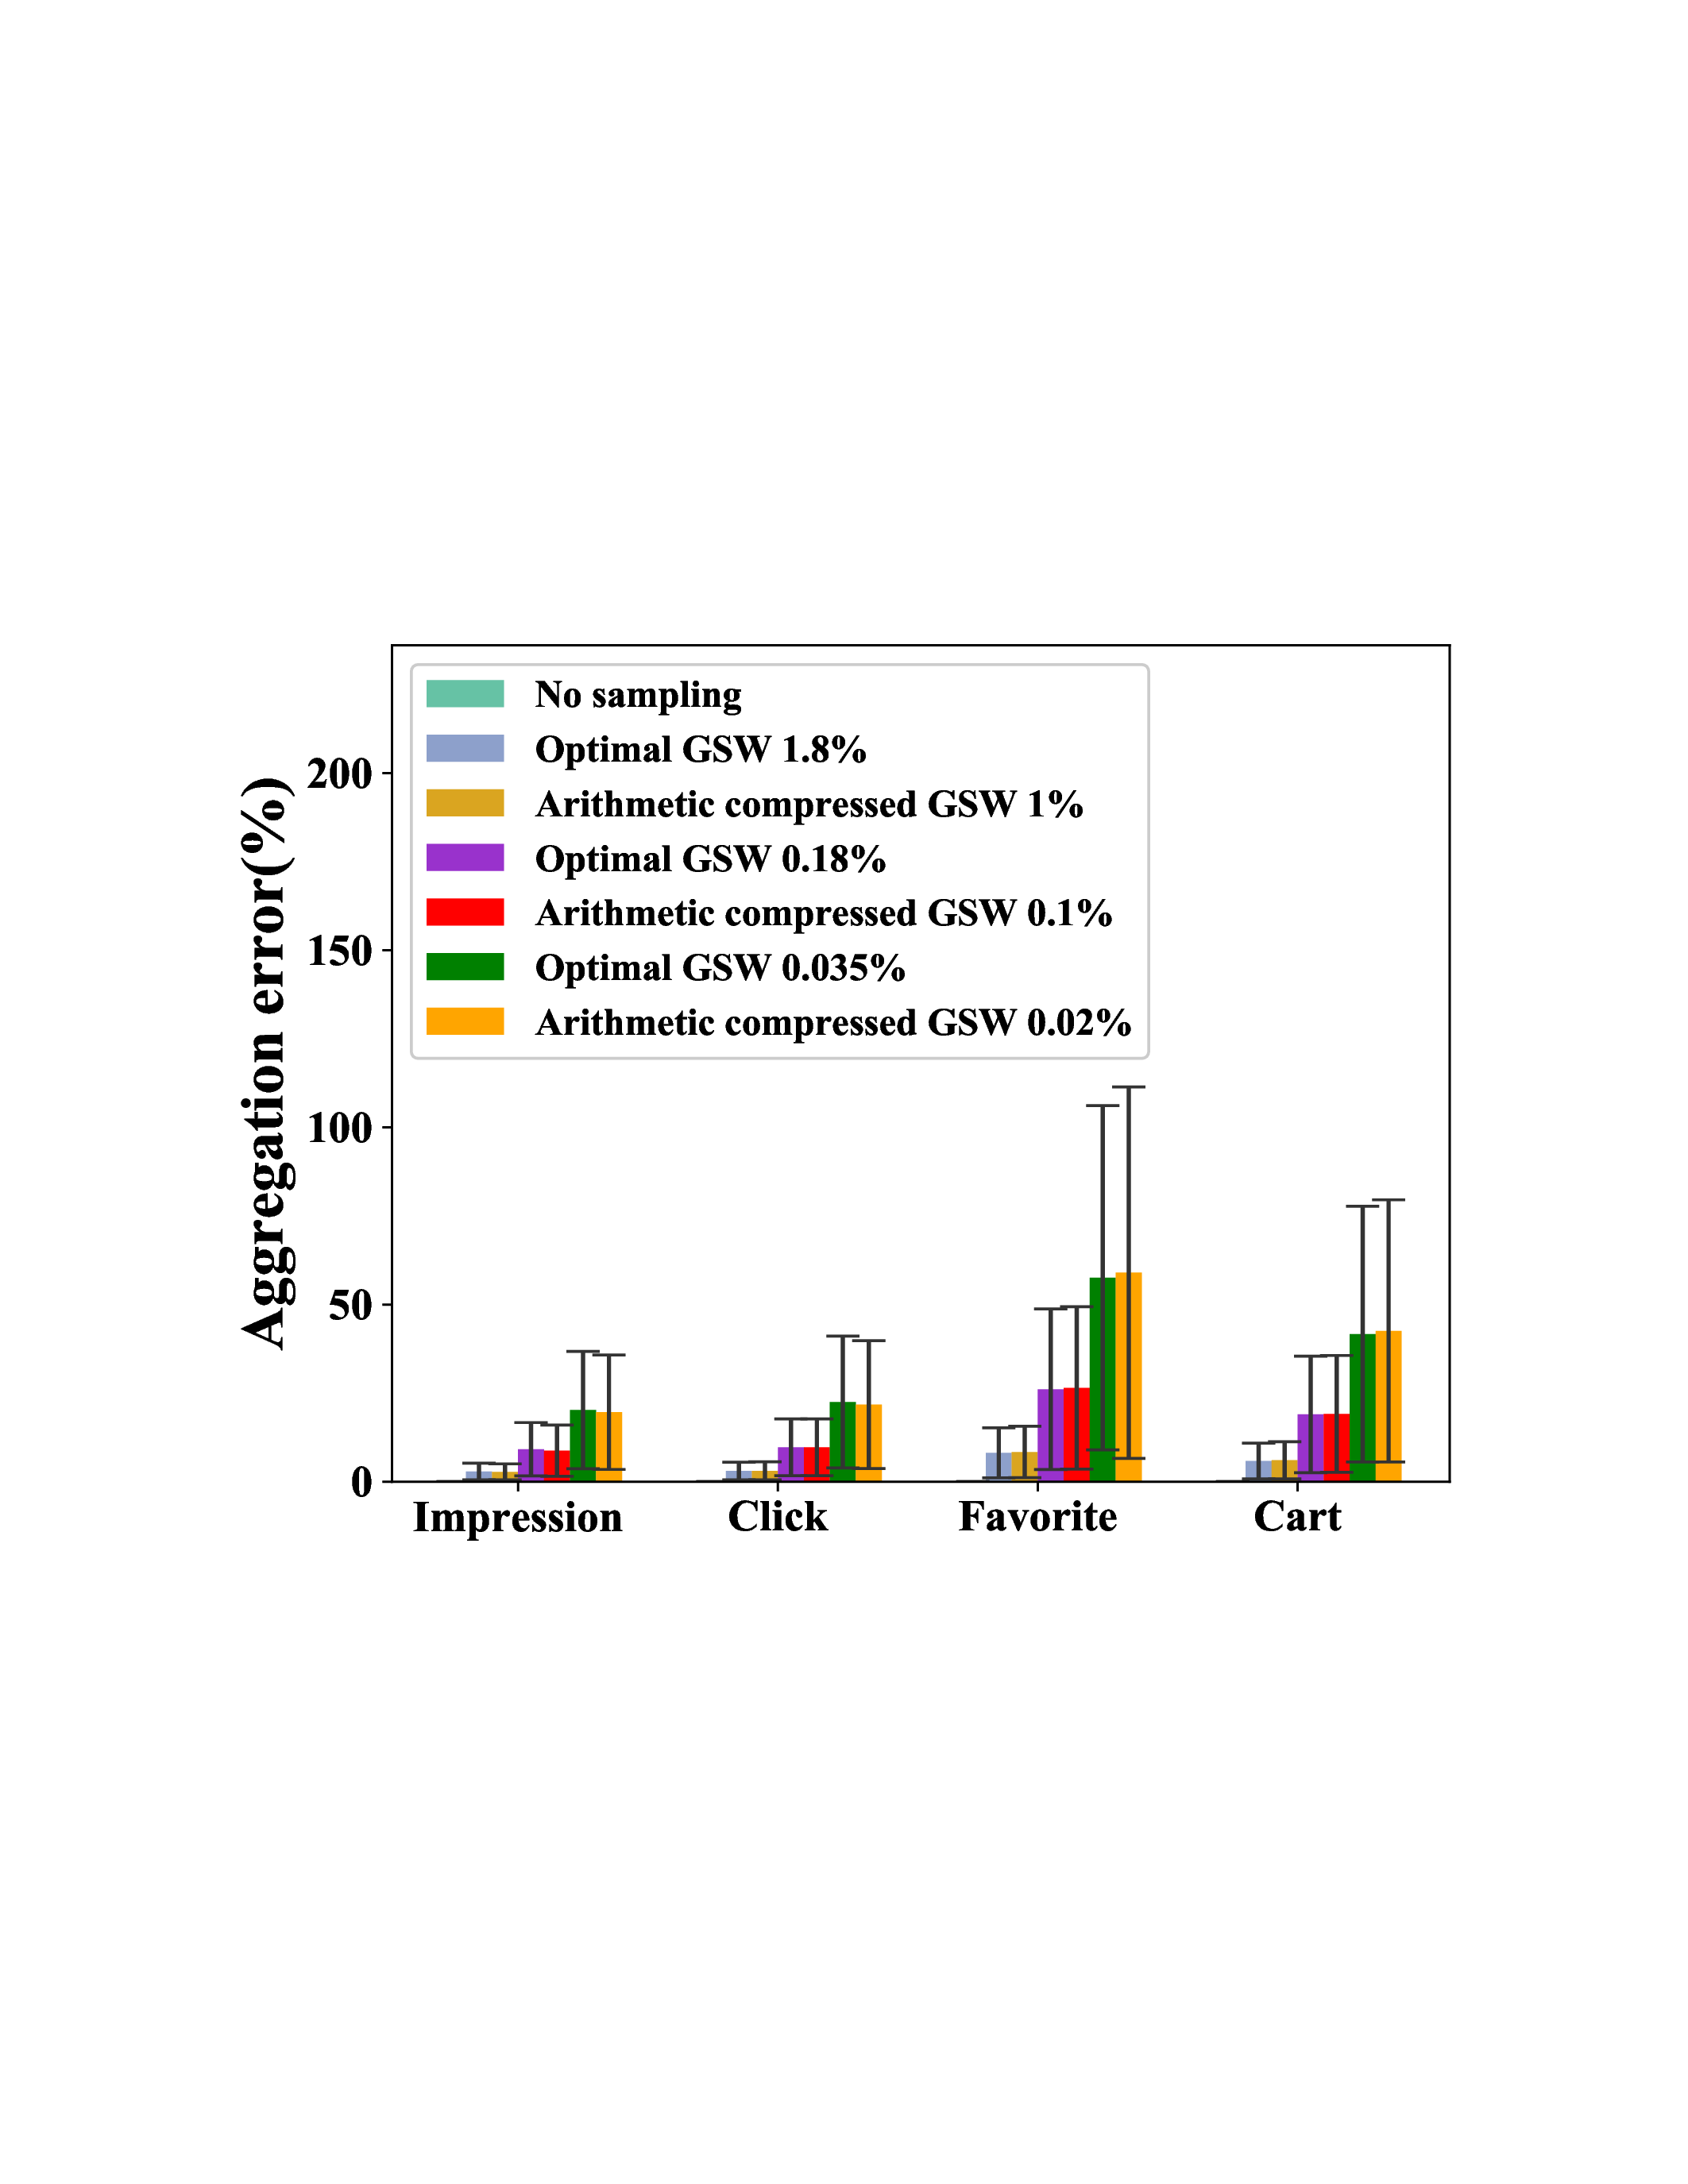}
\end{minipage}
}
\subfigure[Selectivity 5\%]{
\begin{minipage}[t]{0.33\linewidth}
\centering
\includegraphics[width=2.2in, height=2in]{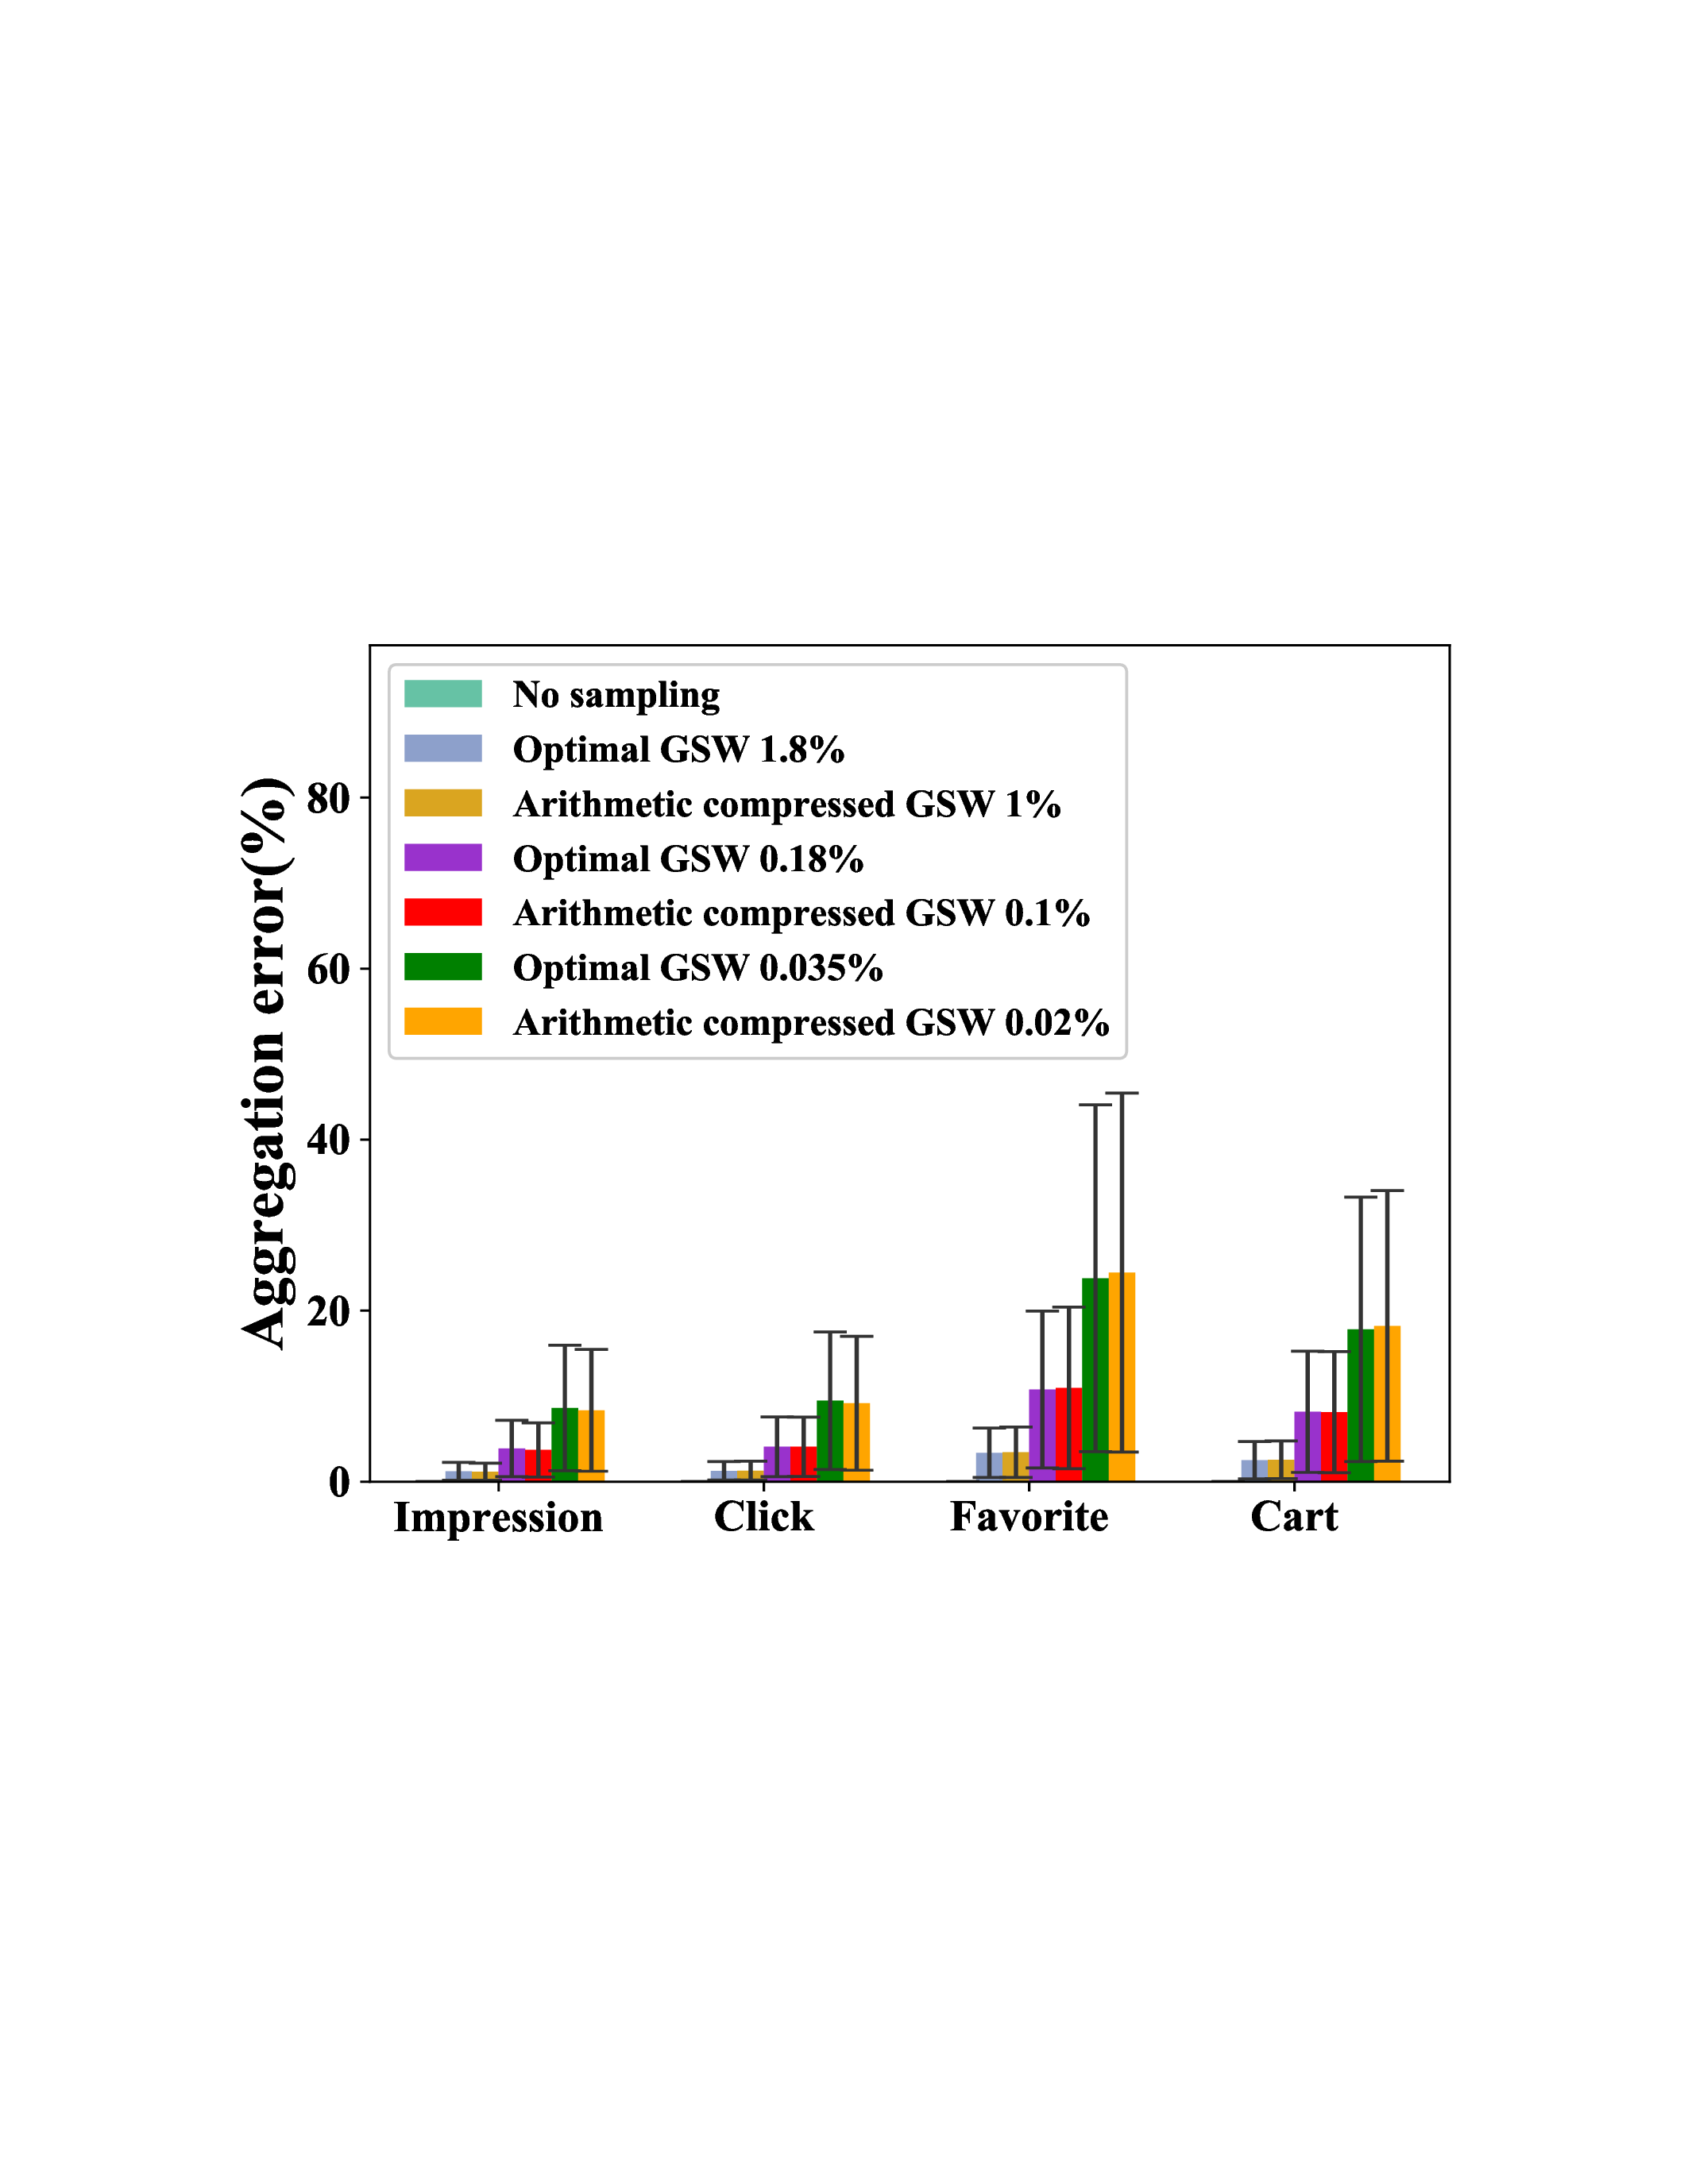}
\end{minipage}
}
\caption{ARIMA aqp error with different selectivity via different sampling methods with nearly aqp error bound (can we add uniform and geometric-mean here? almost no change for different sampling rates? how can we guarantee that aqp error bounds are nearly the same given the same sampling rate?)}
% \label{AQP and ARIMA Performance}
\end{figure*}
}

%-----fig14. predict relative error when binomial sampling aqp error bound close to compressed-arithmetic-mean sampling----------
\begin{figure*}[ht]
\subfigure[Selectivity 0.5\%]{
\begin{minipage}[t]{0.33\linewidth}
\centering
\includegraphics[width=2.2in, height=2in]{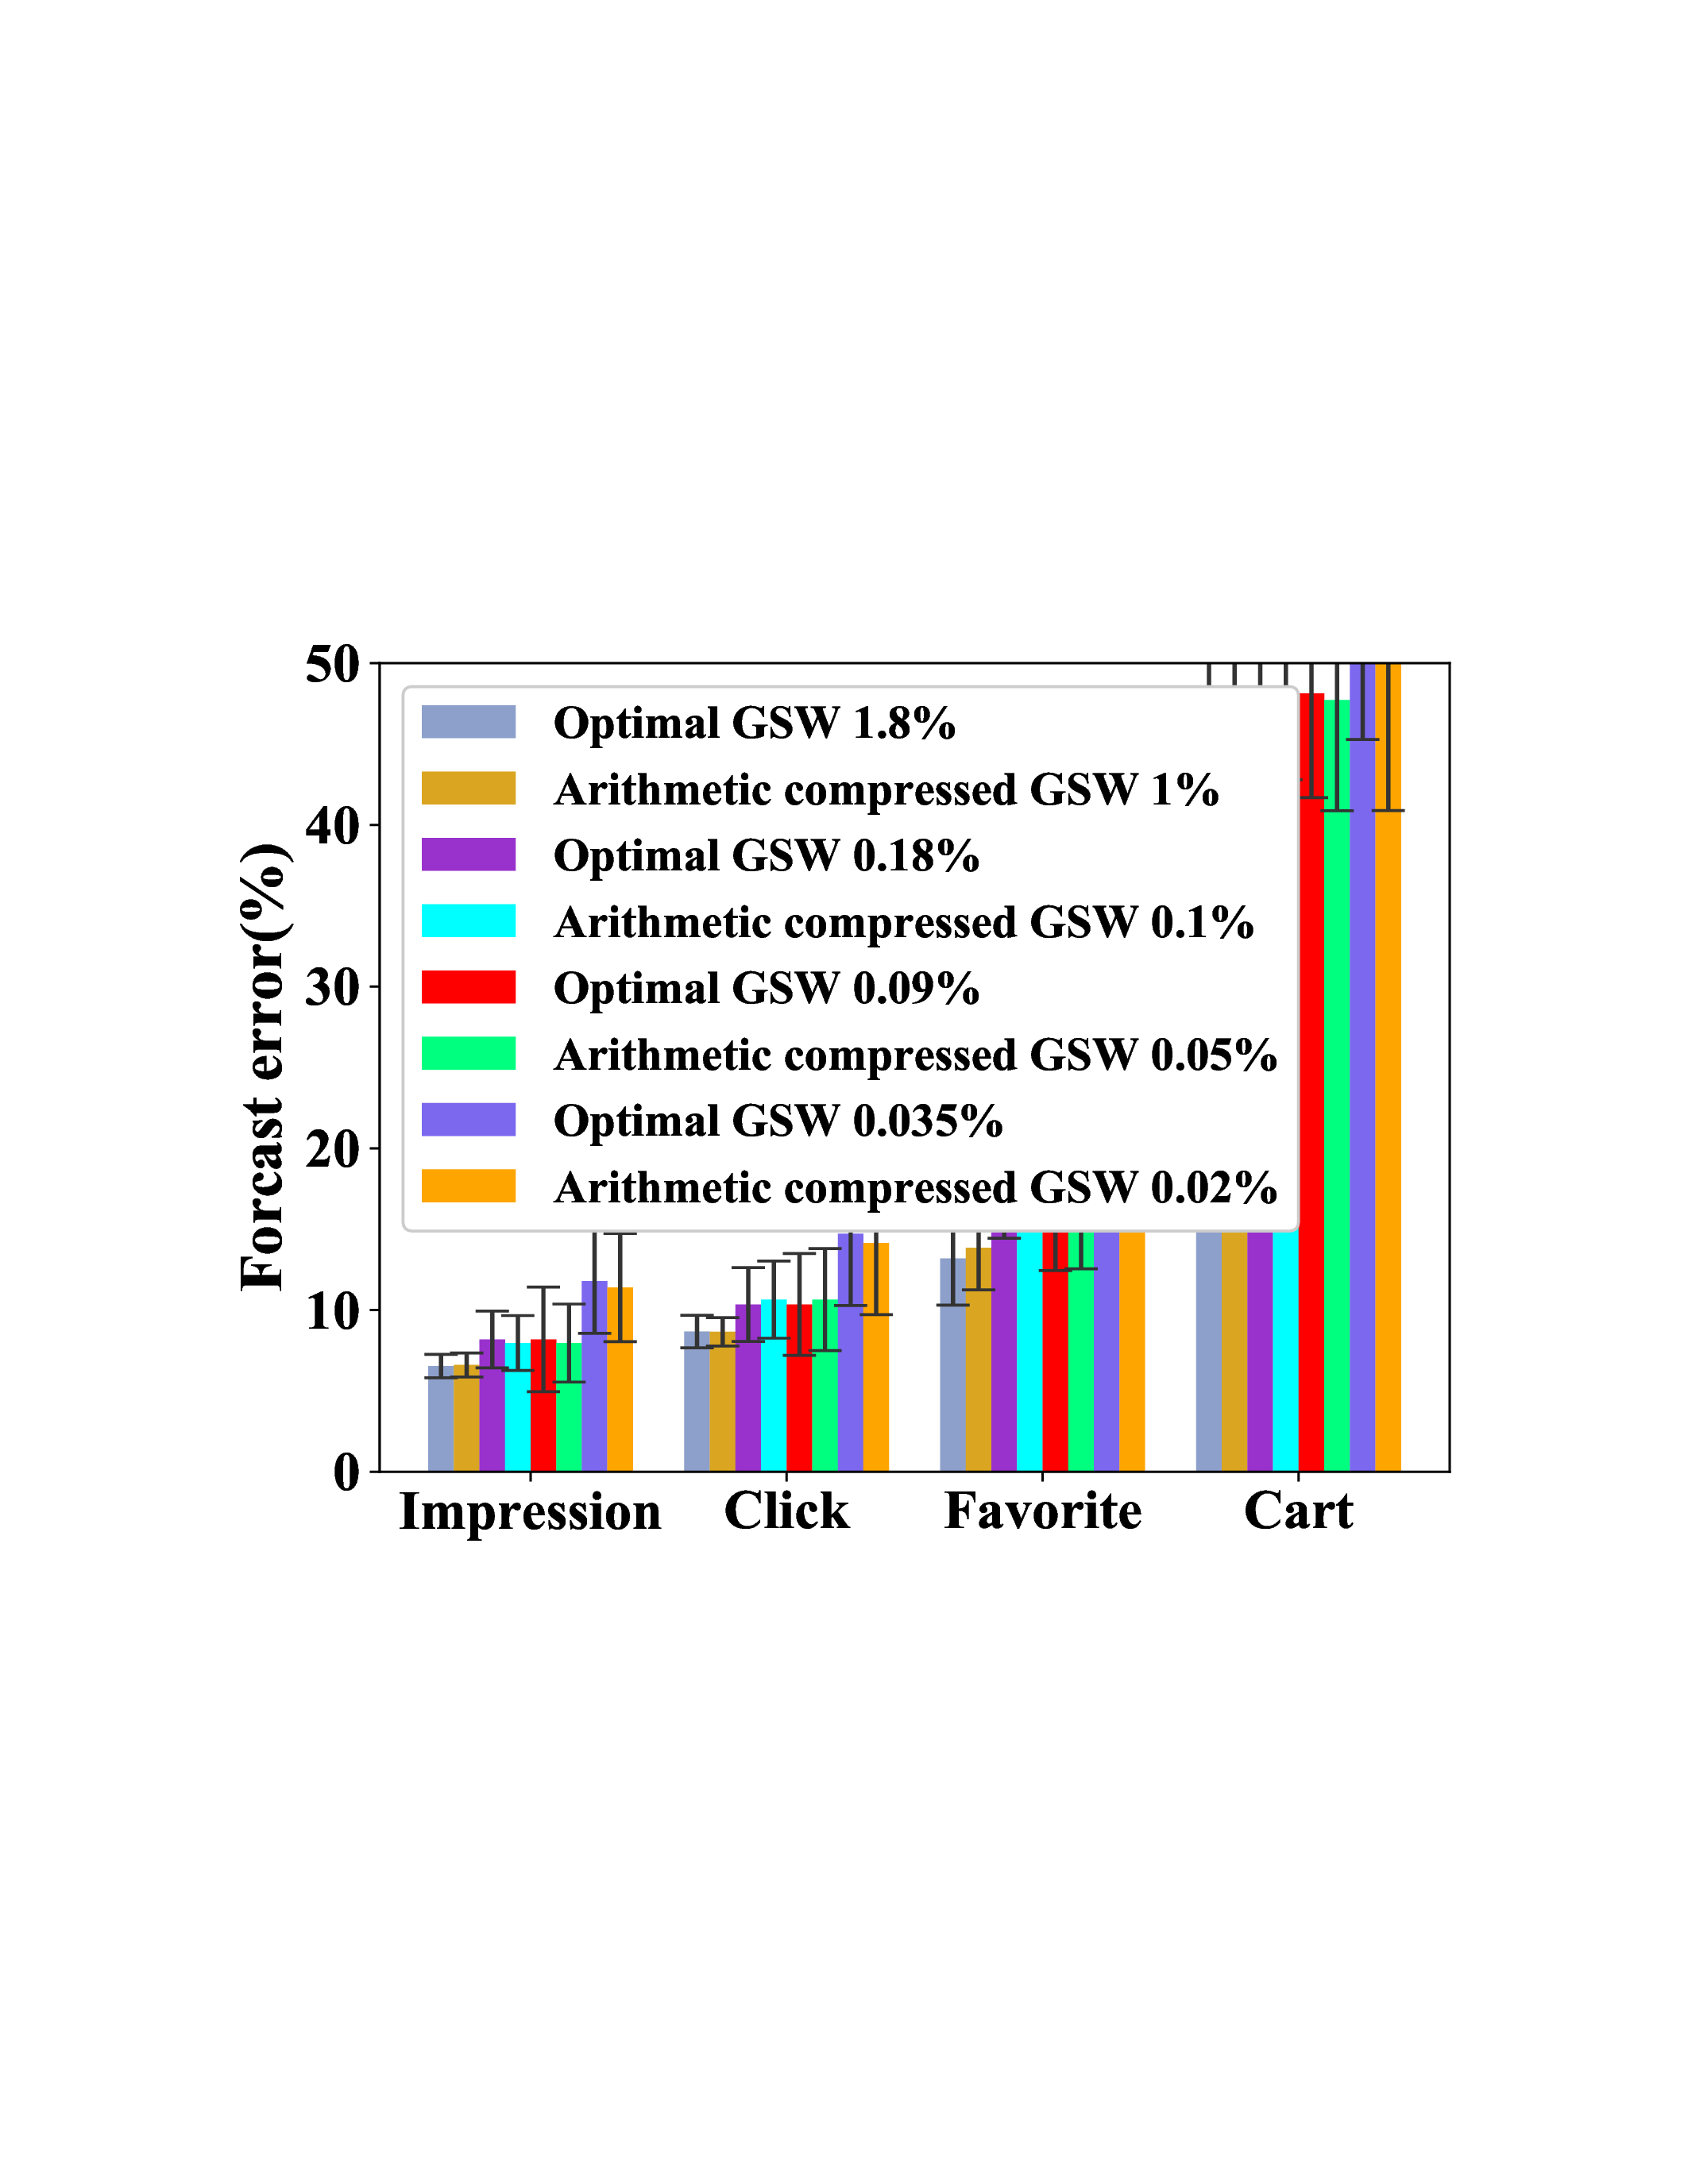}
% \label{fig:side:a}
\end{minipage}
}
\subfigure[Selectivity 1\%]{
\begin{minipage}[t]{0.33\linewidth}
\centering
\includegraphics[width=2.2in, height=2in]{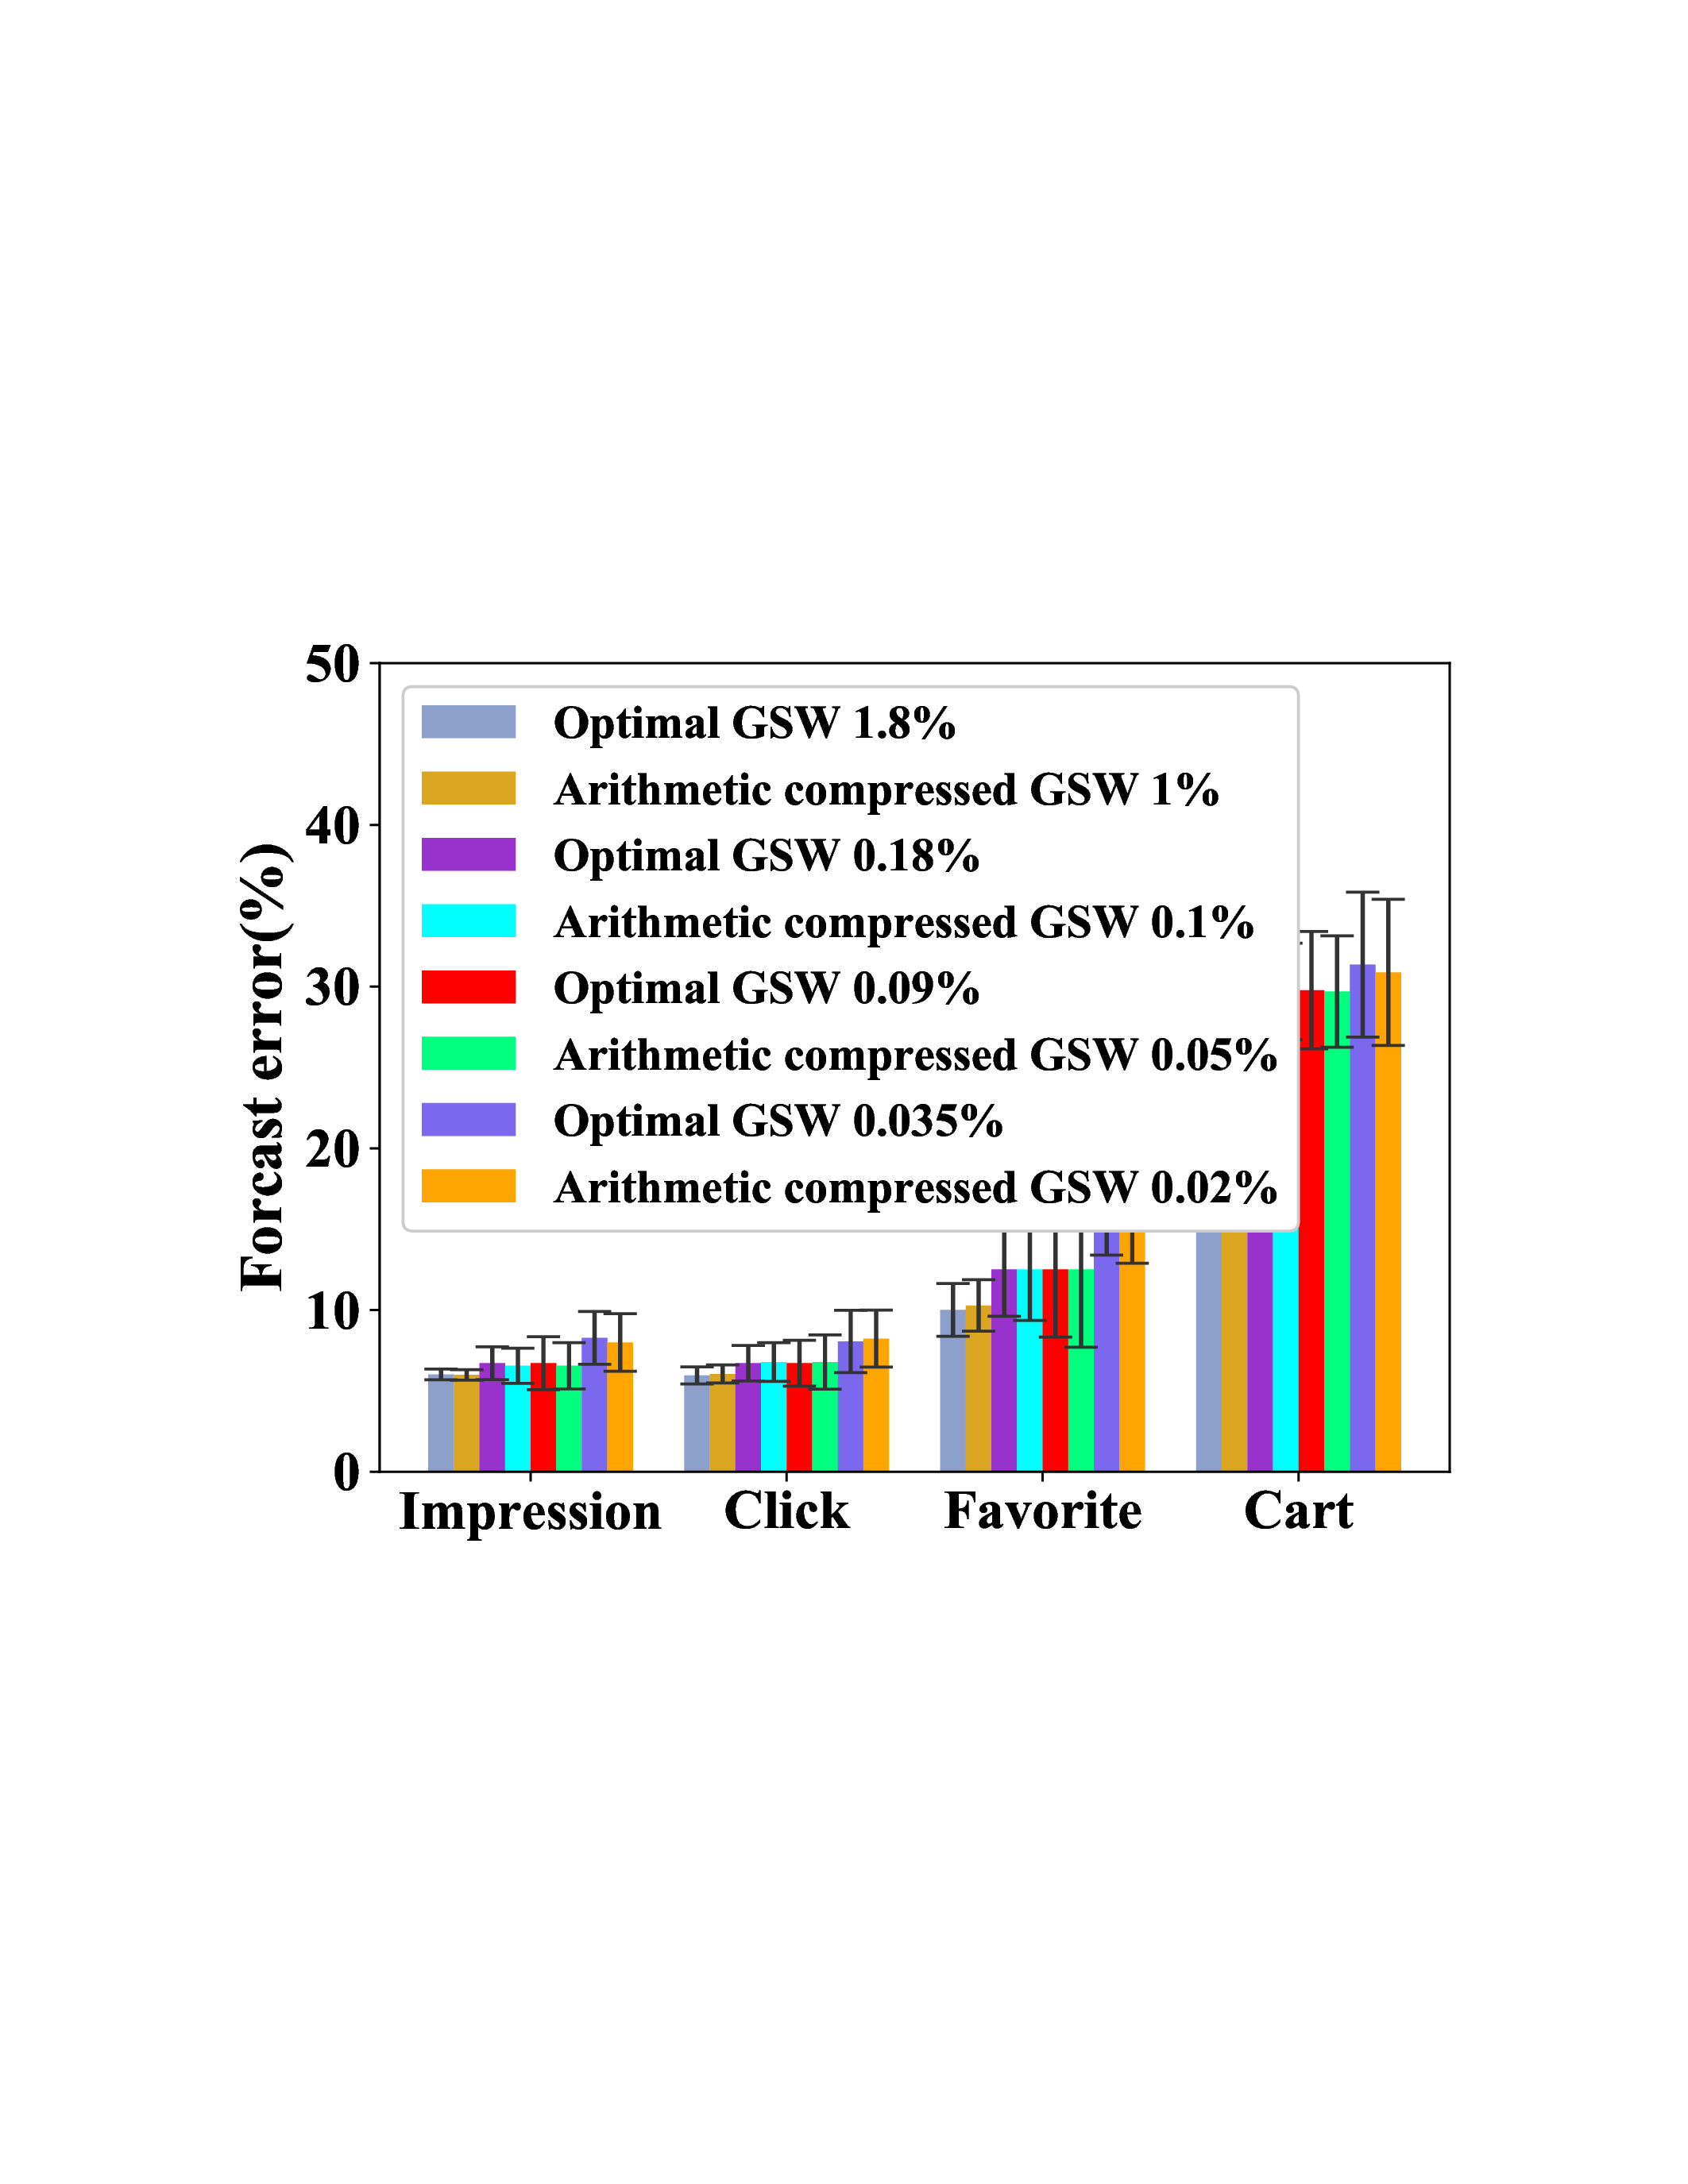}
\end{minipage}
}
\subfigure[Selectivity 5\%]{
\begin{minipage}[t]{0.33\linewidth}
\centering
\includegraphics[width=2.2in, height=2in]{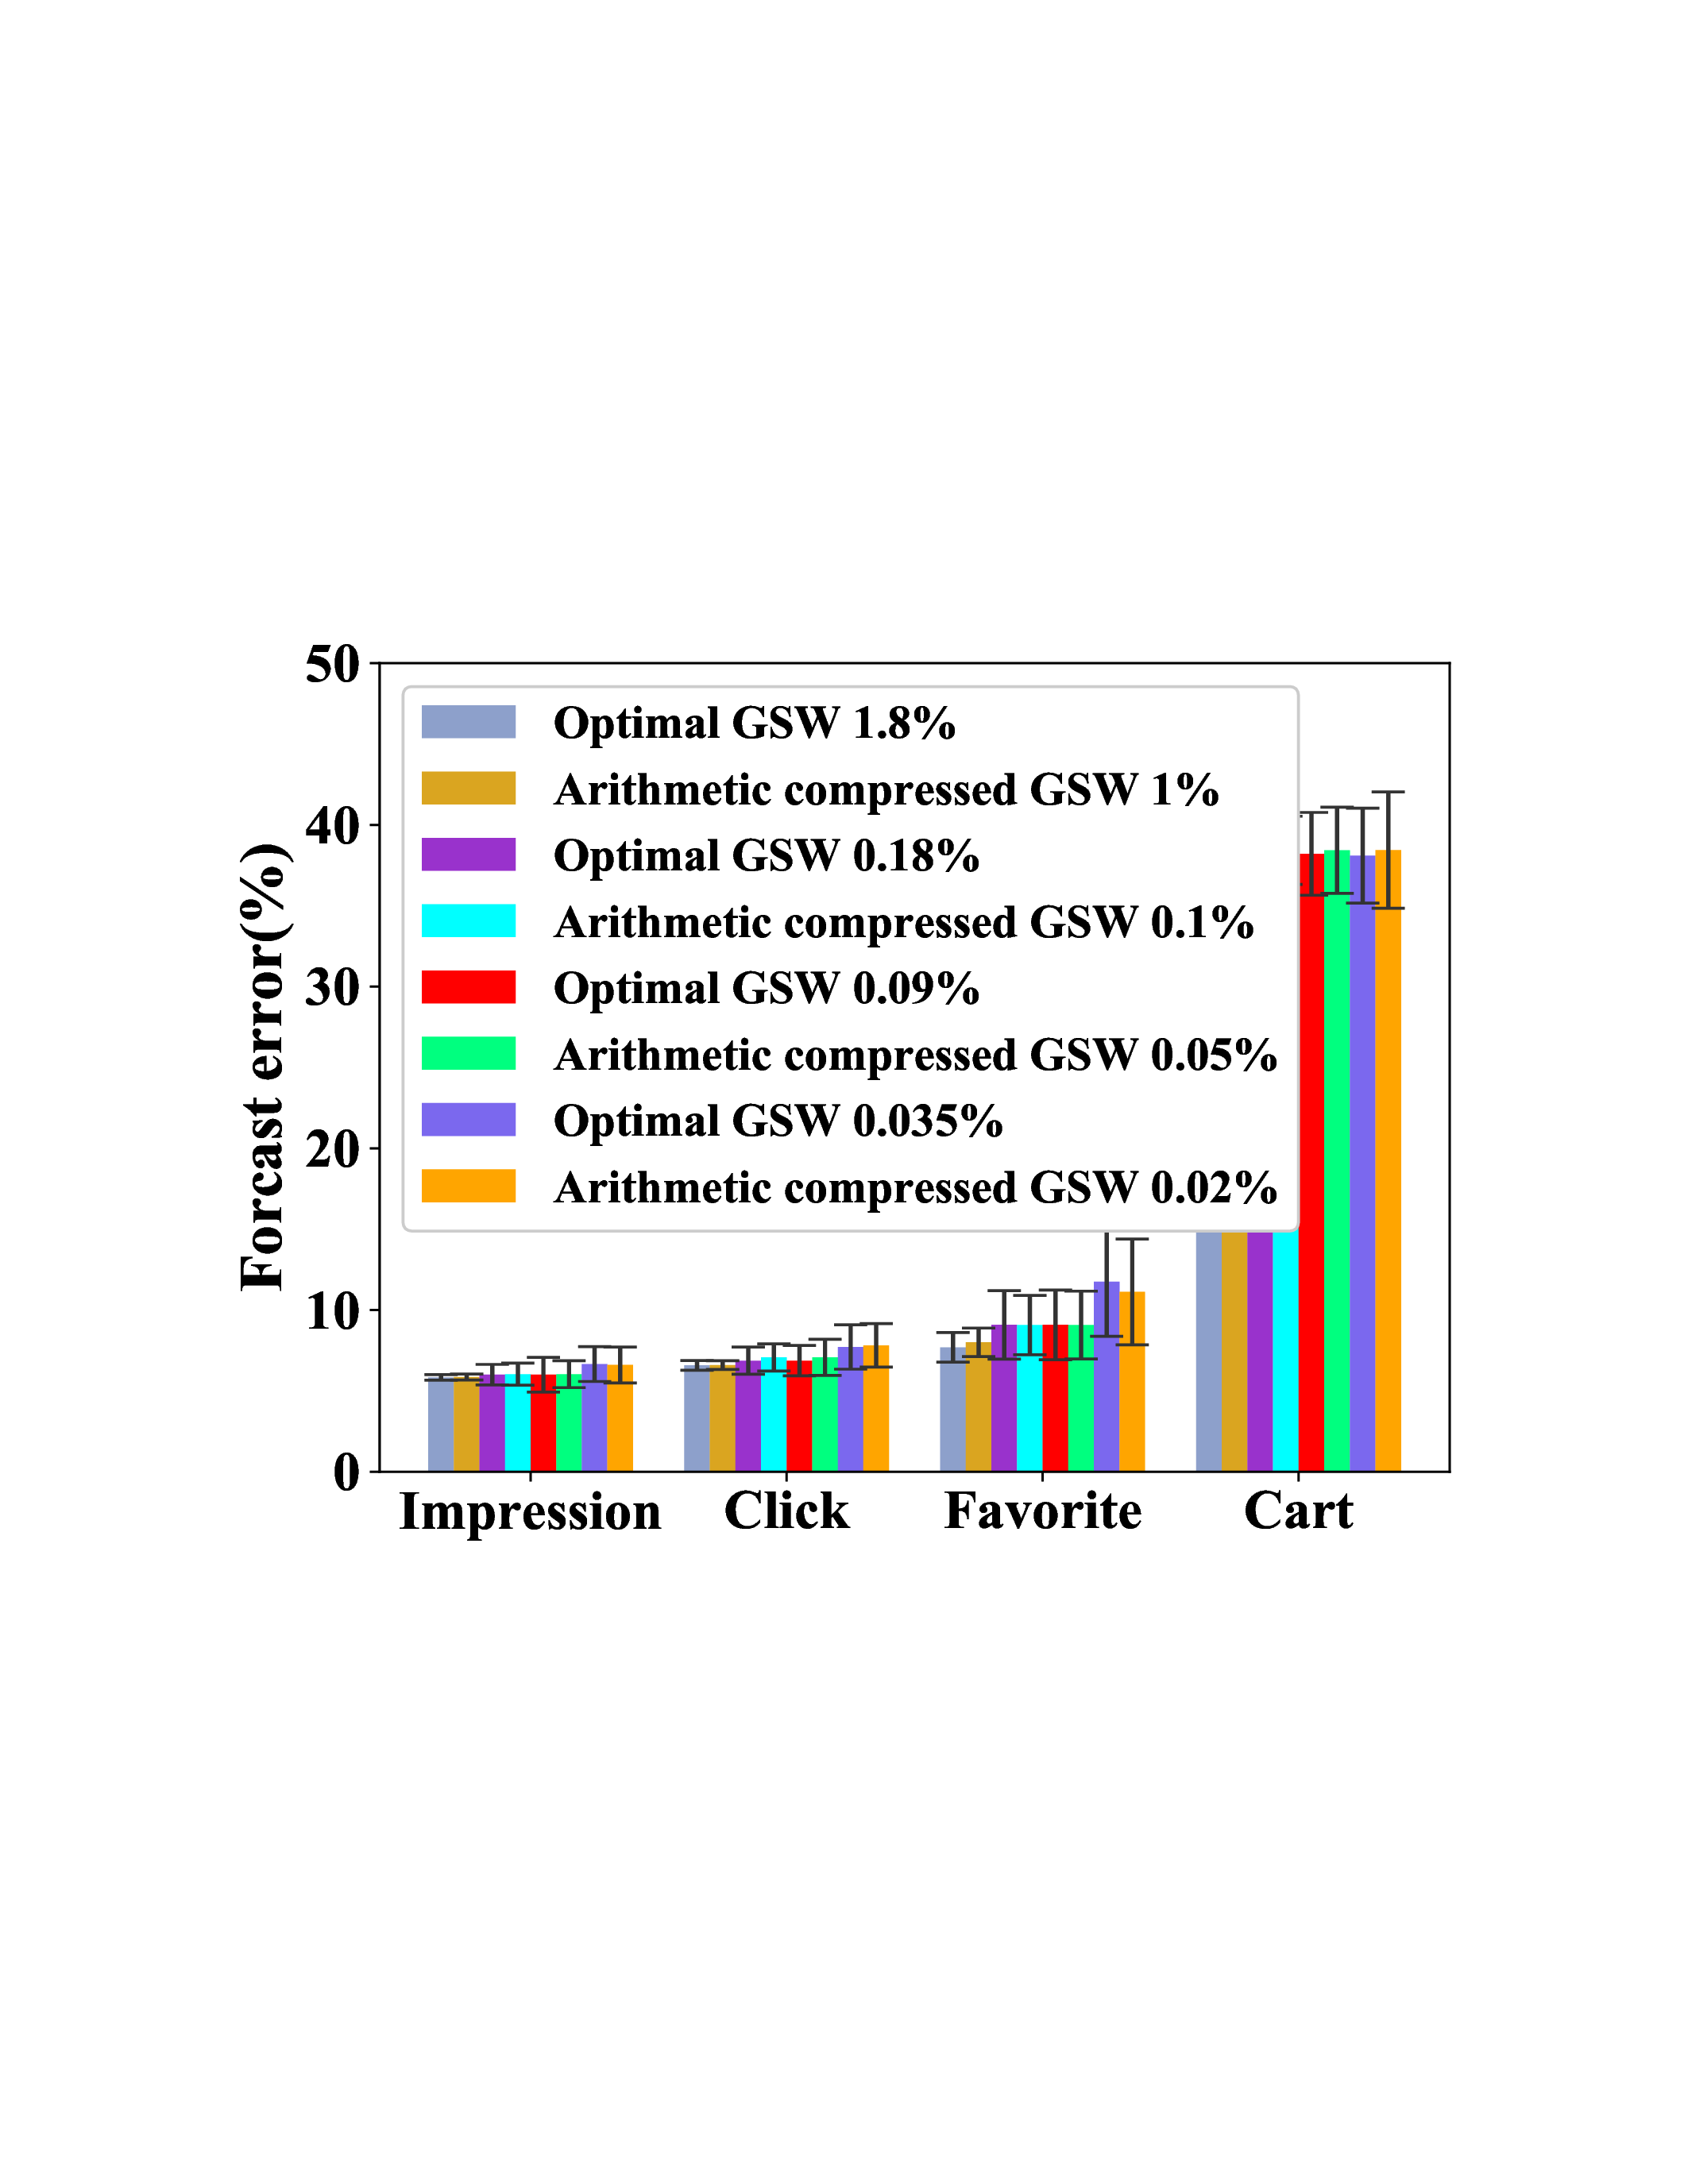}
\end{minipage}
}
\caption{ARIMA prediction error with different selectivity via different sampling methods with nearly aqp error bound (can we add uniform and geometric-mean here? almost no change for different sampling rates? how can we guarantee that aqp error bounds are nearly the same given the same sampling rate?)}
% \label{AQP and ARIMA Performance}
\end{figure*}

%---------end-------------

\begin{figure*}[ht]
\subfigure[Selectivity 0.5\%]{
\begin{minipage}[t]{0.33\linewidth}
\centering
\includegraphics[width=2.2in, height=2in]{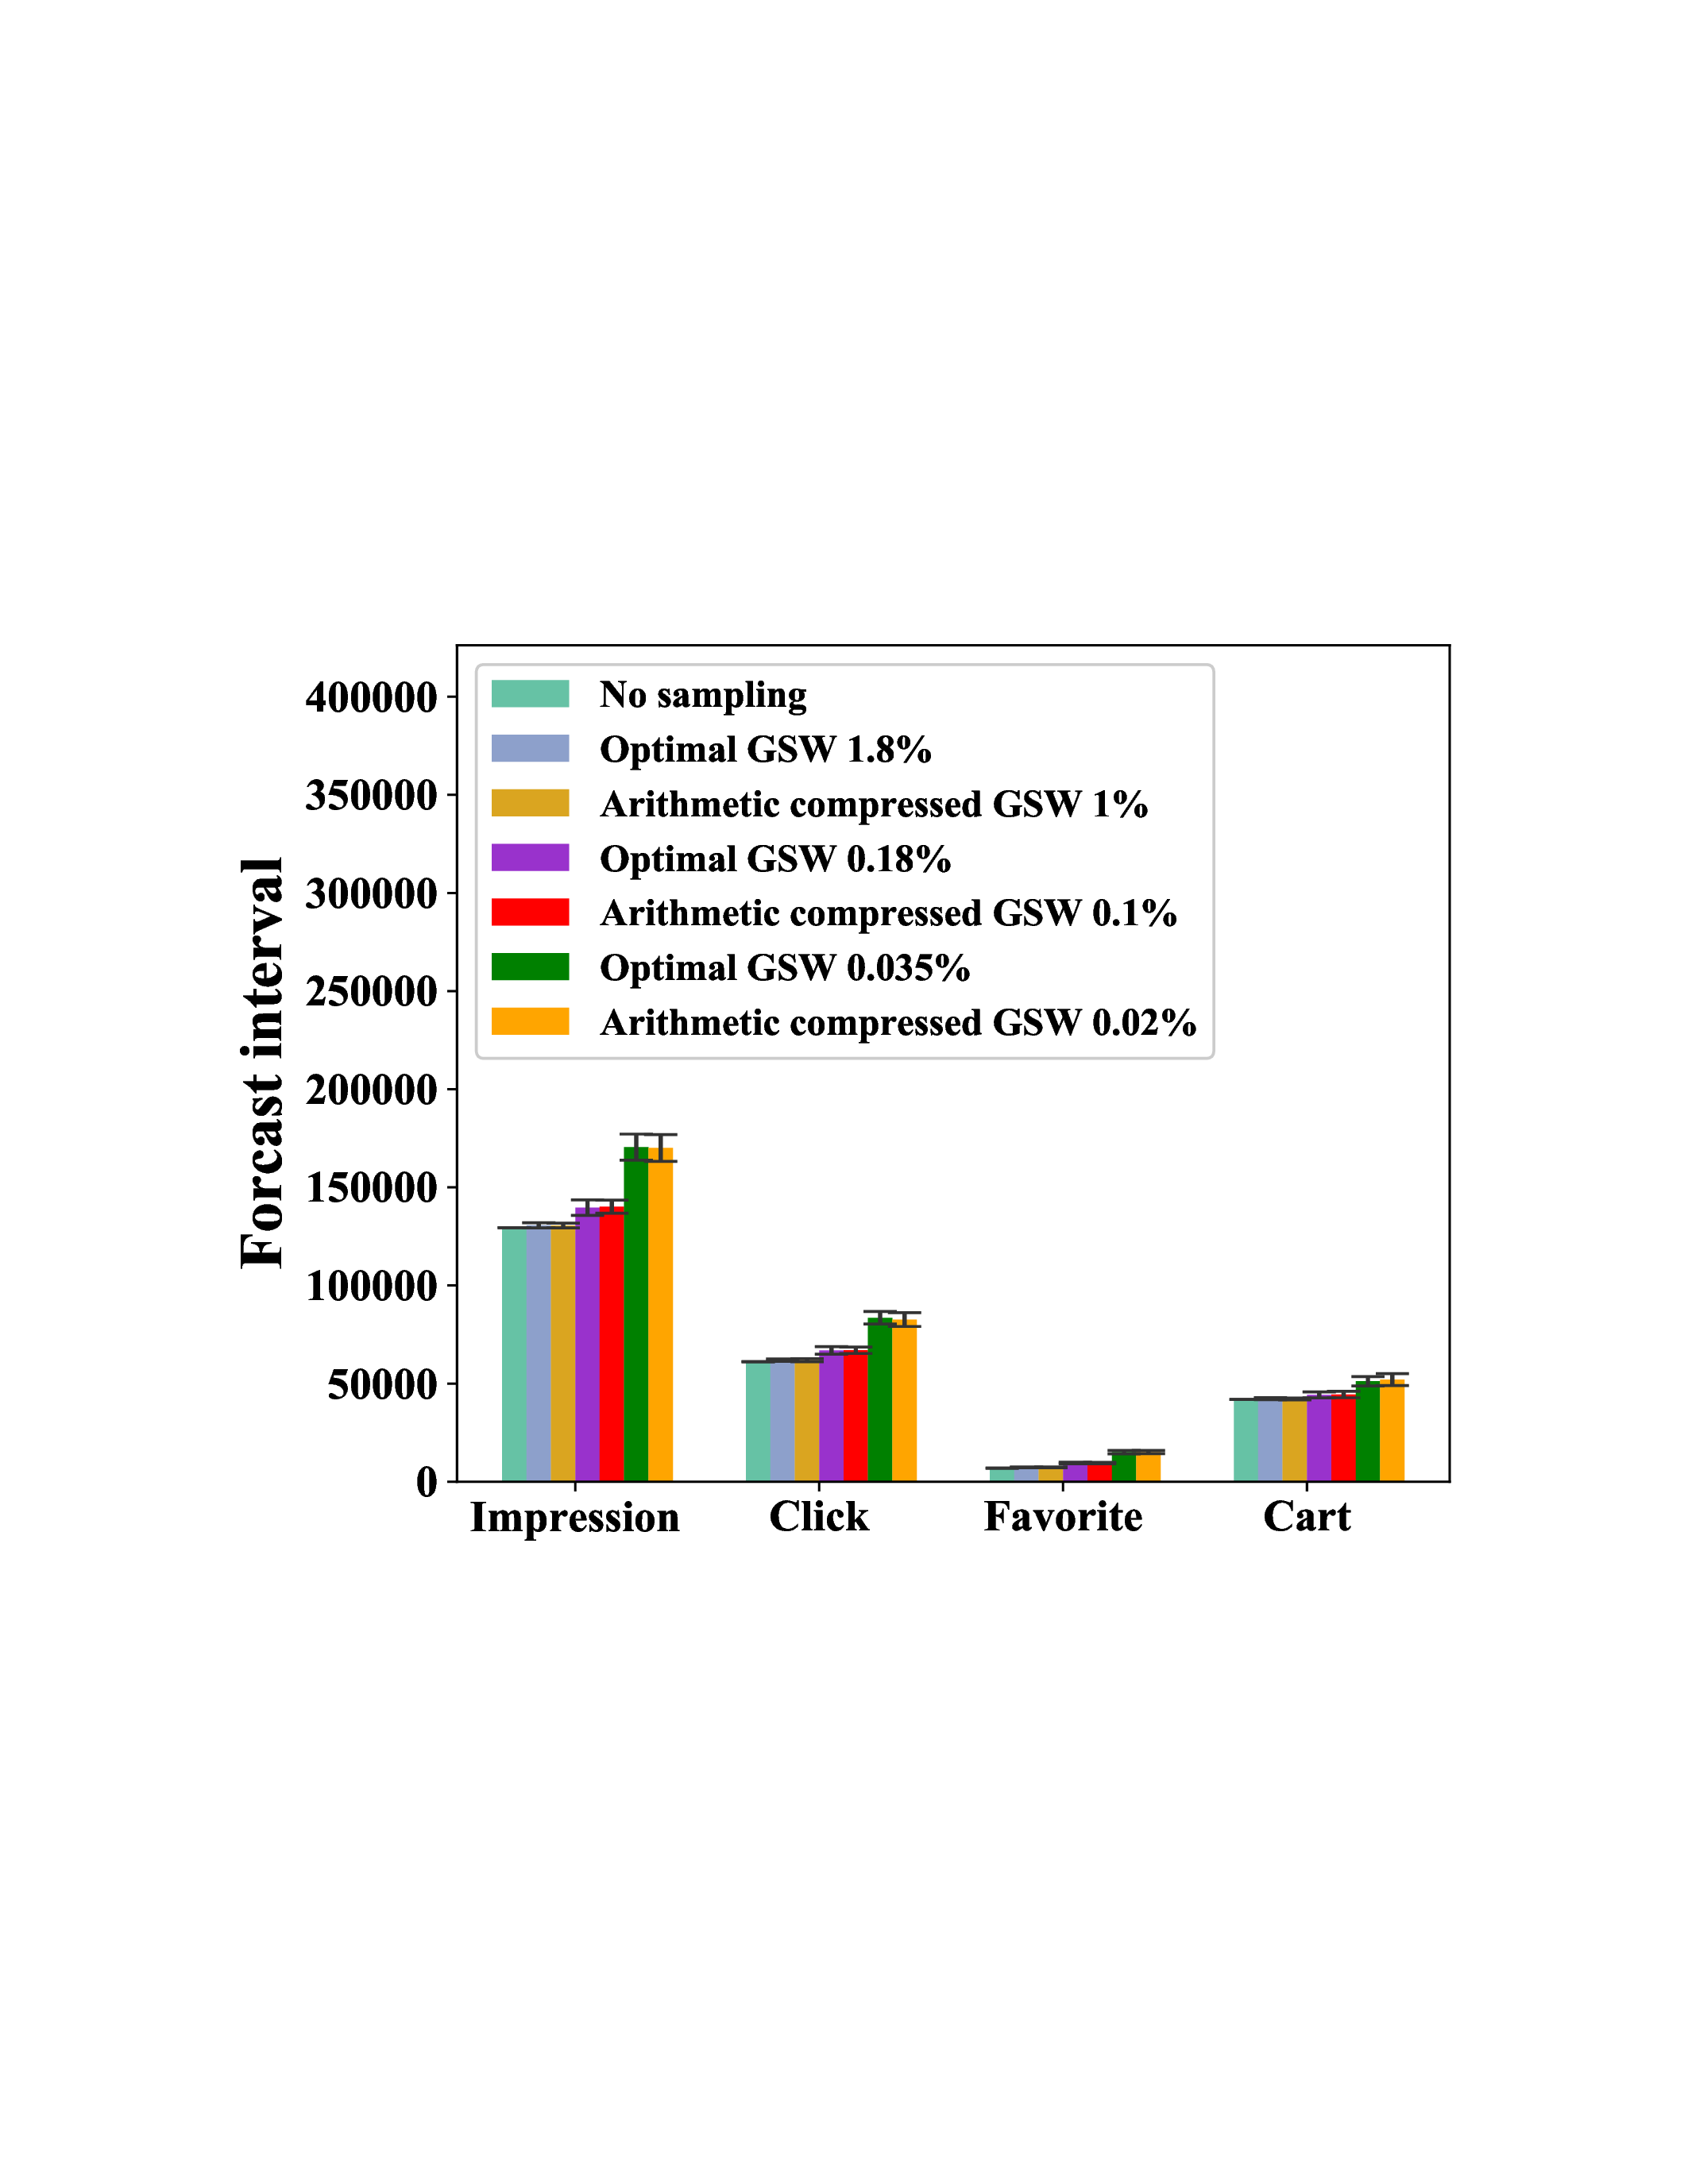}
% \label{fig:side:a}
\end{minipage}
}
\subfigure[Selectivity 1\%]{
\begin{minipage}[t]{0.33\linewidth}
\centering
\includegraphics[width=2.2in, height=2in]{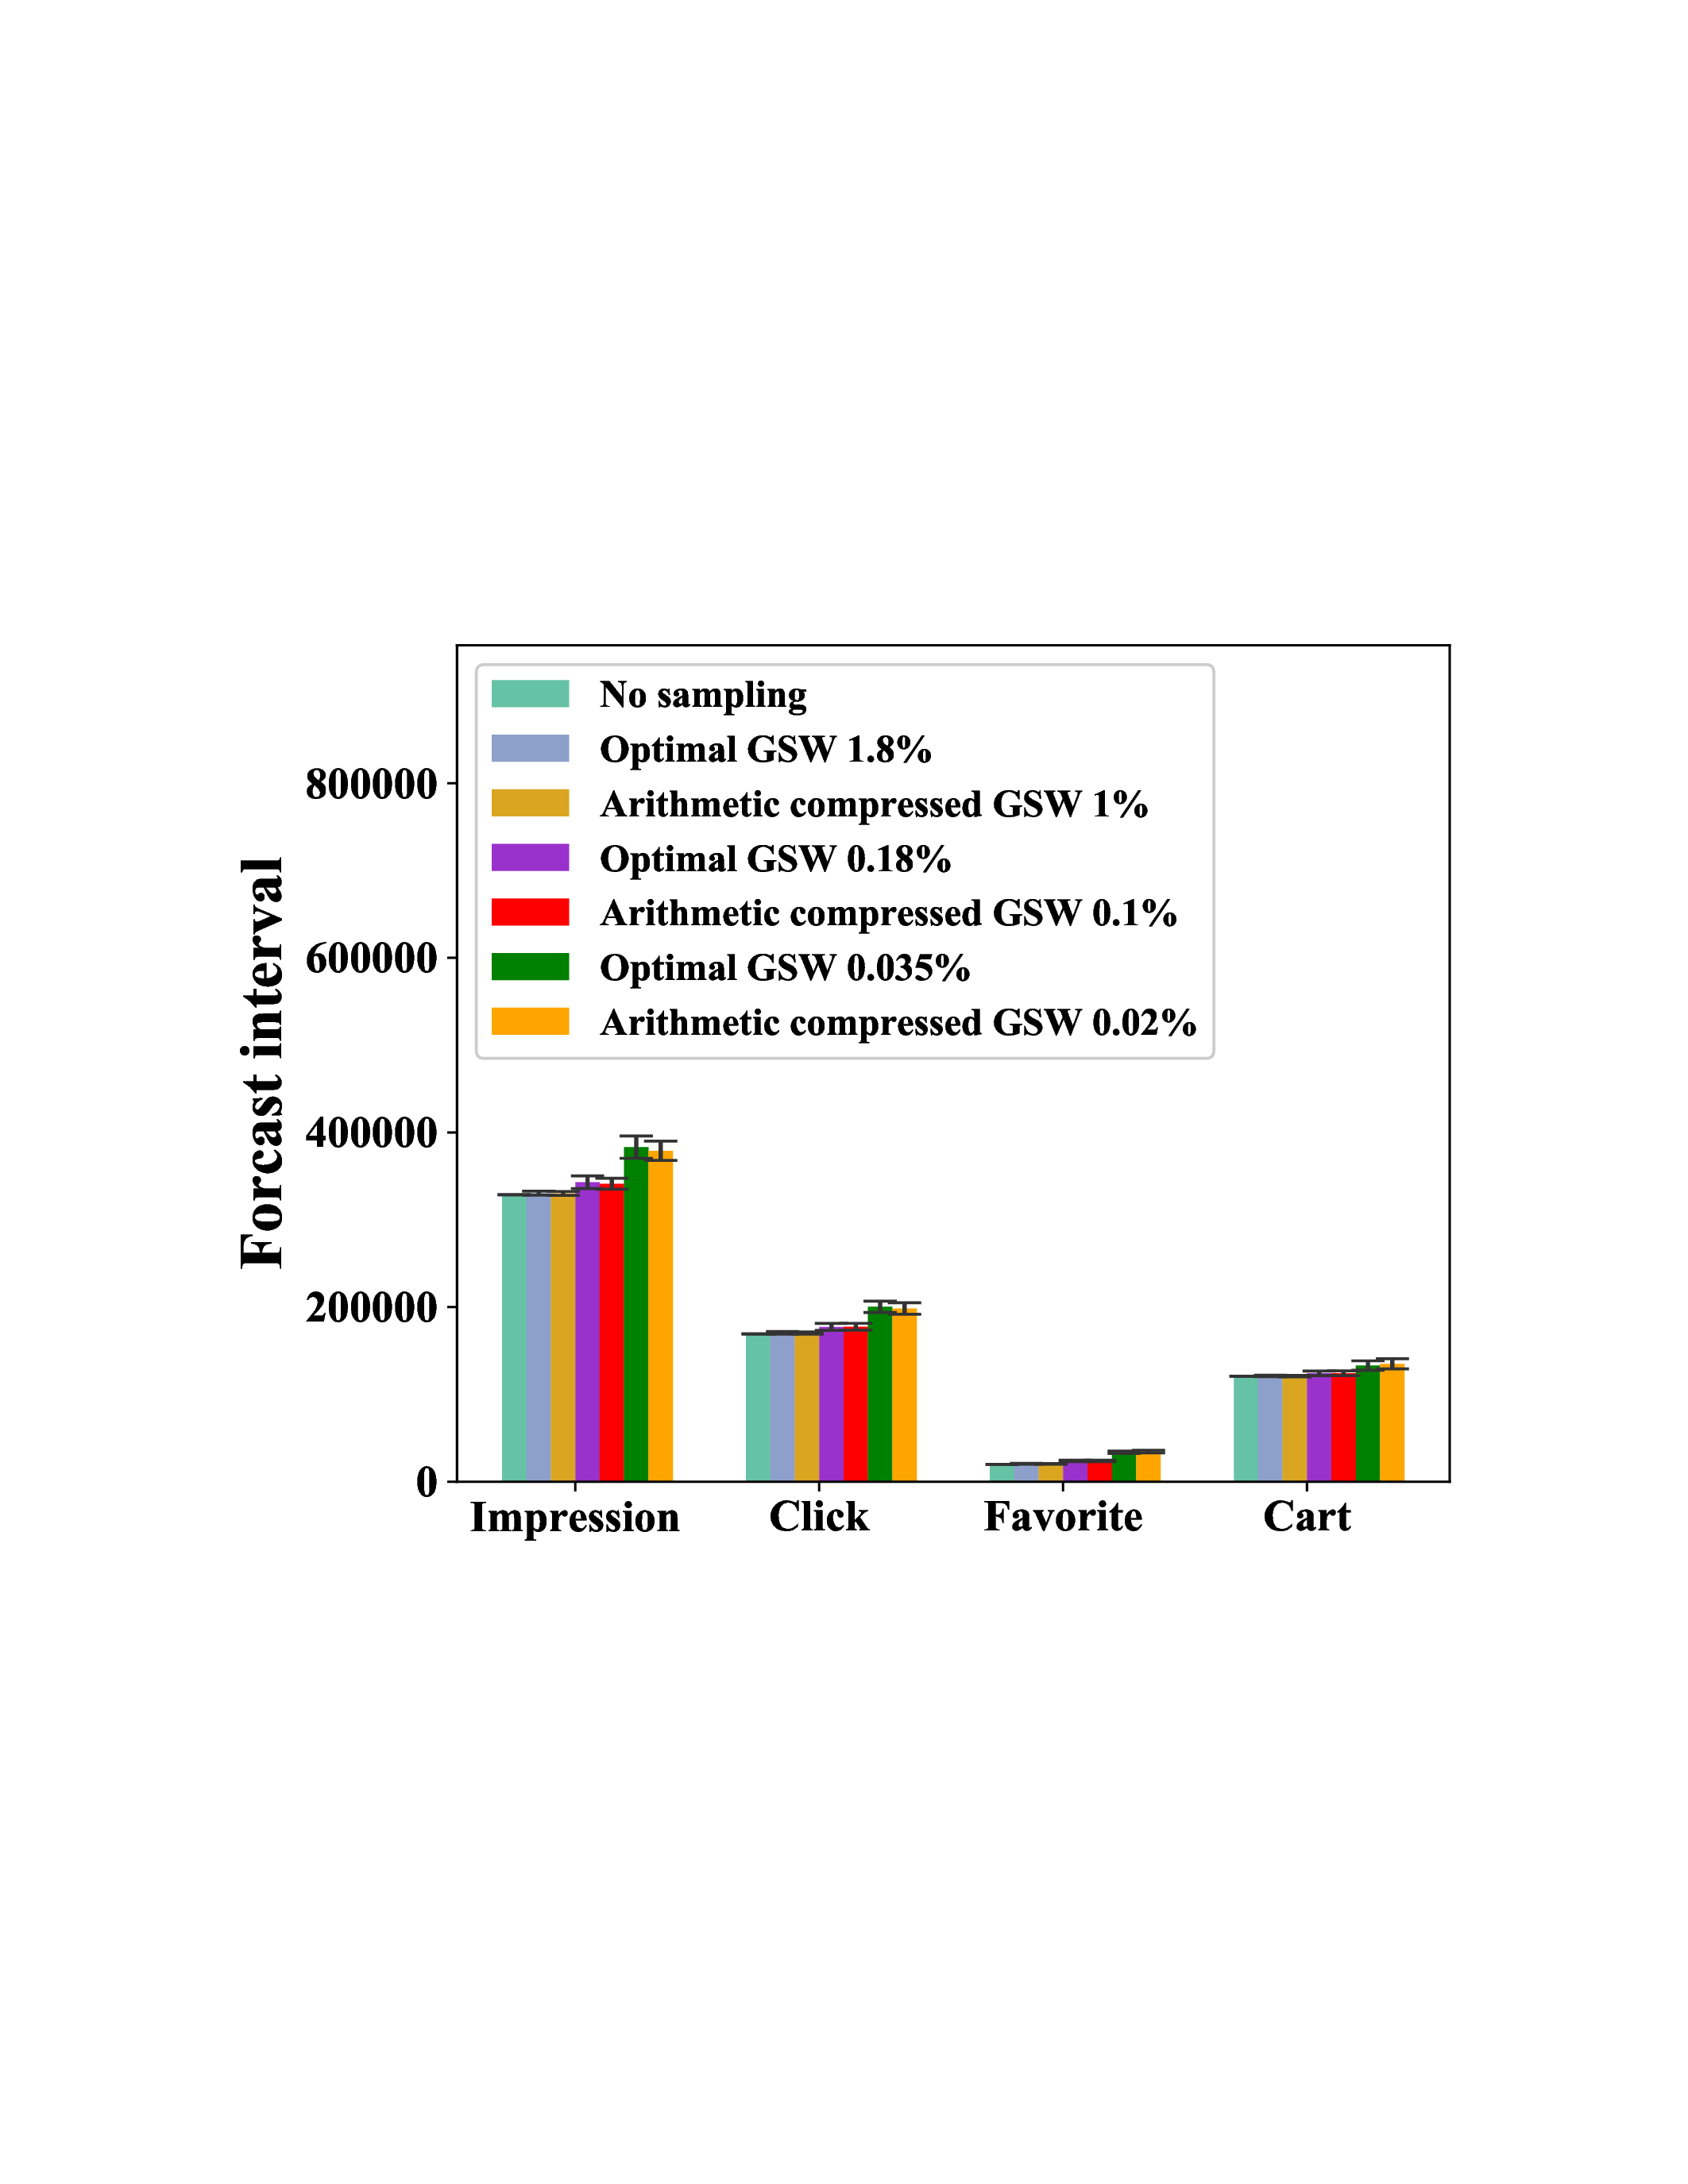}
\end{minipage}
}
\subfigure[Selectivity 5\%]{
\begin{minipage}[t]{0.33\linewidth}
\centering
\includegraphics[width=2.2in, height=2in]{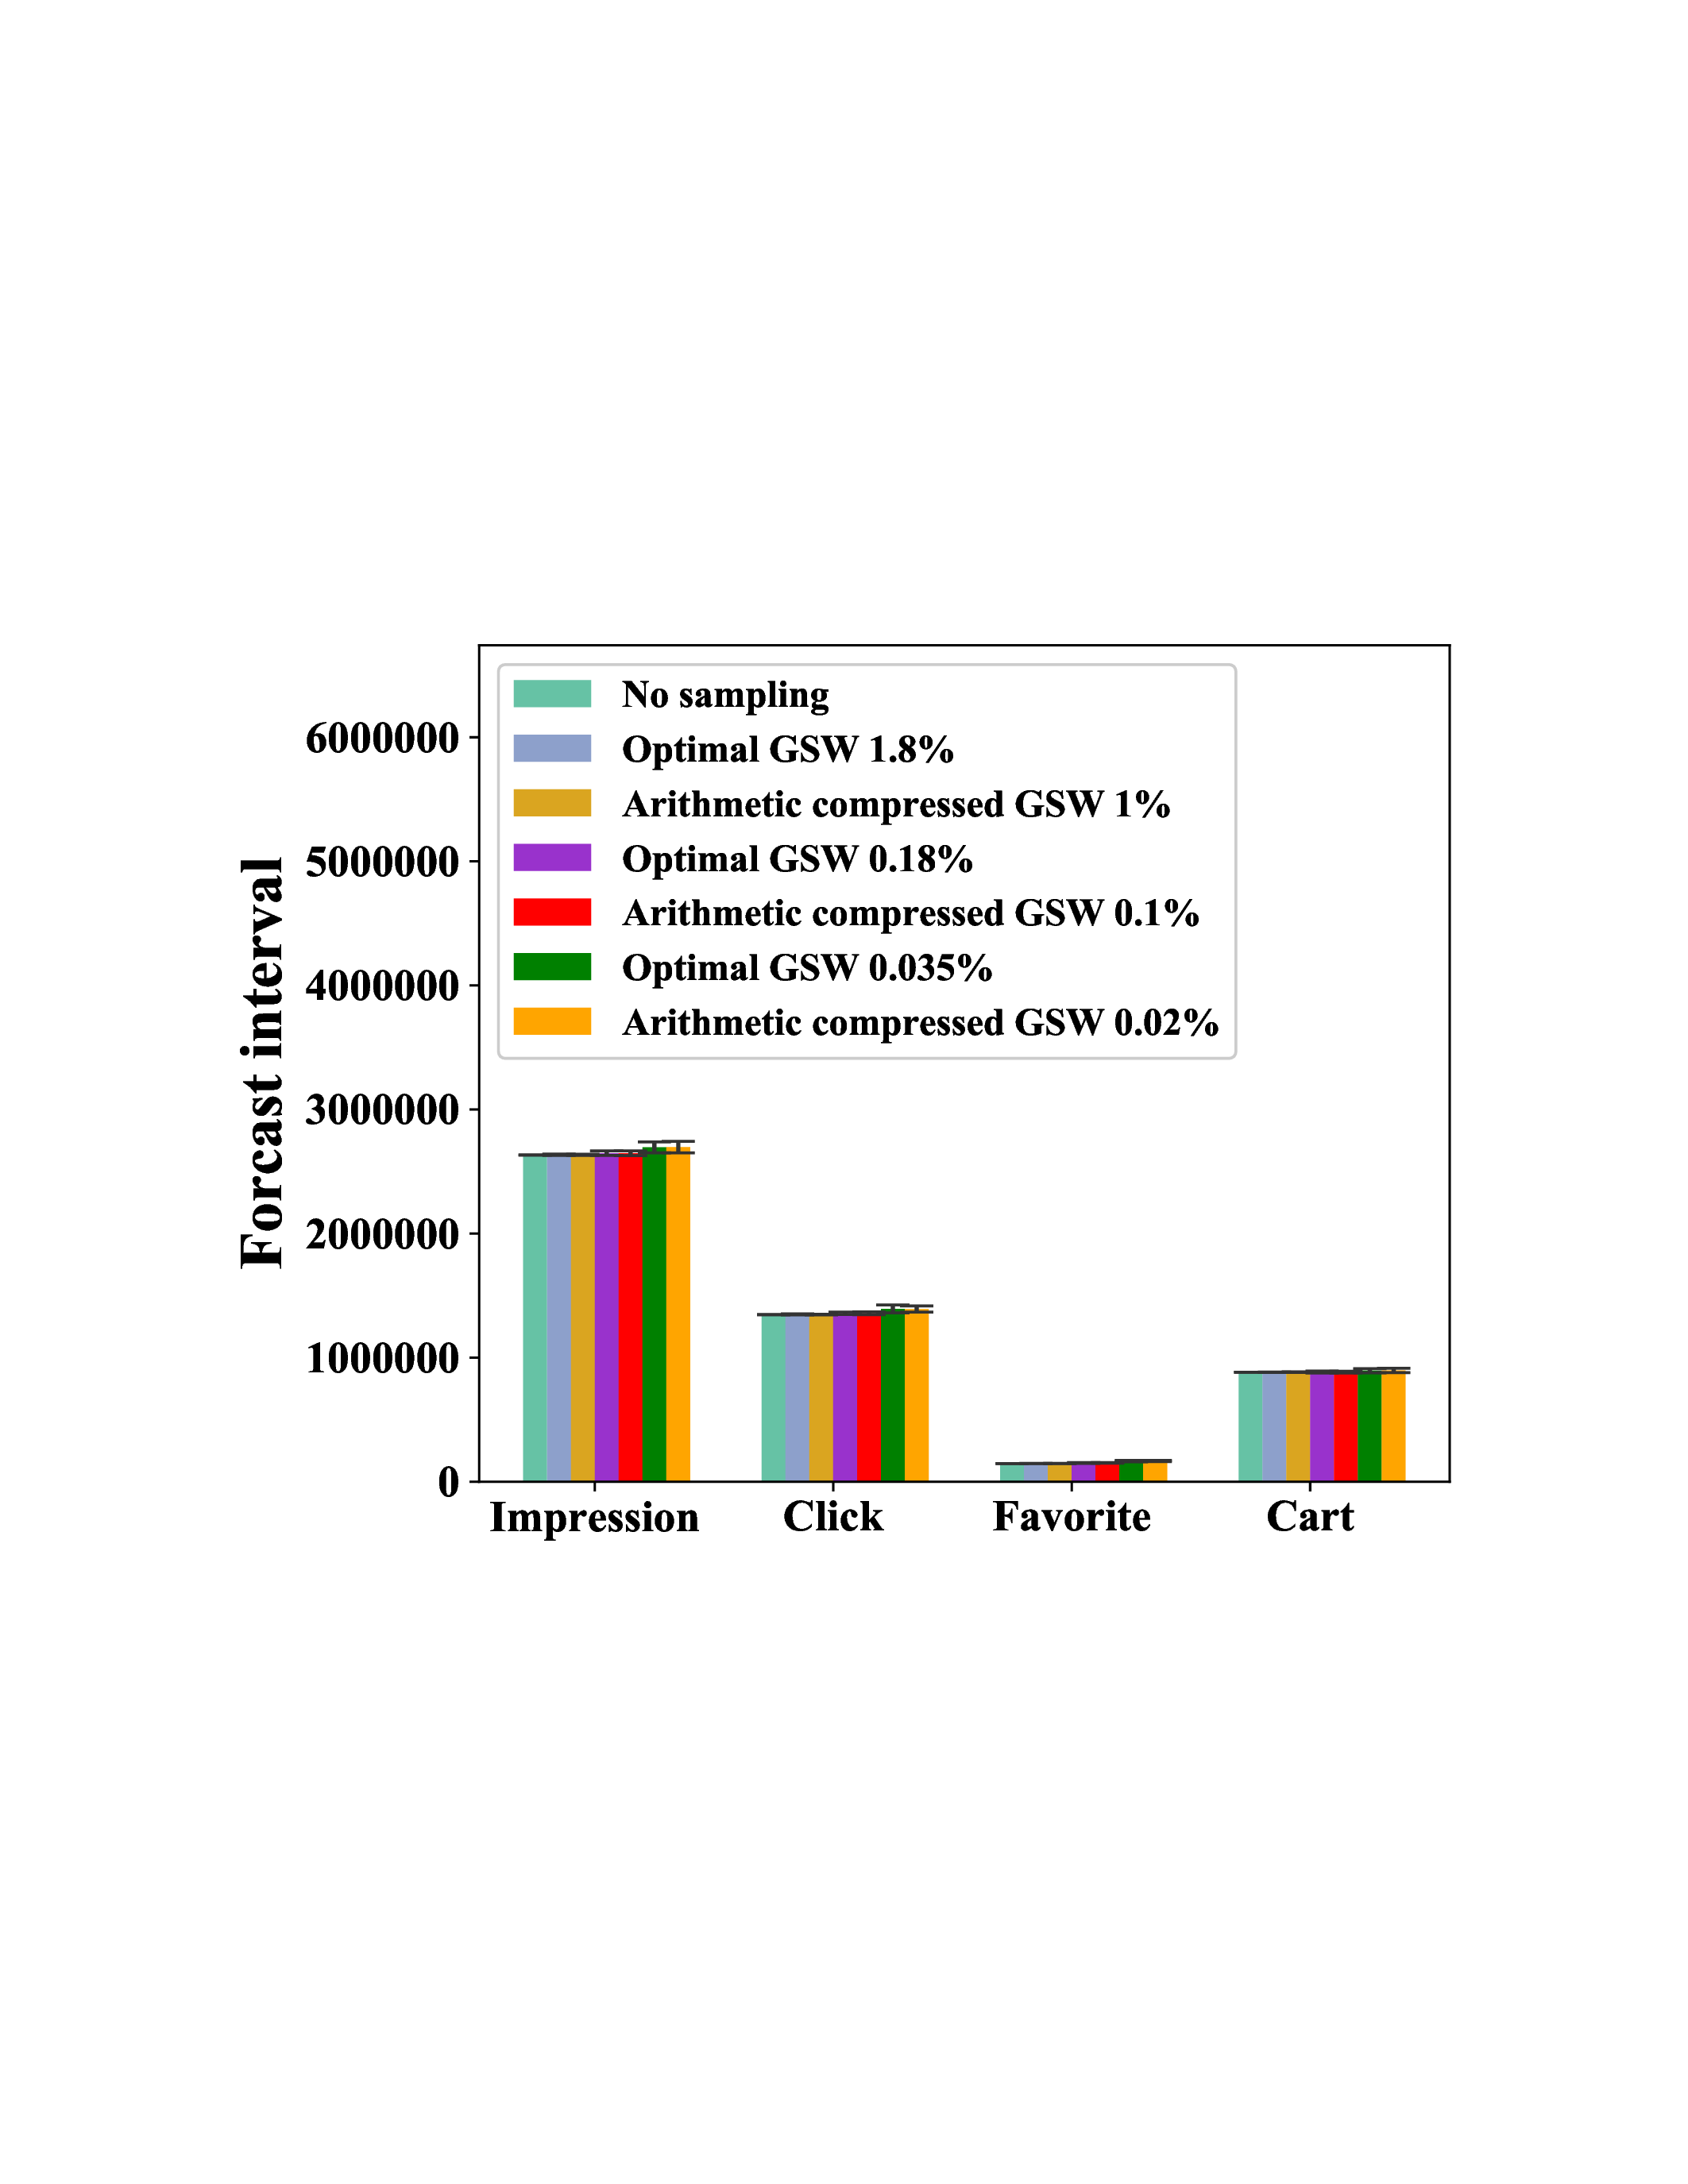}
\end{minipage}
}
\caption{ARIMA prediction interval with different selectivity via different sampling methods with nearly aqp error bound (can we add uniform and geometric-mean here? almost no change for different sampling rates? how can we guarantee that aqp error bounds are nearly the same given the same sampling rate?)}
% \label{AQP and ARIMA Performance}
\end{figure*}
